# Supplementary material for: Classification of second harmonic generation effect in magnetically ordered materials
Source: arXiv:2211.04354 ancillary file (2023-08-15)
Supplement: Supplementary file 1 [file SM.pdf]

# Supplemental Material for “Classification of second harmonic generation effect in magnetic materials”

Rui-Chun Xiao,<sup>1,\*</sup> Ding-Fu Shao,<sup>2</sup> Wei Gan,<sup>1</sup> Huan-Wen Wang,<sup>3</sup> Hui Han,<sup>1</sup> Z. G. Sheng,<sup>4</sup> Changjin Zhang,<sup>1,4</sup> Hua Jiang,<sup>5,†</sup> and Hui Li<sup>1,‡</sup>

<sup>1</sup>*Institute of Physical Science and Information Technology, Anhui University, Hefei 230601, China*

<sup>2</sup>*Key Laboratory of Materials Physics, Institute of Solid State Physics, Chinese Academy of Sciences, Hefei, 230031, China*

<sup>3</sup>*School of Physics, University of Electronic Science and Technology of China, Chengdu 610054, China*

<sup>4</sup>*High Magnetic Field Laboratory, HFIPS, Anhui, Chinese Academy of Sciences, Hefei 230031, China*

<sup>5</sup>*School of Physical Science and Technology, Soochow University, Suzhou 215006, China*

## Contents

|                                                                      |    |
|----------------------------------------------------------------------|----|
| <b>I. Lattice character directions of crystallographic systems</b>   | 2  |
| <b>II. Symmetry of linear magneto-optic effect in all MPGs</b>       | 2  |
| <b>III. Supplementary calculation results</b>                        | 4  |
| A. SHG of effect models with a honeycomb lattice                     | 4  |
| B. Magnetic and band structures of YMnO <sub>3</sub>                 | 6  |
| <b>IV. Symmetry of axial tensor using isomorphic group method</b>    | 8  |
| <b>V. Clarifications of SHG and LMO effects in MAGNDATA database</b> | 15 |
| <b>References</b>                                                    | 43 |

---

\*Electronic address: [xiaoruichun@ahu.edu.cn](mailto:xiaoruichun@ahu.edu.cn)

†Electronic address: [jianghuaphy@suda.edu.cn](mailto:jianghuaphy@suda.edu.cn)

‡Electronic address: [huili@ahu.edu.cn](mailto:huili@ahu.edu.cn)

## I. LATTICE CHARACTER DIRECTIONS OF CRYSTALLOGRAPHIC SYSTEMS

Since the symmetries of the tensors depend on the choice of the coordinate system, we introduce lattice character directions of crystallographic systems adopted in our work. One can also refer *International Tables for Crystallography* - Vol. A [1] for detail.

TABLE S1: Lattice character directions of 32 original point groups.

| Crystallographic system | Point Groups                                                    | Direction 1                        | Direction 2                                                         | Direction 3                                            |
|-------------------------|-----------------------------------------------------------------|------------------------------------|---------------------------------------------------------------------|--------------------------------------------------------|
| Cubic                   | $\bar{2}3$ , $m\bar{3}$ , $432$ , $\bar{4}3m$ , $m\bar{3}m$     | $\mathbf{a}/\mathbf{b}/\mathbf{c}$ | body diagonal<br><i>e.g.</i> $\mathbf{a} + \mathbf{b} + \mathbf{c}$ | face diagonal<br><i>e.g.</i> $\mathbf{a} + \mathbf{b}$ |
| Hexagonal               | $6$ , $\bar{6}$ , $6/m$ , $622$ , $6mm$ , $\bar{6}m2$ , $6/mmm$ | $\mathbf{c}$                       | $\mathbf{a}/\mathbf{b}$                                             | $\mathbf{a} + 2\mathbf{b}/2\mathbf{a} + \mathbf{b}$    |
| Tetragonal              | $4$ , $\bar{4}$ , $4/m$ , $422$ , $4mm$ , $\bar{4}2m$ , $4/mmm$ | $\mathbf{c}$                       | $\mathbf{a}/\mathbf{b}$                                             | face diagonal<br><i>e.g.</i> $\mathbf{a} + \mathbf{b}$ |
| Trigonal                | $3$ , $\bar{3}$ , $32$ , $3m$ , $\bar{3}m$                      | $\mathbf{c}$                       | $\mathbf{a}/\mathbf{b}$                                             | NA                                                     |
| Orthorhombic            | $222$ , $mm2$ , $mmm$                                           | $\mathbf{a}$                       | $\mathbf{b}$                                                        | $\mathbf{c}$                                           |
| Monoclinic              | $2$ , $m$ , $2/m$                                               | $\mathbf{b}$ (unique axis $b$ )    | NA                                                                  | NA                                                     |
| Triclinic               | $1$ , $\bar{1}$                                                 | NA                                 | NA                                                                  | NA                                                     |

1. 'NA' (not available) in the third to the fifth column denotes no symmetries along these character directions.
2. '/' in the third to the fifth column denotes there are two or more equivalent character directions.
3. The character directions for grey MPGs and black-white MPGs obey similar rules to original MPGs.

## II. SYMMETRY OF LINEAR MAGNETO-OPTIC EFFECT IN ALL MPGS

**Method 1:** In the linear regime, the light induces alternating current (AC) in materials,

$$j_i(\omega) = \sum_j \sigma_{ij}(\omega) E_j(\omega) \quad (1)$$

where  $\sigma_{ij}$  is the photoconductivity tensor. The transformation of  $\sigma_{ij}$  under the unitary operation is

$$R : \sigma_{ij} = \sum_{mn} R_{im} R_{jn} \sigma_{mn}. \quad (2)$$

The transformation of  $\sigma_{ij}$  under the anti-unitary operation is

$$R' : \sigma_{ij} = \sum_{mn} R_{im} R_{jn} \sigma_{nm}. \quad (3)$$

Eq. (3) satisfy the Onsager reciprocal relationship  $1'\sigma_{ij} = \sigma_{ji}$ . With the above relationship (Eqs. (2) and (3)), we can drive the optical conductivity of every MPG. The full results of every MPG are studied in Ref. [2], and are listed in [Bilbao Crystallographic Server/MTENSOR](#).

Photoconductivity tensor  $[\sigma_{ij}]_{3 \times 3}$  has 9 elements, and it can be divided into two parts: symmetry part ( $\sigma_{ij}^S = \sigma_{ji}^S$ )

TABLE S2: MPG with magneto-optic effect, and corresponding asymmetry part and asymmetry part of photoconductivity.

| Crystallographic system | MPG                                                               | Axial vector $\mathbf{M}$ | Asymmetry part                                                                                                                       | Symmetry part                                                                                                                                                   |
|-------------------------|-------------------------------------------------------------------|---------------------------|--------------------------------------------------------------------------------------------------------------------------------------|-----------------------------------------------------------------------------------------------------------------------------------------------------------------|
| Triclinic               | $1, \bar{1}$                                                      | $(m_x, m_y, m_z)$         | $\begin{bmatrix} 0 & \sigma_{xy} & -\sigma_{zx} \\ -\sigma_{xy} & 0 & \sigma_{yz} \\ \sigma_{zx} & -\sigma_{yz} & 0 \end{bmatrix}_3$ | $\begin{bmatrix} \sigma_{xx} & \sigma_{xy} & \sigma_{xz} \\ \sigma_{xy} & \sigma_{yy} & \sigma_{yz} \\ \sigma_{xz} & \sigma_{yz} & \sigma_{zz} \end{bmatrix}_6$ |
| Monoclinic              | Original point group:<br>$2, 2/m (2//y), m (m \perp y)$           | $(0, m_y, 0)$             | $\begin{bmatrix} 0 & 0 & -\sigma_{zx} \\ 0 & 0 & 0 \\ \sigma_{zx} & 0 & 0 \end{bmatrix}_1$                                           | $\begin{bmatrix} \sigma_{xx} & 0 & \sigma_{xz} \\ 0 & \sigma_{yy} & 0 \\ \sigma_{xz} & 0 & \sigma_{zz} \end{bmatrix}_4$                                         |
|                         | Black-White group:<br>$2', m', 2'/m'$                             | $(m_x, 0, m_z)$           | $\begin{bmatrix} 0 & \sigma_{xy} & 0 \\ -\sigma_{xy} & 0 & \sigma_{yz} \\ 0 & -\sigma_{yz} & 0 \end{bmatrix}_2$                      |                                                                                                                                                                 |
| Orthorhombic            | Black-White group:<br>$2'2'2, m'm'2, m'm'm$                       | $(0, 0, m_z)$             | $\begin{bmatrix} 0 & \sigma_{xy} & 0 \\ -\sigma_{xy} & 0 & 0 \\ 0 & 0 & 0 \end{bmatrix}_1$                                           | $\begin{bmatrix} \sigma_{xx} & 0 & 0 \\ 0 & \sigma_{yy} & 0 \\ 0 & 0 & \sigma_{zz} \end{bmatrix}_3$                                                             |
|                         | Black-White group:<br>$m'm'2'$                                    | $(0, m_y, 0)$             | $\begin{bmatrix} 0 & 0 & -\sigma_{zx} \\ 0 & 0 & 0 \\ \sigma_{zx} & 0 & 0 \end{bmatrix}_1$                                           |                                                                                                                                                                 |
| Tetragonal,             | Original point group:<br>$4, 4, 4/m, 3, \bar{3}, 6, \bar{6}, 6/m$ | $(0, 0, m_z)$             | $\begin{bmatrix} 0 & \sigma_{xy} & 0 \\ -\sigma_{xy} & 0 & 0 \\ 0 & 0 & 0 \end{bmatrix}_1$                                           | $\begin{bmatrix} \sigma_{xx} & 0 & 0 \\ 0 & \sigma_{xx} & 0 \\ 0 & 0 & \sigma_{zz} \end{bmatrix}_2$                                                             |
| Trigonal,               | Black-White group:<br>$42'2', 4m'm', \bar{4}2'm', 4/mmm',$        |                           |                                                                                                                                      |                                                                                                                                                                 |
| Hexagonal               | $32', 3m', \bar{3}m', 62'2', 6m'm', \bar{6}m'2', 6/mmm'm'$        |                           |                                                                                                                                      |                                                                                                                                                                 |

with 6 independent elements and asymmetry part ( $\sigma_{ij}^A = -\sigma_{ji}^A$ ) with 3 independent elements. Accordingly,  $[\sigma_{ij}]_{3 \times 3}$  in Eq. (1) can be rewritten as

$$[\sigma_{ij}] = \begin{bmatrix} \sigma_{xx}^S & \sigma_{xy}^S & \sigma_{xz}^S \\ \sigma_{xy}^S & \sigma_{yy}^S & \sigma_{yz}^S \\ \sigma_{xz}^S & \sigma_{yz}^S & \sigma_{zz}^S \end{bmatrix} + \begin{bmatrix} 0 & \sigma_{xy}^A & -\sigma_{zx}^A \\ -\sigma_{xy}^A & 0 & \sigma_{yz}^A \\ \sigma_{zx}^A & -\sigma_{yz}^A & 0 \end{bmatrix} \quad (4)$$

The symmetry part is even under the time-reversal symmetry, and cannot lead to the linear magneto-optic effect (LMO). The LMO effect originates from the asymmetry part of optical conductivity  $\sigma_{ij}^A$  (anomalous photoconductivity), which satisfies  $\sigma_{ij}^A = -\sigma_{ji}^A$ .

**Method 2:** The asymmetry part in Eq. (4) has three independent elements, and it is odd under time-reversal symmetry, which can be viewed as a pseudo-vector (axial tensor)  $\mathbf{M} = (m_x, m_y, m_z)$ , where  $m_x \leftrightarrow \sigma_{yz}^A$ ,  $m_y \leftrightarrow \sigma_{zx}^A$ ,  $m_z \leftrightarrow \sigma_{xy}^A$ . According to the transformation rules of pseudo-vector,  $R$  and  $IR$  have the same symmetry constrain on  $\mathbf{M}$ :

$$IRM = R\mathbf{M}. \quad (5)$$

The improper rotation operation ( $IR$ ) act as a proper rotation operation ( $R$ ) for pseudo-vector, and this leads to the original point group of  $C_{nv}$  ( $2mm, 3m, 4mm, 6mm$ ),  $D_n$  ( $222, 32, 422, 622$ ),  $D_{nh}$  ( $mmm, \bar{6}m2, 4/mmm, 6/mmm$ ),  $D_{nd}$  ( $\bar{3}m, \bar{4}m2$ ) and cubic point groups  $T$  ( $23$ ),  $O$  ( $432$ ),  $T_d$  ( $\bar{4}3m$ ),  $T_h$  ( $m\bar{3}$ ),  $O_h$  ( $m\bar{3}m$ ) zero.

For the anti-unitary operation,

$$R'\mathbf{M} = -R\mathbf{M}, \quad (6)$$

because  $T$  operation reverses  $\mathbf{M}$ . According to Eq. (6), the pseudo-vector is zero for grey MPGs and black-white MPGs with  $PT$  ( $G' = S + IS'$ ) symmetry. Besides, the anti-unitary operation  $R'$  ( $R \geq 3$ ) also leads to the vanishing of the pseudo-vector  $\mathbf{M}$ .

Based on the above analysis, there are 31 MPGs (13 original MPGs and 18 black-white MPGs) have the nonzero asymmetry part of photoconductivity (i.e., linear magneto-optic effect), which are listed in Table S2. The results are consistent with that Refs. [3–5].

### III. SUPPLEMENTARY CALCULATION RESULTS

#### A. SHG of effect models with a honeycomb lattice

Here, we consider effect models with honeycomb lattice to explore the SHG types under magnetic groups, and the effect of magnetic moment and spin-orbit coupling (SOC) effect on SHG. To describe a Néel AFM magnetic structure with  $PT$  symmetry, as shown in Fig. S1(a) (with MSG of  $P6'/mm'm$ ). We use the following 4-bands Kane-Mele model [6] to describe it.

$$H = t \sum_{\langle ij \rangle \alpha} c_{i\alpha}^\dagger c_{j\alpha} + \lambda_M \sum_i (-1)^i c_i^\dagger s^z c_i + i\lambda_{SO} \sum_{\langle\langle ij \rangle\rangle} \nu_{ij} c_i^\dagger s^z c_j. \quad (7)$$

The first term in Eq. (7) is the nearest neighbor hopping, the second is the exchange Zeeman field, mimicking the Néel order with an out-of-plane easy axis, and the third term is the intrinsic SOC effect. Here,  $\nu_{ij} = (2/\sqrt{3}) (\mathbf{d}_1 \times \mathbf{d}_2) = \pm 1$ , where  $\mathbf{d}_1$  and  $\mathbf{d}_2$  are the unit vectors of the two bonds connecting site  $i$  to  $j$ , and  $s^z$  is the spin Pauli matrix.  $t=1$  eV,  $\lambda_M = 2$  eV, and  $\lambda_{SO} = 0.05$  eV, here. Due to the  $PT$  symmetry, the band structures are double degenerate as shown in Fig. S1(b). Besides, the time-reversal symmetry is broken as a result of the coupling of SOC effect and magnetism, and +K and -K valleys are nonequivalent [7, 8].

The SHG type of this Néel AFM belongs to the PT-wP according to our classification, where only the odd SHG parts exist. Its tensor is constrained by point group  $\bar{6}2m$  ( $D_{3h}$ ) according to the above symmetry analysis. The calculated nonzero SHG tensor are  $\chi_{xxx}^{\text{odd}} = -\chi_{xyy}^{\text{odd}} = -\chi_{yyx}^{\text{odd}} = -\chi_{yxy}^{\text{odd}}$ , as shown in Fig. S1(b). By switching the sign of  $\lambda_M$  in Eq. (7) to reverse the magnetic moments, and we find all the nonzero SHG tensor elements reverse accordingly, which is consistent with our symmetry analysis. The recently studied  $\text{CrI}_3$  [9–11],  $\text{MnPS}_3$  [12],  $\text{MnPSe}_3$  [13],  $\text{MnBi}_2\text{Te}_4$  [14], and  $\text{CrSBr}$  [15] also have the similar SHG character of the model in Eq. (7), because they belong to the same SHG types (PT-wP). The SHG responses in PT-wP are non-reciprocal, and are reversible by rotating magnetization direction. Besides, without the SOC effect [in Eq. (7)], the odd parts SHG vanish. This indicates that the SOC effect plays an important role in the SHG of magnetic materials (see the analysis in the Discussion parts). The stronger SOC makes the SHG contribute by magnetism more significant, such as  $\text{CrI}_3$  [10, 11] and  $\text{MnBi}_2\text{Te}_4$  [14].

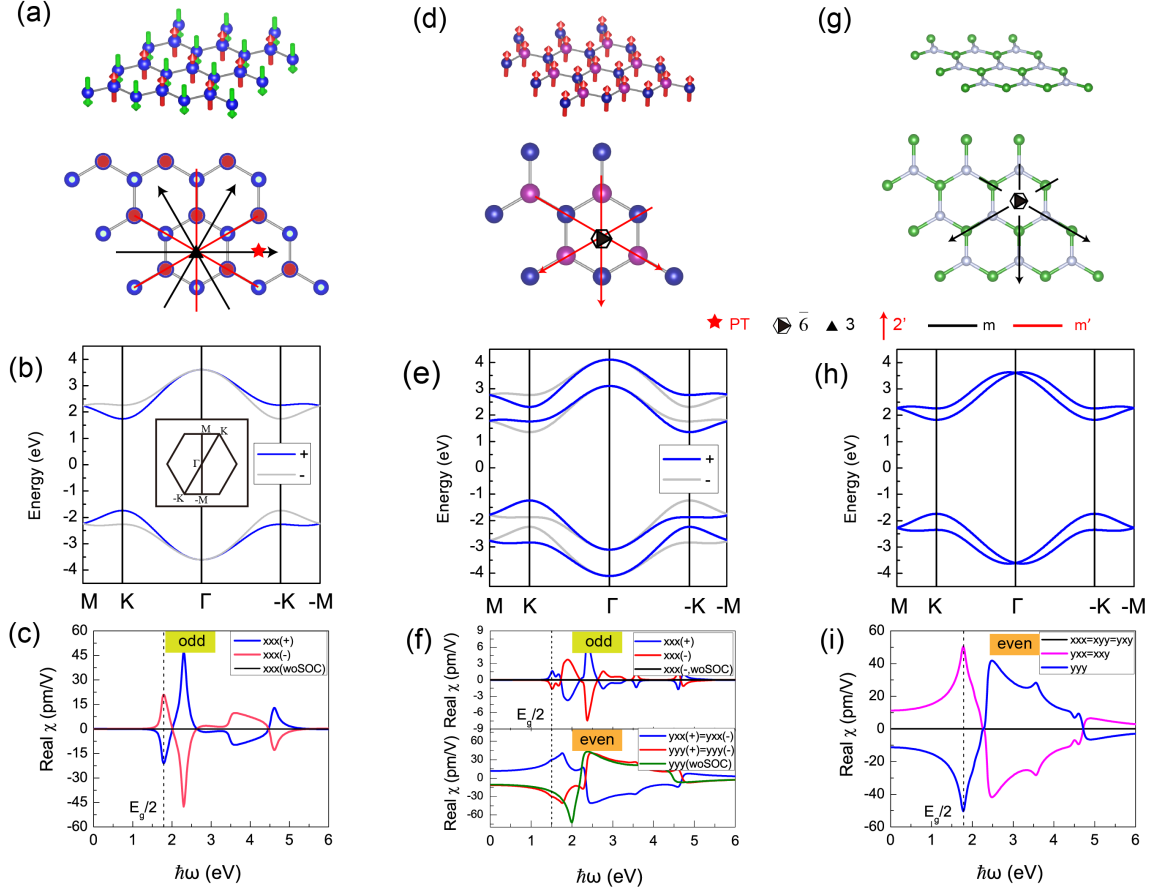

FIG. S1: SHG results of the effective model with 2D honeycomb lattice. (a) Crystal structure, (b) band structures, and (c) SHG (with PT-wP type) susceptibilities of Néel AFM with  $PT$  symmetry. (d) Crystal structure, (e) band structures, and (f) SHG (with BW-woP type) susceptibilities of FM without sub-lattice symmetry ( $\lambda_V = 2$  eV here). (d) Crystal structure, (e) band structures, and (f) SHG susceptibilities of nonmagnetic lattice ( $\lambda_M = 0$ ) without sub-lattice symmetry. The real and imaginary parts of SHG share the same symmetry, and the imaginary parts are not shown. The “+” and “-” signs in (c) and (f) represent the positive and negative magnetic structures.

The 2D ferromagnetic honeycomb model without sub-lattice inversion symmetry (with  $P\bar{6}m'2'$  symmetry, as shown in Fig. S1(d)) can be written as [16]

$$\begin{aligned}
 H = & t \sum_{\langle ij \rangle \alpha} c_{i\alpha}^\dagger c_{j\alpha} + \lambda_M \sum_i (-1)^i c_i^\dagger s^0 c_i + \lambda_V \sum_i (-1)^i c_i^\dagger s^0 c_i \\
 & + i\lambda_{SO} \sum_{\langle ij \rangle} \nu_{ij} c_i^\dagger s^z c_j + i\lambda_R \sum_{\langle ij \rangle} c_i^\dagger (\mathbf{s} \times \hat{\mathbf{d}}_{ij})_z c_j.
 \end{aligned} \tag{8}$$

The second term is the exchange Zeeman field which is different from Eq. (7), because it describes an FM exchange field. The third term breaks the sub-lattice inversion symmetry. The terms in the second line describe the SOC effect, and the first one is also presented in Eq. (7), and the second one describes the Rashba SOC effect, which is essential to get the nonzero SHG for 4-band model [17].  $t=1.0$  eV,  $\lambda_V = 1.0$  eV,  $\lambda_M = 0.5$  eV,  $\lambda_R = 0.2$  eV, and  $\lambda_{SO} = 0.05$  eV, here. Due to the lacking of inversion symmetry and ferromagnetism, the bands split, as shown in Fig. S1(e). According to its symmetry, we can judge its SHG type belongs to BW-woP, where the even and odd SHG coexist. The even parts SHG are constrained by the  $G_0 = \bar{6}m2$  symmetry, leading to  $\chi_{yyy}^{\text{even}} = -\chi_{yxx}^{\text{even}} = -\chi_{xyx}^{\text{even}} = -\chi_{xxy}^{\text{even}}$ .

While the odd parts are constrained by the  $G_1 = \bar{6}2m$  point group, and  $\chi_{xxx}^{\text{odd}} = -\chi_{xyy}^{\text{odd}} = -\chi_{yyx}^{\text{odd}} = -\chi_{yxx}^{\text{odd}}$  (the others are all zeros). The odd and even parts of tensor elements mutually repulse each other, because they are constrained by different symmetries. The calculated SHG results are shown in Fig. S1(f), which are consistent with our symmetry analysis. At the zero frequency limits, the even parts of SHG are nonzero, while the odd parts are zero, as shown in Fig. S1(f), which is consistent with the analysis in Section III-A of the maintext. Besides, the even SHG susceptibilities are invariant when the magnetism switches ( $\lambda_M \rightarrow -\lambda_M$ ), while the odd parts reverse. Without the SOC effect [the fourth and fifth terms of Eq. (8) are zeros], the odd parts of SHG become zeros, while the even parts of SHG survive.

The SG of the parent phase has no inversion symmetry, so the structure asymmetry contributes to the even parts of SHG, and can survive without magnetism. If  $\lambda_M = 0$  in Eq. (8), and it becomes a nonmagnetic 2D model without inversion symmetry, as shown in Fig. S1(g). Its band structures are shown in Fig. S1(h), where the band splits originate from the SOC effect and symmetry breaking of crystal structure. The band energies of  $+\mathbf{k}$  and  $-\mathbf{k}$  points are equivalent because the time-reversal symmetry links these two  $\mathbf{k}$  points. Only the even parts of the SHG survive, as shown in Fig. S1(i). Comparing Fig. S1(f) with Fig. S1(i), we find the magnitude of even parts SHG also change when  $\lambda_M$  is changed from nonzero to zero, therefore the magnetism contributes not only the odd parts of SHG but also the even parts.

### B. Magnetic and band structures of YMnO<sub>3</sub>

The crystal structure of RMnO<sub>3</sub> (R = Y, Sc, In, Ho, Er, Tm, Lu, Yb) is shown in Table S3, R atoms occupy 2a and 4b positions, Mn atoms occupy the 6c positions, and O atoms are at 6c positions. The magnetic structures of different magnetic phases are summarized in Table S4. The crystal structure of YMnO<sub>3</sub> refers to Ref. [18]. The band structure of YMnO<sub>3</sub> with different phase are shown in Fig. S2, where there are little differences between them, except for the degenerate and non-degenerate bands.

TABLE S3: Wyckoff Positions of space group  $P6_3cm$  (No. 185)

| Multiplicity | Wyckoff letter | Site Symmetry | Position                                                                          |
|--------------|----------------|---------------|-----------------------------------------------------------------------------------|
| 6            | <i>c</i>       | <i>m.</i>     | $(x,0,z)$ $(0,x,z)$ $(-x,-x,z)$<br>$(-x,0,z+1/2)$ $(0,-x,z+1/2)$<br>$(x,x,z+1/2)$ |
| 4            | <i>b</i>       | 3..           | $(1/3,2/3,z)$ $(2/3,1/3,z+1/2)$<br>$(1/3,2/3,z+1/2)$ $(2/3,1/3,z)$                |
| 2            | <i>a</i>       | 3 <i>m</i>    | $(0,0,z)$ $(0,0,z+1/2)$                                                           |

TABLE S4: Magnetic moment in each magnetic phase of YMnO<sub>3</sub>.

| Atom No. | Position          | $A_1$                   | $A_2$                   | $B_1$                   | $B_2$                   |
|----------|-------------------|-------------------------|-------------------------|-------------------------|-------------------------|
| 1        | $(x,0,z)$         | $(0,m,0)$               | $(m,0,0)$               | $(m,0,0)$               | $(0,m,0)$               |
| 2        | $(0,x,z)$         | $(-\sqrt{3}m/2,-m/2,0)$ | $(-m/2,\sqrt{3}m/2,0)$  | $(-m/2,\sqrt{3}m/2,z)$  | $(-\sqrt{3}m/2,-m/2,0)$ |
| 3        | $(1-x, 1-x, z)$   | $(\sqrt{3}m/2,-m/2,0)$  | $(-m/2,-\sqrt{3}m/2,0)$ | $(-m/2,-\sqrt{3}m/2,z)$ | $(\sqrt{3}m/2,-m/2,0)$  |
| 4        | $(1-x, 0, 0.5+z)$ | $(0,-m,0)$              | $(-m,0,0)$              | $(m,0,0)$               | $(0,m,0)$               |
| 5        | $(0, 1-x, 0.5+z)$ | $(\sqrt{3}m/2,m/2,0)$   | $(m/2,-\sqrt{3}m/2,0)$  | $(-m/2,\sqrt{3}m/2,z)$  | $(-\sqrt{3}m/2,-m/2,0)$ |
| 6        | $(x, x, 0.5+z)$   | $(-\sqrt{3}m/2,m/2,0)$  | $(m/2,\sqrt{3}m/2,0)$   | $(-m/2,-\sqrt{3}m/2,z)$ | $(\sqrt{3}m/2,-m/2,0)$  |

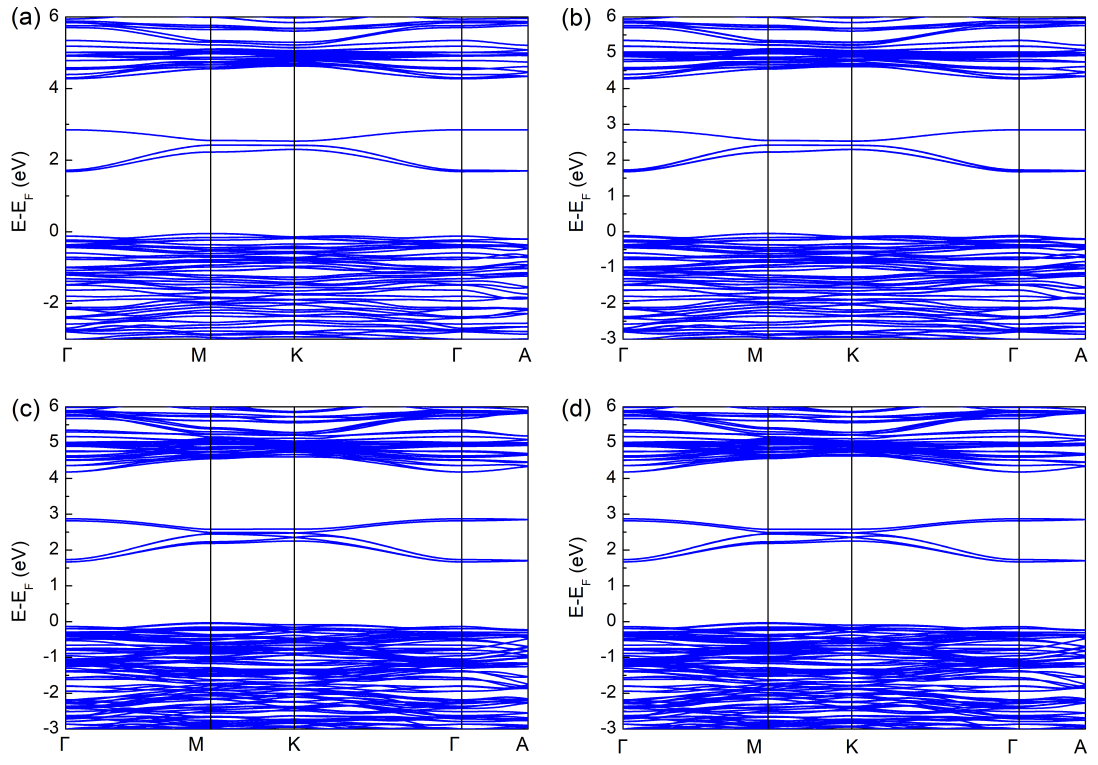

FIG. S2: Band structures of YMnO<sub>3</sub> with (a)  $A_1$ , (b)  $A_2$ , (c)  $B_1$  and (d)  $B_2$  phase, respectively.

#### IV. SYMMETRY OF AXIAL TENSOR USING ISOMORPHIC GROUP METHOD

The circular photogalvanic effect (CPGE) describes circular-polarization-light-induced photocurrent phenomenon, and it is a kind of optical rectification phenomenon. The CPGE coefficient  $\beta_{ij}$  is defined as:

$$\frac{dj_i}{dt} = \beta_{ij}(\omega)[\mathbf{E}(\omega) \times \mathbf{E}^*(\omega)]_j, \quad (9)$$

where the subscript  $i$  is the direction of photocurrent, and the subscript  $j$  is the spread direction of circular-polarization light. Besides, the magnetoelectric susceptibility  $\alpha_{ij}$  describes a linear response of the electric polarization to a magnetic field, and vice versa:

$$\begin{cases} P_i = \sum_j \alpha_{ij} H_j, \\ \mu_0 M_i = \sum_j \alpha_{ij} E_j. \end{cases} \quad (10)$$

The CPGE effect coefficient  $\beta_{ij}$  in Eq. (9) and magnetoelectric susceptibility  $\alpha_{ij}$  in Eq. (10) are all  $3 \times 3$  pseudo-tensors (axial tensor) which exist in systems without inversion symmetry. Because they obey similar symmetry constraint, we focus on the symmetry of CPGE  $\beta_{ij}$  in the following, and the results are also suitable to magnetoelectric susceptibility  $\alpha_{ij}$ .

Similar to SHG susceptibilities, we can divide  $\beta_{ij}$  into even and odd parts

$$\beta_{ij} = \beta_{ij}^{\text{even}} + \beta_{ij}^{\text{odd}}. \quad (11)$$

The unitary  $R$  and anti-unitary  $R'$  operations have the same restriction on tensor  $\beta^{\text{even}}$ :

$$R/R' : \beta^{\text{even}} = \det(R) R \beta^{\text{even}} R^{-1}, \quad (12)$$

where  $\det(R)$  is the determinant of operation  $R$ . The transformations of  $\beta^{\text{odd}}$  under the symmetry  $R$  and  $R'$  are

$$R/R' : \beta^{\text{odd}} = \pm \det(R) R \beta^{\text{odd}} R^{-1}, \quad (13)$$

where the positive sign corresponds to the unitary operation  $R$ , while the minus sign corresponds to the anti-unitary operation  $R'$ .

Because  $-1 = -(I_0)_{3 \times 3}$  ( $I_0$  is the identity matrix), i.e.,  $-1$  is identical to the matrix of inversion symmetry  $I$ , we can transform  $R'$  in Eq. (13) as

$$\begin{aligned} R' : \beta^{\text{odd}} &= -\det(R) R \beta^{\text{odd}} R^{-1} \\ &= \det(-R) (-R) \beta^{\text{odd}} (-R^{-1}) \\ &= \det(IR) (IR) \beta^{\text{odd}} (IR)^{-1}, \end{aligned} \quad (14)$$

i.e., anti-unitary operation  $R'$  is equivalent to a unitary operation  $IR$  for  $\beta^{\text{odd}}$ .

Similar to the SHG tensors, we can study the symmetry of CPGE tensor  $\beta$  in every MPG using the isomorphic group method.

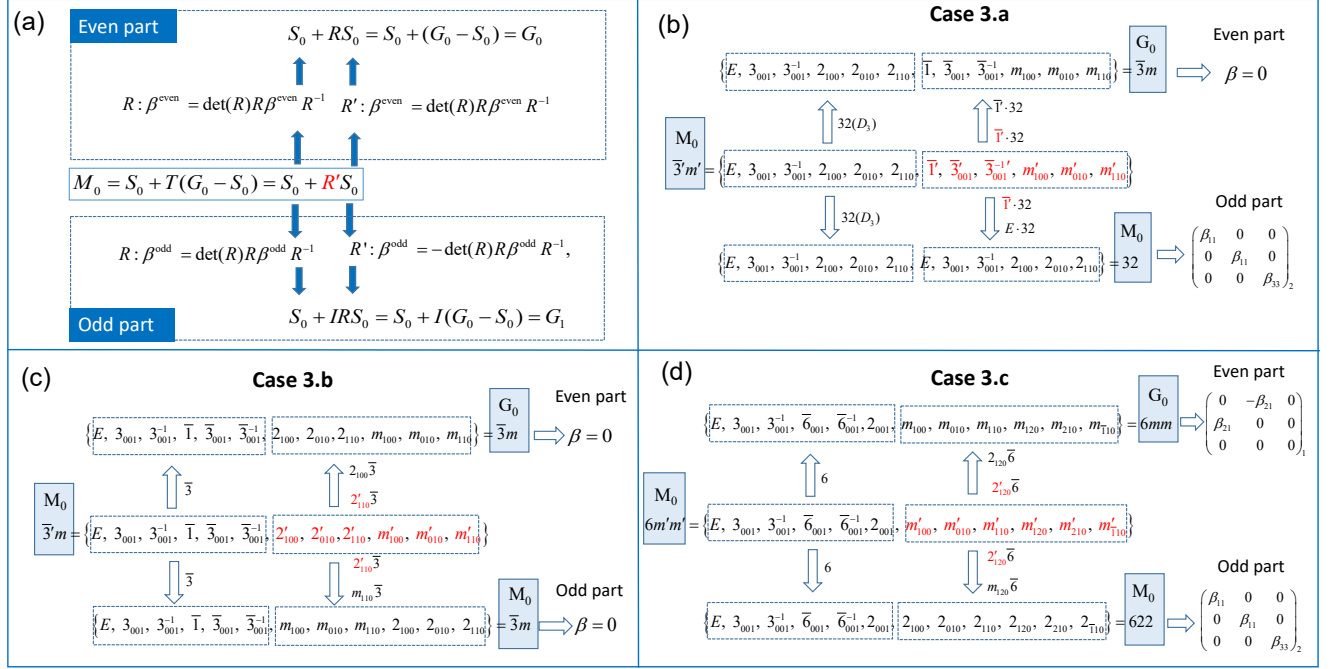

FIG. S3: Seeking the symmetry of axial tensor (CPGE tensor and magnetoelectric susceptibility)  $\beta$  in BW MPGs using the isomorphic group method. (a) Transformation of  $\beta_{ij}^{\text{even}}$  and  $\beta_{ij}^{\text{odd}}$  of BW MPG under unitary and anti-unitary operations, and corresponding isomorphic group. Examples for (b) BW MPG with  $PT$  symmetry, (c) BW MPG with  $P$  symmetry, (d) BW MPG without  $P$  nor  $PT$  symmetry.

(1) For the original point group  $M_0 = G_0$ , there is no anti-unitary symmetry operation, and the  $\beta_{ij}^{\text{even}}$  and  $\beta_{ij}^{\text{odd}}$  have the same symmetry restriction.

(2) For the grey MPGs,  $M_0 = G_0 + TG_0 = G_0 1'$  ( $1'$ : time-reversal symmetry), the combined restriction on  $R$  and  $R'$  leads to the vanish of  $\beta_{ij}^{\text{odd}}$ , and  $\beta_{ij}^{\text{even}}$  is restricted by  $G_0$  equivalently.

(3) For the black-white groups  $M_0 = G_0 + T(G_0 - S_0) = S_0 + R'S_0$ , we can also divide them into three sub-cases:

(3.a) MPG  $M_0$  has the  $PT$  symmetry. The  $\beta_{ij}^{\text{even}}$  vanishes, because  $\bar{1}'$  ( $PT$  symmetry) acts as the inversion symmetry for  $\beta_{ij}^{\text{even}}$ . For the odd part, the symmetry constrain is equivalent to  $G_1 = S_0 + (II)S_0 = S_0$ , if  $\bar{1}' \in R'S_0$ .

(3.b)  $M_0$  has the  $P$  symmetry. In this case, all of the even and odd CPGE tensors vanish due to existing inversion symmetry in  $M_0$ . Besides,  $G_1 = G_0$  according to the analysis in the main text.

(3.c)  $M_0$  has no  $P$  nor  $PT$  symmetry. In this case, both  $\beta_{ij}^{\text{even}}$  and  $\beta_{ij}^{\text{odd}}$  exist. Because the constraint of  $R'$  on the even part acts as a unitary operation  $R$ , the symmetry of  $\beta_{ij}^{\text{even}}$  under  $M_0$  equals to isomorphism point group  $G_0$ . On the other hand, the constraint of  $\beta_{ij}^{\text{odd}}$  under  $M_0$  is equivalent to point group  $G_1 = S_0 + IRS_0$ . Besides,  $G_1 \neq G_0$  (because  $\bar{1} \notin S_0$ ) and  $G_1 \neq S_0$  (because  $\bar{1}' \notin R'S_0$ ) in this case, i.e.  $G_0$  and  $G_1$  are the isomorphic relations.

See Fig. S3 for the three specific examples of the above three sub-cases (3.a, 3.b, and 3.c). The axial tensors (CPGE tensors and magnetoelectric susceptibility tensor) in original and grey MPGs are summarized in Table S5, and the axial tensors of 58 BW MPGs are summarized in Table S6. The results are consistent with Refs. [2] and [19];

moreover, our method simplifies the tensor symmetries under magnetic point groups into nonmagnetic points groups efficiently and captures symmetry rules.

TABLE S5: Axial tensors of original and grey magnetic point groups (MPGs) without inversion symmetry.

| MPG $M_0$                                                          | Axial tensor $[\beta_{ij}]_{3 \times 3}$                                                                                                               | MPG $M_0$                                                                                                          | Axial tensor $[\beta_{ij}]_{3 \times 3}$                                                                            |
|--------------------------------------------------------------------|--------------------------------------------------------------------------------------------------------------------------------------------------------|--------------------------------------------------------------------------------------------------------------------|---------------------------------------------------------------------------------------------------------------------|
| $\mathbf{1}$ (1.1.1)<br>$\mathbf{11}'$ (1.2.2)                     | $\begin{pmatrix} \beta_{11} & \beta_{12} & \beta_{13} \\ \beta_{21} & \beta_{22} & \beta_{23} \\ \beta_{31} & \beta_{32} & \beta_{33} \end{pmatrix}_9$ | $\mathbf{3}$ (16.1.60)<br>$\mathbf{31}'$ (16.2.61)                                                                 | $\begin{pmatrix} \beta_{11} & -\beta_{21} & 0 \\ \beta_{21} & \beta_{11} & 0 \\ 0 & 0 & \beta_{33} \end{pmatrix}_3$ |
| $\mathbf{2}$ (3.1.6)<br>$\mathbf{21}'$ (3.2.7)                     | $\begin{pmatrix} \beta_{11} & 0 & \beta_{13} \\ 0 & \beta_{22} & 0 \\ \beta_{31} & 0 & \beta_{33} \end{pmatrix}_5$                                     | $\mathbf{32}$ (18.1.65)<br>$\mathbf{321}'$ (18.2.66)                                                               | $\begin{pmatrix} \beta_{11} & 0 & 0 \\ 0 & \beta_{11} & 0 \\ 0 & 0 & \beta_{33} \end{pmatrix}_2$                    |
| $\mathbf{m}$ (4.1.9)<br>$\mathbf{m1}'$ (4.2.10)                    | $\begin{pmatrix} 0 & \beta_{12} & 0 \\ \beta_{21} & 0 & \beta_{23} \\ 0 & \beta_{32} & 0 \end{pmatrix}_4$                                              | $\mathbf{3m}$ (19.1.68)<br>$\mathbf{3m1}'$ (19.2.69)                                                               | $\begin{pmatrix} 0 & -\beta_{21} & 0 \\ \beta_{21} & 0 & 0 \\ 0 & 0 & 0 \end{pmatrix}_1$                            |
| $\mathbf{222}$ (6.1.17)<br>$\mathbf{2221}'$ (6.2.18)               | $\begin{pmatrix} \beta_{11} & 0 & 0 \\ 0 & \beta_{22} & 0 \\ 0 & 0 & \beta_{33} \end{pmatrix}_3$                                                       | $\mathbf{6}$ (21.1.76)<br>$\mathbf{61}'$ (21.2.77)                                                                 | $\begin{pmatrix} \beta_{11} & -\beta_{21} & 0 \\ \beta_{21} & \beta_{11} & 0 \\ 0 & 0 & \beta_{33} \end{pmatrix}_3$ |
| $\mathbf{mm2}$ (7.1.20)<br>$\mathbf{mm21}'$ (7.2.21)               | $\begin{pmatrix} 0 & \beta_{12} & 0 \\ \beta_{21} & 0 & 0 \\ 0 & 0 & 0 \end{pmatrix}_2$                                                                | $\bar{\mathbf{6}}$ (22.1.79)<br>$\bar{\mathbf{61}}'$ (22.2.80)                                                     | $\beta=0$                                                                                                           |
| $\mathbf{4}$ (9.1.29)<br>$\mathbf{41}'$ (9.2.30)                   | $\begin{pmatrix} \beta_{11} & -\beta_{21} & 0 \\ \beta_{21} & \beta_{11} & 0 \\ 0 & 0 & \beta_{33} \end{pmatrix}_3$                                    | $\mathbf{622}$ (24.1.87)<br>$\mathbf{6221}'$ (24.2.88)                                                             | $\begin{pmatrix} \beta_{11} & 0 & 0 \\ 0 & \beta_{11} & 0 \\ 0 & 0 & \beta_{33} \end{pmatrix}_2$                    |
| $\bar{\mathbf{4}}$ (10.1.32)<br>$\bar{\mathbf{41}}'$ (10.2.33)     | $\begin{pmatrix} \beta_{11} & \beta_{21} & 0 \\ \beta_{21} & -\beta_{11} & 0 \\ 0 & 0 & 0 \end{pmatrix}_2$                                             | $\mathbf{6mm}$ (25.1.91)<br>$\mathbf{6mm1}'$ (25.2.92)                                                             | $\begin{pmatrix} 0 & -\beta_{21} & 0 \\ \beta_{21} & 0 & 0 \\ 0 & 0 & 0 \end{pmatrix}_1$                            |
| $\mathbf{422}$ (12.1.40)<br>$\mathbf{4221}'$ (12.2.41)             | $\begin{pmatrix} \beta_{11} & 0 & 0 \\ 0 & \beta_{11} & 0 \\ 0 & 0 & \beta_{33} \end{pmatrix}_3$                                                       | $\bar{\mathbf{6m2}}$ (26.1.95)<br>$\bar{\mathbf{6m21}}'$ (26.2.96)                                                 | $\beta=0$                                                                                                           |
| $\mathbf{4mm}$ (13.1.44)<br>$\mathbf{4mm1}'$ (13.2.45)             | $\begin{pmatrix} 0 & -\beta_{21} & 0 \\ \beta_{21} & 0 & 0 \\ 0 & 0 & 0 \end{pmatrix}_1$                                                               | $\mathbf{23}$ (28.1.107)<br>$\mathbf{231}'$ (28.2.108)<br>$\mathbf{432}$ (30.1.112)<br>$\mathbf{4321}'$ (30.2.113) | $\begin{pmatrix} \beta_{11} & 0 & 0 \\ 0 & \beta_{11} & 0 \\ 0 & 0 & \beta_{11} \end{pmatrix}_1$                    |
| $\bar{\mathbf{42m}}$ (14.1.48)<br>$\bar{\mathbf{42m1}}'$ (14.2.49) | $\begin{pmatrix} \beta_{11} & 0 & 0 \\ 0 & -\beta_{11} & 0 \\ 0 & 0 & 0 \end{pmatrix}_1$                                                               | $\bar{\mathbf{43m}}$ (31.1.115)<br>$\bar{\mathbf{43m1}}'$ (31.2.116)                                               | $\beta=0$                                                                                                           |

1. There is only the even part ( $\beta^{\text{even}}$ ) for grey MPGs (the second one of each row, with  $1'$ ), and the odd and even parts ( $\beta^{\text{even}}$ ) and  $\beta^{\text{odd}}$  have same symmetry in original MPGs (the first MPG of each row, without  $1'$ ).
2. The subscript number of the tensor means the independent element number.
3.  $[\beta_{ij}]_{3 \times 3}$  is zero for the original and grey groups not listed here because they have the inversion symmetry.

TABLE S6: Axial tensors of all BW MPGs. Note: (1) MPG  $M_0 = S_0 + T(G_0 - S_0) = S_0 + \mathbf{R}'S_0$ , where  $G_0$  is the isomorphism non-magnetic point group, and  $S_0$  is the invariant subgroup of point group  $G_0$  ( $s = g/2$ ,  $s$  and  $g$  are the order of group  $S_0$  and  $G_0$  respectively). (2) The subscript number of each axial tensor means the independent element number.

| MPG $M_0$                   | Isomorphic PG $G_0$ | $S_0$          | $\mathbf{R}'$    | $G_0$ and $[\beta_{ij}^{\text{even}}]_{3 \times 3}$                                                                        | $G_1$ and $[\beta_{ij}^{\text{odd}}]_{3 \times 3}$                                                                                                                  |
|-----------------------------|---------------------|----------------|------------------|----------------------------------------------------------------------------------------------------------------------------|---------------------------------------------------------------------------------------------------------------------------------------------------------------------|
| $\bar{1}'$<br>(2.3.5)       | $\bar{1}$           | 1              | $\bar{1}'$       | $\bar{1}$<br>$\beta=0$                                                                                                     | $\bar{1}$<br>$\begin{pmatrix} \beta_{11} & \beta_{12} & \beta_{13} \\ \beta_{21} & \beta_{22} & \beta_{23} \\ \beta_{31} & \beta_{32} & \beta_{33} \end{pmatrix}_9$ |
| $2'(2//y)$<br>(3.3.8)       | 2                   | 1              | $2'_{010}$       | $2$<br>$\begin{pmatrix} \beta_{11} & 0 & \beta_{13} \\ 0 & \beta_{22} & 0 \\ \beta_{31} & 0 & \beta_{33} \end{pmatrix}_5$  | $m$<br>$\begin{pmatrix} 0 & \beta_{12} & 0 \\ \beta_{21} & 0 & \beta_{23} \\ 0 & \beta_{32} & 0 \end{pmatrix}_4$                                                    |
| $m'(m \perp y)$<br>(4.3.11) | $m(m \perp y)$      | 1              | $m'_{010}$       | $m$<br>$\begin{pmatrix} 0 & \beta_{12} & 0 \\ \beta_{21} & 0 & \beta_{23} \\ 0 & \beta_{32} & 0 \end{pmatrix}_4$           | $2$<br>$\begin{pmatrix} \beta_{11} & 0 & \beta_{13} \\ 0 & \beta_{22} & 0 \\ \beta_{31} & 0 & \beta_{33} \end{pmatrix}_5$                                           |
| $2'/m(2//y)$<br>(5.3.14)    | $2/m$               | $m$            | $\bar{1}'$       | $2/m$<br>$\beta=0$                                                                                                         | $m$<br>$\begin{pmatrix} 0 & \beta_{12} & 0 \\ \beta_{21} & 0 & \beta_{23} \\ 0 & \beta_{32} & 0 \end{pmatrix}_4$                                                    |
| $2/m'(2//y)$<br>(5.4.15)    | $2/m$               | 2              | $\bar{1}'$       | $2/m$<br>$\beta=0$                                                                                                         | $2$<br>$\begin{pmatrix} \beta_{11} & 0 & \beta_{13} \\ 0 & \beta_{22} & 0 \\ \beta_{31} & 0 & \beta_{33} \end{pmatrix}_5$                                           |
| $2'/m'(2//y)$<br>(5.5.16)   | $2/m$               | $\bar{1}$      | $2'$             | $2/m$<br>$\beta=0$                                                                                                         | $2/m$<br>$\beta=0$                                                                                                                                                  |
| $2'2'2$<br>(6.3.19)         | 222                 | 2 (2//z)       | $2'_{100}$       | $222$<br>$\begin{pmatrix} \beta_{11} & 0 & 0 \\ 0 & \beta_{22} & 0 \\ 0 & 0 & \beta_{33} \end{pmatrix}_3$                  | $mm2$<br>$\begin{pmatrix} 0 & \beta_{12} & 0 \\ \beta_{21} & 0 & 0 \\ 0 & 0 & 0 \end{pmatrix}_2$                                                                    |
| $m'm2'(2//z)$<br>(7.3.22)   | $mm2$               | $m(m \perp y)$ | $2'_{001}$       | $mm2$<br>$\begin{pmatrix} 0 & \beta_{12} & 0 \\ \beta_{21} & 0 & 0 \\ 0 & 0 & 0 \end{pmatrix}_2$                           | $2mm$<br>$\begin{pmatrix} 0 & 0 & 0 \\ 0 & 0 & \beta_{32} \\ 0 & \beta_{23} & 0 \end{pmatrix}_2$                                                                    |
| $m'm'2$<br>(7.4.23)         | $mm2$               | 2 (2//z)       | $m'_{100}$       | $mm2$<br>$\begin{pmatrix} 0 & \beta_{12} & 0 \\ \beta_{21} & 0 & 0 \\ 0 & 0 & 0 \end{pmatrix}_2$                           | $222$<br>$\begin{pmatrix} \beta_{11} & 0 & 0 \\ 0 & \beta_{22} & 0 \\ 0 & 0 & \beta_{33} \end{pmatrix}_3$                                                           |
| $mmm'$<br>(8.3.26)          | $mmm$               | $mm2$          | $\bar{1}'$       | $mmm$<br>$\beta=0$                                                                                                         | $mm2$<br>$\begin{pmatrix} 0 & \beta_{12} & 0 \\ \beta_{21} & 0 & 0 \\ 0 & 0 & 0 \end{pmatrix}_2$                                                                    |
| $m'm'm$<br>(8.4.27)         | $mmm$               | $2/m(2//z)$    | $m'_{100}$       | $mmm$<br>$\beta=0$                                                                                                         | $mmm$<br>$\beta=0$                                                                                                                                                  |
| $m'm'm'$<br>(8.5.28)        | $mmm$               | 222            | $\bar{1}'$       | $mmm$<br>$\beta=0$                                                                                                         | $222$<br>$\begin{pmatrix} \beta_{11} & 0 & 0 \\ 0 & \beta_{22} & 0 \\ 0 & 0 & \beta_{33} \end{pmatrix}_3$                                                           |
| $4'$<br>(9.3.31)            | 4                   | 2 (2//z)       | $4'_{001}$       | $4$<br>$\begin{pmatrix} \beta_{11} & -\beta_{21} & 0 \\ \beta_{21} & \beta_{11} & 0 \\ 0 & 0 & \beta_{33} \end{pmatrix}_3$ | $4$<br>$\begin{pmatrix} \beta_{11} & \beta_{21} & 0 \\ \beta_{21} & -\beta_{11} & 0 \\ 0 & 0 & 0 \end{pmatrix}_2$                                                   |
| $\bar{4}'$<br>(10.3.34)     | $\bar{4}$           | 2 (2//z)       | $\bar{4}'_{001}$ | $\bar{4}$<br>$\begin{pmatrix} \beta_{11} & \beta_{21} & 0 \\ \beta_{21} & -\beta_{11} & 0 \\ 0 & 0 & 0 \end{pmatrix}_2$    | $4$<br>$\begin{pmatrix} \beta_{11} & -\beta_{21} & 0 \\ \beta_{21} & \beta_{11} & 0 \\ 0 & 0 & \beta_{33} \end{pmatrix}_3$                                          |
| $4'/m$<br>(11.3.37)         | $4/m$               | $2/m$          | $4'_{001}$       | $4/m$<br>$\beta=0$                                                                                                         | $4/m$<br>$\beta=0$                                                                                                                                                  |

Continued on next page

TABLE S6 – continued from previous page

| MPG $M_0$                           | Isomorphic PG $G_0$ | $S_0$       | $R'$       | $G_0$ and $[\beta_{ij}^{\text{even}}]_{3 \times 3}$                                                          | $G_1$ and $[\beta_{ij}^{\text{odd}}]_{3 \times 3}$                                                                            |
|-------------------------------------|---------------------|-------------|------------|--------------------------------------------------------------------------------------------------------------|-------------------------------------------------------------------------------------------------------------------------------|
| $\frac{4}{m'}$<br>(11.4.38)         | $4/m$               | 4           | $\bar{1}'$ | $\frac{4}{m}$<br>$\beta=0$                                                                                   | $\frac{4}{\begin{pmatrix} \beta_{11} & -\beta_{21} & 0 \\ \beta_{21} & \beta_{11} & 0 \\ 0 & 0 & \beta_{33} \end{pmatrix}_3}$ |
| $\frac{4'}{m'}$<br>(11.5.39)        | $4/m$               | $\bar{4}$   | $\bar{1}'$ | $\frac{4}{m}$<br>$\beta=0$                                                                                   | $\frac{4}{\begin{pmatrix} \beta_{11} & \beta_{21} & 0 \\ \beta_{21} & -\beta_{11} & 0 \\ 0 & 0 & 0 \end{pmatrix}_2}$          |
| $\frac{4'22'}{}$<br>(12.3.42)       | 422                 | 222         | $4'_{001}$ | $\frac{422}{\begin{pmatrix} \beta_{11} & 0 & 0 \\ 0 & \beta_{11} & 0 \\ 0 & 0 & \beta_{33} \end{pmatrix}_3}$ | $\frac{42m}{\begin{pmatrix} \beta_{11} & 0 & 0 \\ 0 & -\beta_{11} & 0 \\ 0 & 0 & 0 \end{pmatrix}_1}$                          |
| $\frac{42'2'}{}$<br>(12.4.43)       | 422                 | 4           | $2'_{100}$ | $\frac{422}{\begin{pmatrix} \beta_{11} & 0 & 0 \\ 0 & \beta_{11} & 0 \\ 0 & 0 & \beta_{33} \end{pmatrix}_3}$ | $\frac{4mm}{\begin{pmatrix} 0 & -\beta_{21} & 0 \\ \beta_{21} & 0 & 0 \\ 0 & 0 & 0 \end{pmatrix}_1}$                          |
| $\frac{4'm'm}{}$<br>(13.3.46)       | $4mm$               | $2mm$       | $4'_{001}$ | $\frac{4mm}{\begin{pmatrix} 0 & -\beta_{21} & 0 \\ \beta_{21} & 0 & 0 \\ 0 & 0 & 0 \end{pmatrix}_1}$         | $\frac{42m}{\begin{pmatrix} \beta_{11} & 0 & 0 \\ 0 & -\beta_{11} & 0 \\ 0 & 0 & 0 \end{pmatrix}_1}$                          |
| $\frac{4m'm'}{}$<br>(13.4.47)       | $4mm$               | 4           | $m'_{100}$ | $\frac{4mm}{\begin{pmatrix} 0 & -\beta_{21} & 0 \\ \beta_{21} & 0 & 0 \\ 0 & 0 & 0 \end{pmatrix}_1}$         | $\frac{422}{\begin{pmatrix} \beta_{11} & 0 & 0 \\ 0 & \beta_{11} & 0 \\ 0 & 0 & \beta_{33} \end{pmatrix}_3}$                  |
| $\frac{\bar{4}'2'm}{}$<br>(14.3.50) | $\bar{4}2m$         | $2mm$       | $\bar{4}'$ | $\frac{42m}{\begin{pmatrix} \beta_{11} & 0 & 0 \\ 0 & -\beta_{11} & 0 \\ 0 & 0 & 0 \end{pmatrix}_1}$         | $\frac{4mm}{\begin{pmatrix} 0 & -\beta_{21} & 0 \\ \beta_{21} & 0 & 0 \\ 0 & 0 & 0 \end{pmatrix}_1}$                          |
| $\frac{\bar{4}'2m'}{}$<br>(14.4.51) | $\bar{4}2m$         | 222         | $\bar{4}'$ | $\frac{42m}{\begin{pmatrix} \beta_{11} & 0 & 0 \\ 0 & -\beta_{11} & 0 \\ 0 & 0 & 0 \end{pmatrix}_1}$         | $\frac{422}{\begin{pmatrix} \beta_{11} & 0 & 0 \\ 0 & \beta_{11} & 0 \\ 0 & 0 & \beta_{33} \end{pmatrix}_3}$                  |
| $\frac{\bar{4}2'm'}{}$<br>(14.5.52) | $\bar{4}2m$         | $\bar{4}$   | $2'_{100}$ | $\frac{42m}{\begin{pmatrix} \beta_{11} & 0 & 0 \\ 0 & -\beta_{11} & 0 \\ 0 & 0 & 0 \end{pmatrix}_1}$         | $\frac{4m2}{\begin{pmatrix} 0 & \beta_{12} & 0 \\ \beta_{12} & 0 & 0 \\ 0 & 0 & 0 \end{pmatrix}_1}$                           |
| $\frac{4/m'mm}{}$<br>(15.3.55)      | $4/mmm$             | $4mm$       | $\bar{1}'$ | $\frac{4/mmm}{\beta=0}$                                                                                      | $\frac{4mm}{\begin{pmatrix} 0 & -\beta_{21} & 0 \\ \beta_{21} & 0 & 0 \\ 0 & 0 & 0 \end{pmatrix}_1}$                          |
| $\frac{4'/mm'm}{}$<br>(15.4.56)     | $4/mmm$             | $mmm$       | $\bar{4}'$ | $\frac{4/mmm}{\beta=0}$                                                                                      | $\frac{4/mmm}{\beta=0}$                                                                                                       |
| $\frac{4'/m'm'm}{}$<br>(15.5.57)    | $4/mmm$             | $\bar{4}2m$ | $\bar{1}'$ | $\frac{4/mmm}{\beta=0}$                                                                                      | $\frac{42m}{\begin{pmatrix} \beta_{11} & 0 & 0 \\ 0 & -\beta_{11} & 0 \\ 0 & 0 & 0 \end{pmatrix}_1}$                          |
| $\frac{4/mm'm'}{}$<br>(15.6.58)     | $4/mmm$             | $4/m$       | $2'_{100}$ | $\frac{4/mmm}{\beta=0}$                                                                                      | $\frac{4/mmm}{\beta=0}$                                                                                                       |
| $\frac{4/m'm'm'}{}$<br>(15.7.59)    | $4/mmm$             | 422         | $\bar{1}'$ | $\frac{4/mmm}{\beta=0}$                                                                                      | $\frac{422}{\begin{pmatrix} \beta_{11} & 0 & 0 \\ 0 & \beta_{11} & 0 \\ 0 & 0 & \beta_{33} \end{pmatrix}_3}$                  |
| $\frac{\bar{3}'}{}$<br>(17.3.64)    | $\bar{3}$           | 3           | $\bar{1}'$ | $\frac{\bar{3}}{\beta=0}$                                                                                    | $\frac{3}{\begin{pmatrix} \beta_{11} & -\beta_{21} & 0 \\ \beta_{21} & \beta_{11} & 0 \\ 0 & 0 & \beta_{33} \end{pmatrix}_3}$ |

Continued on next page

TABLE S6 – continued from previous page

| MPG $M_0$                  | Isomorphic PG $G_0$ | $S_0$     | $R'$       | $G_0$ and $[\beta_{ij}^{\text{even}}]_{3 \times 3}$                                                                        | $G_1$ and $[\beta_{ij}^{\text{odd}}]_{3 \times 3}$                                                                         |
|----------------------------|---------------------|-----------|------------|----------------------------------------------------------------------------------------------------------------------------|----------------------------------------------------------------------------------------------------------------------------|
| $32'$<br>(18.3.67)         | 32                  | 3         | $2'_{100}$ | $32$<br>$\begin{pmatrix} \beta_{11} & 0 & 0 \\ 0 & \beta_{11} & 0 \\ 0 & 0 & \beta_{33} \end{pmatrix}_2$                   | $3m$<br>$\begin{pmatrix} 0 & -\beta_{21} & 0 \\ \beta_{21} & 0 & 0 \\ 0 & 0 & 0 \end{pmatrix}_1$                           |
| $3m'$<br>(19.3.70)         | $3m$                | 3         | $m'_{100}$ | $3m$<br>$\begin{pmatrix} 0 & -\beta_{21} & 0 \\ \beta_{21} & 0 & 0 \\ 0 & 0 & 0 \end{pmatrix}_1$                           | $32$<br>$\begin{pmatrix} \beta_{11} & 0 & 0 \\ 0 & \beta_{11} & 0 \\ 0 & 0 & \beta_{33} \end{pmatrix}_2$                   |
| $\bar{3}'m$<br>(20.3.73)   | $\bar{3}m$          | $3m$      | $\bar{1}'$ | $\bar{3}m$<br>$\beta=0$                                                                                                    | $3m$<br>$\begin{pmatrix} 0 & -\beta_{21} & 0 \\ \beta_{21} & 0 & 0 \\ 0 & 0 & 0 \end{pmatrix}_1$                           |
| $\bar{3}'m'$<br>(20.4.74)  | $\bar{3}m$          | 32        | $\bar{1}'$ | $\bar{3}m$<br>$\beta=0$                                                                                                    | $32$<br>$\begin{pmatrix} \beta_{11} & 0 & 0 \\ 0 & \beta_{11} & 0 \\ 0 & 0 & \beta_{33} \end{pmatrix}_2$                   |
| $\bar{3}m'$<br>(20.5.75)   | $\bar{3}m$          | $\bar{3}$ | $2'_{100}$ | $\bar{3}m$<br>$\beta=0$                                                                                                    | $\bar{3}m$<br>$\beta=0$                                                                                                    |
| $6'$<br>(21.3.78)          | 6                   | 3         | $2'$       | $6$<br>$\begin{pmatrix} \beta_{11} & -\beta_{21} & 0 \\ \beta_{21} & \beta_{11} & 0 \\ 0 & 0 & \beta_{33} \end{pmatrix}_3$ | $\bar{6}$<br>$\beta=0$                                                                                                     |
| $\bar{6}'$<br>(22.3.81)    | $\bar{6}$           | 3         | $m'_{001}$ | $\bar{6}$<br>$\beta=0$                                                                                                     | $6$<br>$\begin{pmatrix} \beta_{11} & -\beta_{21} & 0 \\ \beta_{21} & \beta_{11} & 0 \\ 0 & 0 & \beta_{33} \end{pmatrix}_3$ |
| $6'/m$<br>(23.3.84)        | $6/m$               | $\bar{6}$ | $\bar{1}'$ | $6/m$<br>$\beta=0$                                                                                                         | $\bar{6}$<br>$\beta=0$                                                                                                     |
| $6/m'$<br>(23.4.85)        | $6/m$               | 6         | $\bar{1}'$ | $6/m$<br>$\beta=0$                                                                                                         | $6$<br>$\begin{pmatrix} \beta_{11} & -\beta_{21} & 0 \\ \beta_{21} & \beta_{11} & 0 \\ 0 & 0 & \beta_{33} \end{pmatrix}_3$ |
| $6'/m'$<br>(23.5.86)       | $6/m$               | $\bar{3}$ | $m'_{001}$ | $6/m$<br>$\beta=0$                                                                                                         | $6/m$<br>$\beta=0$                                                                                                         |
| $6'22'$<br>(24.3.89)       | 622                 | 32        | $2'_{001}$ | $622$<br>$\begin{pmatrix} \beta_{11} & 0 & 0 \\ 0 & \beta_{11} & 0 \\ 0 & 0 & \beta_{33} \end{pmatrix}_2$                  | $\bar{6}2m$<br>$\beta=0$                                                                                                   |
| $62'2'$<br>(24.4.90)       | 622                 | 6         | $2'_{100}$ | $622$<br>$\begin{pmatrix} \beta_{11} & 0 & 0 \\ 0 & \beta_{11} & 0 \\ 0 & 0 & \beta_{33} \end{pmatrix}_2$                  | $6mm$<br>$\begin{pmatrix} 0 & -\beta_{21} & 0 \\ \beta_{21} & 0 & 0 \\ 0 & 0 & 0 \end{pmatrix}_1$                          |
| $6'mm'$<br>(25.3.93)       | $6mm$               | $3m$      | $2'_{001}$ | $6mm$<br>$\begin{pmatrix} 0 & -\beta_{21} & 0 \\ \beta_{21} & 0 & 0 \\ 0 & 0 & 0 \end{pmatrix}_1$                          | $\bar{6}m2$<br>$\beta=0$                                                                                                   |
| $6m'm'$<br>(25.4.94)       | $6mm$               | 6         | $m'_{100}$ | $6mm$<br>$\begin{pmatrix} 0 & -\beta_{21} & 0 \\ \beta_{21} & 0 & 0 \\ 0 & 0 & 0 \end{pmatrix}_1$                          | $622$<br>$\begin{pmatrix} \beta_{11} & 0 & 0 \\ 0 & \beta_{11} & 0 \\ 0 & 0 & \beta_{33} \end{pmatrix}_2$                  |
| $\bar{6}'m'2$<br>(26.3.97) | $\bar{6}m2$         | 32        | $m'_{001}$ | $\bar{6}m2$<br>$\beta=0$                                                                                                   | $622$<br>$\begin{pmatrix} \beta_{11} & 0 & 0 \\ 0 & \beta_{11} & 0 \\ 0 & 0 & \beta_{33} \end{pmatrix}_2$                  |
| $\bar{6}'m2'$<br>(26.4.98) | $\bar{6}m2$         | $3m$      | $m'_{001}$ | $\bar{6}m2$<br>$\beta=0$                                                                                                   | $6mm$<br>$\begin{pmatrix} 0 & -\beta_{21} & 0 \\ \beta_{21} & 0 & 0 \\ 0 & 0 & 0 \end{pmatrix}_1$                          |

Continued on next page

TABLE S6 – continued from previous page

| MPG $M_0$                    | Isomorphic PG $G_0$ | $S_0$       | $R'$             | $G_0$ and $[\beta_{ij}^{\text{even}}]_{3 \times 3}$                                                       | $G_1$ and $[\beta_{ij}^{\text{odd}}]_{3 \times 3}$                                                        |
|------------------------------|---------------------|-------------|------------------|-----------------------------------------------------------------------------------------------------------|-----------------------------------------------------------------------------------------------------------|
| $\bar{6}m'2'$<br>(26.5.99)   | $\bar{6}m2$         | $\bar{6}$   | $m'_{100}$       | $\bar{6}m2$<br>$\beta=0$                                                                                  | $\bar{6}2m$<br>$\beta=0$                                                                                  |
| $6/m'mm$<br>(27.3.102)       | $6/mmm$             | $6mm$       | $\bar{1}'$       | $6/mmm$<br>$\beta=0$                                                                                      | $6mm$<br>$\begin{pmatrix} 0 & -\beta_{21} & 0 \\ \beta_{21} & 0 & 0 \\ 0 & 0 & 0 \end{pmatrix}_1$         |
| $6'/mmm'$<br>(27.4.103)      | $6/mmm$             | $\bar{6}m2$ | $\bar{1}'$       | $6/mmm$<br>$\beta=0$                                                                                      | $\bar{6}m2$<br>$\beta=0$                                                                                  |
| $6'/m'mm'$<br>(27.5.104)     | $6/mmm$             | $\bar{3}m$  | $6'_{001}$       | $6/mmm$<br>$\beta=0$                                                                                      | $6/mmm$<br>$\beta=0$                                                                                      |
| $6/mm'm'$<br>(27.6.105)      | $6/mmm$             | $6/m$       | $2'_{100}$       | $6/mmm$<br>$\beta=0$                                                                                      | $6/mmm$<br>$\beta=0$                                                                                      |
| $6/m'm'm'$<br>(27.7.106)     | $6/mmm$             | $622$       | $\bar{1}'$       | $6/mmm$<br>$\beta=0$                                                                                      | $622$<br>$\begin{pmatrix} \beta_{11} & 0 & 0 \\ 0 & \beta_{11} & 0 \\ 0 & 0 & \beta_{33} \end{pmatrix}_2$ |
| $m'\bar{3}'$<br>(29.3.111)   | $m\bar{3}$          | $23$        | $\bar{1}'$       | $m\bar{3}$<br>$\beta=0$                                                                                   | $23$<br>$\begin{pmatrix} \beta_{11} & 0 & 0 \\ 0 & \beta_{11} & 0 \\ 0 & 0 & \beta_{11} \end{pmatrix}_1$  |
| $4'32'$<br>(30.3.114)        | $432$               | $23$        | $4'_{001}$       | $432$<br>$\begin{pmatrix} \beta_{11} & 0 & 0 \\ 0 & \beta_{11} & 0 \\ 0 & 0 & \beta_{11} \end{pmatrix}_1$ | $\bar{4}3m$<br>$\beta=0$                                                                                  |
| $\bar{4}'3m'$<br>(31.3.117)  | $\bar{4}3m$         | $23$        | $\bar{4}'_{001}$ | $\bar{4}3m$<br>$\beta=0$                                                                                  | $432$<br>$\begin{pmatrix} \beta_{11} & 0 & 0 \\ 0 & \beta_{11} & 0 \\ 0 & 0 & \beta_{11} \end{pmatrix}_1$ |
| $m'\bar{3}'m$<br>(32.3.120)  | $m\bar{3}m$         | $\bar{4}3m$ | $\bar{1}'$       | $m\bar{3}m$<br>$\beta=0$                                                                                  | $\bar{4}3m$<br>$\beta=0$                                                                                  |
| $m\bar{3}m'$<br>(32.4.121)   | $m\bar{3}m$         | $m\bar{3}$  | $4'_{100}$       | $m\bar{3}m$<br>$\beta=0$                                                                                  | $m\bar{3}m$<br>$\beta=0$                                                                                  |
| $m'\bar{3}'m'$<br>(32.5.122) | $m\bar{3}m$         | $432$       | $\bar{1}'$       | $m\bar{3}m$<br>$\beta=0$                                                                                  | $432$<br>$\begin{pmatrix} \beta_{11} & 0 & 0 \\ 0 & \beta_{11} & 0 \\ 0 & 0 & \beta_{11} \end{pmatrix}_1$ |

## V. CLARIFICATIONS OF SHG AND LMO EFFECTS IN MAGNDATA DATABASE

TABLE S7: Clarifications of SHG and LMO effects in [MAGNDATA](#) database (BCS-ID 0.1-0.835, 1.0.1-1.0.52, 1.1-1.663, 2.1-2.86, and 3.1-3.19). The underline wave symbols mean the materials have been appears in front of this table. The meaning of the SHG type see Table III in the main text, the symmetries of LMO effect refer to Table S2.

| BCS-ID | Formula                                                                          | Parent SG                       | MSG                                                     | MPG             | SHG    | LMO |
|--------|----------------------------------------------------------------------------------|---------------------------------|---------------------------------------------------------|-----------------|--------|-----|
| 0.1    | <a href="#">LaMnO<sub>3</sub></a>                                                | <i>Pnma</i> (62)                | <i>Pn'ma'</i> (62.448)                                  | <i>m'm'm</i>    | ×      | ✓   |
| 0.2    | <a href="#">Cd<sub>2</sub>Os<sub>2</sub>O<sub>7</sub></a>                        | <i>Fd3m</i> (227)               | <i>Fd3m'</i> (227.131)                                  | <i>m3m'</i>     | ×      | ×   |
| 0.3    | <a href="#">Ca<sub>3</sub>LiOsO<sub>6</sub></a>                                  | <i>R3c</i> (167)                | <i>C2'/c</i> (15.89)                                    | <i>2'/m'</i>    | ×      | ✓   |
| 0.4    | <a href="#">NiCr<sub>2</sub>O<sub>4</sub></a>                                    | <i>I4<sub>1</sub>/amd</i> (141) | <i>Fd'd'd</i> (70.530)                                  | <i>m'm'm</i>    | ×      | ✓   |
| 0.5    | <a href="#">Cr<sub>2</sub>S<sub>3</sub></a>                                      | <i>R3</i> (148)                 | <i>P1</i> (2.4)                                         | <i>1</i>        | ×      | ✓   |
| 0.6    | <a href="#">YMnO<sub>3</sub></a>                                                 | <i>P6<sub>3</sub>cm</i> (185)   | <i>P6<sub>3</sub>cm</i> (185.197)                       | <i>6mm</i>      | O-woP  | ×   |
| 0.7    | <a href="#">ScMnO<sub>3</sub></a>                                                | <i>P6<sub>3</sub>cm</i> (185)   | <i>P6<sub>3</sub>c'm'</i> (185.201)                     | <i>6m'm'</i>    | BW-woP | ✓   |
| 0.8    | <a href="#">ScMnO<sub>3</sub></a>                                                | <i>P6<sub>3</sub>cm</i> (185)   | <i>P6<sub>3</sub></i> (173.129)                         | <i>6</i>        | O-woP  | ✓   |
| 0.9    | <a href="#">GdB<sub>4</sub></a>                                                  | <i>P4/mbm</i> (127)             | <i>P4/m'b'm'</i> (127.395)                              | <i>4/m'm'm'</i> | PT-wP  | ×   |
| 0.10   | <a href="#">DyFeO<sub>3</sub></a>                                                | <i>Pnma</i> (62)                | <i>P2<sub>1</sub>2<sub>1</sub>2<sub>1</sub></i> (19.25) | <i>222</i>      | O-wP   | ×   |
| 0.11   | <a href="#">DyFeO<sub>3</sub></a>                                                | <i>Pnma</i> (62)                | <i>Pn'a'2<sub>1</sub></i> (33.148)                      | <i>m'm'2</i>    | BW-wP  | ✓   |
| 0.12   | <a href="#">U<sub>3</sub>Ru<sub>4</sub>Al<sub>12</sub></a>                       | <i>P6<sub>3</sub>/mmc</i> (194) | <i>Cmcm'</i> (63.461)                                   | <i>m'mm</i>     | PT-wP  | ×   |
| 0.13   | <a href="#">Ca<sub>3</sub>Co<sub>2-x</sub>Mn<sub>x</sub>O<sub>6</sub></a>        | <i>R3c</i> (167)                | <i>R3c</i> (161.69)                                     | <i>3m</i>       | O-wP   | ×   |
| 0.14   | <a href="#">Gd<sub>5</sub>Ge<sub>4</sub></a>                                     | <i>Pnma</i> (62)                | <i>Pnm'a</i> (62.444)                                   | <i>m'mm</i>     | PT-wP  | ×   |
| 0.15   | <a href="#">MnF<sub>2</sub></a>                                                  | <i>P4<sub>2</sub>/mnm</i> (136) | <i>P4<sub>2</sub>/mnm'</i> (136.499)                    | <i>4'/mm'm</i>  | ×      | ×   |
| 0.16   | <a href="#">EuTiO<sub>3</sub></a>                                                | <i>I4/mcm</i> (140)             | <i>Fm'mm</i> (69.523)                                   | <i>m'mm</i>     | PT-wP  | ×   |
| 0.17   | <a href="#">FePO<sub>4</sub></a>                                                 | <i>Pnma</i> (62)                | <i>P2<sub>1</sub>2<sub>1</sub>2<sub>1</sub></i> (19.25) | <i>222</i>      | O-wP   | ×   |
| 0.18   | <a href="#">BaMn<sub>2</sub>As<sub>2</sub></a>                                   | <i>I4/mmm</i> (139)             | <i>I4'/m'm'm</i> (139.536)                              | <i>4'/m'm'm</i> | PT-wP  | ×   |
| 0.19   | <a href="#">MnTiO<sub>3</sub></a>                                                | <i>R3</i> (148)                 | <i>R3'</i> (148.19)                                     | <i>3'</i>       | PT-wP  | ×   |
| 0.20   | <a href="#">MnTe<sub>2</sub></a>                                                 | <i>Pa3</i> (205)                | <i>Pa3</i> (205.33)                                     | <i>m3</i>       | ×      | ×   |
| 0.21   | <a href="#">PbNiO<sub>3</sub></a>                                                | <i>R3c</i> (161)                | <i>R3c</i> (161.69)                                     | <i>3m</i>       | O-woP  | ×   |
| 0.22   | <a href="#">DyB<sub>4</sub></a>                                                  | <i>P4/mbm</i> (127)             | <i>Pb'am</i> (55.355)                                   | <i>m'mm</i>     | PT-wP  | ×   |
| 0.23   | <a href="#">Ca<sub>3</sub>Mn<sub>2</sub>O<sub>7</sub></a>                        | <i>Cmc2<sub>1</sub></i> (36)    | <i>Cm'c'2<sub>1</sub></i> (36.174)                      | <i>m'm2'</i>    | BW-woP | ✓   |
| 0.24   | <a href="#">LiMnPO<sub>4</sub></a>                                               | <i>Pnma</i> (62)                | <i>Pn'm'a'</i> (62.449)                                 | <i>m'm'm'</i>   | PT-wP  | ×   |
| 0.25   | <a href="#">NaOsO<sub>3</sub></a>                                                | <i>Pnma</i> (62)                | <i>Pn'ma'</i> (62.448)                                  | <i>m'm'm</i>    | ×      | ✓   |
| 0.26   | <a href="#">TmAgGe</a>                                                           | <i>P6<sub>2</sub>m</i> (189)    | <i>Am'm'2</i> (38.191)                                  | <i>m'm'2</i>    | BW-woP | ✓   |
| 0.27   | <a href="#">YFe<sub>4</sub>Ge<sub>2</sub></a>                                    | <i>Pnnm</i> (58)                | <i>Pn'n'm'</i> (58.399)                                 | <i>m'm'm'</i>   | PT-wP  | ×   |
| 0.28   | <a href="#">LiFeSi<sub>2</sub>O<sub>6</sub></a>                                  | <i>P2<sub>1</sub>/c</i> (14)    | <i>P2<sub>1</sub>/c'</i> (14.78)                        | <i>2/m'</i>     | PT-wP  | ×   |
| 0.29   | <a href="#">Er<sub>2</sub>Ti<sub>2</sub>O<sub>7</sub></a>                        | <i>Fd3m</i> (227)               | <i>I4<sub>1</sub>/am'd</i> (141.554)                    | <i>4'/mm'm</i>  | ×      | ×   |
| 0.30   | <a href="#">YbMnO<sub>3</sub></a>                                                | <i>P6<sub>3</sub>cm</i> (185)   | <i>P6<sub>3</sub>c'm</i> (185.199)                      | <i>6'mm'</i>    | BW-woP | ×   |
| 0.31   | <a href="#">HoMnO<sub>3</sub></a>                                                | <i>P6<sub>3</sub>cm</i> (185)   | <i>P6<sub>3</sub>c'm'</i> (185.201)                     | <i>6m'm'</i>    | BW-woP | ✓   |
| 0.32   | <a href="#">HoMnO<sub>3</sub></a>                                                | <i>P6<sub>3</sub>cm</i> (185)   | <i>P6<sub>3</sub>cm</i> (185.197)                       | <i>6mm</i>      | O-woP  | ×   |
| 0.33   | <a href="#">HoMnO<sub>3</sub></a>                                                | <i>P6<sub>3</sub>cm</i> (185)   | <i>P6<sub>3</sub>cm</i> (185.197)                       | <i>6mm</i>      | O-woP  | ×   |
| 0.34   | <a href="#">La<sub>0.5</sub>Sr<sub>0.5</sub>FeO<sub>2.5</sub>F<sub>0.5</sub></a> | <i>Pnma</i> (62)                | <i>Pn'ma'</i> (62.448)                                  | <i>m'm'm</i>    | ×      | ✓   |
| 0.35   | <a href="#">Cu<sub>2</sub>OSeO<sub>3</sub></a>                                   | <i>P2<sub>1</sub>3</i> (198)    | <i>R3</i> (146.10)                                      | <i>3</i>        | O-woP  | ✓   |
| 0.36   | <a href="#">NiF<sub>2</sub></a>                                                  | <i>P4<sub>2</sub>/mnm</i> (136) | <i>Pnn'm'</i> (58.398)                                  | <i>m'm'm</i>    | ×      | ✓   |
| 0.37   | <a href="#">U<sub>3</sub>Al<sub>2</sub>Si<sub>3</sub></a>                        | <i>I4</i> (79)                  | <i>C2'</i> (5.15)                                       | <i>2'</i>       | BW-woP | ✓   |
| 0.38   | <a href="#">GaFeO<sub>3</sub></a>                                                | <i>Pna2<sub>1</sub></i> (33)    | <i>Pna'2<sub>1</sub></i> (33.147)                       | <i>m'm2'</i>    | BW-woP | ✓   |
| 0.39   | <a href="#">Nd<sub>2</sub>NaRuO<sub>6</sub></a>                                  | <i>P2<sub>1</sub>/n</i> (14)    | <i>P2<sub>1</sub>/c</i> (14.75)                         | <i>2/m</i>      | ×      | ✓   |
| 0.40   | <a href="#">Mn<sub>2</sub>O<sub>3</sub>-alpha</a>                                | <i>Pbca</i> (61)                | <i>Pbca</i> (61.433)                                    | <i>mmm</i>      | ×      | ×   |
| 0.41   | <a href="#">Mn<sub>2</sub>O<sub>3</sub>-alpha</a>                                | <i>Pbca</i> (61)                | <i>Pbca</i> (61.433)                                    | <i>mmm</i>      | ×      | ×   |
| 0.42   | <a href="#">HoMnO<sub>3</sub></a>                                                | <i>P6<sub>3</sub>cm</i> (185)   | <i>P6<sub>3</sub>c'm</i> (185.199)                      | <i>6'mm'</i>    | BW-woP | ×   |
| 0.43   | <a href="#">HoMnO<sub>3</sub></a>                                                | <i>P6<sub>3</sub>cm</i> (185)   | <i>P6<sub>3</sub>c'm'</i> (185.2)                       | <i>6'mm'</i>    | BW-woP | ×   |
| 0.44   | <a href="#">YMnO<sub>3</sub></a>                                                 | <i>P6<sub>3</sub>cm</i> (185)   | <i>P6<sub>3</sub></i> (173.131)                         | <i>6'</i>       | BW-woP | ×   |
| 0.45   | <a href="#">La<sub>2</sub>NiO<sub>4</sub></a>                                    | <i>P4<sub>2</sub>/ncm</i> (138) | <i>Pc'c'n</i> (56.369)                                  | <i>m'm'm</i>    | ×      | ✓   |
| 0.46   | <a href="#">CaBaCo<sub>4</sub>O<sub>7</sub></a>                                  | <i>Pbn2<sub>1</sub></i> (33)    | <i>Pna'2<sub>1</sub></i> (33.147)                       | <i>m'm2'</i>    | BW-woP | ✓   |
| 0.47   | <a href="#">Gd<sub>2</sub>Sn<sub>2</sub>O<sub>7</sub></a>                        | <i>Fd3m</i> (227)               | <i>I4<sub>1</sub>/amd'</i> (141.555)                    | <i>4'/mm'm</i>  | ×      | ×   |
| 0.48   | <a href="#">Tb<sub>2</sub>Sn<sub>2</sub>O<sub>7</sub></a>                        | <i>Fd3m</i> (227)               | <i>I4<sub>1</sub>/am'd'</i> (141.557)                   | <i>4/mm'm'</i>  | ×      | ✓   |
| 0.49   | <a href="#">Ho<sub>2</sub>Ru<sub>2</sub>O<sub>7</sub></a>                        | <i>Fd3m</i> (227)               | <i>I4<sub>1</sub>/am'd'</i> (141.557)                   | <i>4/mm'm'</i>  | ×      | ✓   |
| 0.50   | <a href="#">MnTiO<sub>3</sub></a>                                                | <i>R3c</i> (161)                | <i>Cc'</i> (9.39)                                       | <i>m'</i>       | BW-woP | ✓   |
| 0.51   | <a href="#">Ho<sub>2</sub>Ru<sub>2</sub>O<sub>7</sub></a>                        | <i>Fd3m</i> (227)               | <i>I4<sub>1</sub>/am'd'</i> (141.557)                   | <i>4/mm'm'</i>  | ×      | ✓   |
| 0.52   | <a href="#">K<sub>y</sub>Fe<sub>2-x</sub>Se<sub>2</sub></a>                      | <i>I4/m</i> (87)                | <i>C2'/m'</i> (12.62)                                   | <i>2'/m'</i>    | ×      | ✓   |

Continued on next page

TABLE S7 – continued from previous page

| BCS-ID | Formula                                                                                                                          | Parent                                   | MSG                                          | MPG             | SHG type | LMO |
|--------|----------------------------------------------------------------------------------------------------------------------------------|------------------------------------------|----------------------------------------------|-----------------|----------|-----|
| 0.53   | Rb <sub>y</sub> Fe <sub>2-x</sub> Se <sub>2</sub>                                                                                | <i>I4/m</i> (87)                         | <i>C2'/m'</i> (12.62)                        | <i>2'/m'</i>    | ×        | ✓   |
| 0.54   | Rb <sub>y</sub> Fe <sub>2-x</sub> Se <sub>2</sub>                                                                                | <i>I4/m</i> (87)                         | <i>I4/m'</i> (87.78)                         | <i>4/m'</i>     | PT-wP    | ×   |
| 0.55   | K <sub>y</sub> Fe <sub>2-x</sub> Se <sub>2</sub>                                                                                 | <i>I4/m</i> (87)                         | <i>I4/m'</i> (87.78)                         | <i>4/m'</i>     | PT-wP    | ×   |
| 0.56   | Ba <sub>2</sub> CoGe <sub>2</sub> O <sub>7</sub>                                                                                 | <i>P42<sub>1</sub>m</i> (113)            | <i>Cm'm2'</i> (35.167)                       | <i>m'm2'</i>    | BW-woP   | ✓   |
| 0.57   | ScFeO <sub>3</sub>                                                                                                               | <i>R3c</i> (161)                         | <i>Cc'</i> (9.39)                            | <i>m'</i>       | BW-woP   | ✓   |
| 0.58   | CoAl <sub>2</sub> O <sub>4</sub>                                                                                                 | <i>Fd3m</i> (227)                        | <i>I4<sub>1</sub>/a'm'd</i> (141.556)        | <i>4'/m'm'm</i> | PT-wP    | ×   |
| 0.59   | Cr <sub>2</sub> O <sub>3</sub>                                                                                                   | <i>R3c</i> (167)                         | <i>R3'c'</i> (167.106)                       | <i>3'm'</i>     | PT-wP    | ×   |
| 0.60   | [NH <sub>2</sub> (CH <sub>3</sub> ) <sub>2</sub> ] <sub>n</sub> [Fe <sup>II</sup> (H <sub>2</sub> O) <sub>6</sub> ] <sub>n</sub> | <i>R3c'</i> (167.107)                    | <i>R3c'</i> (167.107)                        | <i>3m'</i>      | ×        | ✓   |
| 0.61   | Li <sub>2</sub> FeP <sub>2</sub> O <sub>7</sub>                                                                                  | <i>P2<sub>1</sub>/c</i> (14)             | <i>P2<sub>1</sub>/c</i> (14.75)              | <i>2/m</i>      | ×        | ✓   |
| 0.62   | SrMn <sub>2</sub> V <sub>2</sub> O <sub>8</sub>                                                                                  | <i>I4<sub>1</sub>cd</i> (110)            | <i>Ib'a2'</i> (45.237)                       | <i>m'm2'</i>    | BW-woP   | ✓   |
| 0.63   | Ho <sub>2</sub> CrSbO <sub>7</sub>                                                                                               | <i>Fd3m</i> (227)                        | <i>I4<sub>1</sub>/am'd'</i> (141.557)        | <i>4'/mm'm'</i> | ×        | ✓   |
| 0.64   | MnV <sub>2</sub> O <sub>4</sub>                                                                                                  | <i>I4<sub>1</sub>/a</i> (88)             | <i>I4<sub>1</sub>/a</i> (88.81)              | <i>4/m</i>      | ×        | ✓   |
| 0.65   | Fe <sub>2</sub> O <sub>3</sub> -alpha                                                                                            | <i>R3c</i> (167)                         | <i>C2'/c'</i> (15.89)                        | <i>2'/m'</i>    | ×        | ✓   |
| 0.66   | Fe <sub>2</sub> O <sub>3</sub> -alpha                                                                                            | <i>R3c</i> (167)                         | <i>P1</i> (2.4)                              | <i>1</i>        | ×        | ✓   |
| 0.67   | BiFe <sub>0.5</sub> Sc <sub>0.5</sub> O <sub>3</sub>                                                                             | <i>Ima2</i> (46)                         | <i>Im'a2'</i> (46.243)                       | <i>m'm2'</i>    | BW-woP   | ✓   |
| 0.68   | BiFe <sub>0.5</sub> Sc <sub>0.5</sub> O <sub>3</sub>                                                                             | <i>Pnma</i> (62)                         | <i>Pn'm'a</i> (62.446)                       | <i>m'm'm</i>    | ×        | ✓   |
| 0.69   | Co <sub>4</sub> (OH) <sub>2</sub> (C <sub>10</sub> H <sub>16</sub> O <sub>2</sub> ) <sub>2</sub>                                 | <i>P2<sub>1</sub>/c</i> (14)             | <i>P2<sub>1</sub>/c'</i> (14.79)             | <i>2'/m'</i>    | ×        | ✓   |
| 0.70   | Na <sub>3</sub> Co(CO <sub>3</sub> ) <sub>2</sub> Cl                                                                             | <i>Fd3</i> (203)                         | <i>Fd3</i> (203.26)                          | <i>m3</i>       | ×        | ×   |
| 0.71   | Li <sub>2</sub> Ni(SO <sub>4</sub> ) <sub>2</sub>                                                                                | <i>Pbca</i> (61)                         | <i>Pb'c'a'</i> (61.437)                      | <i>m'm'm'</i>   | PT-wP    | ×   |
| 0.72   | CaMnBi <sub>2</sub>                                                                                                              | <i>P4/nmm</i> (129)                      | <i>P4'/n'm'm</i> (129.416)                   | <i>4'/m'm'm</i> | PT-wP    | ×   |
| 0.73   | SrMnBi <sub>2</sub>                                                                                                              | <i>I4/mmm</i> (139)                      | <i>I4'/m'm'm</i> (139.536)                   | <i>4'/m'm'm</i> | PT-wP    | ×   |
| 0.74   | Mn <sub>3</sub> Cu <sub>0.5</sub> Ge <sub>0.5</sub> N                                                                            | <i>Pm3m</i> (221)                        | <i>R3m</i> (166.97)                          | <i>3m</i>       | ×        | ×   |
| 0.75   | Cr <sub>2</sub> WO <sub>6</sub>                                                                                                  | <i>P4<sub>2</sub>/mnm</i> (136)          | <i>Pn'nm</i> (58.395)                        | <i>m'mm</i>     | PT-wP    | ×   |
| 0.76   | Cr <sub>2</sub> TeO <sub>6</sub>                                                                                                 | <i>P4<sub>2</sub>/mnm</i> (136)          | <i>Pn'nm</i> (58.395)                        | <i>m'mm</i>     | PT-wP    | ×   |
| 0.77   | Tb <sub>2</sub> Ti <sub>2</sub> O <sub>7</sub>                                                                                   | <i>Fd3m</i> (227)                        | <i>R3m'</i> (166.101)                        | <i>3m'</i>      | ×        | ✓   |
| 0.78   | NiN <sub>2</sub> O <sub>6</sub>                                                                                                  | <i>R3</i> (148)                          | <i>R3</i> (148.17)                           | <i>3</i>        | ×        | ✓   |
| 0.79   | CaIrO <sub>3</sub>                                                                                                               | <i>Cmcm</i> (63)                         | <i>Cm'cm'</i> (63.464)                       | <i>m'm'm</i>    | ×        | ✓   |
| 0.80   | U <sub>2</sub> Pd <sub>2</sub> In                                                                                                | <i>P4/mbm</i> (127)                      | <i>P4'/m'bm'</i> (127.394)                   | <i>4'/m'm'm</i> | PT-wP    | ×   |
| 0.81   | U <sub>2</sub> Pd <sub>2</sub> Sn                                                                                                | <i>P4/mbm</i> (127)                      | <i>P4'/m'bm'</i> (127.394)                   | <i>4'/m'm'm</i> | PT-wP    | ×   |
| 0.82   | Gd <sub>2</sub> CuO <sub>4</sub>                                                                                                 | <i>Aeam</i> (64)                         | <i>Cm'ca'</i> (64.476)                       | <i>m'm'm</i>    | ×        | ✓   |
| 0.83   | LiFeP <sub>2</sub> O <sub>7</sub>                                                                                                | <i>P2<sub>1</sub></i> (4)                | <i>P2<sub>1</sub></i> (4.7)                  | <i>2</i>        | O-woP    | ✓   |
| 0.84   | Mn <sub>2</sub> FeMoO <sub>6</sub>                                                                                               | <i>R3</i> (146)                          | <i>R3</i> (146.10)                           | <i>3</i>        | O-woP    | ✓   |
| 0.85   | KCo <sub>4</sub> (PO <sub>4</sub> ) <sub>3</sub>                                                                                 | <i>Pnnm</i> (58)                         | <i>Pnn'm'</i> (58.398)                       | <i>m'm'm</i>    | ×        | ✓   |
| 0.86   | KMn <sub>4</sub> (PO <sub>4</sub> ) <sub>3</sub>                                                                                 | <i>Pnam</i> (62)                         | <i>Pnma'</i> (62.445)                        | <i>m'mm</i>     | PT-wP    | ×   |
| 0.87   | NaFePO <sub>4</sub>                                                                                                              | <i>Pnma</i> (62)                         | <i>Pnma'</i> (62.445)                        | <i>m'mm</i>     | PT-wP    | ×   |
| 0.88   | LiNiPO <sub>4</sub>                                                                                                              | <i>Pnma</i> (62)                         | <i>Pnn'm'a</i> (62.444)                      | <i>m'mm</i>     | PT-wP    | ×   |
| 0.89   | BaMn <sub>2</sub> Bi <sub>2</sub>                                                                                                | <i>I4/mmm</i> (139)                      | <i>I4'/m'm'm</i> (139.536)                   | <i>4'/m'm'm</i> | PT-wP    | ×   |
| 0.90   | Rb <sub>2</sub> Fe <sub>2</sub> O(AsO <sub>4</sub> ) <sub>2</sub>                                                                | <i>Pnma</i> (62)                         | <i>Pnma</i> (62.441)                         | <i>mmm</i>      | ×        | ×   |
| 0.91   | Rb <sub>2</sub> Fe <sub>2</sub> O(AsO <sub>4</sub> ) <sub>2</sub>                                                                | <i>Pnma</i> (62)                         | <i>Pn'ma'</i> (62.448)                       | <i>m'm'm</i>    | ×        | ✓   |
| 0.92   | CaMn <sub>2</sub> Sb <sub>2</sub>                                                                                                | <i>P3m1</i> (164)                        | <i>C2'/m</i> (12.60)                         | <i>2'/m</i>     | PT-wP    | ×   |
| 0.93   | Ca <sub>2</sub> Fe <sub>2</sub> O <sub>5</sub>                                                                                   | <i>Pcmn</i> (62)                         | <i>Pcm'n'</i> (62.446)                       | <i>m'm'm</i>    | ×        | ✓   |
| 0.94   | TeNiO <sub>3</sub>                                                                                                               | <i>Pnma</i> (62)                         | <i>Pn'm'a</i> (62.446)                       | <i>m'm'm</i>    | ×        | ✓   |
| 0.95   | LiFePO <sub>4</sub>                                                                                                              | <i>Pnma</i> (62)                         | <i>Pnma'</i> (62.445)                        | <i>m'mm</i>     | PT-wP    | ×   |
| 0.96   | CoSO <sub>4</sub>                                                                                                                | <i>Pnma</i> (62)                         | <i>Pnma</i> (62.441)                         | <i>mmm</i>      | ×        | ×   |
| 0.97   | FeSb <sub>2</sub> O <sub>4</sub>                                                                                                 | <i>P4<sub>2</sub>/mbc</i> (135)          | <i>Pmc2<sub>1</sub></i> (26.66)              | <i>mm2</i>      | O-wP     | ×   |
| 0.98   | YBaMn <sub>2</sub> O <sub>5.5</sub>                                                                                              | <i>Icam</i> (72)                         | <i>Ib'a'm</i> (72.543)                       | <i>m'm'm</i>    | ×        | ✓   |
| 0.99   | YBaMn <sub>2</sub> O <sub>5.5</sub>                                                                                              | <i>Icam</i> (72)                         | <i>C2/m</i> (12.58)                          | <i>2/m</i>      | ×        | ✓   |
| 0.100  | YCr <sub>0.5</sub> Mn <sub>0.5</sub> O <sub>3</sub>                                                                              | <i>Pnma</i> (62)                         | <i>Pn'ma'</i> (62.448)                       | <i>m'm'm</i>    | ×        | ✓   |
| 0.101  | Mn <sub>2</sub> GeO <sub>4</sub>                                                                                                 | <i>Pnma</i> (62)                         | <i>Pn'm'a</i> (62.446)                       | <i>m'm'm</i>    | ×        | ✓   |
| 0.102  | Mn <sub>2</sub> GeO <sub>4</sub>                                                                                                 | <i>Pnma</i> (62)                         | <i>Pnma</i> (62.441)                         | <i>mmm</i>      | ×        | ×   |
| 0.103  | Mn <sub>2</sub> GeO <sub>4</sub>                                                                                                 | <i>Pnma</i> (62)                         | <i>P2<sub>1</sub>/c</i> (14.75)              | <i>2/m</i>      | ×        | ✓   |
| 0.104  | ErVO <sub>3</sub>                                                                                                                | <i>Pbnm</i> (62)                         | <i>P2<sub>1</sub>/m'</i> (11.54)             | <i>2'/m'</i>    | ×        | ✓   |
| 0.105  | ErVO <sub>3</sub>                                                                                                                | <i>Pbnm</i> (62)                         | <i>P2<sub>1</sub>/c</i> (14.75)              | <i>2/m</i>      | ×        | ✓   |
| 0.106  | DyVO <sub>3</sub>                                                                                                                | <i>Pbnm</i> (62)                         | <i>P2<sub>1</sub>/m'</i> (11.54)             | <i>2'/m'</i>    | ×        | ✓   |
| 0.107  | Ho <sub>2</sub> Ge <sub>2</sub> O <sub>7</sub>                                                                                   | <i>P4<sub>1</sub>2<sub>1</sub>2</i> (92) | <i>P4<sub>1</sub>2<sub>1</sub>2</i> (92.111) | <i>422</i>      | O-woP    | ×   |
| 0.108  | Mn <sub>3</sub> Ir                                                                                                               | <i>Pm3m</i> (221)                        | <i>R3m'</i> (166.101)                        | <i>3m'</i>      | ×        | ✓   |
| 0.109  | Mn <sub>3</sub> Pt                                                                                                               | <i>Pm3m</i> (221)                        | <i>R3m'</i> (166.101)                        | <i>3m'</i>      | ×        | ✓   |
| 0.110  | Cr <sub>2</sub> O <sub>3</sub>                                                                                                   | <i>R3c</i> (167)                         | <i>C2'/c</i> (15.87)                         | <i>2'/m</i>     | PT-wP    | ×   |

Continued on next page

TABLE S7 – continued from previous page

| BCS-ID | Formula                                                                  | Parent             | MSG                     | MPG          | SHG type | LMO |
|--------|--------------------------------------------------------------------------|--------------------|-------------------------|--------------|----------|-----|
| 0.111  | <a href="#">Co<sub>4</sub>Nb<sub>2</sub>O<sub>9</sub></a>                | $P\bar{3}c1$ (165) | $P\bar{3}'c'1$ (165.94) | $\bar{3}'m'$ | PT-wP    | ×   |
| 0.112  | <a href="#">FeBO<sub>3</sub></a>                                         | $R\bar{3}c$ (167)  | $C2'/c'$ (15.89)        | $2'/m'$      | ×        | ✓   |
| 0.113  | <a href="#">NiCO<sub>3</sub></a>                                         | $R\bar{3}c$ (167)  | $C2/c$ (15.85)          | $2/m$        | ×        | ✓   |
| 0.114  | <a href="#">CoCO<sub>3</sub></a>                                         | $R\bar{3}c$ (167)  | $C2/c$ (15.85)          | $2/m$        | ×        | ✓   |
| 0.115  | <a href="#">MnCO<sub>3</sub></a>                                         | $R\bar{3}c$ (167)  | $C2/c$ (15.85)          | $2/m$        | ×        | ✓   |
| 0.116  | <a href="#">FeCO<sub>3</sub></a>                                         | $R\bar{3}c$ (167)  | $R\bar{3}c$ (167.103)   | $3m$         | ×        | ×   |
| 0.117  | <a href="#">LuFeO<sub>3</sub></a>                                        | $P6_3cm$ (185)     | $P6_3c'm'$ (185.201)    | $6m'm'$      | BW-woP   | ✓   |
| 0.118  | <a href="#">Ba<sub>5</sub>Co<sub>5</sub>ClO<sub>13</sub></a>             | $P6_3/mmc$ (194)   | $P6_3/m'm'c$ (194.268)  | $6'/m'mm'$   | ×        | ×   |
| 0.119  | <a href="#">CoSe<sub>2</sub>O<sub>5</sub></a>                            | $Pbcn$ (60)        | $Pb'cn$ (60.419)        | $m'mm$       | PT-wP    | ×   |
| 0.120  | <a href="#">LiFe(SO<sub>4</sub>)<sub>2</sub></a>                         | $P2_1/c$ (14)      | $P2_1/c$ (14.75)        | $2/m$        | ×        | ✓   |
| 0.121  | <a href="#">Li<sub>2</sub>Co(SO<sub>4</sub>)<sub>2</sub></a>             | $P2_1/c$ (14)      | $P2_1'/c'$ (14.79)      | $2'/m'$      | ×        | ✓   |
| 0.122  | <a href="#">Li<sub>2</sub>Mn(SO<sub>4</sub>)<sub>2</sub></a>             | $P2_1/c$ (14)      | $P2_1/c$ (14.75)        | $2/m$        | ×        | ✓   |
| 0.123  | <a href="#">Mn<sub>3</sub>NiN</a>                                        | $Pm\bar{3}m$ (221) | $R\bar{3}$ (148.17)     | $\bar{3}$    | ×        | ✓   |
| 0.124  | <a href="#">Mn<sub>3</sub>NiN</a>                                        | $Pm\bar{3}m$ (221) | $R\bar{3}$ (148.17)     | $\bar{3}$    | ×        | ✓   |
| 0.125  | <a href="#">MnGeO<sub>3</sub></a>                                        | $R\bar{3}$ (148)   | $R\bar{3}'$ (148.19)    | $\bar{3}'$   | PT-wP    | ×   |
| 0.126  | <a href="#">NpCo<sub>2</sub></a>                                         | $Fd\bar{3}m$ (227) | $I4_1'/a'm'd$ (141.556) | $4'/m'm'm$   | PT-wP    | ×   |
| 0.127  | <a href="#">Dy<sub>3</sub>Al<sub>5</sub>O<sub>12</sub></a>               | $Ia\bar{3}d$ (230) | $Ia\bar{3}d'$ (230.148) | $m\bar{3}m'$ | ×        | ×   |
| 0.128  | <a href="#">FeSO<sub>4</sub>F</a>                                        | $C2/c$ (15)        | $C2'/c'$ (15.89)        | $2'/m'$      | ×        | ✓   |
| 0.129  | <a href="#">Cu<sub>3</sub>Mo<sub>2</sub>O<sub>9</sub></a>                | $Pnma$ (62)        | $P2_1'2_1'2_1$ (19.27)  | $2'2'2$      | BW-wP    | ✓   |
| 0.130  | <a href="#">Cu<sub>3</sub>Mo<sub>2</sub>O<sub>9</sub></a>                | $Pnma$ (62)        | $Pm'c2_1'$ (26.68)      | $m'm2'$      | BW-wP    | ✓   |
| 0.131  | <a href="#">Mn(N(CN<sub>2</sub>))<sub>2</sub></a>                        | $Pnnm$ (58)        | $Pnn'm'$ (58.398)       | $m'm'm$      | ×        | ✓   |
| 0.132  | <a href="#">Fe(N(CN<sub>2</sub>))<sub>2</sub></a>                        | $Pnnm$ (58)        | $Pnn'm'$ (58.398)       | $m'm'm$      | ×        | ✓   |
| 0.133  | <a href="#">Ni<sub>3</sub>B<sub>7</sub>O<sub>13</sub>Cl</a>              | $Pca2_1$ (29)      | $Pc'a2_1'$ (29.101)     | $m'm2'$      | BW-woP   | ✓   |
| 0.134  | <a href="#">Mn<sub>3</sub>B<sub>7</sub>O<sub>13</sub>I</a>               | $Pca2_1$ (29)      | $Pc'a2_1'$ (29.101)     | $m'm2'$      | BW-woP   | ✓   |
| 0.135  | <a href="#">Ni<sub>3</sub>B<sub>7</sub>O<sub>13</sub>Br</a>              | $Pca2_1$ (29)      | $Pc'a2_1'$ (29.101)     | $m'm2'$      | BW-woP   | ✓   |
| 0.136  | <a href="#">Co<sub>3</sub>B<sub>7</sub>O<sub>13</sub>Br</a>              | $Pca2_1$ (29)      | $Pc'a2_1'$ (29.101)     | $m'm2'$      | BW-woP   | ✓   |
| 0.137  | <a href="#">Cu<sub>2</sub>V<sub>2</sub>O<sub>7</sub></a>                 | $Fdd2$ (43)        | $Fd'd'2$ (43.227)       | $m'm'2$      | BW-woP   | ✓   |
| 0.138  | <a href="#">BiCrO<sub>3</sub></a>                                        | $C2/c$ (15)        | $C2/c$ (15.85)          | $2/m$        | ×        | ✓   |
| 0.139  | <a href="#">BiCrO<sub>3</sub></a>                                        | $C2/c$ (15)        | $P1$ (2.4)              | $1$          | ×        | ✓   |
| 0.140  | <a href="#">LuFe<sub>4</sub>Ge<sub>2</sub></a>                           | $P4_2/mnm$ (136)   | $Pn'n'm'$ (58.399)      | $m'm'm'$     | PT-wP    | ×   |
| 0.141  | <a href="#">Tb<sub>5</sub>Ge<sub>4</sub></a>                             | $Pnma$ (62)        | $Pnm'a$ (62.444)        | $m'mm$       | PT-wP    | ×   |
| 0.142  | <a href="#">Fe<sub>2</sub>TeO<sub>6</sub></a>                            | $P4_2/mnm$ (136)   | $P4_2/m'n'm'$ (136.503) | $4'/m'm'm'$  | PT-wP    | ×   |
| 0.143  | <a href="#">Cr<sub>2</sub>TeO<sub>6</sub></a>                            | $P4_2/mnm$ (136)   | $Pn'nm$ (58.395)        | $m'mm$       | PT-wP    | ×   |
| 0.144  | <a href="#">Cr<sub>2</sub>WO<sub>6</sub></a>                             | $P4_2/mnm$ (136)   | $Pn'nm$ (58.395)        | $m'mm$       | PT-wP    | ×   |
| 0.145  | <a href="#">Co<sub>3</sub>TeO<sub>6</sub></a>                            | $C2/c$ (15)        | $C2'/c$ (15.87)         | $2'/m$       | PT-wP    | ×   |
| 0.146  | <a href="#">EuZrO<sub>3</sub></a>                                        | $Pnma$ (62)        | $Pnm'a$ (62.444)        | $m'mm$       | PT-wP    | ×   |
| 0.147  | <a href="#">EuZrO<sub>3</sub></a>                                        | $Pnma$ (62)        | $Pn'm'a'$ (62.449)      | $m'm'm'$     | PT-wP    | ×   |
| 0.148  | <a href="#">La<sub>2</sub>LiRuO<sub>6</sub></a>                          | $P2_1/n$ (14)      | $P2_1/c$ (14.75)        | $2/m$        | ×        | ✓   |
| 0.149  | <a href="#">Nd<sub>3</sub>Ru<sub>4</sub>Al<sub>12</sub></a>              | $P6_3/mmc$ (194)   | $Cm'c'm$ (63.462)       | $m'm'm$      | ×        | ✓   |
| 0.15   | <a href="#">NiS<sub>2</sub></a>                                          | $Pa\bar{3}$ (205)  | $Pa\bar{3}$ (205.33)    | $m\bar{3}$   | ×        | ×   |
| 0.151  | <a href="#">Tm<sub>2</sub>Mn<sub>2</sub>O<sub>7</sub></a>                | $Fd\bar{3}m$ (227) | $I4_1/am'd'$ (141.557)  | $4/mm'm'$    | ×        | ✓   |
| 0.152  | <a href="#">LiFePO<sub>4</sub></a>                                       | $Pnma$ (62)        | $P2_1/c'$ (14.78)       | $2/m'$       | PT-wP    | ×   |
| 0.153  | <a href="#">Bi<sub>2</sub>RuMnO<sub>7</sub></a>                          | $Fd\bar{3}m$ (227) | $Fd'd'd$ (70.530)       | $m'm'm$      | ×        | ✓   |
| 0.154  | <a href="#">Er<sub>2</sub>Ru<sub>2</sub>O<sub>7</sub></a>                | $Fd\bar{3}m$ (227) | $I4_1'/am'd$ (141.554)  | $4'/mm'm$    | ×        | ×   |
| 0.155  | <a href="#">CaMnGe<sub>2</sub>O<sub>6</sub></a>                          | $C2/c$ (15)        | $P1'$ (2.6)             | $\bar{1}'$   | PT-wP    | ×   |
| 0.156  | <a href="#">CaMnGe<sub>2</sub>O<sub>6</sub></a>                          | $C2/c$ (15)        | $C2'/c$ (15.87)         | $2'/m$       | PT-wP    | ×   |
| 0.157  | <a href="#">Yb<sub>2</sub>Sn<sub>2</sub>O<sub>7</sub></a>                | $Fd\bar{3}m$ (227) | $I4_1/am'd'$ (141.557)  | $4/mm'm'$    | ×        | ✓   |
| 0.158  | <a href="#">Yb<sub>2</sub>Ti<sub>2</sub>O<sub>7</sub></a>                | $Fd\bar{3}m$ (227) | $I4_1/am'd'$ (141.557)  | $4/mm'm'$    | ×        | ✓   |
| 0.159  | <a href="#">DyCoO<sub>3</sub></a>                                        | $Pbnm$ (62)        | $Pn'm'a'$ (62.449)      | $m'm'm'$     | PT-wP    | ×   |
| 0.160  | <a href="#">TbCoO<sub>3</sub></a>                                        | $Pbnm$ (62)        | $Pnm'a$ (62.444)        | $m'mm$       | PT-wP    | ×   |
| 0.161  | <a href="#">CoSe<sub>2</sub>O<sub>5</sub></a>                            | $Pbcn$ (60)        | $Pb'cn$ (60.419)        | $m'mm$       | PT-wP    | ×   |
| 0.162  | <a href="#">NdCrTiO<sub>5</sub></a>                                      | $Pbam$ (55)        | $Pbam'$ (55.356)        | $m'mm$       | PT-wP    | ×   |
| 0.163  | <a href="#">MnPS<sub>3</sub></a>                                         | $C2/m$ (12)        | $C2'/m$ (12.60)         | $2'/m$       | PT-wP    | ×   |
| 0.164  | <a href="#">Y<sub>2</sub>MnCoO<sub>6</sub></a>                           | $P2_1/c$ (14)      | $P2_1'/c'$ (14.79)      | $2'/m'$      | ×        | ✓   |
| 0.165  | <a href="#">SrMn(VO<sub>4</sub>)(OH)</a>                                 | $P2_12_1'2_1$ (19) | $P2_1$ (4.7)            | $2$          | O-woP    | ✓   |
| 0.166  | <a href="#">Ce<sub>2</sub>PdGe<sub>3</sub></a>                           | $P4_2/mmc$ (131)   | $P4_2/m'm'c$ (131.440)  | $4'/m'm'm$   | PT-wP    | ×   |
| 0.167  | <a href="#">Nd<sub>3</sub>Sb<sub>3</sub>Mg<sub>2</sub>O<sub>14</sub></a> | $R\bar{3}m$ (166)  | $R\bar{3}m'$ (166.101)  | $\bar{3}m'$  | ×        | ✓   |

Continued on next page

TABLE S7 – continued from previous page

| BCS-ID | Formula                                                                                         | Parent                                   | MSG                                            | MPG             | SHG type | LMO |
|--------|-------------------------------------------------------------------------------------------------|------------------------------------------|------------------------------------------------|-----------------|----------|-----|
| 0.168  | <a href="#">NH<sub>4</sub>Fe<sub>2</sub>F<sub>6</sub></a>                                       | <i>Pnma</i> (62)                         | <i>Pnma</i> (62.441)                           | <i>mmm</i>      | ×        | ×   |
| 0.169  | <a href="#">U<sub>3</sub>As<sub>4</sub></a>                                                     | <i>I43d</i> (220)                        | <i>R3c'</i> (161.71)                           | <i>3m'</i>      | BW-woP   | ✓   |
| 0.170  | <a href="#">U<sub>3</sub>P<sub>4</sub></a>                                                      | <i>I43d</i> (220)                        | <i>R3c'</i> (161.71)                           | <i>3m'</i>      | BW-woP   | ✓   |
| 0.171  | <a href="#">DyScO<sub>3</sub></a>                                                               | <i>Pnma</i> (62)                         | <i>Pn'm'a'</i> (62.449)                        | <i>m'm'm'</i>   | PT-wP    | ×   |
| 0.172  | <a href="#">Y<sub>3</sub>Co<sub>3.25</sub>Al<sub>0.75</sub></a>                                 | <i>Cmcm</i> (63)                         | <i>Cm'cm'</i> (63.464)                         | <i>m'm'm</i>    | ×        | ✓   |
| 0.173  | <a href="#">Pr<sub>3</sub>Ru<sub>4</sub>Al<sub>12</sub></a>                                     | <i>P6<sub>3</sub>/mmc</i> (194)          | <i>Cm'c'm</i> (63.462)                         | <i>m'm'm</i>    | ×        | ✓   |
| 0.174  | <a href="#">Pr<sub>3</sub>Ru<sub>4</sub>Al<sub>12</sub></a>                                     | <i>P6<sub>3</sub>/mmc</i> (194)          | <i>C2'/c'</i> (15.89)                          | <i>2'/m'</i>    | ×        | ✓   |
| 0.175  | <a href="#">Ca<sub>2</sub>CoSi<sub>2</sub>O<sub>7</sub></a>                                     | <i>P4<sub>2</sub>1m</i> (113)            | <i>P2<sub>1</sub>2'<sub>1</sub>2'</i> (18.19)  | <i>2'2'2</i>    | BW-woP   | ✓   |
| 0.176  | <a href="#">Mn<sub>3</sub>Ti<sub>2</sub>Te<sub>6</sub></a>                                      | <i>P31c</i> (163)                        | <i>C2'/c'</i> (15.89)                          | <i>2'/m'</i>    | ×        | ✓   |
| 0.177  | <a href="#">Mn<sub>3</sub>GaN</a>                                                               | <i>Pm3m</i> (221)                        | <i>R3m</i> (166.97)                            | <i>3m</i>       | ×        | ×   |
| 0.178  | <a href="#">CoF<sub>2</sub></a>                                                                 | <i>P4<sub>2</sub>/mnm</i> (136)          | <i>P4<sub>2</sub>/mnm'</i> (136.499)           | <i>4'/mm'm</i>  | ×        | ×   |
| 0.179  | <a href="#">FeCl<sub>5</sub>D<sub>2</sub>O(ND<sub>4</sub>)<sub>2</sub></a>                      | <i>P2<sub>1</sub>/c</i> (14)             | <i>P2'<sub>1</sub></i> (4.9)                   | <i>2'</i>       | BW-wP    | ✓   |
| 0.180  | <a href="#">MnPS<sub>3</sub></a>                                                                | <i>R3</i> (148)                          | <i>P1'</i> (2.6)                               | <i>1'</i>       | PT-wP    | ×   |
| 0.181  | <a href="#">Nd<sub>15</sub>Ge<sub>9</sub>C<sub>0.39</sub></a>                                   | <i>P6<sub>3</sub>mc</i> (186)            | <i>P6<sub>3</sub>m'c'</i> (186.207)            | <i>6m'm'</i>    | BW-woP   | ✓   |
| 0.182  | <a href="#">KCrF<sub>4</sub></a>                                                                | <i>Pnma</i> (62)                         | <i>Pn'ma</i> (62.443)                          | <i>m'mm</i>     | PT-wP    | ×   |
| 0.183  | <a href="#">KMnFeF<sub>6</sub></a>                                                              | <i>P4<sub>2</sub>bc</i> (106)            | <i>Pb'a2'</i> (32.137)                         | <i>m'm2'</i>    | BW-woP   | ✓   |
| 0.184  | <a href="#">Nd<sub>5</sub>Si<sub>4</sub></a>                                                    | <i>P4<sub>1</sub>2<sub>1</sub>2</i> (92) | <i>P4<sub>1</sub>2'<sub>1</sub>2'</i> (92.114) | <i>42'2'</i>    | BW-woP   | ✓   |
| 0.185  | <a href="#">Nd<sub>5</sub>Ge<sub>4</sub></a>                                                    | <i>Pnma</i> (62)                         | <i>Pnm'a'</i> (62.447)                         | <i>m'm'm</i>    | ×        | ✓   |
| 0.186  | <a href="#">CeMnAsO</a>                                                                         | <i>P4/nmm</i> (129)                      | <i>P4'/n'm'm</i> (129.416)                     | <i>4'/m'm'm</i> | PT-wP    | ×   |
| 0.187  | <a href="#">CeMnAsO</a>                                                                         | <i>P4/nmm</i> (129)                      | <i>Pm'mn</i> (59.407)                          | <i>m'mm</i>     | PT-wP    | ×   |
| 0.188  | <a href="#">CeMnAsO</a>                                                                         | <i>P4/nmm</i> (129)                      | <i>P2'/c</i> (13.67)                           | <i>2'/m</i>     | PT-wP    | ×   |
| 0.189  | <a href="#">CeMn<sub>2</sub>Ge<sub>4</sub>O<sub>12</sub></a>                                    | <i>P4/nbm</i> (125)                      | <i>P4'/nbm'</i> (125.367)                      | <i>4'/mm'm</i>  | ×        | ×   |
| 0.190  | <a href="#">CeMnCoGe<sub>4</sub>O<sub>12</sub></a>                                              | <i>P4/nbm</i> (125)                      | <i>Pb'an'</i> (50.282)                         | <i>m'm'm</i>    | ×        | ✓   |
| 0.191  | <a href="#">BaCuF<sub>4</sub></a>                                                               | <i>Cmc2<sub>1</sub></i> (36)             | <i>Cm'c'2<sub>1</sub></i> (36.176)             | <i>m'm'2</i>    | BW-woP   | ✓   |
| 0.192  | <a href="#">RbFe<sub>2</sub>F<sub>6</sub></a>                                                   | <i>Pnma</i> (62)                         | <i>Pnma</i> (62.441)                           | <i>mmm</i>      | ×        | ×   |
| 0.193  | <a href="#">LiCoPO<sub>4</sub></a>                                                              | <i>Pnma</i> (62)                         | <i>Pnma'</i> (62.445)                          | <i>m'mm</i>     | PT-wP    | ×   |
| 0.194  | <a href="#">UPt<sub>2</sub>Si<sub>2</sub></a>                                                   | <i>P4/nmm</i> (129)                      | <i>P4/n'm'm'</i> (129.419)                     | <i>4/m'm'm'</i> | PT-wP    | ×   |
| 0.195  | <a href="#">Sr<sub>2</sub>Ir<sub>0.92</sub>Sn<sub>0.08</sub>O<sub>4</sub></a>                   | <i>I4<sub>1</sub>/acd</i> (142)          | <i>Ib'c'a</i> (73.551)                         | <i>m'm'm</i>    | ×        | ✓   |
| 0.196  | <a href="#">Co<sub>4</sub>Nb<sub>2</sub>O<sub>9</sub></a>                                       | <i>P3c1</i> (165)                        | <i>C2'/c'</i> (15.88)                          | <i>2/m'</i>     | PT-wP    | ×   |
| 0.197  | <a href="#">Co<sub>4</sub>Nb<sub>2</sub>O<sub>9</sub></a>                                       | <i>P3c1</i> (165)                        | <i>C2'/c'</i> (15.88)                          | <i>2/m'</i>     | PT-wP    | ×   |
| 0.198  | <a href="#">GdVO<sub>4</sub></a>                                                                | <i>I4<sub>1</sub>/amd</i> (141)          | <i>I4<sub>1</sub>/a'm'd</i> (141.556)          | <i>4'/m'm'm</i> | PT-wP    | ×   |
| 0.199  | <a href="#">Mn<sub>3</sub>Sn</a>                                                                | <i>P6<sub>3</sub>/mmc</i> (194)          | <i>Cmc'm'</i> (63.463)                         | <i>m'm'm</i>    | ×        | ✓   |
| 0.200  | <a href="#">Mn<sub>3</sub>Sn</a>                                                                | <i>P6<sub>3</sub>/mmc</i> (194)          | <i>Cm'cm'</i> (63.464)                         | <i>m'm'm</i>    | ×        | ✓   |
| 0.201  | <a href="#">Ca<sub>2</sub>PrCr<sub>2</sub>NbO<sub>9</sub></a>                                   | <i>Pnma</i> (62)                         | <i>Pn'ma</i> (62.446)                          | <i>m'm'm</i>    | ×        | ✓   |
| 0.202  | <a href="#">Ca<sub>2</sub>PrCr<sub>2</sub>TaO<sub>9</sub></a>                                   | <i>Pnma</i> (62)                         | <i>Pn'm'a</i> (62.446)                         | <i>m'm'm</i>    | ×        | ✓   |
| 0.203  | <a href="#">Mn<sub>3</sub>Ge</a>                                                                | <i>P6<sub>3</sub>/mmc</i> (194)          | <i>C2'/m'</i> (12.62)                          | <i>2'/m'</i>    | ×        | ✓   |
| 0.204  | <a href="#">Ca<sub>2</sub>MnReO<sub>6</sub></a>                                                 | <i>P2<sub>1</sub>/c</i> (14)             | <i>P2<sub>1</sub>/c</i> (14.75)                | <i>2/m</i>      | ×        | ✓   |
| 0.205  | <a href="#">Sr<sub>2</sub>MnReO<sub>6</sub></a>                                                 | <i>P2<sub>1</sub>/c</i> (14)             | <i>P2'<sub>1</sub>/c'</i> (14.79)              | <i>2'/m'</i>    | ×        | ✓   |
| 0.206  | <a href="#">Ca<sub>2</sub>Fe<sub>0.885</sub>Cr<sub>0.125</sub>Co<sub>0.8</sub>O<sub>6</sub></a> | <i>Pnma</i> (62)                         | <i>Pn'm'a</i> (62.446)                         | <i>m'm'm</i>    | ×        | ✓   |
| 0.207  | <a href="#">TlFe<sub>1.6</sub>Se<sub>2</sub></a>                                                | <i>I4/m</i> (87)                         | <i>I4/m</i> (87.75)                            | <i>4/m</i>      | ×        | ✓   |
| 0.208  | <a href="#">TlFe<sub>1.6</sub>Se<sub>2</sub></a>                                                | <i>I4/m</i> (87)                         | <i>C2'/m</i> (12.60)                           | <i>2'/m</i>     | PT-wP    | ×   |
| 0.209  | <a href="#">TlFe<sub>1.6</sub>Se<sub>2</sub></a>                                                | <i>I4/m</i> (87)                         | <i>I4/m'</i> (87.78)                           | <i>4/m'</i>     | PT-wP    | ×   |
| 0.210  | <a href="#">Sr<sub>2</sub>CoOsO<sub>6</sub></a>                                                 | <i>B2/n</i> (15)                         | <i>C2/c</i> (15.85)                            | <i>2/m</i>      | ×        | ✓   |
| 0.211  | <a href="#">Ca<sub>2</sub>MnO<sub>4</sub></a>                                                   | <i>I4<sub>1</sub>/acd</i> (142)          | <i>I4<sub>1</sub>/a'cd'</i> (142.568)          | <i>4'/m'm'm</i> | PT-wP    | ×   |
| 0.212  | <a href="#">Sr<sub>2</sub>Mn<sub>3</sub>As<sub>2</sub>O<sub>2</sub></a>                         | <i>I4/mmm</i> (139)                      | <i>I4'/m'm'm</i> (139.536)                     | <i>4'/m'm'm</i> | PT-wP    | ×   |
| 0.213  | <a href="#">Sr<sub>2</sub>Mn<sub>2</sub>CuAs<sub>2</sub>O<sub>2</sub></a>                       | <i>I4/mmm</i> (139)                      | <i>I4'/mm'm'</i> (139.537)                     | <i>4'/mm'm'</i> | ×        | ✓   |
| 0.214  | <a href="#">FePbBiO<sub>4</sub></a>                                                             | <i>P4<sub>2</sub>/mbc</i> (135)          | <i>Pmc2<sub>1</sub></i> (26.66)                | <i>mm2</i>      | O-wP     | ×   |
| 0.215  | <a href="#">BaNi<sub>2</sub>P<sub>2</sub>O<sub>8</sub></a>                                      | <i>R3</i> (148)                          | <i>P1'</i> (2.6)                               | <i>1'</i>       | PT-wP    | ×   |
| 0.216  | <a href="#">SrEr<sub>2</sub>O<sub>4</sub></a>                                                   | <i>Pnma</i> (62)                         | <i>Pnma'</i> (62.445)                          | <i>m'mm</i>     | PT-wP    | ×   |
| 0.217  | <a href="#">LiCrGe<sub>2</sub>O<sub>6</sub></a>                                                 | <i>P2<sub>1</sub>/c</i> (14)             | <i>P2'<sub>1</sub>/c</i> (14.77)               | <i>2'/m</i>     | PT-wP    | ×   |
| 0.218  | <a href="#">Co<sub>2</sub>SiO<sub>4</sub></a>                                                   | <i>Pnma</i> (62)                         | <i>Pnma</i> (62.441)                           | <i>mmm</i>      | ×        | ×   |
| 0.219  | <a href="#">Co<sub>2</sub>SiO<sub>4</sub></a>                                                   | <i>Pnma</i> (62)                         | <i>Pnma</i> (62.441)                           | <i>mmm</i>      | ×        | ×   |
| 0.220  | <a href="#">Mn<sub>2</sub>SiO<sub>4</sub></a>                                                   | <i>Pnma</i> (62)                         | <i>Pn'm'a</i> (62.446)                         | <i>m'm'm</i>    | ×        | ✓   |
| 0.221  | <a href="#">Fe<sub>2</sub>SiO<sub>4</sub></a>                                                   | <i>Pnma</i> (62)                         | <i>Pnma</i> (62.441)                           | <i>mmm</i>      | ×        | ×   |
| 0.222  | <a href="#">CuMnAs</a>                                                                          | <i>P4/nmm</i> (129)                      | <i>Pm'mn</i> (59.407)                          | <i>m'mm</i>     | PT-wP    | ×   |
| 0.223  | <a href="#">Cu<sub>0.95</sub>MnAs</a>                                                           | <i>Pnma</i> (62)                         | <i>Pn'ma</i> (62.443)                          | <i>m'mm</i>     | PT-wP    | ×   |
| 0.224  | <a href="#">Nd<sub>0.5</sub>Tb<sub>0.5</sub>Co<sub>2</sub></a>                                  | <i>Fd3m</i> (227)                        | <i>C2'/m'</i> (12.62)                          | <i>2'/m'</i>    | ×        | ✓   |
| 0.225  | <a href="#">Nd<sub>0.5</sub>Tb<sub>0.5</sub>Co<sub>2</sub></a>                                  | <i>Fd3m</i> (227)                        | <i>C2'/m'</i> (12.62)                          | <i>2'/m'</i>    | ×        | ✓   |

Continued on next page

TABLE S7 – continued from previous page

| BCS-ID | Formula                                                                                              | Parent             | MSG                    | MPG         | SHG type | LMO |
|--------|------------------------------------------------------------------------------------------------------|--------------------|------------------------|-------------|----------|-----|
| 0.226  | NdCo <sub>2</sub>                                                                                    | $Fd\bar{3}m$ (227) | $C2'/c'$ (15.89)       | $2'/m'$     | ×        | ✓   |
| 0.227  | NdCo <sub>2</sub>                                                                                    | $Fd\bar{3}m$ (227) | $I4_1/am'd'$ (141.557) | $4/mm'm'$   | ×        | ✓   |
| 0.228  | TbCo <sub>2</sub>                                                                                    | $Fd\bar{3}m$ (227) | $R\bar{3}m'$ (166.101) | $3m'$       | ×        | ✓   |
| 0.229  | Ba <sub>2</sub> MnSi <sub>2</sub> O <sub>7</sub>                                                     | $P42_1m$ (113)     | $P42_1m$ (113.267)     | $42m$       | O-woP    | ×   |
| 0.230  | K <sub>2</sub> CoP <sub>2</sub> O <sub>7</sub>                                                       | $P4_2/mnm$ (136)   | $Pn'nm$ (58.395)       | $m'mm$      | PT-wP    | ×   |
| 0.231  | TmMn <sub>3</sub> O <sub>6</sub>                                                                     | $Pmmn$ (59)        | $Pmm'n'$ (59.410)      | $m'm'm$     | ×        | ✓   |
| 0.232  | TmMn <sub>3</sub> O <sub>6</sub>                                                                     | $Pmmn$ (59)        | $Pm'm'n$ (59.409)      | $m'm'm$     | ×        | ✓   |
| 0.233  | Mn <sub>2</sub> FeSbO <sub>6</sub>                                                                   | $R\bar{3}$ (148)   | $P\bar{1}$ (2.4)       | $\bar{1}$   | ×        | ✓   |
| 0.234  | MnLaMnSbO <sub>6</sub>                                                                               | $P4_2/n$ (86)      | $P2'/c'$ (13.69)       | $2'/m'$     | ×        | ✓   |
| 0.235  | MnPrMnSbO <sub>6</sub>                                                                               | $P4_2/n$ (86)      | $P42/n$ (86.67)        | $4/m$       | ×        | ✓   |
| 0.236  | CaFe <sub>4</sub> Al <sub>8</sub>                                                                    | $I4/mmm$ (139)     | $I4'/mmm'$ (139.535)   | $4'/mm'm$   | ×        | ×   |
| 0.237  | Er <sub>2</sub> Sn <sub>2</sub> O <sub>7</sub>                                                       | $Fd\bar{3}m$ (227) | $I4_1/amd'$ (141.555)  | $4'/mm'm$   | ×        | ×   |
| 0.238  | Er <sub>2</sub> Pt <sub>2</sub> O <sub>7</sub>                                                       | $Fd\bar{3}m$ (227) | $I4_1'/amd'$ (141.555) | $4'/mm'm$   | ×        | ×   |
| 0.239  | Ca <sub>3</sub> LiRuO <sub>6</sub>                                                                   | $R\bar{3}c$ (167)  | $C2'/c'$ (15.89)       | $2'/m'$     | ×        | ✓   |
| 0.240  | Er <sub>2</sub> Cu <sub>2</sub> O <sub>5</sub>                                                       | $Pna2_1$ (33)      | $Pna2_1$ (33.144)      | $mm2$       | O-woP    | ×   |
| 0.241  | Y <sub>2</sub> Cu <sub>2</sub> O <sub>5</sub>                                                        | $Pna2_1$ (33)      | $Pna2_1$ (33.144)      | $mm2$       | O-woP    | ×   |
| 0.242  | Tm <sub>2</sub> Cu <sub>2</sub> O <sub>5</sub>                                                       | $Pna2_1$ (33)      | $Pn'a'2_1$ (33.148)    | $m'm'2$     | BW-woP   | ✓   |
| 0.243  | Li <sub>2</sub> Fe(SO <sub>4</sub> ) <sub>2</sub>                                                    | $Pbca$ (61)        | $P2_1/c$ (14.77)       | $2'/m$      | PT-wP    | ×   |
| 0.244  | Li <sub>2</sub> Co(SO <sub>4</sub> ) <sub>2</sub>                                                    | $Pbca$ (61)        | $Pb'c'a'$ (61.437)     | $m'm'm'$    | PT-wP    | ×   |
| 0.245  | Li <sub>1.5</sub> Fe(SO <sub>4</sub> ) <sub>2</sub>                                                  | $Pbca$ (61)        | $P2_1/c$ (14.77)       | $2'/m$      | PT-wP    | ×   |
| 0.246  | LiFe(SO <sub>4</sub> ) <sub>2</sub>                                                                  | $Pbca$ (61)        | $Pb'c'a'$ (61.437)     | $m'm'm'$    | PT-wP    | ×   |
| 0.247  | Nd <sub>2</sub> NiO <sub>4.11</sub>                                                                  | $P4_2/nm$ (138)    | $P4_2/nc'm'$ (138.525) | $4'/mm'm'$  | ×        | ✓   |
| 0.248  | TbPt <sub>0.8</sub> Cu <sub>0.2</sub>                                                                | $Pnma$ (62)        | $Pn'm'a$ (62.446)      | $m'm'm$     | ×        | ✓   |
| 0.249  | NdNi <sub>0.6</sub> Cu <sub>0.4</sub>                                                                | $Pnma$ (62)        | $Pnm'a'$ (62.447)      | $m'm'm$     | ×        | ✓   |
| 0.250  | (NH <sub>2</sub> (CH <sub>3</sub> ) <sub>2</sub> )(FeCoP <sub>2</sub> O <sub>7</sub> )               | $Pbca$ (61)        | $C2'/c'$ (15.89)       | $2'/m'$     | ×        | ✓   |
| 0.251  | (NH <sub>2</sub> (CH <sub>3</sub> ) <sub>2</sub> )(FeMn <sub>2</sub> P <sub>2</sub> O <sub>7</sub> ) | $Pbca$ (61)        | $C2'/c'$ (15.89)       | $2'/m'$     | ×        | ✓   |
| 0.252  | Cs <sub>2</sub> FeCl <sub>5</sub> .D <sub>2</sub> O                                                  | $C2/c$ (15)        | $C2'/c$ (15.87)        | $2'/m$      | PT-wP    | ×   |
| 0.253  | Cs <sub>2</sub> FeCl <sub>5</sub> .D <sub>2</sub> O                                                  | $C2/c$ (15)        | $C2$ (5.13)            | $2$         | O-wP     | ✓   |
| 0.254  | [C(ND <sub>2</sub> ) <sub>3</sub> ]Cu(DCO <sub>2</sub> ) <sub>2</sub>                                | $Pna2_1$ (33)      | $Pna2_1$ (33.144)      | $mm2$       | O-woP    | ×   |
| 0.255  | [C(ND <sub>2</sub> ) <sub>3</sub> ]Cu(DCO <sub>2</sub> ) <sub>2</sub>                                | $Pna2_1$ (33)      | $Pn'a'2_1$ (33.148)    | $m'm'2$     | BW-woP   | ✓   |
| 0.256  | [C(ND <sub>2</sub> ) <sub>3</sub> ]Mn(DCO <sub>2</sub> ) <sub>2</sub>                                | $Pnma$ (52)        | $Pn'n'a$ (52.310)      | $m'm'm$     | ×        | ✓   |
| 0.257  | [C(ND <sub>2</sub> ) <sub>3</sub> ]Co(DCO <sub>2</sub> ) <sub>2</sub>                                | $Pnma$ (52)        | $Pn'na'$ (52.312)      | $m'm'm$     | ×        | ✓   |
| 0.258  | Li <sub>3</sub> Fe <sub>2</sub> (PO <sub>4</sub> ) <sub>3</sub>                                      | $P2_1/n$ (14)      | $P2_1'/c'$ (14.79)     | $2'/m'$     | ×        | ✓   |
| 0.259  | Li <sub>3</sub> Fe <sub>2</sub> (PO <sub>4</sub> ) <sub>3</sub>                                      | $R\bar{3}$ (148)   | $R\bar{3}$ (148.17)    | $\bar{3}$   | ×        | ✓   |
| 0.260  | CuFePO <sub>5</sub>                                                                                  | $Pnma$ (62)        | $Pnma$ (62.441)        | $mmm$       | ×        | ×   |
| 0.261  | NiFePO <sub>5</sub>                                                                                  | $Pnma$ (62)        | $Pnma$ (62.441)        | $mmm$       | ×        | ×   |
| 0.262  | CoFePO <sub>5</sub>                                                                                  | $Pnma$ (62)        | $Pnm'a'$ (62.447)      | $m'm'm$     | ×        | ✓   |
| 0.263  | Fe <sub>2</sub> PO <sub>5</sub>                                                                      | $Pnma$ (62)        | $Pnma$ (62.441)        | $mmm$       | ×        | ×   |
| 0.264  | Fe <sub>3</sub> (PO <sub>4</sub> ) <sub>2</sub>                                                      | $P2_1/c$ (14)      | $P2_1'/c'$ (14.78)     | $2'/m'$     | PT-wP    | ×   |
| 0.265  | Mn <sub>3</sub> (Co <sub>0.61</sub> Mn <sub>0.39</sub> )P <sub>2</sub> O <sub>7</sub>                | $Pm\bar{3}m$ (221) | $R\bar{3}$ (148.17)    | $\bar{3}$   | ×        | ✓   |
| 0.266  | Na <sub>2</sub> BaCo(VO <sub>4</sub> ) <sub>2</sub>                                                  | $P3m1$ (164)       | $P3m'1$ (164.89)       | $\bar{3}m'$ | ×        | ✓   |
| 0.267  | YbMnBi <sub>2</sub>                                                                                  | $P4/nmm$ (129)     | $P4'/n'm'm$ (129.416)  | $4'/m'm'm$  | PT-wP    | ×   |
| 0.268  | Tb <sub>2</sub> MnNiO <sub>6</sub>                                                                   | $P2_1/c$ (14)      | $P2_1'$ (4.9)          | $2'$        | BW-wP    | ✓   |
| 0.269  | Tb <sub>2</sub> MnNiO <sub>6</sub>                                                                   | $P2_1/c$ (14)      | $P2_1'/c'$ (14.79)     | $2'/m'$     | ×        | ✓   |
| 0.270  | Tb <sub>2</sub> MnNiO <sub>6</sub>                                                                   | $P2_1/c$ (14)      | $P2_1'/c'$ (14.79)     | $2'/m'$     | ×        | ✓   |
| 0.271  | Tb <sub>2</sub> MnNiO <sub>6</sub>                                                                   | $P2_1/c$ (14)      | $P2_1'/c'$ (14.79)     | $2'/m'$     | ×        | ✓   |
| 0.272  | Tb <sub>2</sub> MnNiO <sub>6</sub>                                                                   | $P2_1/c$ (14)      | $P2_1/c$ (14.75)       | $2/m$       | ×        | ✓   |
| 0.273  | Mn <sub>3</sub> ZnN                                                                                  | $Pm\bar{3}m$ (221) | $R\bar{3}m$ (166.97)   | $\bar{3}m$  | ×        | ×   |
| 0.274  | Mn <sub>4</sub> N                                                                                    | $Pm\bar{3}m$ (221) | $R\bar{3}m'$ (166.101) | $\bar{3}m'$ | ×        | ✓   |
| 0.275  | Mn <sub>3</sub> AlN                                                                                  | $Pm\bar{3}m$ (221) | $R\bar{3}m'$ (166.101) | $\bar{3}m'$ | ×        | ✓   |
| 0.276  | Mn <sub>3</sub> AlN                                                                                  | $Pm\bar{3}m$ (221) | $Cmm'm'$ (65.486)      | $m'm'm$     | ×        | ✓   |
| 0.277  | MgMnO <sub>3</sub>                                                                                   | $R\bar{3}$ (148)   | $R\bar{3}'$ (148.19)   | $\bar{3}'$  | PT-wP    | ×   |
| 0.278  | Cu <sub>0.82</sub> Mn <sub>1.18</sub> As                                                             | $P\bar{6}$ (174)   | $P\bar{6}'$ (174.135)  | $\bar{6}'$  | BW-woP   | ×   |
| 0.279  | Mn <sub>3</sub> As                                                                                   | $P6_3/mmc$ (194)   | $Cmc'm'$ (63.463)      | $m'm'm$     | ×        | ✓   |
| 0.280  | Mn <sub>3</sub> As                                                                                   | $P6_3/mmc$ (194)   | $Cm'cm'$ (63.464)      | $m'm'm$     | ×        | ✓   |
| 0.281  | Co <sub>2</sub> V <sub>2</sub> O <sub>7</sub>                                                        | $P2_1/c$ (14)      | $P2_1'/c'$ (14.78)     | $2'/m'$     | PT-wP    | ×   |
| 0.282  | U <sub>14</sub> Au <sub>5</sub> 1                                                                    | $P6/m$ (175)       | $P6'/m$ (175.139)      | $6'/m$      | PT-wP    | ×   |

Continued on next page

TABLE S7 – continued from previous page

| BCS-ID | Formula                                                                       | Parent                                               | MSG                                                     | MPG             | SHG type | LMO |
|--------|-------------------------------------------------------------------------------|------------------------------------------------------|---------------------------------------------------------|-----------------|----------|-----|
| 0.283  | <a href="#">U<sub>14</sub>Au<sub>5</sub>I</a>                                 | <i>P6/m</i> (175)                                    | <i>P6/m'</i> (175.140)                                  | <i>6/m'</i>     | PT-wP    | ×   |
| 0.284  | <a href="#">KO<sub>8</sub>O<sub>4</sub></a>                                   | <i>I4<sub>1</sub>/a</i> (88)                         | <i>I4<sub>1</sub>'/a'</i> (88.85)                       | <i>4'/m'</i>    | PT-wP    | ×   |
| 0.285  | <a href="#">KRuO<sub>4</sub></a>                                              | <i>I4<sub>1</sub>/a</i> (88)                         | <i>I4<sub>1</sub>'/a'</i> (88.85)                       | <i>4'/m'</i>    | PT-wP    | ×   |
| 0.286  | <a href="#">Mn<sub>5</sub>Ge<sub>3</sub></a>                                  | <i>P6<sub>3</sub>/mcm</i> (193)                      | <i>P6<sub>3</sub>/mc'm'</i> (193.260)                   | <i>6'/mm'm'</i> | ×        | ✓   |
| 0.287  | <a href="#">SrCo(VO<sub>4</sub>)(OH)</a>                                      | <i>P2<sub>1</sub>2<sub>1</sub>2<sub>1</sub></i> (19) | <i>P2<sub>1</sub>2<sub>1</sub>2<sub>1</sub></i> (19.25) | 222             | O-woP    | ×   |
| 0.288  | <a href="#">NdMnO<sub>3</sub></a>                                             | <i>Pnma</i> (62)                                     | <i>Pn'ma'</i> (62.448)                                  | <i>m'm'm</i>    | ×        | ✓   |
| 0.289  | <a href="#">NdMnO<sub>3</sub></a>                                             | <i>Pnma</i> (62)                                     | <i>Pn'ma'</i> (62.448)                                  | <i>m'm'm</i>    | ×        | ✓   |
| 0.290  | <a href="#">CeCu<sub>2</sub></a>                                              | <i>Imma</i> (74)                                     | <i>Im'm'a'</i> (74.560)                                 | <i>m'm'm'</i>   | PT-wP    | ×   |
| 0.291  | <a href="#">Ti<sub>2</sub>NiMnO<sub>6</sub></a>                               | <i>P2<sub>1</sub>/c</i> (14)                         | <i>P2<sub>1</sub>/c</i> (14.75)                         | <i>2/m</i>      | ×        | ✓   |
| 0.292  | <a href="#">NiTe<sub>2</sub>O<sub>5</sub></a>                                 | <i>Pnma</i> (62)                                     | <i>Pnma</i> (62.441)                                    | <i>mmm</i>      | ×        | ×   |
| 0.293  | <a href="#">(Tm<sub>0.7</sub>Mn<sub>0.3</sub>)MnO<sub>4</sub></a>             | <i>Pnma</i> (62)                                     | <i>Pnm'a'</i> (62.447)                                  | <i>m'm'm</i>    | ×        | ✓   |
| 0.294  | <a href="#">Cu<sub>4</sub>(OD)<sub>6</sub>FBr</a>                             | <i>Pnma</i> (62)                                     | <i>Pn'm'a</i> (62.446)                                  | <i>m'm'm</i>    | ×        | ✓   |
| 0.295  | <a href="#">Cu<sub>2</sub>(OD)<sub>3</sub>Cl</a>                              | <i>P2<sub>1</sub>/c</i> (14)                         | <i>P2<sub>1</sub>/c</i> (14.75)                         | <i>2/m</i>      | ×        | ✓   |
| 0.296  | <a href="#">Cu<sub>2</sub>(OD)<sub>3</sub>Cl</a>                              | <i>P2<sub>1</sub>/c</i> (14)                         | <i>P2<sub>1</sub>/c</i> (14.75)                         | <i>2/m</i>      | ×        | ✓   |
| 0.297  | <a href="#">NaCrGe<sub>2</sub>O<sub>6</sub></a>                               | <i>C2/c</i> (15)                                     | <i>C2'/c'</i> (15.89)                                   | <i>2'/m'</i>    | ×        | ✓   |
| 0.298  | <a href="#">Na<sub>2</sub>BaFe(VO<sub>4</sub>)<sub>2</sub></a>                | <i>C2/c</i> (15)                                     | <i>C2'/c'</i> (15.89)                                   | <i>2'/m'</i>    | ×        | ✓   |
| 0.299  | <a href="#">Fe<sub>2</sub>O<sub>3</sub></a>                                   | <i>Pna2<sub>1</sub></i> (33)                         | <i>Pna'2<sub>1</sub>'</i> (33.147)                      | <i>m'm2'</i>    | BW-woP   | ✓   |
| 0.300  | <a href="#">Fe<sub>2</sub>O<sub>3</sub></a>                                   | <i>Pna2<sub>1</sub></i> (33)                         | <i>Pna'2<sub>1</sub>'</i> (33.147)                      | <i>m'm2'</i>    | BW-woP   | ✓   |
| 0.301  | <a href="#">Sr<sub>2</sub>CoTeO<sub>6</sub></a>                               | <i>P2<sub>1</sub>/n</i> (14)                         | <i>P2<sub>1</sub>/c</i> (14.75)                         | <i>2/m</i>      | ×        | ✓   |
| 0.302  | <a href="#">Sr<sub>2</sub>Co<sub>0.9</sub>Mg<sub>0.1</sub>TeO<sub>6</sub></a> | <i>P2<sub>1</sub>/n</i> (14)                         | <i>P2<sub>1</sub>/c</i> (14.75)                         | <i>2/m</i>      | ×        | ✓   |
| 0.303  | <a href="#">BaCrF<sub>5</sub></a>                                             | <i>P2<sub>1</sub>2<sub>1</sub>2<sub>1</sub></i> (19) | <i>P2<sub>1</sub>2<sub>1</sub>2<sub>1</sub></i> (19.27) | <i>2'2'2</i>    | BW-woP   | ✓   |
| 0.304  | <a href="#">Pr<sub>0.5</sub>Sr<sub>0.5</sub>CoO<sub>3</sub></a>               | <i>Imma</i> (74)                                     | <i>Im'm'a</i> (74.558)                                  | <i>m'm'm</i>    | ×        | ✓   |
| 0.305  | <a href="#">Pr<sub>0.5</sub>Sr<sub>0.5</sub>CoO<sub>3</sub></a>               | <i>I4/mcm</i> (140)                                  | <i>Fm'm'm</i> (69.524)                                  | <i>m'm'm</i>    | ×        | ✓   |
| 0.306  | <a href="#">GaFeO<sub>3</sub></a>                                             | <i>R3c</i> (161)                                     | <i>Cc'</i> (9.39)                                       | <i>m'</i>       | BW-woP   | ✓   |
| 0.307  | <a href="#">ScCrO<sub>3</sub></a>                                             | <i>Pnma</i> (62)                                     | <i>Pnma</i> (62.441)                                    | <i>mmm</i>      | ×        | ×   |
| 0.308  | <a href="#">InCrO<sub>3</sub></a>                                             | <i>Pnma</i> (62)                                     | <i>Pnma</i> (62.441)                                    | <i>mmm</i>      | ×        | ×   |
| 0.309  | <a href="#">TlCrO<sub>3</sub></a>                                             | <i>Pnma</i> (62)                                     | <i>Pnma</i> (62.441)                                    | <i>mmm</i>      | ×        | ×   |
| 0.310  | <a href="#">NaMnFeF<sub>6</sub></a>                                           | <i>P321</i> (150)                                    | <i>P32'1</i> (150.27)                                   | <i>32'</i>      | BW-woP   | ✓   |
| 0.311  | <a href="#">CoGeO<sub>3</sub></a>                                             | <i>Pbca</i> (61)                                     | <i>Pb'ca</i> (61.435)                                   | <i>m'mm</i>     | PT-wP    | ×   |
| 0.312  | <a href="#">MnGeO<sub>3</sub></a>                                             | <i>C2/c</i> (15)                                     | <i>C2'/c</i> (15.87)                                    | <i>2'/m</i>     | PT-wP    | ×   |
| 0.313  | <a href="#">MnGeO<sub>3</sub></a>                                             | <i>Pbca</i> (61)                                     | <i>Pb'ca</i> (61.435)                                   | <i>m'mm</i>     | PT-wP    | ×   |
| 0.314  | <a href="#">ZrCo<sub>2</sub>Ge<sub>4</sub>O<sub>12</sub></a>                  | <i>P4/nbm</i> (125)                                  | <i>Pb'an'</i> (50.282)                                  | <i>m'm'm</i>    | ×        | ✓   |
| 0.315  | <a href="#">ZrMn<sub>2</sub>Ge<sub>4</sub>O<sub>12</sub></a>                  | <i>P4/nbm</i> (125)                                  | <i>P4'/nbm'</i> (125.367)                               | <i>4'/mm'm</i>  | ×        | ×   |
| 0.316  | <a href="#">DyCrWO<sub>6</sub></a>                                            | <i>Pna2<sub>1</sub></i> (33)                         | <i>P2<sub>1</sub></i> (4.7)                             | 2               | O-woP    | ✓   |
| 0.317  | <a href="#">Ho<sub>2</sub>CoMnO<sub>6</sub></a>                               | <i>P2<sub>1</sub>/c</i> (14)                         | <i>P2<sub>1</sub>'/c'</i> (14.79)                       | <i>2'/m'</i>    | ×        | ✓   |
| 0.318  | <a href="#">Tm<sub>2</sub>CoMnO<sub>6</sub></a>                               | <i>P2<sub>1</sub>/c</i> (14)                         | <i>P2<sub>1</sub>'/c'</i> (14.79)                       | <i>2'/m'</i>    | ×        | ✓   |
| 0.319  | <a href="#">Tm<sub>2</sub>CoMnO<sub>6</sub></a>                               | <i>P2<sub>1</sub>/c</i> (14)                         | <i>P2<sub>1</sub>'/c'</i> (14.79)                       | <i>2'/m'</i>    | ×        | ✓   |
| 0.320  | <a href="#">U<sub>2</sub>Pd<sub>2</sub>In</a>                                 | <i>P4/mbm</i> (127)                                  | <i>P4'/m'bm'</i> (127.394)                              | <i>4'/m'm'm</i> | PT-wP    | ×   |
| 0.321  | <a href="#">U<sub>2</sub>Pd<sub>2</sub>Sn</a>                                 | <i>P4/mbm</i> (127)                                  | <i>P4'/m'bm'</i> (127.394)                              | <i>4'/m'm'm</i> | PT-wP    | ×   |
| 0.322  | <a href="#">Cu<sub>1.94</sub>Mn<sub>1.06</sub>BO<sub>5</sub></a>              | <i>P2<sub>1</sub>/c</i> (14)                         | <i>P2<sub>1</sub>'/c'</i> (14.79)                       | <i>2'/m'</i>    | ×        | ✓   |
| 0.323  | <a href="#">LaCrO<sub>3</sub></a>                                             | <i>Pnma</i> (62)                                     | <i>Pnma</i> (62.441)                                    | <i>mmm</i>      | ×        | ×   |
| 0.324  | <a href="#">CdYb<sub>2</sub>S<sub>4</sub></a>                                 | <i>Fd3m</i> (227)                                    | <i>I4<sub>1</sub>/amd</i> (141.551)                     | <i>4'/mmm</i>   | ×        | ×   |
| 0.325  | <a href="#">CdYb<sub>2</sub>Se<sub>4</sub></a>                                | <i>Fd3m</i> (227)                                    | <i>I4<sub>1</sub>/amd</i> (141.551)                     | <i>4'/mmm</i>   | ×        | ×   |
| 0.326  | <a href="#">Nd<sub>2</sub>Sn<sub>2</sub>O<sub>7</sub></a>                     | <i>Fd3m</i> (227)                                    | <i>Fd3m'</i> (227.131)                                  | <i>m3m'</i>     | ×        | ×   |
| 0.327  | <a href="#">CsMnF<sub>4</sub></a>                                             | <i>P4/nmm</i> (129)                                  | <i>Pmm'n'</i> (59.410)                                  | <i>m'm'm</i>    | ×        | ✓   |
| 0.328  | <a href="#">KMnF<sub>4</sub></a>                                              | <i>P2<sub>1</sub>/a</i> (14)                         | <i>P2<sub>1</sub>'/c'</i> (14.79)                       | <i>2'/m'</i>    | ×        | ✓   |
| 0.329  | <a href="#">RbMnF<sub>4</sub></a>                                             | <i>P2<sub>1</sub>/a</i> (14)                         | <i>P1</i> (2.4)                                         | 1               | ×        | ✓   |
| 0.330  | <a href="#">ErGe<sub>3</sub></a>                                              | <i>Cmcm</i> (63)                                     | <i>P2<sub>1</sub>/m'</i> (11.53)                        | <i>2/m'</i>     | PT-wP    | ×   |
| 0.331  | <a href="#">Fe<sub>2</sub>Mo<sub>3</sub>O<sub>8</sub></a>                     | <i>P6<sub>3</sub>mc</i> (186)                        | <i>P6<sub>3</sub>m'c</i> (186.205)                      | <i>6'mm'</i>    | BW-woP   | ×   |
| 0.332  | <a href="#">Co<sub>2</sub>Mo<sub>3</sub>O<sub>8</sub></a>                     | <i>P6<sub>3</sub>mc</i> (186)                        | <i>P6<sub>3</sub>m'c</i> (186.205)                      | <i>6'mm'</i>    | BW-woP   | ×   |
| 0.333  | <a href="#">Mn<sub>2</sub>Mo<sub>3</sub>O<sub>8</sub></a>                     | <i>P6<sub>3</sub>mc</i> (186)                        | <i>P6<sub>3</sub>m'c'</i> (186.207)                     | <i>6m'm'</i>    | BW-woP   | ✓   |
| 0.334  | <a href="#">CoF<sub>3</sub></a>                                               | <i>R3c</i> (167)                                     | <i>R3c</i> (167.103)                                    | <i>3m</i>       | ×        | ×   |
| 0.335  | <a href="#">FeF<sub>3</sub></a>                                               | <i>R3c</i> (167)                                     | <i>C2'/c'</i> (15.89)                                   | <i>2'/m'</i>    | ×        | ✓   |
| 0.336  | <a href="#">NdFeO<sub>3</sub></a>                                             | <i>Pnma</i> (62)                                     | <i>Pn'ma'</i> (62.448)                                  | <i>m'm'm</i>    | ×        | ✓   |
| 0.337  | <a href="#">NdFeO<sub>3</sub></a>                                             | <i>Pnma</i> (62)                                     | <i>P2<sub>1</sub>'/c'</i> (14.79)                       | <i>2'/m'</i>    | ×        | ✓   |
| 0.338  | <a href="#">Co<sub>2</sub>Mo<sub>3</sub>O<sub>8</sub></a>                     | <i>P6<sub>3</sub>mc</i> (186)                        | <i>P6<sub>3</sub>m'c</i> (186.205)                      | <i>6'mm'</i>    | BW-woP   | ×   |
| 0.339  | <a href="#">Nd<sub>2</sub>Hf<sub>2</sub>O<sub>7</sub></a>                     | <i>Fd3m</i> (227)                                    | <i>Fd3m'</i> (227.131)                                  | <i>m3m'</i>     | ×        | ×   |

Continued on next page

TABLE S7 – continued from previous page

| BCS-ID | Formula                                                                                  | Parent                          | MSG                                                     | MPG             | SHG type | LMO |
|--------|------------------------------------------------------------------------------------------|---------------------------------|---------------------------------------------------------|-----------------|----------|-----|
| 0.340  | Nd <sub>2</sub> Zr <sub>2</sub> O <sub>7</sub>                                           | <i>Fd3m</i> (227)               | <i>Fd3m'</i> (227.131)                                  | <i>m3m'</i>     | ×        | ×   |
| 0.341  | DyGe <sub>1.75</sub>                                                                     | <i>Cmmm</i> (65)                | <i>Cm'mm</i> (65.483)                                   | <i>m'mm</i>     | PT-wP    | ×   |
| 0.342  | Tb <sub>3</sub> Ge <sub>5</sub>                                                          | <i>Fdd2</i> (43)                | <i>Fdd2</i> (43.224)                                    | <i>mm2</i>      | O-woP    | ×   |
| 0.343  | TbGe <sub>2</sub>                                                                        | <i>Cmmm</i> (65)                | <i>Cm'mm</i> (65.483)                                   | <i>m'mm</i>     | PT-wP    | ×   |
| 0.344  | ErGe <sub>1.83</sub>                                                                     | <i>Cmc2<sub>1</sub></i> (36)    | <i>Cmc2<sub>1</sub></i> (36.172)                        | <i>mm2</i>      | O-woP    | ×   |
| 0.345  | Tb <sub>2</sub> C <sub>3</sub>                                                           | <i>I43d</i> (220)               | <i>Fd'd2'</i> (43.226)                                  | <i>m'm2'</i>    | BW-woP   | ✓   |
| 0.346  | Tb <sub>2</sub> ReC <sub>2</sub>                                                         | <i>Pnma</i> (62)                | <i>Pnma'</i> (62.445)                                   | <i>m'mm</i>     | PT-wP    | ×   |
| 0.347  | Er <sub>2</sub> ReC <sub>2</sub>                                                         | <i>Pnma</i> (62)                | <i>P2<sub>1</sub>/c</i> (14.77)                         | <i>2'/m</i>     | PT-wP    | ×   |
| 0.348  | Bi <sub>2</sub> CuO <sub>4</sub>                                                         | <i>P4/ncc</i> (130)             | <i>P4/n'c'c'</i> (130.431)                              | <i>4/m'm'm'</i> | PT-wP    | ×   |
| 0.349  | Nd <sub>2</sub> NiO <sub>4</sub>                                                         | <i>P4<sub>2</sub>/ncm</i> (138) | <i>P4<sub>2</sub>/nc'm'</i> (138.525)                   | <i>4/mm'm'</i>  | ×        | ✓   |
| 0.350  | TbAlO <sub>3</sub>                                                                       | <i>Pbnm</i> (62)                | <i>Pn'm'a'</i> (62.449)                                 | <i>m'm'm'</i>   | PT-wP    | ×   |
| 0.351  | TbFeO <sub>3</sub>                                                                       | <i>Pbnm</i> (62)                | <i>Pn'ma'</i> (62.448)                                  | <i>m'm'm</i>    | ×        | ✓   |
| 0.352  | TbFeO <sub>3</sub>                                                                       | <i>Pbnm</i> (62)                | <i>Pn'm'a</i> (62.446)                                  | <i>m'm'm</i>    | ×        | ✓   |
| 0.353  | TbFeO <sub>3</sub>                                                                       | <i>Pbnm</i> (62)                | <i>P2<sub>1</sub>2<sub>1</sub>2<sub>1</sub></i> (19.27) | <i>2'2'2</i>    | BW-wP    | ✓   |
| 0.354  | TbCrO <sub>3</sub>                                                                       | <i>Pbnm</i> (62)                | <i>Pn'm'a</i> (62.446)                                  | <i>m'm'm</i>    | ×        | ✓   |
| 0.355  | Mn <sub>2.85</sub> Ga <sub>1.15</sub>                                                    | <i>P6<sub>3</sub>/mmc</i> (194) | <i>P6<sub>3</sub>/m'm'c</i> (194.268)                   | <i>6'/m'mm'</i> | ×        | ×   |
| 0.356  | Mn <sub>2.85</sub> Ga <sub>1.15</sub>                                                    | <i>I4/mmm</i> (139)             | <i>I4/mm'm'</i> (139.537)                               | <i>4/mm'm'</i>  | ×        | ✓   |
| 0.357  | CaFe <sub>5</sub> O <sub>7</sub>                                                         | <i>P2<sub>1</sub>/m</i> (11)    | <i>P2<sub>1</sub>/m</i> (11.50)                         | <i>2/m</i>      | ×        | ✓   |
| 0.358  | CaFe <sub>5</sub> O <sub>7</sub>                                                         | <i>P2<sub>1</sub>/m</i> (11)    | <i>P2<sub>1</sub>'/m'</i> (11.54)                       | <i>2'/m'</i>    | ×        | ✓   |
| 0.359  | Mn <sub>2</sub> ScSbO <sub>6</sub>                                                       | <i>R3</i> (146)                 | <i>P1</i> (1.1)                                         | <i>1</i>        | O-woP    | ✓   |
| 0.360  | Mn <sub>2</sub> ScSbO <sub>6</sub>                                                       | <i>P2<sub>1</sub>/n</i> (14)    | <i>P2<sub>1</sub>/c</i> (14.75)                         | <i>2/m</i>      | ×        | ✓   |
| 0.361  | Sr <sub>3</sub> LiRuO <sub>6</sub>                                                       | <i>R3c</i> (167)                | <i>C2'/c'</i> (15.89)                                   | <i>2'/m'</i>    | ×        | ✓   |
| 0.362  | RbFeCl <sub>5</sub> (D <sub>2</sub> O)                                                   | <i>Pnma</i> (62)                | <i>Pn'm'a'</i> (62.449)                                 | <i>m'm'm'</i>   | PT-wP    | ×   |
| 0.363  | KFeCl <sub>5</sub> (D <sub>2</sub> O)                                                    | <i>Pnma</i> (62)                | <i>Pn'm'a'</i> (62.449)                                 | <i>m'm'm'</i>   | PT-wP    | ×   |
| 0.364  | SrCr <sub>2</sub> As <sub>2</sub>                                                        | <i>I4/mmm</i> (139)             | <i>I4'/m'm'm</i> (139.536)                              | <i>4'/m'm'm</i> | PT-wP    | ×   |
| 0.365  | BaCr <sub>2</sub> As <sub>2</sub>                                                        | <i>I4/mmm</i> (139)             | <i>I4'/m'm'm</i> (139.536)                              | <i>4'/m'm'm</i> | PT-wP    | ×   |
| 0.366  | BaCrFeAs <sub>2</sub>                                                                    | <i>I4/mmm</i> (139)             | <i>I4'/m'm'm</i> (139.536)                              | <i>4'/m'm'm</i> | PT-wP    | ×   |
| 0.367  | EuCr <sub>2</sub> As <sub>2</sub>                                                        | <i>I4/mmm</i> (139)             | <i>I4m'2'</i> (119.319)                                 | <i>42'm'</i>    | BW-wP    | ✓   |
| 0.368  | (CH <sub>3</sub> NH <sub>3</sub> )(Co(CO) <sub>2</sub> ) <sub>2</sub>                    | <i>Pnma</i> (62)                | <i>Pn'ma'</i> (62.448)                                  | <i>m'm'm</i>    | ×        | ✓   |
| 0.369  | (CH <sub>3</sub> NH <sub>3</sub> )(Co(CO) <sub>2</sub> ) <sub>2</sub>                    | <i>P2<sub>1</sub>/n</i> (14)    | <i>P2<sub>1</sub>'/c'</i> (14.79)                       | <i>2'/m'</i>    | ×        | ✓   |
| 0.370  | NdMnO <sub>3</sub>                                                                       | <i>Pnma</i> (62)                | <i>Pn'ma'</i> (62.448)                                  | <i>m'm'm</i>    | ×        | ✓   |
| 0.371  | NdMnO <sub>3</sub>                                                                       | <i>Pnma</i> (62)                | <i>Pn'ma'</i> (62.448)                                  | <i>m'm'm</i>    | ×        | ✓   |
| 0.372  | DyCrO <sub>4</sub>                                                                       | <i>I4<sub>1</sub>/a</i> (88)    | <i>C2'/c</i> (15.87)                                    | <i>2'/m</i>     | PT-wP    | ×   |
| 0.373  | La <sub>0.75</sub> Bi <sub>0.25</sub> Fe <sub>0.5</sub> Cr <sub>1.5</sub> O <sub>6</sub> | <i>Pnma</i> (62)                | <i>Pnma</i> (62.441)                                    | <i>mmm</i>      | ×        | ×   |
| 0.374  | YNi <sub>4</sub> Si                                                                      | <i>Cmmm</i> (65)                | <i>Cmm'm'</i> (65.486)                                  | <i>m'm'm'</i>   | ×        | ✓   |
| 0.375  | La <sub>2</sub> CoIrO <sub>6</sub>                                                       | <i>P2<sub>1</sub>/n</i> (14)    | <i>P2<sub>1</sub>/c</i> (14.75)                         | <i>2/m</i>      | ×        | ✓   |
| 0.376  | LaCaFeO <sub>4</sub>                                                                     | <i>Cmce</i> (64)                | <i>Cm'c'a</i> (64.474)                                  | <i>m'm'm</i>    | ×        | ✓   |
| 0.377  | Mn <sub>3</sub> Ge                                                                       | <i>P6<sub>3</sub>/mmc</i> (194) | <i>Cm'cm'</i> (63.464)                                  | <i>m'm'm</i>    | ×        | ✓   |
| 0.378  | UBi <sub>2</sub>                                                                         | <i>P4/nmm</i> (129)             | <i>P4/n'm'm'</i> (129.419)                              | <i>4/m'm'm'</i> | PT-wP    | ×   |
| 0.379  | SmFeO <sub>3</sub>                                                                       | <i>Pbnm</i> (62)                | <i>Pn'm'a</i> (62.446)                                  | <i>m'm'm</i>    | ×        | ✓   |
| 0.380  | SmFeO <sub>3</sub>                                                                       | <i>Pnma</i> (62)                | <i>Pn'ma'</i> (62.448)                                  | <i>m'm'm</i>    | ×        | ✓   |
| 0.381  | Co <sub>6</sub> (OH) <sub>3</sub> (TeO <sub>3</sub> ) <sub>4</sub>                       | <i>P6<sub>3</sub>/mc</i> (186)  | <i>P6<sub>3</sub>mc'</i> (186.206)                      | <i>6'mm'</i>    | BW-woP   | ×   |
| 0.382  | LiMnPO <sub>4</sub>                                                                      | <i>Pnma</i> (62)                | <i>Pn'm'a'</i> (62.449)                                 | <i>m'm'm'</i>   | PT-wP    | ×   |
| 0.383  | LiCoPO <sub>4</sub>                                                                      | <i>Pnma</i> (62)                | <i>Pnma'</i> (62.445)                                   | <i>m'mm</i>     | PT-wP    | ×   |
| 0.384  | LiCoPO <sub>4</sub>                                                                      | <i>Pnma</i> (62)                | <i>P2<sub>1</sub>/c</i> (14.77)                         | <i>2'/m</i>     | PT-wP    | ×   |
| 0.385  | LiCoPO <sub>4</sub>                                                                      | <i>Pnma</i> (62)                | <i>P2<sub>1</sub>/c'</i> (14.78)                        | <i>2'/m'</i>    | PT-wP    | ×   |
| 0.386  | Fe <sub>3</sub> BO <sub>5</sub>                                                          | <i>Pnma</i> (62)                | <i>Pnm'a</i> (62.444)                                   | <i>m'mm</i>     | PT-wP    | ×   |
| 0.387  | Fe <sub>3</sub> BO <sub>5</sub>                                                          | <i>Pnma</i> (62)                | <i>Pm'c2<sub>1</sub></i> (26.68)                        | <i>m'm2'</i>    | BW-wP    | ✓   |
| 0.388  | Co <sub>3</sub> Al <sub>2</sub> Si <sub>3</sub> O <sub>12</sub>                          | <i>Ia3d</i> (230)               | <i>I4<sub>1</sub>/a'cd</i> (142.563)                    | <i>4/m'mm</i>   | PT-wP    | ×   |
| 0.389  | Fe <sub>1.5</sub> Mn <sub>1.5</sub> BO <sub>5</sub>                                      | <i>Pbam</i> (55)                | <i>Pbam</i> (55.353)                                    | <i>mmm</i>      | ×        | ×   |
| 0.390  | Y <sub>2</sub> SrCu <sub>0.6</sub> Co <sub>1.4</sub> O <sub>6</sub>                      | <i>Ibam</i> (72)                | <i>Ib'a'm</i> (72.543)                                  | <i>m'm'm</i>    | ×        | ✓   |
| 0.391  | Y <sub>2</sub> SrCu <sub>0.6</sub> Co <sub>1.4</sub> O <sub>6</sub>                      | <i>Ibam</i> (72)                | <i>Ib'a'm</i> (72.543)                                  | <i>m'm'm</i>    | ×        | ✓   |
| 0.392  | Fe <sub>3</sub> (PO <sub>4</sub> ) <sub>2</sub> (OH) <sub>2</sub>                        | <i>P2<sub>1</sub>/c</i> (14)    | <i>P2<sub>1</sub>/c</i> (14.75)                         | <i>2/m</i>      | ×        | ✓   |
| 0.393  | Cu <sub>4</sub> (OH) <sub>6</sub> FBr                                                    | <i>P6<sub>3</sub>/m</i> (176)   | <i>P2<sub>1</sub>'/m'</i> (11.54)                       | <i>2'/m'</i>    | ×        | ✓   |
| 0.394  | Cu <sub>2</sub> CdB <sub>2</sub> O <sub>6</sub>                                          | <i>P2<sub>1</sub>/c</i> (14)    | <i>P2<sub>1</sub>/c'</i> (14.78)                        | <i>2'/m'</i>    | PT-wP    | ×   |
| 0.395  | MnPtGa                                                                                   | <i>P6<sub>3</sub>/mmc</i> (194) | <i>Cm'c'm</i> (63.462)                                  | <i>m'm'm</i>    | ×        | ✓   |
| 0.396  | MnPtGa                                                                                   | <i>P6<sub>3</sub>/mmc</i> (194) | <i>Cm'c'm</i> (63.462)                                  | <i>m'm'm</i>    | ×        | ✓   |
| 0.397  | Mn <sub>3</sub> Si <sub>2</sub> Te <sub>6</sub>                                          | <i>P31c</i> (163)               | <i>C2'/c'</i> (15.89)                                   | <i>2'/m'</i>    | ×        | ✓   |

Continued on next page

TABLE S7 – continued from previous page

| BCS-ID | Formula                                                                       | Parent                                   | MSG                                            | MPG             | SHG type | LMO |
|--------|-------------------------------------------------------------------------------|------------------------------------------|------------------------------------------------|-----------------|----------|-----|
| 0.398  | <a href="#">Ca<sub>2</sub>RuO<sub>4</sub></a>                                 | <i>Pbca</i> (61)                         | <i>Pbca</i> (61.433)                           | <i>mmm</i>      | ×        | ×   |
| 0.399  | <a href="#">FeOOH</a>                                                         | <i>Pbnm</i> (62)                         | <i>Pnma'</i> (62.445)                          | <i>m'mm</i>     | PT-wP    | ×   |
| 0.400  | <a href="#">Sr<sub>2</sub>Fe<sub>1.9</sub>Co<sub>0.1</sub>O<sub>5.5</sub></a> | <i>Cmmm</i> (65)                         | <i>Cm'm'm'</i> (65.487)                        | <i>m'm'm'</i>   | PT-wP    | ×   |
| 0.401  | <a href="#">Sr<sub>4</sub>Fe<sub>4</sub>O<sub>11</sub></a>                    | <i>Cmmm</i> (65)                         | <i>Cm'm'm'</i> (65.487)                        | <i>m'm'm'</i>   | PT-wP    | ×   |
| 0.402  | <a href="#">Sr<sub>4</sub>Fe<sub>4</sub>O<sub>11</sub></a>                    | <i>Cmmm</i> (65)                         | <i>Cmm'm'</i> (65.486)                         | <i>m'm'm</i>    | ×        | ✓   |
| 0.403  | <a href="#">NdCo<sub>2</sub></a>                                              | <i>Fd3m</i> (227)                        | <i>Imm'a'</i> (74.559)                         | <i>m'm'm</i>    | ×        | ✓   |
| 0.404  | <a href="#">Sr<sub>3</sub>NaRuO<sub>6</sub></a>                               | <i>R3c</i> (167)                         | <i>C2'/c'</i> (15.89)                          | <i>2'/m'</i>    | ×        | ✓   |
| 0.405  | <a href="#">CsCoF<sub>4</sub></a>                                             | <i>I4c2</i> (120)                        | <i>I4'</i> (82.41)                             | <i>4'</i>       | BW-woP   | ×   |
| 0.406  | <a href="#">GdNiSi<sub>3</sub></a>                                            | <i>Cmmm</i> (65)                         | <i>Cmmm'</i> (65.484)                          | <i>m'mm</i>     | PT-wP    | ×   |
| 0.407  | <a href="#">NdSi</a>                                                          | <i>Pnma</i> (62)                         | <i>Pn'm'a</i> (62.446)                         | <i>m'm'm</i>    | ×        | ✓   |
| 0.408  | <a href="#">PrSi</a>                                                          | <i>Pnma</i> (62)                         | <i>Pnm'a'</i> (62.447)                         | <i>m'm'm</i>    | ×        | ✓   |
| 0.409  | <a href="#">TmNi</a>                                                          | <i>Pnma</i> (62)                         | <i>Pn'm'a</i> (62.446)                         | <i>m'm'm</i>    | ×        | ✓   |
| 0.410  | <a href="#">GdAlO<sub>3</sub></a>                                             | <i>Pbnm</i> (62)                         | <i>Pn'm'a'</i> (62.449)                        | <i>m'm'm'</i>   | PT-wP    | ×   |
| 0.411  | <a href="#">Tb<sub>5</sub>Ge<sub>4</sub></a>                                  | <i>Pnma</i> (62)                         | <i>Pnm'a</i> (62.444)                          | <i>m'mm</i>     | PT-wP    | ×   |
| 0.412  | <a href="#">Tb<sub>5</sub>Ge<sub>4</sub></a>                                  | <i>Pnma</i> (62)                         | <i>Pnm'a</i> (62.444)                          | <i>m'mm</i>     | PT-wP    | ×   |
| 0.413  | <a href="#">UGeSe</a>                                                         | <i>I4/mmm</i> (139)                      | <i>I4/m'm'm'</i> (139.539)                     | <i>4/m'm'm'</i> | PT-wP    | ×   |
| 0.414  | <a href="#">AlFe<sub>2</sub>B<sub>2</sub></a>                                 | <i>Cmmm</i> (65)                         | <i>Cmm'm'</i> (65.486)                         | <i>m'm'm</i>    | ×        | ✓   |
| 0.415  | <a href="#">EuFe<sub>2</sub>P<sub>2</sub></a>                                 | <i>I4/mmm</i> (139)                      | <i>C2'/m'</i> (12.62)                          | <i>2'/m'</i>    | ×        | ✓   |
| 0.416  | <a href="#">LaCrO<sub>3</sub></a>                                             | <i>R3c</i> (167)                         | <i>R3c</i> (167.103)                           | <i>3m</i>       | ×        | ×   |
| 0.417  | <a href="#">LaCrO<sub>3</sub></a>                                             | <i>Pnma</i> (62)                         | <i>Pn'ma'</i> (62.448)                         | <i>m'm'm</i>    | ×        | ✓   |
| 0.418  | <a href="#">K<sub>0.8</sub>Fe<sub>1.8</sub>Se<sub>2</sub></a>                 | <i>I4/m</i> (87)                         | <i>I4/m'</i> (87.78)                           | <i>4/m'</i>     | PT-wP    | ×   |
| 0.419  | <a href="#">ErGe<sub>2</sub>O<sub>7</sub></a>                                 | <i>P4<sub>1</sub>2<sub>1</sub>2</i> (92) | <i>P4'<sub>1</sub>2<sub>1</sub>2'</i> (92.113) | <i>4'22'</i>    | BW-woP   | ×   |
| 0.420  | <a href="#">Sr<sub>2</sub>LuRuO<sub>6</sub></a>                               | <i>P2<sub>1</sub>/n</i> (14)             | <i>P2<sub>1</sub>/c</i> (14.75)                | <i>2/m</i>      | ×        | ✓   |
| 0.421  | <a href="#">EuMnSb<sub>2</sub></a>                                            | <i>Pnma</i> (62)                         | <i>Pn'm'a'</i> (62.449)                        | <i>m'm'm'</i>   | PT-wP    | ×   |
| 0.422  | <a href="#">EuMnSb<sub>2</sub></a>                                            | <i>Pnma</i> (62)                         | <i>P2<sub>1</sub>/m'</i> (11.53)               | <i>2/m'</i>     | PT-wP    | ×   |
| 0.423  | <a href="#">EuMnSb<sub>2</sub></a>                                            | <i>Pnma</i> (62)                         | <i>Pn'm'a'</i> (62.449)                        | <i>m'm'm'</i>   | PT-wP    | ×   |
| 0.424  | <a href="#">EuMnSb<sub>2</sub></a>                                            | <i>Pnma</i> (62)                         | <i>Pn'm'a'</i> (62.449)                        | <i>m'm'm'</i>   | PT-wP    | ×   |
| 0.425  | <a href="#">Na<sub>2</sub>CoP<sub>2</sub>O<sub>7</sub></a>                    | <i>Pna2<sub>1</sub></i> (33)             | <i>Pn'a2<sub>1</sub>'</i> (33.146)             | <i>m'm2'</i>    | BW-woP   | ✓   |
| 0.426  | <a href="#">EuMnBi<sub>2</sub></a>                                            | <i>I4/mmm</i> (139)                      | <i>I4'/m'm'm</i> (139.536)                     | <i>4'/m'm'm</i> | PT-wP    | ×   |
| 0.427  | <a href="#">Sm<sub>2</sub>Ti<sub>2</sub>O<sub>7</sub></a>                     | <i>Fd3m</i> (227)                        | <i>Fd3m'</i> (227.131)                         | <i>m3m'</i>     | ×        | ×   |
| 0.428  | <a href="#">BaMn<sub>2</sub>Si<sub>2</sub>O<sub>7</sub></a>                   | <i>C2/c</i> (15)                         | <i>C2/c</i> (15.85)                            | <i>2/m</i>      | ×        | ✓   |
| 0.429  | <a href="#">CaCr<sub>0.86</sub>Fe<sub>3.14</sub>As<sub>3</sub></a>            | <i>Pnma</i> (62)                         | <i>Pn'ma</i> (62.443)                          | <i>m'mm</i>     | PT-wP    | ×   |
| 0.430  | <a href="#">Yb<sub>3</sub>Pt<sub>4</sub></a>                                  | <i>R3</i> (148)                          | <i>R3'</i> (148.19)                            | <i>3'</i>       | PT-wP    | ×   |
| 0.431  | <a href="#">CuB<sub>2</sub>O<sub>4</sub></a>                                  | <i>I42d</i> (122)                        | <i>P1</i> (1.1)                                | <i>1</i>        | O-woP    | ✓   |
| 0.432  | <a href="#">KMnF<sub>3</sub></a>                                              | <i>Pnma</i> (62)                         | <i>Pn'ma'</i> (62.448)                         | <i>m'm'm</i>    | ×        | ✓   |
| 0.433  | <a href="#">KMnF<sub>3</sub></a>                                              | <i>I4/mcm</i> (140)                      | <i>I4/mcm</i> (140.541)                        | <i>4/mmm</i>    | ×        | ×   |
| 0.434  | <a href="#">K<sub>2</sub>ReI<sub>6</sub></a>                                  | <i>P2<sub>1</sub>/n</i> (14)             | <i>P2<sub>1</sub>/c</i> (14.75)                | <i>2/m</i>      | ×        | ✓   |
| 0.435  | <a href="#">Pb<sub>5</sub>Fe<sub>3</sub>TiO<sub>11</sub>Cl</a>                | <i>P4/mmm</i> (123)                      | <i>P<sub>B</sub>mma</i> (51.302)               | <i>mmm1'</i>    | ×        | ×   |
| 0.436  | <a href="#">TbNi<sub>4</sub>Si</a>                                            | <i>Cmmm</i> (65)                         | <i>Cmm'm'</i> (65.486)                         | <i>m'm'm</i>    | ×        | ✓   |
| 0.437  | <a href="#">Ho<sub>3</sub>NiGe<sub>2</sub></a>                                | <i>Pnma</i> (62)                         | <i>Pnm'a'</i> (62.447)                         | <i>m'm'm</i>    | ×        | ✓   |
| 0.438  | <a href="#">Pr<sub>3</sub>CoGe<sub>2</sub></a>                                | <i>Pnma</i> (62)                         | <i>Pnm'a'</i> (62.447)                         | <i>m'm'm</i>    | ×        | ✓   |
| 0.439  | <a href="#">Tb<sub>3</sub>NiGe<sub>2</sub></a>                                | <i>Pnma</i> (62)                         | <i>Pn'ma'</i> (62.448)                         | <i>m'm'm</i>    | ×        | ✓   |
| 0.440  | <a href="#">SrCuTe<sub>2</sub>O<sub>6</sub></a>                               | <i>P4<sub>1</sub>32</i> (213)            | <i>P4<sub>1</sub>32</i> (213.63)               | <i>432</i>      | ×        | ×   |
| 0.441  | <a href="#">Fe<sub>4</sub>Nb<sub>2</sub>O<sub>9</sub></a>                     | <i>P3c1</i> (165)                        | <i>C2'/c'</i> (15.88)                          | <i>2/m'</i>     | PT-wP    | ×   |
| 0.442  | <a href="#">Fe<sub>4</sub>Nb<sub>2</sub>O<sub>9</sub></a>                     | <i>C2/c</i> (15)                         | <i>C2'/c'</i> (15.88)                          | <i>2/m'</i>     | PT-wP    | ×   |
| 0.443  | <a href="#">Fe<sub>4</sub>Nb<sub>2</sub>O<sub>9</sub></a>                     | <i>P3c1</i> (165)                        | <i>C2'/c'</i> (15.88)                          | <i>2/m'</i>     | PT-wP    | ×   |
| 0.444  | <a href="#">YbCl<sub>3</sub></a>                                              | <i>C2/m</i> (12)                         | <i>C2'/m</i> (12.60)                           | <i>2'/m</i>     | PT-wP    | ×   |
| 0.445  | <a href="#">MnCoGe</a>                                                        | <i>Pnma</i> (62)                         | <i>Pn'm'a</i> (62.446)                         | <i>m'm'm</i>    | ×        | ✓   |
| 0.446  | <a href="#">MnCoGeB<sub>0.05</sub></a>                                        | <i>P6<sub>3</sub>/mmc</i> (194)          | <i>Cm'c'm</i> (63.462)                         | <i>m'm'm</i>    | ×        | ✓   |
| 0.447  | <a href="#">MnCoGeB<sub>0.05</sub></a>                                        | <i>P6<sub>3</sub>/mmc</i> (194)          | <i>P6<sub>3</sub>/mm'c'</i> (194.270)          | <i>6'/mm'm'</i> | ×        | ✓   |
| 0.448  | <a href="#">Ce<sub>4</sub>Ge<sub>3</sub></a>                                  | <i>I43d</i> (220)                        | <i>I42d</i> (122.333)                          | <i>42m</i>      | O-woP    | ×   |
| 0.449  | <a href="#">Tb<sub>2</sub>Pt</a>                                              | <i>Pnma</i> (62)                         | <i>P2<sub>1</sub>/m'</i> (11.54)               | <i>2'/m'</i>    | ×        | ✓   |
| 0.450  | <a href="#">Nd<sub>5</sub>Ge<sub>4</sub></a>                                  | <i>Pnma</i> (62)                         | <i>Pnm'a'</i> (62.447)                         | <i>m'm'm</i>    | ×        | ✓   |
| 0.451  | <a href="#">DyRuAsO</a>                                                       | <i>Pmmn</i> (59)                         | <i>Pm'mn</i> (59.407)                          | <i>m'mm</i>     | PT-wP    | ×   |
| 0.452  | <a href="#">TbRuAsO</a>                                                       | <i>P4/nmm</i> (129)                      | <i>Pm'mn</i> (59.407)                          | <i>m'mm</i>     | PT-wP    | ×   |
| 0.453  | <a href="#">DyCoSi<sub>2</sub></a>                                            | <i>Cmcm</i> (63)                         | <i>Cm'cm</i> (63.459)                          | <i>m'mm</i>     | PT-wP    | ×   |
| 0.454  | <a href="#">PrScSb</a>                                                        | <i>I4/mmm</i> (139)                      | <i>P14/mnc</i> (128.410)                       | <i>4'/mmm1'</i> | ×        | ×   |
| 0.455  | <a href="#">RbFeO<sub>2</sub></a>                                             | <i>Pbca</i> (61)                         | <i>Pb'c'a'</i> (61.437)                        | <i>m'm'm'</i>   | PT-wP    | ×   |

Continued on next page

TABLE S7 – continued from previous page

| BCS-ID | Formula                                                                  | Parent                          | MSG                                   | MPG             | SHG type | LMO |
|--------|--------------------------------------------------------------------------|---------------------------------|---------------------------------------|-----------------|----------|-----|
| 0.456  | RbFeO <sub>2</sub>                                                       | <i>Fd3m</i> (227)               | <i>I4'_1/a'm'd</i> (141.556)          | <i>4'/m'm'm</i> | PT-wP    | ×   |
| 0.457  | CsFeO <sub>2</sub>                                                       | <i>Pbca</i> (61)                | <i>Pb'c'a'</i> (61.437)               | <i>m'm'm'</i>   | PT-wP    | ×   |
| 0.458  | CsFeO <sub>2</sub>                                                       | <i>Fd3m</i> (227)               | <i>I4'_1/a'm'd</i> (141.556)          | <i>4'/m'm'm</i> | PT-wP    | ×   |
| 0.459  | KFeO <sub>2</sub>                                                        | <i>Pbca</i> (61)                | <i>Pb'ca</i> (61.435)                 | <i>m'mm</i>     | PT-wP    | ×   |
| 0.460  | KFeO <sub>2</sub>                                                        | <i>Pbca</i> (61)                | <i>Pb'ca</i> (61.435)                 | <i>m'mm</i>     | PT-wP    | ×   |
| 0.461  | CoRh <sub>2</sub> O <sub>4</sub>                                         | <i>Fd3m</i> (227)               | <i>I4'_1/a'm'd</i> (141.556)          | <i>4'/m'm'm</i> | PT-wP    | ×   |
| 0.462  | MnAl <sub>2</sub> O <sub>4</sub>                                         | <i>Fd3m</i> (227)               | <i>I4'_1/a'm'd</i> (141.556)          | <i>4'/m'm'm</i> | PT-wP    | ×   |
| 0.463  | Co <sub>3</sub> O <sub>4</sub>                                           | <i>Fd3m</i> (227)               | <i>I4'_1/a'm'd</i> (141.556)          | <i>4'/m'm'm</i> | PT-wP    | ×   |
| 0.464  | BaMn <sub>2</sub> P <sub>2</sub>                                         | <i>I4/mmm</i> (139)             | <i>I4'/m'm'm</i> (139.536)            | <i>4'/m'm'm</i> | PT-wP    | ×   |
| 0.465  | HoCr <sub>2</sub> Si <sub>2</sub>                                        | <i>I4/mmm</i> (139)             | <i>I4'/m'm'm</i> (139.536)            | <i>4'/m'm'm</i> | PT-wP    | ×   |
| 0.466  | ThCr <sub>2</sub> Si <sub>2</sub>                                        | <i>I4/mmm</i> (139)             | <i>Im'mm</i> (71.535)                 | <i>m'mm</i>     | PT-wP    | ×   |
| 0.467  | TbPO <sub>4</sub>                                                        | <i>I4_1/amd</i> (141)           | <i>I4'_1/a'm'd</i> (141.556)          | <i>4'/m'm'm</i> | PT-wP    | ×   |
| 0.468  | ErB <sub>4</sub>                                                         | <i>P4/mbm</i> (127)             | <i>Pb'am</i> (55.355)                 | <i>m'mm</i>     | PT-wP    | ×   |
| 0.469  | TbB <sub>4</sub>                                                         | <i>P4/mbm</i> (127)             | <i>Pb'a'm'</i> (55.359)               | <i>m'm'm'</i>   | PT-wP    | ×   |
| 0.470  | BaMn <sub>2</sub> Sb <sub>2</sub>                                        | <i>I4/mmm</i> (139)             | <i>I4'/m'm'm</i> (139.536)            | <i>4'/m'm'm</i> | PT-wP    | ×   |
| 0.471  | Ba <sub>2</sub> Mn <sub>3</sub> Sb <sub>2</sub> O <sub>2</sub>           | <i>I4/mmm</i> (139)             | <i>I4'/m'm'm</i> (139.536)            | <i>4'/m'm'm</i> | PT-wP    | ×   |
| 0.472  | LaMn <sub>2</sub> Si <sub>2</sub>                                        | <i>I4/mmm</i> (139)             | <i>I4'/m'm'm</i> (139.536)            | <i>4'/m'm'm</i> | PT-wP    | ×   |
| 0.473  | LaMn <sub>2</sub> Si <sub>2</sub>                                        | <i>I4/mmm</i> (139)             | <i>Im'm2'</i> (44.231)                | <i>m'm2'</i>    | BW-wP    | ✓   |
| 0.474  | EuMn <sub>2</sub> Ge <sub>2</sub>                                        | <i>I4/mmm</i> (139)             | <i>I4'/m'm'm</i> (139.536)            | <i>4'/m'm'm</i> | PT-wP    | ×   |
| 0.475  | Sr <sub>2</sub> TbIrO <sub>6</sub>                                       | <i>P2<sub>1</sub>/n</i> (14)    | <i>P2<sub>1</sub>/c</i> (14.75)       | <i>2'/m</i>     | ×        | ✓   |
| 0.476  | Cs <sub>2</sub> [FeCl <sub>5</sub> (H <sub>2</sub> O)]                   | <i>I2/c</i> (15)                | <i>C2'/c</i> (15.87)                  | <i>2'/m</i>     | PT-wP    | ×   |
| 0.477  | Mn <sub>4</sub> Ta <sub>2</sub> O <sub>9</sub>                           | <i>P3c1</i> (165)               | <i>P3'c'1</i> (165.94)                | <i>3'm'</i>     | PT-wP    | ×   |
| 0.478  | SmCrO <sub>3</sub>                                                       | <i>Pnma</i> (62)                | <i>Pnma</i> (62.441)                  | <i>mmm</i>      | ×        | ×   |
| 0.479  | SmCrO <sub>3</sub>                                                       | <i>Pnma</i> (62)                | <i>Pn'm</i> (62.448)                  | <i>m'm'm</i>    | ×        | ✓   |
| 0.480  | HoNi                                                                     | <i>Pnma</i> (62)                | <i>Pnm'a'</i> (62.447)                | <i>m'm'm</i>    | ×        | ✓   |
| 0.481  | HoNi                                                                     | <i>Pnma</i> (62)                | <i>P2<sub>1</sub>/c'</i> (14.79)      | <i>2'/m'</i>    | ×        | ✓   |
| 0.482  | SrMn <sub>2</sub> As <sub>2</sub>                                        | <i>P3m1</i> (164)               | <i>C2'/m</i> (12.60)                  | <i>2'/m</i>     | PT-wP    | ×   |
| 0.483  | YbMn <sub>2</sub> Sb <sub>2</sub>                                        | <i>P3m1</i> (164)               | <i>P1'</i> (2.6)                      | <i>1'</i>       | PT-wP    | ×   |
| 0.484  | U <sub>2</sub> N <sub>2</sub> S                                          | <i>P3m1</i> (164)               | <i>P3'm'1</i> (164.88)                | <i>3'm'</i>     | PT-wP    | ×   |
| 0.485  | U <sub>2</sub> N <sub>2</sub> Se                                         | <i>P3m1</i> (164)               | <i>P3'm'1</i> (164.88)                | <i>3'm'</i>     | PT-wP    | ×   |
| 0.486  | ErCr <sub>2</sub> Si <sub>2</sub>                                        | <i>I4/mmm</i> (139)             | <i>I4'/m'm'm</i> (139.536)            | <i>4'/m'm'm</i> | PT-wP    | ×   |
| 0.487  | ErCr <sub>2</sub> Si <sub>2</sub>                                        | <i>I4/mmm</i> (139)             | <i>Im'm'2</i> (44.232)                | <i>m'm'2</i>    | BW-wP    | ✓   |
| 0.488  | YbMnO <sub>3</sub>                                                       | <i>P6<sub>3</sub>cm</i> (185)   | <i>P6<sub>3</sub>c'm</i> (185.199)    | <i>6'mm'</i>    | BW-woP   | ×   |
| 0.489  | YbMnO <sub>3</sub>                                                       | <i>P6<sub>3</sub>cm</i> (185)   | <i>P6<sub>3</sub>c'm</i> (185.199)    | <i>6'mm'</i>    | BW-woP   | ×   |
| 0.490  | YbMnO <sub>3</sub>                                                       | <i>P6<sub>3</sub>cm</i> (185)   | <i>P6<sub>3</sub>c'm'</i> (185.201)   | <i>6m'm'</i>    | BW-woP   | ✓   |
| 0.491  | NdB <sub>4</sub>                                                         | <i>P4/mbm</i> (127)             | <i>P4/m'</i> (83.46)                  | <i>4/m'</i>     | PT-wP    | ×   |
| 0.492  | NdB <sub>4</sub>                                                         | <i>P4/mbm</i> (127)             | <i>P2<sub>1</sub>/c</i> (14.77)       | <i>2'/m</i>     | PT-wP    | ×   |
| 0.493  | Ho(Co <sub>0.667</sub> Ga <sub>0.333</sub> ) <sub>2</sub>                | <i>P6<sub>3</sub>/mmc</i> (194) | <i>C2'/c'</i> (15.89)                 | <i>2'/m'</i>    | ×        | ✓   |
| 0.494  | Er(Co <sub>0.667</sub> Ga <sub>0.333</sub> ) <sub>2</sub>                | <i>P6<sub>3</sub>/mmc</i> (194) | <i>P6<sub>3</sub>/mm'c'</i> (194.270) | <i>6/mm'm'</i>  | ×        | ✓   |
| 0.495  | LaMn <sub>2</sub> Si <sub>2</sub>                                        | <i>I4/mmm</i> (139)             | <i>Im'm2'</i> (44.231)                | <i>m'm2'</i>    | BW-wP    | ✓   |
| 0.496  | LaMn <sub>2</sub> Si <sub>2</sub>                                        | <i>I4/mmm</i> (139)             | <i>Im'm2'</i> (44.231)                | <i>m'm2'</i>    | BW-wP    | ✓   |
| 0.497  | LaMn <sub>2</sub> Si <sub>2</sub>                                        | <i>I4/mmm</i> (139)             | <i>Im'm2'</i> (44.231)                | <i>m'm2'</i>    | BW-wP    | ✓   |
| 0.498  | LaMn <sub>2</sub> Si <sub>2</sub>                                        | <i>I4/mmm</i> (139)             | <i>I4'/m'm'm</i> (139.536)            | <i>4'/m'm'm</i> | PT-wP    | ×   |
| 0.499  | UCr <sub>2</sub> Si <sub>2</sub> C                                       | <i>P4/mmm</i> (123)             | <i>Pm'm'm</i> (47.252)                | <i>m'm'm</i>    | ×        | ✓   |
| 0.500  | Ca <sub>2</sub> FeMn <sub>0.5</sub> W <sub>0.5</sub> O <sub>8</sub>      | <i>P2<sub>1</sub>/n</i> (14)    | <i>P2<sub>1</sub>/c'</i> (14.79)      | <i>2'/m'</i>    | ×        | ✓   |
| 0.501  | LiFe <sub>2</sub> F <sub>6</sub>                                         | <i>P4<sub>2</sub>/mnm</i> (136) | <i>P4<sub>2</sub>/mnm'</i> (136.499)  | <i>4'/mm'm</i>  | ×        | ×   |
| 0.502  | La <sub>2</sub> Ni <sub>1.19</sub> Os <sub>0.81</sub> O <sub>6</sub>     | <i>P2<sub>1</sub>/c</i> (14)    | <i>P2<sub>1</sub>/c'</i> (14.79)      | <i>2'/m'</i>    | ×        | ✓   |
| 0.503  | K <sub>1.62</sub> Fe <sub>4</sub> O <sub>6.62</sub> (OH) <sub>0.98</sub> | <i>P31c</i> (163)               | <i>P31c</i> (163.79)                  | <i>3m</i>       | ×        | ×   |
| 0.504  | NaCrSi <sub>2</sub> O <sub>6</sub>                                       | <i>C2/c</i> (15)                | <i>P1'</i> (2.6)                      | <i>1'</i>       | PT-wP    | ×   |
| 0.505  | Pb <sub>2</sub> VO(PO <sub>4</sub> ) <sub>2</sub>                        | <i>P2<sub>1</sub>/a</i> (14)    | <i>P2<sub>1</sub>/c'</i> (14.78)      | <i>2'/m'</i>    | PT-wP    | ×   |
| 0.506  | Cs <sub>2</sub> Cu <sub>3</sub> SnF <sub>12</sub>                        | <i>P2<sub>1</sub>/n</i> (14)    | <i>P2<sub>1</sub>/c'</i> (14.79)      | <i>2'/m'</i>    | ×        | ✓   |
| 0.507  | Mn <sub>4</sub> Nb <sub>2</sub> O <sub>9</sub>                           | <i>P3c1</i> (165)               | <i>P3'c'1</i> (165.94)                | <i>3'm'</i>     | PT-wP    | ×   |
| 0.508  | FeMnO <sub>3</sub>                                                       | <i>Ia3</i> (206)                | <i>Ib'c'a</i> (73.551)                | <i>m'm'm</i>    | ×        | ✓   |
| 0.509  | BaFe <sub>12</sub> O <sub>19</sub>                                       | <i>P6<sub>3</sub>/mmc</i> (194) | <i>P6<sub>3</sub>/mm'c'</i> (194.270) | <i>6/mm'm'</i>  | ×        | ✓   |
| 0.510  | Mn <sub>2</sub> NiReO <sub>6</sub>                                       | <i>P2<sub>1</sub>/n</i> (14)    | <i>P2<sub>1</sub>/c</i> (14.75)       | <i>2'/m</i>     | ×        | ✓   |
| 0.511  | Co <sub>4</sub> Ta <sub>2</sub> O <sub>9</sub>                           | <i>P3c1</i> (165)               | <i>C2'/c</i> (15.87)                  | <i>2'/m</i>     | PT-wP    | ×   |
| 0.512  | Mn <sub>3</sub> As <sub>2</sub>                                          | <i>C2/m</i> (12)                | <i>C2'/m</i> (12.58)                  | <i>2'/m</i>     | ×        | ✓   |

Continued on next page

TABLE S7 – continued from previous page

| BCS-ID | Formula                                                                     | Parent                          | MSG                                             | MPG             | SHG type | LMO |
|--------|-----------------------------------------------------------------------------|---------------------------------|-------------------------------------------------|-----------------|----------|-----|
| 0.513  | <a href="#">YRuO<sub>3</sub></a>                                            | <i>Pnma</i> (62)                | <i>Pn'ma'</i> (62.448)                          | <i>m'm'm</i>    | ×        | ✓   |
| 0.514  | <a href="#">CoFe<sub>3</sub>O<sub>5</sub></a>                               | <i>Cmcm</i> (63)                | <i>Cm'cm'</i> (63.464)                          | <i>m'm'm</i>    | ×        | ✓   |
| 0.515  | <a href="#">CoFe<sub>3</sub>O<sub>5</sub></a>                               | <i>Cmcm</i> (63)                | <i>P2<sub>1</sub>'/m'</i> (11.54)               | <i>2'/m'</i>    | ×        | ✓   |
| 0.516  | <a href="#">BaMg<sub>2</sub>Fe<sub>16</sub>O<sub>27</sub></a>               | <i>P6<sub>3</sub>/mmc</i> (194) | <i>P6<sub>3</sub>/mm'c'</i> (194.270)           | <i>6'/mm'm'</i> | ×        | ✓   |
| 0.517  | <a href="#">BaCo<sub>2</sub>Fe<sub>16</sub>O<sub>27</sub></a>               | <i>P6<sub>3</sub>/mmc</i> (194) | <i>P6<sub>3</sub>/mm'c'</i> (194.270)           | <i>6'/mm'm'</i> | ×        | ✓   |
| 0.518  | <a href="#">TbCr<sub>2</sub>Si<sub>2</sub></a>                              | <i>I4/mmm</i> (139)             | <i>I4'/m'm'm</i> (139.536)                      | <i>4'/m'm'm</i> | PT-wP    | ×   |
| 0.519  | <a href="#">HoCr<sub>2</sub>Si<sub>2</sub></a>                              | <i>I4/mmm</i> (139)             | <i>I4'/m'm'm</i> (139.536)                      | <i>4'/m'm'm</i> | PT-wP    | ×   |
| 0.520  | <a href="#">TbCoO<sub>3</sub></a>                                           | <i>Pbnm</i> (62)                | <i>Pnm'a</i> (62.444)                           | <i>m'mm</i>     | PT-wP    | ×   |
| 0.521  | <a href="#">DyCoO<sub>3</sub></a>                                           | <i>Pbnm</i> (62)                | <i>Pn'm'a'</i> (62.449)                         | <i>m'm'm'</i>   | PT-wP    | ×   |
| 0.522  | <a href="#">La<sub>2</sub>O<sub>3</sub>FeMnSe<sub>2</sub></a>               | <i>I4/mmm</i> (139)             | <i>Im'm'm</i> (71.536)                          | <i>m'm'm</i>    | ×        | ✓   |
| 0.523  | <a href="#">CaMn<sub>2</sub>Sb<sub>2</sub></a>                              | <i>P3m1</i> (164)               | <i>P1'</i> (2.6)                                | <i>1'</i>       | PT-wP    | ×   |
| 0.524  | <a href="#">MnPS<sub>3</sub></a>                                            | <i>R3</i> (148)                 | <i>P1'</i> (2.6)                                | <i>1'</i>       | PT-wP    | ×   |
| 0.525  | <a href="#">NaCeO<sub>2</sub></a>                                           | <i>I41/amd</i> (141)            | <i>I4<sub>1</sub>'/a'm'd</i> (141.556)          | <i>4'/m'm'm</i> | PT-wP    | ×   |
| 0.526  | <a href="#">Mn<sub>4</sub>Ta<sub>2</sub>O<sub>9</sub></a>                   | <i>P3c1</i> (165)               | <i>P3'c'1</i> (165.94)                          | <i>3'm'</i>     | PT-wP    | ×   |
| 0.527  | <a href="#">Er<sub>2</sub>Si<sub>2</sub>O<sub>7</sub></a>                   | <i>C2/m</i> (12)                | <i>C2'/m</i> (12.60)                            | <i>2'/m</i>     | PT-wP    | ×   |
| 0.528  | <a href="#">CrSb</a>                                                        | <i>P6<sub>3</sub>/mmc</i> (194) | <i>P6<sub>3</sub>/m'm'c</i> (194.268)           | <i>6'/m'mm'</i> | ×        | ×   |
| 0.529  | <a href="#">Co<sub>4</sub>Nb<sub>2</sub>O<sub>9</sub></a>                   | <i>P3c1</i> (165)               | <i>C2'/c'</i> (15.88)                           | <i>2'/m'</i>    | PT-wP    | ×   |
| 0.530  | <a href="#">SrCuTe<sub>2</sub>O<sub>6</sub></a>                             | <i>P4<sub>1</sub>32</i> (213)   | <i>P4<sub>1</sub>32</i> (213.63)                | 432             | ×        | ×   |
| 0.531  | <a href="#">Sr<sub>0.7</sub>Tb<sub>0.3</sub>CoO<sub>2.9</sub></a>           | <i>I4/mmm</i> (139)             | <i>I4'/mmm'</i> (139.535)                       | <i>4'/mm'm</i>  | ×        | ×   |
| 0.532  | <a href="#">Sr<sub>0.7</sub>Ho<sub>0.3</sub>CoO<sub>2.7</sub></a>           | <i>I4/mmm</i> (139)             | <i>I4'/mmm'</i> (139.535)                       | <i>4'/mm'm</i>  | ×        | ×   |
| 0.533  | <a href="#">Sr<sub>0.7</sub>Er<sub>0.3</sub>CoO<sub>2.8</sub></a>           | <i>I4/mmm</i> (139)             | <i>I4'/mmm'</i> (139.535)                       | <i>4'/mm'm</i>  | ×        | ×   |
| 0.534  | <a href="#">Tb<sub>0.55</sub>Sr<sub>0.45</sub>MnO<sub>3</sub></a>           | <i>Pnma</i> (62)                | <i>Pnm'a'</i> (62.447)                          | <i>m'm'm</i>    | ×        | ✓   |
| 0.535  | <a href="#">Tb<sub>0.55</sub>Sr<sub>0.45</sub>MnO<sub>3</sub></a>           | <i>Pnma</i> (62)                | <i>Pnm'a'</i> (62.447)                          | <i>m'm'm</i>    | ×        | ✓   |
| 0.536  | <a href="#">Tb<sub>0.55</sub>Sr<sub>0.45</sub>MnO<sub>3</sub></a>           | <i>Pnma</i> (62)                | <i>Pnm'a'</i> (62.447)                          | <i>m'm'm</i>    | ×        | ✓   |
| 0.537  | <a href="#">CaMn<sub>0.7</sub>Co<sub>1.3</sub>ReO<sub>6</sub></a>           | <i>P4<sub>2</sub>/n</i> (86)    | <i>P4<sub>2</sub>/n</i> (86.67)                 | <i>4/m</i>      | ×        | ✓   |
| 0.538  | <a href="#">CaMn<sub>1.2</sub>Ni<sub>0.8</sub>ReO<sub>6</sub></a>           | <i>P4<sub>2</sub>/n</i> (86)    | <i>P4<sub>2</sub>/n</i> (86.67)                 | <i>4/m</i>      | ×        | ✓   |
| 0.539  | <a href="#">Mn<sub>2</sub>Fe<sub>0.8</sub>Mo<sub>1.2</sub>O<sub>6</sub></a> | <i>P2<sub>1</sub>/n</i> (14)    | <i>P2<sub>1</sub>/c</i> (14.75)                 | <i>2/m</i>      | ×        | ✓   |
| 0.540  | <a href="#">Mn<sub>2</sub>Fe<sub>0.8</sub>Mo<sub>1.2</sub>O<sub>6</sub></a> | <i>P2<sub>1</sub>/n</i> (14)    | <i>P2<sub>1</sub>/c</i> (14.75)                 | <i>2/m</i>      | ×        | ✓   |
| 0.541  | <a href="#">Mn<sub>2</sub>FeReO<sub>6</sub></a>                             | <i>P2<sub>1</sub>/c</i> (14)    | <i>P2<sub>1</sub>'/c'</i> (14.79)               | <i>2'/m'</i>    | ×        | ✓   |
| 0.542  | <a href="#">Mn<sub>2</sub>FeReO<sub>6</sub></a>                             | <i>P2<sub>1</sub>/c</i> (14)    | <i>P1</i> (2.4)                                 | <i>1</i>        | ×        | ✓   |
| 0.543  | <a href="#">Mn<sub>2</sub>FeReO<sub>6</sub></a>                             | <i>P2<sub>1</sub>/c</i> (14)    | <i>P1</i> (2.4)                                 | <i>1</i>        | ×        | ✓   |
| 0.544  | <a href="#">Mn<sub>2</sub>FeReO<sub>6</sub></a>                             | <i>P2<sub>1</sub>/c</i> (14)    | <i>P1</i> (2.4)                                 | <i>1</i>        | ×        | ✓   |
| 0.545  | <a href="#">Mn<sub>2</sub>FeReO<sub>6</sub></a>                             | <i>P2<sub>1</sub>/c</i> (14)    | <i>P1</i> (2.4)                                 | <i>1</i>        | ×        | ✓   |
| 0.546  | <a href="#">Mn<sub>2</sub>FeReO<sub>6</sub></a>                             | <i>P2<sub>1</sub>/c</i> (14)    | <i>P2<sub>1</sub>'/c'</i> (14.79)               | <i>2'/m'</i>    | ×        | ✓   |
| 0.547  | <a href="#">Mn<sub>2</sub>FeReO<sub>6</sub></a>                             | <i>P2<sub>1</sub>/c</i> (14)    | <i>P2<sub>1</sub>'/c'</i> (14.79)               | <i>2'/m'</i>    | ×        | ✓   |
| 0.548  | <a href="#">Mn<sub>2</sub>FeReO<sub>6</sub></a>                             | <i>P2<sub>1</sub>/c</i> (14)    | <i>P1</i> (2.4)                                 | <i>1</i>        | ×        | ✓   |
| 0.549  | <a href="#">Mn<sub>2</sub>FeReO<sub>6</sub></a>                             | <i>P2<sub>1</sub>/c</i> (14)    | <i>P1</i> (2.4)                                 | <i>1</i>        | ×        | ✓   |
| 0.550  | <a href="#">Mn<sub>3</sub>ReO<sub>6</sub></a>                               | <i>P2<sub>1</sub>/c</i> (14)    | <i>P<sub>S</sub>1</i> (2.7)                     | <i>11'</i>      | ×        | ×   |
| 0.551  | <a href="#">Mn<sub>3</sub>ReO<sub>6</sub></a>                               | <i>P2<sub>1</sub>/c</i> (14)    | <i>P<sub>S</sub>1</i> (2.7)                     | <i>11'</i>      | ×        | ×   |
| 0.552  | <a href="#">Pb<sub>2</sub>MnO<sub>4</sub></a>                               | <i>P4<sub>2</sub>1c</i> (114)   | <i>P4<sub>2</sub>'2<sub>1</sub>c'</i> (114.278) | <i>4'2m'</i>    | BW-woP   | ×   |
| 0.553  | <a href="#">K<sub>2</sub>ReI<sub>6</sub></a>                                | <i>P2<sub>1</sub>/n</i> (14)    | <i>P2<sub>1</sub>/c</i> (14.75)                 | <i>2/m</i>      | ×        | ✓   |
| 0.554  | <a href="#">Co<sub>2</sub>MnSi</a>                                          | <i>Fm3m</i> (225)               | <i>I4/mmm'm'</i> (139.537)                      | <i>4'/mm'm'</i> | ×        | ✓   |
| 0.555  | <a href="#">Ho<sub>0.05</sub>Bi<sub>0.95</sub>FeO<sub>3</sub></a>           | <i>R3c</i> (161)                | <i>R3c</i> (161.69)                             | <i>3m</i>       | O-woP    | ×   |
| 0.556  | <a href="#">Ho<sub>0.1</sub>Bi<sub>0.9</sub>FeO<sub>3</sub></a>             | <i>R3c</i> (161)                | <i>R3c</i> (161.69)                             | <i>3m</i>       | O-woP    | ×   |
| 0.557  | <a href="#">Ho<sub>0.15</sub>Bi<sub>0.85</sub>FeO<sub>3</sub></a>           | <i>R3c</i> (161)                | <i>Cc</i> (9.37)                                | <i>m</i>        | O-woP    | ✓   |
| 0.558  | <a href="#">Ho<sub>0.2</sub>Bi<sub>0.8</sub>FeO<sub>3</sub></a>             | <i>R3c</i> (161)                | <i>Cc</i> (9.37)                                | <i>m</i>        | O-woP    | ✓   |
| 0.559  | <a href="#">Ho<sub>0.15</sub>Bi<sub>0.85</sub>FeO<sub>3</sub></a>           | <i>Pnma</i> (62)                | <i>Pn'ma'</i> (62.448)                          | <i>m'm'm</i>    | ×        | ✓   |
| 0.560  | <a href="#">Ho<sub>0.2</sub>Bi<sub>0.8</sub>FeO<sub>3</sub></a>             | <i>Pnma</i> (62)                | <i>Pn'ma'</i> (62.448)                          | <i>m'm'm</i>    | ×        | ✓   |
| 0.561  | <a href="#">NdNiGe<sub>2</sub></a>                                          | <i>Cmcm</i> (63)                | <i>Cm'c'm</i> (63.462)                          | <i>m'm'm</i>    | ×        | ✓   |
| 0.562  | <a href="#">Ce<sub>2</sub>Ni<sub>3</sub>Ge<sub>5</sub></a>                  | <i>Ibam</i> (72)                | <i>P<sub>1</sub>bcn</i> (60.432)                | <i>mmm1'</i>    | ×        | ×   |
| 0.563  | <a href="#">Ce<sub>2</sub>Ni<sub>3</sub>Ge<sub>5</sub></a>                  | <i>Ibam</i> (72)                | <i>P<sub>1</sub>ccn</i> (56.376)                | <i>mmm1'</i>    | ×        | ×   |
| 0.564  | <a href="#">U<sub>2</sub>Rh<sub>3</sub>Si<sub>5</sub></a>                   | <i>I2/c</i> (15)                | <i>P<sub>C</sub>2/c</i> (13.74)                 | <i>2/m1'</i>    | ×        | ×   |
| 0.565  | <a href="#">Ce<sub>2</sub>Ni<sub>3</sub>Ge<sub>5</sub></a>                  | <i>Ibam</i> (72)                | <i>P<sub>1</sub>bcn</i> (60.432)                | <i>mmm1'</i>    | ×        | ×   |
| 0.566  | <a href="#">TbNiGe<sub>2</sub></a>                                          | <i>Cmcm</i> (63)                | <i>Cm'cm</i> (63.459)                           | <i>m'mm</i>     | PT-wP    | ×   |
| 0.567  | <a href="#">HoNi<sub>0.64</sub>Ge<sub>2</sub></a>                           | <i>Cmcm</i> (63)                | <i>Cm'cm</i> (63.459)                           | <i>m'mm</i>     | PT-wP    | ×   |
| 0.568  | <a href="#">TbNi<sub>0.4</sub>Ge<sub>2</sub></a>                            | <i>Cmcm</i> (63)                | <i>Cm'cm</i> (63.459)                           | <i>m'mm</i>     | PT-wP    | ×   |
| 0.569  | <a href="#">TbCu<sub>0.4</sub>Ge<sub>2</sub></a>                            | <i>Cmcm</i> (63)                | <i>Cm'cm</i> (63.459)                           | <i>m'mm</i>     | PT-wP    | ×   |

Continued on next page

TABLE S7 – continued from previous page

| BCS-ID | Formula                                                                 | Parent                          | MSG                                   | MPG             | SHG type | LMO |
|--------|-------------------------------------------------------------------------|---------------------------------|---------------------------------------|-----------------|----------|-----|
| 0.570  | <a href="#">Li<sub>0.5</sub>FeCr<sub>1.5</sub>O<sub>4</sub></a>         | <i>Fd3m</i> (227)               | <i>I4<sub>1</sub>/am'd'</i> (141.557) | <i>4/mm'm'</i>  | ×        | ✓   |
| 0.571  | <a href="#">CoSO<sub>4</sub></a>                                        | <i>Pbnm</i> (62)                | <i>Pnma</i> (62.441)                  | <i>mmm</i>      | ×        | ×   |
| 0.572  | <a href="#">Na<sub>2</sub>NiCrF<sub>7</sub></a>                         | <i>Imma</i> (74)                | <i>Im'm'a</i> (74.558)                | <i>m'm'm</i>    | ×        | ✓   |
| 0.573  | <a href="#">Na<sub>2</sub>NiCrF<sub>7</sub></a>                         | <i>Imma</i> (74)                | <i>Im'm'a</i> (74.558)                | <i>m'm'm</i>    | ×        | ✓   |
| 0.574  | <a href="#">MnFeF<sub>5</sub>(H<sub>2</sub>O)<sub>2</sub></a>           | <i>Imm2</i> (44)                | <i>C2'</i> (5.15)                     | <i>2'</i>       | BW-woP   | ✓   |
| 0.575  | <a href="#">ZnFeF<sub>5</sub>(H<sub>2</sub>O)<sub>2</sub></a>           | <i>Imm2</i> (44)                | <i>Imm2</i> (44.229)                  | <i>mm2</i>      | O-woP    | ×   |
| 0.576  | <a href="#">Cr<sub>2</sub>F<sub>5</sub></a>                             | <i>C2/c</i> (15)                | <i>C2/c</i> (15.85)                   | <i>2/m</i>      | ×        | ✓   |
| 0.577  | <a href="#">BaMnFeF<sub>7</sub></a>                                     | <i>P2<sub>1</sub>/c</i> (14)    | <i>P2<sub>1</sub>'/c'</i> (14.79)     | <i>2'/m'</i>    | ×        | ✓   |
| 0.578  | <a href="#">NaBaFe<sub>2</sub>F<sub>9</sub></a>                         | <i>P2<sub>1</sub>/c</i> (14)    | <i>P2<sub>1</sub>'/c</i> (14.75)      | <i>2/m</i>      | ×        | ✓   |
| 0.579  | <a href="#">Na<sub>2</sub>NiFeF<sub>7</sub></a>                         | <i>Imma</i> (74)                | <i>Imm'a'</i> (74.559)                | <i>m'm'm</i>    | ×        | ✓   |
| 0.580  | <a href="#">Na<sub>2</sub>NiFeF<sub>7</sub></a>                         | <i>Imma</i> (74)                | <i>Imm'a'</i> (74.559)                | <i>m'm'm</i>    | ×        | ✓   |
| 0.581  | <a href="#">FeF<sub>3</sub></a>                                         | <i>R3c</i> (167)                | <i>C2'/c'</i> (15.89)                 | <i>2'/m'</i>    | ×        | ✓   |
| 0.582  | <a href="#">Fe<sub>3</sub>F<sub>8</sub>(H<sub>2</sub>O)<sub>2</sub></a> | <i>C2/m</i> (12)                | <i>C2'/m'</i> (12.62)                 | <i>2'/m'</i>    | ×        | ✓   |
| 0.583  | <a href="#">Fe<sub>2</sub>F<sub>5</sub>(H<sub>2</sub>O)<sub>2</sub></a> | <i>Imma</i> (74)                | <i>Imm'a'</i> (74.559)                | <i>m'm'm</i>    | ×        | ✓   |
| 0.584  | <a href="#">Fe<sub>2</sub>F<sub>5</sub>(H<sub>2</sub>O)<sub>2</sub></a> | <i>Imma</i> (74)                | <i>C2'/c'</i> (15.89)                 | <i>2'/m'</i>    | ×        | ✓   |
| 0.585  | <a href="#">YbCl<sub>3</sub></a>                                        | <i>C2/m</i> (12)                | <i>C2'/m</i> (12.60)                  | <i>2'/m</i>     | PT-wP    | ×   |
| 0.586  | <a href="#">YCrO<sub>3</sub></a>                                        | <i>Pbnm</i> (62)                | <i>Pn'ma'</i> (62.448)                | <i>m'm'm</i>    | ×        | ✓   |
| 0.587  | <a href="#">TmCrO<sub>3</sub></a>                                       | <i>Pbnm</i> (62)                | <i>Pn'ma'</i> (62.448)                | <i>m'm'm</i>    | ×        | ✓   |
| 0.588  | <a href="#">PrCrO<sub>3</sub></a>                                       | <i>Pbnm</i> (62)                | <i>Pn'ma'</i> (62.448)                | <i>m'm'm</i>    | ×        | ✓   |
| 0.589  | <a href="#">NdCrO<sub>3</sub></a>                                       | <i>Pbnm</i> (62)                | <i>P2<sub>1</sub>/m</i> (11.50)       | <i>2/m</i>      | ×        | ✓   |
| 0.590  | <a href="#">ErCrO<sub>3</sub></a>                                       | <i>Pbnm</i> (62)                | <i>P2<sub>1</sub>/m</i> (11.50)       | <i>2/m</i>      | ×        | ✓   |
| 0.591  | <a href="#">ErCrO<sub>3</sub></a>                                       | <i>Pbnm</i> (62)                | <i>Pn'ma'</i> (62.448)                | <i>m'm'm</i>    | ×        | ✓   |
| 0.592  | <a href="#">DyCrO<sub>3</sub></a>                                       | <i>Pbnm</i> (62)                | <i>Pn'm'a</i> (62.446)                | <i>m'm'm</i>    | ×        | ✓   |
| 0.593  | <a href="#">UPSe</a>                                                    | <i>P4/nmm</i> (129)             | <i>P4/nm'm'</i> (129.417)             | <i>4/mm'm'</i>  | ×        | ✓   |
| 0.594  | <a href="#">UAsS</a>                                                    | <i>P4/nmm</i> (129)             | <i>P4/nm'm'</i> (129.417)             | <i>4/mm'm'</i>  | ×        | ✓   |
| 0.595  | <a href="#">UPTe</a>                                                    | <i>I4/mmm</i> (139)             | <i>I4/mmm'm'</i> (139.537)            | <i>4/mm'm'</i>  | ×        | ✓   |
| 0.596  | <a href="#">UAsTe</a>                                                   | <i>I4/mmm</i> (139)             | <i>I4/mmm'm'</i> (139.537)            | <i>4/mm'm'</i>  | ×        | ✓   |
| 0.597  | <a href="#">MnBi<sub>8</sub>Te<sub>13</sub></a>                         | <i>R3m</i> (166)                | <i>R3m'</i> (166.101)                 | <i>3m'</i>      | ×        | ✓   |
| 0.598  | <a href="#">AlCr<sub>2</sub></a>                                        | <i>I4/mmm</i> (139)             | <i>PA2<sub>1</sub>/c</i> (14.83)      | <i>2/m1'</i>    | ×        | ×   |
| 0.599  | <a href="#">CaMnSi</a>                                                  | <i>P4/nmm</i> (129)             | <i>P4'/n'm'm</i> (129.416)            | <i>4'/m'm'm</i> | PT-wP    | ×   |
| 0.600  | <a href="#">CaMnSi</a>                                                  | <i>P4/nmm</i> (129)             | <i>P4'/n'm'm</i> (129.416)            | <i>4'/m'm'm</i> | PT-wP    | ×   |
| 0.601  | <a href="#">CaMnGe</a>                                                  | <i>P4/nmm</i> (129)             | <i>P2<sub>1</sub>/m'</i> (11.53)      | <i>2/m'</i>     | PT-wP    | ×   |
| 0.602  | <a href="#">CaMnGe</a>                                                  | <i>P4/nmm</i> (129)             | <i>P2<sub>1</sub>/m'</i> (11.53)      | <i>2/m'</i>     | PT-wP    | ×   |
| 0.603  | <a href="#">CaMn<sub>2</sub>Ge<sub>2</sub></a>                          | <i>I4/mmm</i> (139)             | <i>I4'/m'm'm</i> (139.536)            | <i>4'/m'm'm</i> | PT-wP    | ×   |
| 0.604  | <a href="#">CaMn<sub>2</sub>Ge<sub>2</sub></a>                          | <i>I4/mmm</i> (139)             | <i>I4'/m'm'm</i> (139.536)            | <i>4'/m'm'm</i> | PT-wP    | ×   |
| 0.605  | <a href="#">BaMn<sub>2</sub>Ge<sub>2</sub></a>                          | <i>I4/mmm</i> (139)             | <i>I4'/m'm'm</i> (139.536)            | <i>4'/m'm'm</i> | PT-wP    | ×   |
| 0.606  | <a href="#">BaMn<sub>2</sub>Ge<sub>2</sub></a>                          | <i>I4/mmm</i> (139)             | <i>I4'/m'm'm</i> (139.536)            | <i>4'/m'm'm</i> | PT-wP    | ×   |
| 0.607  | <a href="#">RuO<sub>2</sub></a>                                         | <i>P4<sub>2</sub>/mnm</i> (136) | <i>P4<sub>2</sub>'/mnm'</i> (136.499) | <i>4'/mm'm</i>  | ×        | ×   |
| 0.608  | <a href="#">PrMnO<sub>3</sub></a>                                       | <i>Pbnm</i> (62)                | <i>Pn'ma'</i> (62.448)                | <i>m'm'm</i>    | ×        | ✓   |
| 0.609  | <a href="#">NdMnO<sub>3</sub></a>                                       | <i>Pbnm</i> (62)                | <i>P2<sub>1</sub>/m</i> (11.50)       | <i>2/m</i>      | ×        | ✓   |
| 0.610  | <a href="#">Pr<sub>0.95</sub>Ko<sub>0.05</sub>MnO<sub>3</sub></a>       | <i>Pbnm</i> (62)                | <i>Pn'ma'</i> (62.448)                | <i>m'm'm</i>    | ×        | ✓   |
| 0.611  | <a href="#">BaMnSb<sub>2</sub></a>                                      | <i>I4/mmm</i> (139)             | <i>I4'/m'm'm</i> (139.536)            | <i>4'/m'm'm</i> | PT-wP    | ×   |
| 0.612  | <a href="#">Cu<sub>2</sub>OSO<sub>4</sub></a>                           | <i>C2/m</i> (12)                | <i>C2/m</i> (12.58)                   | <i>2/m</i>      | ×        | ✓   |
| 0.613  | <a href="#">FeCr<sub>2</sub>S<sub>4</sub></a>                           | <i>Fd3m</i> (227)               | <i>I4<sub>1</sub>/am'd'</i> (141.557) | <i>4/mm'm'</i>  | ×        | ✓   |
| 0.614  | <a href="#">FeCr<sub>2</sub>S<sub>4</sub></a>                           | <i>Fd3m</i> (227)               | <i>I4<sub>1</sub>/am'd'</i> (141.557) | <i>4/mm'm'</i>  | ×        | ✓   |
| 0.615  | <a href="#">FeCr<sub>2</sub>S<sub>4</sub></a>                           | <i>Fd3m</i> (227)               | <i>I4<sub>1</sub>/am'd'</i> (141.557) | <i>4/mm'm'</i>  | ×        | ✓   |
| 0.616  | <a href="#">HoB<sub>2</sub></a>                                         | <i>P6/mmm</i> (191)             | <i>C2'/m'</i> (12.62)                 | <i>2'/m'</i>    | ×        | ✓   |
| 0.617  | <a href="#">KMnSb</a>                                                   | <i>P4/nmm</i> (129)             | <i>P4'/n'm'm</i> (129.416)            | <i>4'/m'm'm</i> | PT-wP    | ×   |
| 0.618  | <a href="#">KMnBi</a>                                                   | <i>P4/nmm</i> (129)             | <i>P4'/n'm'm</i> (129.416)            | <i>4'/m'm'm</i> | PT-wP    | ×   |
| 0.619  | <a href="#">LaMnAsO</a>                                                 | <i>P4/nmm</i> (129)             | <i>P4'/n'm'm</i> (129.416)            | <i>4'/m'm'm</i> | PT-wP    | ×   |
| 0.620  | <a href="#">NdMnAsO</a>                                                 | <i>P4/nmm</i> (129)             | <i>P4'/n'm'm</i> (129.416)            | <i>4'/m'm'm</i> | PT-wP    | ×   |
| 0.621  | <a href="#">NdMnAsO</a>                                                 | <i>P4/nmm</i> (129)             | <i>Pm'mn</i> (59.407)                 | <i>m'mm</i>     | PT-wP    | ×   |
| 0.622  | <a href="#">NdMnAsO</a>                                                 | <i>P4/nmm</i> (129)             | <i>Pm'mn</i> (59.407)                 | <i>m'mm</i>     | PT-wP    | ×   |
| 0.623  | <a href="#">NdMnAsO</a>                                                 | <i>P4/nmm</i> (129)             | <i>P4'/n'm'm</i> (129.416)            | <i>4'/m'm'm</i> | PT-wP    | ×   |
| 0.624  | <a href="#">LaMnAsO</a>                                                 | <i>P4/nmm</i> (129)             | <i>P4'/n'm'm</i> (129.416)            | <i>4'/m'm'm</i> | PT-wP    | ×   |
| 0.625  | <a href="#">U<sub>2</sub>Pd<sub>2</sub>In</a>                           | <i>P4/mbm</i> (127)             | <i>P4'/m'bm'</i> (127.394)            | <i>4'/m'm'm</i> | PT-wP    | ×   |
| 0.626  | <a href="#">NaMnP</a>                                                   | <i>P4/nmm</i> (129)             | <i>P4'/n'm'm</i> (129.416)            | <i>4'/m'm'm</i> | PT-wP    | ×   |
| 0.627  | <a href="#">NaMnP</a>                                                   | <i>P4/nmm</i> (129)             | <i>P4'/n'm'm</i> (129.416)            | <i>4'/m'm'm</i> | PT-wP    | ×   |

Continued on next page

TABLE S7 – continued from previous page

| BCS-ID | Formula                                                                                       | Parent           | MSG                    | MPG        | SHG type | LMO |
|--------|-----------------------------------------------------------------------------------------------|------------------|------------------------|------------|----------|-----|
| 0.628  | <a href="#">NaMnP</a>                                                                         | $P4/nmm$ (129)   | $P4'/n'm'm$ (129.416)  | $4'/m'm'm$ | PT-wP    | ×   |
| 0.629  | <a href="#">NaMnAs</a>                                                                        | $P4/nmm$ (129)   | $P4'/n'm'm$ (129.416)  | $4'/m'm'm$ | PT-wP    | ×   |
| 0.630  | <a href="#">NaMnAs</a>                                                                        | $P4/nmm$ (129)   | $P4'/n'm'm$ (129.416)  | $4'/m'm'm$ | PT-wP    | ×   |
| 0.631  | <a href="#">NaMnSb</a>                                                                        | $P4/nmm$ (129)   | $P4'/n'm'm$ (129.416)  | $4'/m'm'm$ | PT-wP    | ×   |
| 0.632  | <a href="#">NaMnSb</a>                                                                        | $P4/nmm$ (129)   | $P4'/n'm'm$ (129.416)  | $4'/m'm'm$ | PT-wP    | ×   |
| 0.633  | <a href="#">KFeS<sub>2</sub></a>                                                              | $C2/c$ (15)      | $C2'/c$ (15.87)        | $2'/m$     | PT-wP    | ×   |
| 0.634  | <a href="#">NaMnBi</a>                                                                        | $P4/nmm$ (129)   | $P4'/n'm'm$ (129.416)  | $4'/m'm'm$ | PT-wP    | ×   |
| 0.635  | <a href="#">NaMnBi</a>                                                                        | $P4/nmm$ (129)   | $P4'/n'm'm$ (129.416)  | $4'/m'm'm$ | PT-wP    | ×   |
| 0.636  | <a href="#">RbFeS<sub>2</sub></a>                                                             | $C2/c$ (15)      | $C2'/c$ (15.87)        | $2'/m$     | PT-wP    | ×   |
| 0.637  | <a href="#">KFeSe<sub>2</sub></a>                                                             | $C2/c$ (15)      | $C2'/c'$ (15.88)       | $2/m'$     | PT-wP    | ×   |
| 0.638  | <a href="#">RbFeSe<sub>2</sub></a>                                                            | $C2/c$ (15)      | $C2'/c'$ (15.88)       | $2/m'$     | PT-wP    | ×   |
| 0.639  | <a href="#">Mn<sub>2</sub>Au</a>                                                              | $I4/mmm$ (139)   | $Im'mm$ (71.535)       | $m'mm$     | PT-wP    | ×   |
| 0.640  | <a href="#">Mn<sub>2</sub>Au</a>                                                              | $I4/mmm$ (139)   | $Im'mm$ (71.535)       | $m'mm$     | PT-wP    | ×   |
| 0.641  | <a href="#">Mn<sub>3</sub>Ga</a>                                                              | $I4/mmm$ (139)   | $C2'/m'$ (12.62)       | $2'/m'$    | ×        | ✓   |
| 0.642  | <a href="#">LaMnO<sub>3</sub></a>                                                             | $Pnma$ (62)      | $Pn'ma'$ (62.448)      | $m'm'm$    | ×        | ✓   |
| 0.643  | <a href="#">La<sub>0.95</sub>Ca<sub>0.05</sub>MnO<sub>3</sub></a>                             | $Pnma$ (62)      | $Pn'ma'$ (62.448)      | $m'm'm$    | ×        | ✓   |
| 0.644  | <a href="#">La<sub>0.95</sub>Ba<sub>0.05</sub>MnO<sub>3</sub></a>                             | $Pnma$ (62)      | $Pn'ma'$ (62.448)      | $m'm'm$    | ×        | ✓   |
| 0.645  | <a href="#">La<sub>0.95</sub>Ba<sub>0.05</sub>Mn<sub>0.95</sub>O<sub>3</sub></a>              | $Pnma$ (62)      | $Pn'ma'$ (62.448)      | $m'm'm$    | ×        | ✓   |
| 0.646  | <a href="#">La<sub>0.90</sub>Ba<sub>0.10</sub>Mn<sub>0.90</sub>O<sub>3</sub></a>              | $Pnma$ (62)      | $Pn'ma'$ (62.448)      | $m'm'm$    | ×        | ✓   |
| 0.647  | <a href="#">La<sub>0.875</sub>Ba<sub>0.125</sub>Mn<sub>0.875</sub>O<sub>3</sub></a>           | $Pnma$ (62)      | $Pn'ma'$ (62.448)      | $m'm'm$    | ×        | ✓   |
| 0.648  | <a href="#">(Ho<sub>0.8</sub>Mn<sub>0.2</sub>)MnO<sub>3</sub></a>                             | $Pnma$ (62)      | $Pnm'a'$ (62.447)      | $m'm'm$    | ×        | ✓   |
| 0.649  | <a href="#">(Ho<sub>0.8</sub>Mn<sub>0.2</sub>)MnO<sub>3</sub></a>                             | $Pnma$ (62)      | $Pnm'a'$ (62.447)      | $m'm'm$    | ×        | ✓   |
| 0.650  | <a href="#">ErSi<sub>2</sub>O<sub>7</sub></a>                                                 | $C2/m$ (12)      | $C2'/m$ (12.60)        | $2'/m$     | PT-wP    | ×   |
| 0.651  | <a href="#">Er<sub>3</sub>Cu<sub>4</sub>Sn<sub>4</sub></a>                                    | $C2/m$ (12)      | $Cc2'/m$ (12.63)       | $2/m1'$    | ×        | ×   |
| 0.652  | <a href="#">HoMnO<sub>3</sub></a>                                                             | $P6_3cm$ (185)   | $P6_3cm'$ (185.2)      | $6'mm'$    | BW-woP   | ×   |
| 0.653  | <a href="#">HoMn<sub>0.99</sub>Fe<sub>0.01</sub>O<sub>3</sub></a>                             | $P6_3cm$ (185)   | $P6_3cm'$ (185.2)      | $6'mm'$    | BW-woP   | ×   |
| 0.654  | <a href="#">HoMn<sub>0.95</sub>Fe<sub>0.05</sub>O<sub>3</sub></a>                             | $P6_3cm$ (185)   | $P6_3cm'$ (185.2)      | $6'mm'$    | BW-woP   | ×   |
| 0.655  | <a href="#">HoMn<sub>0.9</sub>Fe<sub>0.1</sub>O<sub>3</sub></a>                               | $P6_3cm$ (185)   | $P6_3cm'$ (185.2)      | $6'mm'$    | BW-woP   | ×   |
| 0.656  | <a href="#">NdMn<sub>2</sub>Ge<sub>2</sub></a>                                                | $I4/mmm$ (139)   | $Im'm2'$ (44.231)      | $m'm2'$    | BW-wP    | ✓   |
| 0.657  | <a href="#">PrMn<sub>2</sub>Ge<sub>2</sub></a>                                                | $I4/mmm$ (139)   | $Im'm2'$ (44.231)      | $m'm2'$    | BW-wP    | ✓   |
| 0.658  | <a href="#">BaCuTe<sub>2</sub>O<sub>6</sub></a>                                               | $P4_132$ (213)   | $P4_132'$ (213.65)     | $4'32'$    | BW-woP   | ×   |
| 0.659  | <a href="#">NdMn<sub>0.8</sub>Fe<sub>0.2</sub>O<sub>3</sub></a>                               | $Pnma$ (62)      | $Pn'ma'$ (62.448)      | $m'm'm$    | ×        | ✓   |
| 0.660  | <a href="#">NdMn<sub>0.8</sub>Fe<sub>0.2</sub>O<sub>3</sub></a>                               | $Pnma$ (62)      | $Pn'ma'$ (62.448)      | $m'm'm$    | ×        | ✓   |
| 0.661  | <a href="#">(Lu<sub>0.6</sub>Mn<sub>0.4</sub>)MnO<sub>3</sub></a>                             | $Pnma$ (62)      | $Pnm'a'$ (62.447)      | $m'm'm$    | ×        | ✓   |
| 0.662  | <a href="#">Mn<sub>3</sub>Sn<sub>2</sub></a>                                                  | $Pnma$ (62)      | $Pn'ma'$ (62.448)      | $m'm'm$    | ×        | ✓   |
| 0.663  | <a href="#">Mn<sub>3</sub>Sn<sub>2</sub></a>                                                  | $Pnma$ (62)      | $Pn'ma'$ (62.448)      | $m'm'm$    | ×        | ✓   |
| 0.664  | <a href="#">Mn<sub>3</sub>Sn<sub>2</sub></a>                                                  | $Pnma$ (62)      | $P2_1'/c'$ (14.79)     | $2'/m'$    | ×        | ✓   |
| 0.665  | <a href="#">CeMnSbO</a>                                                                       | $P4/nmm$ (129)   | $P4'/n'm'm$ (129.416)  | $4'/m'm'm$ | PT-wP    | ×   |
| 0.666  | <a href="#">CeMnSbO</a>                                                                       | $P4/nmm$ (129)   | $Pm'mn$ (59.407)       | $m'mm$     | PT-wP    | ×   |
| 0.667  | <a href="#">LaMnSbO</a>                                                                       | $P4/nmm$ (129)   | $P4'/n'm'm$ (129.416)  | $4'/m'm'm$ | PT-wP    | ×   |
| 0.668  | <a href="#">PrMnSbO</a>                                                                       | $P4/nmm$ (129)   | $Pm'mn$ (59.407)       | $m'mm$     | PT-wP    | ×   |
| 0.669  | <a href="#">Sr<sub>2</sub>YbRuO<sub>6</sub></a>                                               | $P112_1/n$ (14)  | $P2_1/c$ (14.75)       | $2/m$      | ×        | ✓   |
| 0.670  | <a href="#">Sr<sub>2</sub>YbRuO<sub>6</sub></a>                                               | $P2_1/n$ (14)    | $P2_1/c$ (14.75)       | $2/m$      | ×        | ✓   |
| 0.671  | <a href="#">Sr<sub>2</sub>TmRuO<sub>6</sub></a>                                               | $P2_1/n$ (14)    | $P2_1/c$ (14.75)       | $2/m$      | ×        | ✓   |
| 0.672  | <a href="#">CaCu<sub>3</sub>Fe<sub>2</sub>Sb<sub>2</sub>O<sub>12</sub></a>                    | $Pn3$ (201)      | $Pn'n'n$ (48.260)      | $m'm'm$    | ×        | ✓   |
| 0.673  | <a href="#">MnFe<sub>4</sub>Si<sub>3</sub></a>                                                | $P6_3/mcm$ (193) | $P6_3/mc'm'$ (193.260) | $6/mm'm'$  | ×        | ✓   |
| 0.674  | <a href="#">MnFe<sub>4</sub>Si<sub>3</sub></a>                                                | $P6_3/mcm$ (193) | $P6_3/mc'm'$ (193.260) | $6/mm'm'$  | ×        | ✓   |
| 0.675  | <a href="#">MnFe<sub>4</sub>Si<sub>3</sub></a>                                                | $P6_3/mcm$ (193) | $P6_3/mc'm'$ (193.260) | $6/mm'm'$  | ×        | ✓   |
| 0.676  | <a href="#">Nd<sub>0.95</sub>Sr<sub>0.05</sub>CrO<sub>3</sub></a>                             | $P$ (62)         | $Pnma$ (62.441)        | $mmm$      | ×        | ×   |
| 0.677  | <a href="#">Nd<sub>0.9</sub>Sr<sub>0.1</sub>CrO<sub>3</sub></a>                               | $Pbnm$ (62)      | $Pnma$ (62.441)        | $mmm$      | ×        | ×   |
| 0.678  | <a href="#">Nd<sub>0.85</sub>Sr<sub>0.15</sub>CrO<sub>3</sub></a>                             | $Pbnm$ (62)      | $Pnma$ (62.441)        | $mmm$      | ×        | ×   |
| 0.679  | <a href="#">TbCr<sub>0.5</sub>Mn<sub>0.5</sub>O<sub>3</sub></a>                               | $Pbnm$ (62)      | $Pn'ma'$ (62.448)      | $m'm'm$    | ×        | ✓   |
| 0.680  | <a href="#">Bi<sub>0.8</sub>La<sub>0.2</sub>Fe<sub>0.5</sub>Mn<sub>0.3</sub>O<sub>7</sub></a> | $I4/m$ (74)      | $Imm'a'$ (74.559)      | $m'm'm$    | ×        | ✓   |
| 0.681  | <a href="#">Ce<sub>4</sub>Sb<sub>3</sub></a>                                                  | $I43d$ (220)     | $I4'2d'$ (122.336)     | $4'2m'$    | BW-woP   | ×   |
| 0.682  | <a href="#">Ca<sub>2</sub>FeOsO<sub>6</sub></a>                                               | $P2_1/n$ (14)    | $P2_1'/c'$ (14.79)     | $2'/m'$    | ×        | ✓   |
| 0.683  | <a href="#">SrCaFeOsO<sub>6</sub></a>                                                         | $P2_1/n$ (14)    | $P2_1'/c'$ (14.79)     | $2'/m'$    | ×        | ✓   |
| 0.684  | <a href="#">TbPt</a>                                                                          | $Pnma$ (62)      | $Pn'm'a$ (62.446)      | $m'm'm$    | ×        | ✓   |
| 0.685  | <a href="#">ErPt</a>                                                                          | $Pnma$ (62)      | $Pnm'a'$ (62.447)      | $m'm'm$    | ×        | ✓   |

Continued on next page

TABLE S7 – continued from previous page

| BCS-ID | Formula                                                                | Parent                          | MSG                                   | MPG             | SHG type | LMO |
|--------|------------------------------------------------------------------------|---------------------------------|---------------------------------------|-----------------|----------|-----|
| 0.686  | HoPt                                                                   | <i>Pnma</i> (62)                | <i>Pnm'a'</i> (62.447)                | <i>m'm'm</i>    | ×        | ✓   |
| 0.687  | DyPt                                                                   | <i>Pnma</i> (62)                | <i>Pn'm'a</i> (62.446)                | <i>m'm'm</i>    | ×        | ✓   |
| 0.688  | TmPt                                                                   | <i>Pnma</i> (62)                | <i>Pnm'a'</i> (62.447)                | <i>m'm'm</i>    | ×        | ✓   |
| 0.689  | PrPt                                                                   | <i>Cmcm</i> (63)                | <i>Cm'c'm</i> (63.462)                | <i>m'm'm</i>    | ×        | ✓   |
| 0.690  | NdPt                                                                   | <i>Cmcm</i> (63)                | <i>C2'/c'</i> (15.89)                 | <i>2'/m'</i>    | ×        | ✓   |
| 0.691  | CaCo <sub>1.86</sub> As <sub>2</sub>                                   | <i>I4/mmm</i> (139)             | <i>P4/nnc</i> (126.386)               | <i>4/mmm1'</i>  | ×        | ×   |
| 0.692  | Ba <sub>4</sub> Ru <sub>3</sub> O <sub>10</sub>                        | <i>Cmce</i> (64)                | <i>Cm'ca</i> (64.471)                 | <i>m'mm</i>     | PT-wP    | ×   |
| 0.693  | Ba <sub>4</sub> Ru <sub>3</sub> O <sub>10</sub>                        | <i>Cmce</i> (64)                | <i>Cm'ca</i> (64.472)                 | <i>m'mm</i>     | PT-wP    | ×   |
| 0.694  | Bi <sub>2</sub> CuO <sub>4</sub>                                       | <i>P4/ncc</i> (130)             | <i>P4/n'c'c'</i> (130.431)            | <i>4/m'm'm'</i> | PT-wP    | ×   |
| 0.695  | Bi <sub>2</sub> CuO <sub>4</sub>                                       | <i>P4/ncc</i> (130)             | <i>Pc'cn</i> (56.367)                 | <i>m'mm</i>     | PT-wP    | ×   |
| 0.696  | SmCrO <sub>3</sub>                                                     | <i>Pbnm</i> (62)                | <i>Pn'ma'</i> (62.448)                | <i>m'm'm</i>    | ×        | ✓   |
| 0.697  | SmCrO <sub>3</sub>                                                     | <i>Pbnm</i> (62)                | <i>Pn'm'a</i> (62.446)                | <i>m'm'm</i>    | ×        | ✓   |
| 0.698  | SmCrO <sub>3</sub>                                                     | <i>Pbnm</i> (62)                | <i>Pbn'm'</i> (62.446)                | <i>m'm'm</i>    | ×        | ✓   |
| 0.699  | LiMn <sub>6</sub> Sn <sub>6</sub>                                      | <i>P6/mmm</i> (191)             | <i>Cmm'm'</i> (65.486)                | <i>m'm'm</i>    | ×        | ✓   |
| 0.700  | TbMn <sub>6</sub> Sn <sub>6</sub>                                      | <i>P6/mmm</i> (191)             | <i>P6/mmm'm'</i> (191.240)            | <i>6/mmm'm'</i> | ×        | ✓   |
| 0.701  | TbMn <sub>6</sub> Sn <sub>6</sub>                                      | <i>P6/mmm</i> (191)             | <i>P6/mmm'm'</i> (191.240)            | <i>6/mmm'm'</i> | ×        | ✓   |
| 0.702  | TbMn <sub>6</sub> Sn <sub>6</sub>                                      | <i>P6/mmm</i> (191)             | <i>C2'/m'</i> (12.62)                 | <i>2'/m'</i>    | ×        | ✓   |
| 0.703  | HoMn <sub>6</sub> Sn <sub>6</sub>                                      | <i>P6/mmm</i> (191)             | <i>C2'/m'</i> (12.62)                 | <i>2'/m'</i>    | ×        | ✓   |
| 0.704  | HoMn <sub>6</sub> Sn <sub>6</sub>                                      | <i>P6/mmm</i> (191)             | <i>C2'/m'</i> (12.62)                 | <i>2'/m'</i>    | ×        | ✓   |
| 0.705  | HoMn <sub>6</sub> Sn <sub>6</sub>                                      | <i>P6/mmm</i> (191)             | <i>Cmm'm'</i> (65.486)                | <i>m'm'm</i>    | ×        | ✓   |
| 0.706  | Tb <sub>2</sub> Ir <sub>3</sub> Ga <sub>9</sub>                        | <i>Cmcm</i> (63)                | <i>Cm'cm'</i> (63.464)                | <i>m'm'm</i>    | ×        | ✓   |
| 0.707  | Tb <sub>2</sub> Ir <sub>3</sub> Ga <sub>9</sub>                        | <i>Cmcm</i> (63)                | <i>Cm'cm'</i> (63.464)                | <i>m'm'm</i>    | ×        | ✓   |
| 0.708  | CrNb <sub>4</sub> S <sub>8</sub>                                       | <i>P6<sub>3</sub>/mmc</i> (194) | <i>P6<sub>3</sub>'m'm'c</i> (194.268) | <i>6'/m'mm'</i> | ×        | ×   |
| 0.709  | MnNb <sub>4</sub> S <sub>8</sub>                                       | <i>P6<sub>3</sub>/mmc</i> (194) | <i>Cmc'm'</i> (63.463)                | <i>m'm'm</i>    | ×        | ✓   |
| 0.710  | MnNb <sub>3</sub> S <sub>6</sub>                                       | <i>P6<sub>3</sub>22</i> (182)   | <i>C22'2<sub>1</sub>'</i> (20.34)     | <i>2'2'2</i>    | BW-woP   | ✓   |
| 0.711  | MnTa <sub>4</sub> S <sub>8</sub>                                       | <i>P6<sub>3</sub>/mmc</i> (194) | <i>Cmc'm'</i> (63.463)                | <i>m'm'm</i>    | ×        | ✓   |
| 0.712  | VNb <sub>3</sub> S <sub>6</sub>                                        | <i>P6<sub>3</sub>22</i> (182)   | <i>C2'2'2<sub>1</sub>'</i> (20.33)    | <i>2'2'2</i>    | BW-woP   | ✓   |
| 0.713  | NiFe <sub>2</sub> O <sub>4</sub>                                       | <i>Fd3m</i> (227)               | <i>I4<sub>1</sub>/am'd'</i> (141.557) | <i>4/mmm'm'</i> | ×        | ✓   |
| 0.714  | Li <sub>2</sub> Ni(SO <sub>4</sub> ) <sub>2</sub>                      | <i>P2<sub>1</sub>/c</i> (14)    | <i>P2<sub>1</sub>/c</i> (14.75)       | <i>2/m</i>      | ×        | ✓   |
| 0.715  | HoCrWO <sub>6</sub>                                                    | <i>Pna2<sub>1</sub></i> (33)    | <i>Pna2<sub>1</sub></i> (33.144)      | <i>mm2</i>      | O-woP    | ×   |
| 0.716  | HoCrWO <sub>6</sub>                                                    | <i>Pna2<sub>1</sub></i> (33)    | <i>Pna2<sub>1</sub></i> (33.144)      | <i>mm2</i>      | O-woP    | ×   |
| 0.717  | Pr <sub>0.5</sub> Sr <sub>0.4</sub> Ba <sub>0.1</sub> CoO <sub>4</sub> | <i>P4/nma</i> (74)              | <i>Im'm'a</i> (74.558)                | <i>m'm'm</i>    | ×        | ✓   |
| 0.718  | Pr <sub>0.5</sub> Sr <sub>0.4</sub> Ba <sub>0.1</sub> CoO <sub>4</sub> | <i>P4/mcm</i> (140)             | <i>Fm'm'm</i> (69.524)                | <i>m'm'm</i>    | ×        | ✓   |
| 0.719  | Yb <sub>0.42</sub> Sc <sub>0.58</sub> FeO <sub>3</sub>                 | <i>P6<sub>3</sub>cm</i> (185)   | <i>P6<sub>3</sub>c'm'</i> (185.201)   | <i>6m'm'</i>    | BW-woP   | ✓   |
| 0.720  | Yb <sub>0.42</sub> Sc <sub>0.58</sub> FeO <sub>3</sub>                 | <i>P6<sub>3</sub>cm</i> (185)   | <i>P6<sub>3</sub></i> (173.129)       | <i>6</i>        | O-woP    | ✓   |
| 0.721  | Yb <sub>0.42</sub> Sc <sub>0.58</sub> FeO <sub>3</sub>                 | <i>P6<sub>3</sub>cm</i> (185)   | <i>P6<sub>3</sub></i> (173.129)       | <i>6</i>        | O-woP    | ✓   |
| 0.722  | Mn <sub>4</sub> Nb <sub>2</sub> O <sub>9</sub>                         | <i>Cc</i> (9)                   | <i>Cc</i> (9.37)                      | <i>m</i>        | O-woP    | ✓   |
| 0.723  | YbCl <sub>3</sub>                                                      | <i>C2/m</i> (12)                | <i>C2'/m</i> (12.60)                  | <i>2'/m</i>     | PT-wP    | ×   |
| 0.724  | BaCoSiO <sub>4</sub>                                                   | <i>P6<sub>3</sub></i> (173)     | <i>P6<sub>3</sub></i> (173.129)       | <i>6</i>        | O-woP    | ✓   |
| 0.725  | Ce <sub>5</sub> TeO <sub>8</sub>                                       | <i>Fd3m</i> (227)               | <i>I4<sub>1</sub>/am'd'</i> (141.557) | <i>4/mmm'm'</i> | ×        | ✓   |
| 0.726  | CsMn <sub>2</sub> F <sub>6</sub>                                       | <i>Pnma</i> (62)                | <i>Pnm'a'</i> (62.447)                | <i>m'm'm</i>    | ×        | ✓   |
| 0.727  | CsMn <sub>2</sub> F <sub>6</sub>                                       | <i>Pnma</i> (62)                | <i>P2<sub>1</sub>/c</i> (14.75)       | <i>2/m</i>      | ×        | ✓   |
| 0.728  | MoP <sub>3</sub> SiO <sub>11</sub>                                     | <i>R3c</i> (167)                | <i>C2'/c'</i> (15.88)                 | <i>2'/m'</i>    | PT-wP    | ×   |
| 0.729  | ErNi <sub>4</sub> B                                                    | <i>P6/mmm</i> (191)             | <i>P6/mmm'm'</i> (191.240)            | <i>6/mmm'm'</i> | ×        | ✓   |
| 0.730  | TbNi <sub>4</sub> B                                                    | <i>P6/mmm</i> (191)             | <i>C2'/m'</i> (12.62)                 | <i>2'/m'</i>    | ×        | ✓   |
| 0.731  | HoNi <sub>4</sub> B                                                    | <i>P6/mmm</i> (191)             | <i>C2'/m'</i> (12.62)                 | <i>2'/m'</i>    | ×        | ✓   |
| 0.732  | SrRuO <sub>3</sub>                                                     | <i>Pnma</i> (62)                | <i>Pn'm'a</i> (62.446)                | <i>m'm'm</i>    | ×        | ✓   |
| 0.733  | AgRuO <sub>3</sub>                                                     | <i>R3c</i> (167)                | <i>R3'c'</i> (167.106)                | <i>3'm'</i>     | PT-wP    | ×   |
| 0.734  | Mn <sub>3</sub> Ta <sub>2</sub> O <sub>8</sub>                         | <i>I4<sub>1</sub>/a</i> (88)    | <i>C2'/c</i> (15.87)                  | <i>2'/m</i>     | PT-wP    | ×   |
| 0.735  | LaBaMn <sub>2</sub> O <sub>5</sub>                                     | <i>P4/nmm</i> (129)             | <i>P4/nm'm'</i> (129.417)             | <i>4/mmm'm'</i> | ×        | ✓   |
| 0.736  | LaBaMn <sub>2</sub> O <sub>6</sub>                                     | <i>Pm3m</i> (221)               | <i>P4/mmm'm'</i> (123.345)            | <i>4/mmm'm'</i> | ×        | ✓   |
| 0.737  | LaBaMn <sub>2</sub> O <sub>6</sub>                                     | <i>P4/mmm</i> (123)             | <i>P4/mmm'm'</i> (123.345)            | <i>4/mmm'm'</i> | ×        | ✓   |
| 0.738  | LaBaMn <sub>2</sub> O <sub>6</sub>                                     | <i>P4/mmm</i> (123)             | <i>P4/mmm'm'</i> (123.345)            | <i>4/mmm'm'</i> | ×        | ✓   |
| 0.739  | YBaMn <sub>2</sub> O <sub>5</sub>                                      | <i>P4/nmm</i> (129)             | <i>P4/nm'm'</i> (129.417)             | <i>4/mmm'm'</i> | ×        | ✓   |
| 0.740  | Dy <sub>3</sub> Ga <sub>5</sub> O <sub>12</sub>                        | <i>Ia3d</i> (230)               | <i>Ia3d'</i> (230.148)                | <i>m3m'</i>     | ×        | ×   |
| 0.741  | Er <sub>3</sub> Ga <sub>5</sub> O <sub>12</sub>                        | <i>Ia3d</i> (230)               | <i>Ia3d'</i> (230.148)                | <i>m3m'</i>     | ×        | ×   |
| 0.742  | Tb <sub>3</sub> Ga <sub>5</sub> O <sub>12</sub>                        | <i>Ia3d</i> (230)               | <i>Ia3d'</i> (230.148)                | <i>m3m'</i>     | ×        | ×   |

Continued on next page

TABLE S7 – continued from previous page

| BCS-ID | Formula                                                                                                                            | Parent                                     | MSG                                              | MPG                  | SHG type | LMO |
|--------|------------------------------------------------------------------------------------------------------------------------------------|--------------------------------------------|--------------------------------------------------|----------------------|----------|-----|
| 0.743  | <a href="#">Ho<sub>3</sub>Al<sub>5</sub>O<sub>12</sub></a>                                                                         | <i>Ia</i> $\bar{3}d$ (230)                 | <i>Ia</i> $\bar{3}d'$ (230.148)                  | <i>m</i> $\bar{3}m'$ | ×        | ×   |
| 0.744  | <a href="#">Tb<sub>3</sub>Al<sub>5</sub>O<sub>12</sub></a>                                                                         | <i>Ia</i> $\bar{3}d$ (230)                 | <i>Ia</i> $\bar{3}d'$ (230.148)                  | <i>m</i> $\bar{3}m'$ | ×        | ×   |
| 0.745  | <a href="#">Ho<sub>3</sub>Ga<sub>5</sub>O<sub>12</sub></a>                                                                         | <i>Ia</i> $\bar{3}d$ (230)                 | <i>Ia</i> $\bar{3}d'$ (230.148)                  | <i>m</i> $\bar{3}m'$ | ×        | ×   |
| 0.746  | <a href="#">Tb<sub>3</sub>Ga<sub>5</sub>O<sub>12</sub></a>                                                                         | <i>Ia</i> $\bar{3}d$ (230)                 | <i>Ia</i> $\bar{3}d'$ (230.148)                  | <i>m</i> $\bar{3}m'$ | ×        | ×   |
| 0.747  | <a href="#">Ba<sub>3</sub>CoIr<sub>2</sub>O<sub>9</sub></a>                                                                        | <i>C</i> 2/ <i>c</i> (15)                  | <i>C</i> 2/ <i>c</i> (15.85)                     | 2/ <i>m</i>          | ×        | ✓   |
| 0.748  | <a href="#">Ba<sub>3</sub>NiRu<sub>2</sub>O<sub>9</sub></a>                                                                        | <i>P</i> 6 <sub>3</sub> / <i>mmc</i> (194) | <i>P</i> 6 <sub>3</sub> / <i>m'm'c</i> (194.268) | 6'/ <i>m'mm'</i>     | ×        | ×   |
| 0.749  | <a href="#">Ba<sub>3</sub>CoRu<sub>2</sub>O<sub>9</sub></a>                                                                        | <i>Cmcm</i> (63)                           | <i>P</i> <i>Bnma</i> (62.454)                    | <i>mmm</i> 1'        | ×        | ×   |
| 0.750  | <a href="#">Ba<sub>3</sub>CoRu<sub>2</sub>O<sub>9</sub></a>                                                                        | <i>P</i> 6 <sub>3</sub> / <i>mmc</i> (194) | <i>P</i> <i>Bnma</i> (62.454)                    | <i>mmm</i> 1'        | ×        | ×   |
| 0.751  | <a href="#">Ca<sub>2</sub>YZr<sub>2</sub>Fe<sub>3</sub>O<sub>12</sub></a>                                                          | <i>Ia</i> $\bar{3}d$ (230)                 | <i>R</i> $\bar{3}'c$ (167.105)                   | $\bar{3}'m$          | PT-wP    | ×   |
| 0.752  | <a href="#">Ca<sub>2</sub>YZr<sub>2</sub>Fe<sub>3</sub>O<sub>12</sub></a>                                                          | <i>Ia</i> $\bar{3}d$ (230)                 | <i>R</i> $\bar{3}'c$ (167.105)                   | $\bar{3}'m$          | PT-wP    | ×   |
| 0.753  | <a href="#">Ca<sub>2</sub>LaZr<sub>2</sub>Fe<sub>3</sub>O<sub>12</sub></a>                                                         | <i>Ia</i> $\bar{3}d$ (230)                 | <i>R</i> $\bar{3}'c$ (167.105)                   | $\bar{3}'m$          | PT-wP    | ×   |
| 0.754  | <a href="#">Ca<sub>2</sub>LaZr<sub>2</sub>Fe<sub>3</sub>O<sub>12</sub></a>                                                         | <i>Ia</i> $\bar{3}d$ (230)                 | <i>R</i> $\bar{3}'c$ (167.105)                   | $\bar{3}'m$          | PT-wP    | ×   |
| 0.755  | <a href="#">Mn<sub>2</sub>SeO<sub>3</sub>F<sub>2</sub></a>                                                                         | <i>Pnma</i> (62)                           | <i>Pn'ma'</i> (62.448)                           | <i>m'm'm</i>         | ×        | ✓   |
| 0.756  | <a href="#">GaV<sub>4</sub>S<sub>8</sub></a>                                                                                       | <i>R</i> 3 <i>m</i> (160)                  | <i>R</i> 3 <i>m'</i> (160.67)                    | 3 <i>m'</i>          | BW-woP   | ✓   |
| 0.757  | <a href="#">CeFeO<sub>3</sub></a>                                                                                                  | <i>Pbnm</i> (62)                           | <i>Pn'ma'</i> (62.448)                           | <i>m'm'm</i>         | ×        | ✓   |
| 0.758  | <a href="#">CeFeO<sub>3</sub></a>                                                                                                  | <i>Pbnm</i> (62)                           | <i>Pnma</i> (62.441)                             | <i>mmm</i>           | ×        | ×   |
| 0.759  | <a href="#">CeFeO<sub>3</sub></a>                                                                                                  | <i>Pbnm</i> (62)                           | <i>Pnma</i> (62.441)                             | <i>mmm</i>           | ×        | ×   |
| 0.760  | <a href="#">FeOHSO<sub>4</sub></a>                                                                                                 | <i>C</i> 2/ <i>c</i> (15)                  | <i>C</i> 2'/ <i>c'</i> (15.89)                   | 2'/ <i>m'</i>        | ×        | ✓   |
| 0.761  | <a href="#">SrFe<sub>2</sub>Se<sub>2</sub>O</a>                                                                                    | <i>Pmmn</i> (59)                           | <i>Pm'm'n'</i> (59.411)                          | <i>m'm'm'</i>        | PT-wP    | ×   |
| 0.762  | <a href="#">SrFe<sub>2</sub>S<sub>2</sub>O</a>                                                                                     | <i>Pmmn</i> (59)                           | <i>Pm'm'n'</i> (59.411)                          | <i>m'm'm'</i>        | PT-wP    | ×   |
| 0.763  | <a href="#">Mn<sub>5</sub>(PO<sub>4</sub>)<sub>2</sub>(PO<sub>3</sub>(<del>OP</del>)<sub>2</sub>e(<del>H5</del>)H)<sub>4</sub></a> | <i>C</i> 2'/ <i>c'</i> (15.89)             | <i>C</i> 2'/ <i>c'</i> (15.89)                   | 2'/ <i>m'</i>        | ×        | ✓   |
| 0.764  | <a href="#">Mn<sub>5</sub>(PO<sub>4</sub>)<sub>2</sub>(PO<sub>3</sub>(<del>OP</del>)<sub>2</sub>e(<del>H5</del>)H)<sub>4</sub></a> | <i>C</i> 2'/ <i>c'</i> (15.89)             | <i>C</i> 2'/ <i>c'</i> (15.89)                   | 2'/ <i>m'</i>        | ×        | ✓   |
| 0.765  | <a href="#">Mn<sub>5</sub>(PO<sub>4</sub>)<sub>2</sub>(PO<sub>3</sub>(<del>OP</del>)<sub>2</sub>e(<del>H5</del>)H)<sub>4</sub></a> | <i>C</i> 2'/ <i>c'</i> (15.89)             | <i>C</i> 2'/ <i>c'</i> (15.89)                   | 2'/ <i>m'</i>        | ×        | ✓   |
| 0.766  | <a href="#">YbMnSb<sub>2</sub></a>                                                                                                 | <i>P</i> 4/ <i>mmm</i> (129)               | <i>P</i> 4'/ <i>n'm'm</i> (129.416)              | 4'/ <i>m'm'm</i>     | PT-wP    | ×   |
| 0.767  | <a href="#">SrMnSb<sub>2</sub></a>                                                                                                 | <i>Pnma</i> (62)                           | <i>Pn'ma'</i> (62.448)                           | <i>m'm'm</i>         | ×        | ✓   |
| 0.768  | <a href="#">SrMnSb<sub>2</sub></a>                                                                                                 | <i>Pnma</i> (62)                           | <i>Pn'a'2<sub>1</sub></i> (33.148)               | <i>m'm'2</i>         | BW-wP    | ✓   |
| 0.769  | <a href="#">YbMnBi<sub>2</sub></a>                                                                                                 | <i>P</i> 4/ <i>mmm</i> (129)               | <i>P</i> 4'/ <i>n'm'm</i> (129.416)              | 4'/ <i>m'm'm</i>     | PT-wP    | ×   |
| 0.770  | <a href="#">Fe<sub>2</sub>Co<sub>2</sub>Nb<sub>2</sub>O<sub>9</sub></a>                                                            | <i>P</i> 31 <i>c</i> (165)                 | <i>C</i> 2'/ <i>c'</i> (15.88)                   | 2'/ <i>m'</i>        | PT-wP    | ×   |
| 0.771  | <a href="#">PrMnSi<sub>2</sub></a>                                                                                                 | <i>Cmcm</i> (63)                           | <i>Cm'cm'</i> (63.464)                           | <i>m'm'm</i>         | ×        | ✓   |
| 0.772  | <a href="#">PrMnSi<sub>2</sub></a>                                                                                                 | <i>Cmcm</i> (63)                           | <i>Cm'cm'</i> (63.464)                           | <i>m'm'm</i>         | ×        | ✓   |
| 0.773  | <a href="#">NdMnSi<sub>2</sub></a>                                                                                                 | <i>Cmcm</i> (63)                           | <i>C</i> 2'/ <i>m'</i> (12.62)                   | 2'/ <i>m'</i>        | ×        | ✓   |
| 0.774  | <a href="#">NdMnSi<sub>2</sub></a>                                                                                                 | <i>Cmcm</i> (63)                           | <i>Cm'cm'</i> (63.464)                           | <i>m'm'm</i>         | ×        | ✓   |
| 0.775  | <a href="#">NdMnSi<sub>2</sub></a>                                                                                                 | <i>Cmcm</i> (63)                           | <i>Cm'cm'</i> (63.464)                           | <i>m'm'm</i>         | ×        | ✓   |
| 0.776  | <a href="#">CeMnSi<sub>2</sub></a>                                                                                                 | <i>Cmcm</i> (63)                           | <i>Cm'cm'</i> (63.464)                           | <i>m'm'm</i>         | ×        | ✓   |
| 0.777  | <a href="#">CeMnSi<sub>2</sub></a>                                                                                                 | <i>Cmcm</i> (63)                           | <i>Cm'cm'</i> (63.464)                           | <i>m'm'm</i>         | ×        | ✓   |
| 0.778  | <a href="#">LaMnSi<sub>2</sub></a>                                                                                                 | <i>Cmcm</i> (63)                           | <i>Cm'cm'</i> (63.464)                           | <i>m'm'm</i>         | ×        | ✓   |
| 0.779  | <a href="#">LaMnSi<sub>2</sub></a>                                                                                                 | <i>Cmcm</i> (63)                           | <i>Cm'cm'</i> (63.464)                           | <i>m'm'm</i>         | ×        | ✓   |
| 0.780  | <a href="#">LaMnSi<sub>2</sub></a>                                                                                                 | <i>Cmcm</i> (63)                           | <i>Cm'cm'</i> (63.464)                           | <i>m'm'm</i>         | ×        | ✓   |
| 0.781  | <a href="#">CeMnSi<sub>2</sub></a>                                                                                                 | <i>Cmcm</i> (63)                           | <i>Cm'cm'</i> (63.464)                           | <i>m'm'm</i>         | ×        | ✓   |
| 0.782  | <a href="#">NdScO<sub>3</sub></a>                                                                                                  | <i>Pbnm</i> (62)                           | <i>Pnm'a</i> (62.444)                            | <i>m'mm</i>          | PT-wP    | ×   |
| 0.783  | <a href="#">NdInO<sub>3</sub></a>                                                                                                  | <i>Pbnm</i> (62)                           | <i>Pnm'a</i> (62.444)                            | <i>m'mm</i>          | PT-wP    | ×   |
| 0.784  | <a href="#">NdCoO<sub>3</sub></a>                                                                                                  | <i>Pbnm</i> (62)                           | <i>Pnma</i> (62.441)                             | <i>mmm</i>           | ×        | ×   |
| 0.785  | <a href="#">NdVO<sub>3</sub></a>                                                                                                   | <i>Pbnm</i> (62)                           | <i>P</i> 2' <sub>1</sub> / <i>m'</i> (11.54)     | 2'/ <i>m'</i>        | ×        | ✓   |
| 0.786  | <a href="#">NdVO<sub>3</sub></a>                                                                                                   | <i>Pbnm</i> (62)                           | <i>P</i> 2' <sub>1</sub> / <i>m'</i> (11.54)     | 2'/ <i>m'</i>        | ×        | ✓   |
| 0.787  | <a href="#">YVO<sub>3</sub></a>                                                                                                    | <i>Pbnm</i> (62)                           | <i>Pn'm'a</i> (62.446)                           | <i>m'm'm</i>         | ×        | ✓   |
| 0.788  | <a href="#">YVO<sub>3</sub></a>                                                                                                    | <i>P</i> 2 <sub>1</sub> / <i>b</i> 11 (14) | <i>P</i> 1 (2.4)                                 | 1                    | ×        | ✓   |
| 0.789  | <a href="#">CeCuSi</a>                                                                                                             | <i>P</i> 6 <sub>3</sub> / <i>mmc</i> (194) | <i>Cmc'm'</i> (63.463)                           | <i>m'm'm</i>         | ×        | ✓   |
| 0.790  | <a href="#">Sr<sub>2</sub>DyRuO<sub>6</sub></a>                                                                                    | <i>P</i> 2 <sub>1</sub> / <i>n</i> (14)    | <i>P</i> 2' <sub>1</sub> / <i>c'</i> (14.79)     | 2'/ <i>m'</i>        | ×        | ✓   |
| 0.791  | <a href="#">Sr<sub>2</sub>TbRuO<sub>6</sub></a>                                                                                    | <i>P</i> 2 <sub>1</sub> / <i>n</i> (14)    | <i>P</i> 2 <sub>1</sub> / <i>c</i> (14.75)       | 2/ <i>m</i>          | ×        | ✓   |
| 0.792  | <a href="#">Sr<sub>2</sub>HoRuO<sub>6</sub></a>                                                                                    | <i>P</i> 2 <sub>1</sub> / <i>n</i> (14)    | <i>P</i> 2 <sub>1</sub> / <i>c</i> (14.75)       | 2/ <i>m</i>          | ×        | ✓   |
| 0.793  | <a href="#">Sr<sub>2</sub>HoRuO<sub>6</sub></a>                                                                                    | <i>P</i> 2 <sub>1</sub> / <i>n</i> (14)    | <i>P</i> 2 <sub>1</sub> / <i>c</i> (14.75)       | 2/ <i>m</i>          | ×        | ✓   |
| 0.794  | <a href="#">Sr<sub>2</sub>HoRuO<sub>6</sub></a>                                                                                    | <i>P</i> 2 <sub>1</sub> / <i>n</i> (14)    | <i>P</i> 2 <sub>1</sub> / <i>c</i> (14.75)       | 2/ <i>m</i>          | ×        | ✓   |
| 0.795  | <a href="#">Sr<sub>2</sub>YRuO<sub>6</sub></a>                                                                                     | <i>P</i> 2 <sub>1</sub> / <i>c</i> (14)    | <i>P</i> 2 <sub>1</sub> / <i>c</i> (14.75)       | 2/ <i>m</i>          | ×        | ✓   |
| 0.796  | <a href="#">Ca<sub>2</sub>NiOsO<sub>6</sub></a>                                                                                    | <i>P</i> 2 <sub>1</sub> / <i>n</i> (14)    | <i>P</i> 2' <sub>1</sub> / <i>c'</i> (14.79)     | 2'/ <i>m'</i>        | ×        | ✓   |
| 0.797  | <a href="#">SmBaMn<sub>2</sub>O<sub>5</sub></a>                                                                                    | <i>P</i> 4/ <i>mmm</i> (129)               | <i>P</i> 4/ <i>nm'm'</i> (129.417)               | 4/ <i>mm'm'</i>      | ×        | ✓   |
| 0.798  | <a href="#">MnPd<sub>2</sub></a>                                                                                                   | <i>Pnma</i> (62)                           | <i>Pnma'</i> (62.445)                            | <i>m'mm</i>          | PT-wP    | ×   |
| 0.799  | <a href="#">Sr<sub>2</sub>Co<sub>2</sub>O<sub>5</sub></a>                                                                          | <i>Ima</i> 2 (46)                          | <i>P</i> <i>1nc</i> 2 (30.122)                   | <i>mm</i> 21'        | G-woP    | ×   |

Continued on next page

TABLE S7 – continued from previous page

| BCS-ID | Formula                                                                                    | Parent           | MSG                    | MPG        | SHG type | LMO |
|--------|--------------------------------------------------------------------------------------------|------------------|------------------------|------------|----------|-----|
| 0.800  | MnTe                                                                                       | $P6_3/mmc$ (194) | $Cmcm$ (63.457)        | $mmm$      | ×        | ×   |
| 0.801  | Tl <sub>3</sub> Fe <sub>2</sub> S <sub>4</sub>                                             | $Pnma$ (62)      | $Pnma'$ (62.445)       | $m'mm$     | PT-wP    | ×   |
| 0.802  | CuFeS <sub>2</sub>                                                                         | $I42d$ (122)     | $I42d$ (122.333)       | $42m$      | O-woP    | ×   |
| 0.803  | NbMnP                                                                                      | $Pnma$ (62)      | $Pm'n2'_1$ (31.125)    | $m'm2'$    | BW-wP    | ✓   |
| 0.804  | MoP <sub>3</sub> SiO <sub>11</sub>                                                         | $R3c$ (167)      | $C2/c'$ (15.88)        | $2/m'$     | PT-wP    | ×   |
| 0.805  | DyBaCuO <sub>5</sub>                                                                       | $Pnma$ (62)      | $Pnm'a$ (62.444)       | $mm'm$     | PT-wP    | ×   |
| 0.806  | Fe <sub>2</sub> Se <sub>2</sub> O <sub>7</sub>                                             | $Pccn$ (56)      | $Pc'cn$ (56.367)       | $m'mm$     | PT-wP    | ×   |
| 0.807  | Fe <sub>2</sub> Se <sub>2</sub> O <sub>7</sub>                                             | $Pccn$ (56)      | $Pc'cn$ (56.367)       | $m'mm$     | PT-wP    | ×   |
| 0.808  | Fe <sub>2</sub> Se <sub>2</sub> O <sub>7</sub>                                             | $Pccn$ (56)      | $Pc'cn$ (56.367)       | $m'mm$     | PT-wP    | ×   |
| 0.809  | Fe <sub>2</sub> WO <sub>6</sub>                                                            | $P2_1/c$ (14)    | $P2_1/c'$ (14.78)      | $2/m'$     | PT-wP    | ×   |
| 0.810  | Fe <sub>2</sub> WO <sub>6</sub>                                                            | $Pbcn$ (60)      | $Pbc'n'$ (60.423)      | $m'm'm$    | ×        | ✓   |
| 0.811  | Fe <sub>2</sub> WO <sub>6</sub>                                                            | $Pbcn$ (60)      | $Pbc'n'$ (60.423)      | $m'm'm$    | ×        | ✓   |
| 0.812  | Fe <sub>2</sub> WO <sub>6</sub>                                                            | $Pbcn$ (60)      | $Pn'c2'$ (30.113)      | $m'm2'$    | BW-wP    | ✓   |
| 0.813  | Fe <sub>2</sub> WO <sub>6</sub>                                                            | $Pbcn$ (60)      | $Pbc'n'$ (60.423)      | $m'm'm$    | ×        | ✓   |
| 0.814  | Fe <sub>2</sub> WO <sub>6</sub>                                                            | $Pbcn$ (60)      | $Pb'cn$ (60.419)       | $m'mm$     | PT-wP    | ×   |
| 0.815  | MnNb <sub>2</sub> O <sub>6</sub>                                                           | $Pbcn$ (60)      | $Pb'cn$ (60.419)       | $m'mm$     | PT-wP    | ×   |
| 0.816  | MnTa <sub>2</sub> O <sub>6</sub>                                                           | $Pbcn$ (60)      | $Pb'cn$ (60.419)       | $m'mm$     | PT-wP    | ×   |
| 0.817  | Mn(Nb <sub>0.5</sub> Ta <sub>0.5</sub> ) <sub>2</sub> O <sub>6</sub>                       | $Pbcn$ (60)      | $Pb'cn$ (60.419)       | $m'mm$     | PT-wP    | ×   |
| 0.818  | MnTa <sub>2</sub> O <sub>6</sub>                                                           | $Pbcn$ (60)      | $Pb'cn$ (60.419)       | $m'mm$     | PT-wP    | ×   |
| 0.819  | MnNb <sub>2</sub> O <sub>6</sub>                                                           | $Pbcn$ (60)      | $Pb'cn$ (60.419)       | $m'mm$     | PT-wP    | ×   |
| 0.820  | Bi <sub>0.85</sub> Ca <sub>0.15</sub> Fe <sub>0.55</sub> Mn <sub>0.45</sub> O <sub>6</sub> | $Pnma$ (62)      | $Pn'm'a$ (62.446)      | $m'm'm$    | ×        | ✓   |
| 0.821  | SrGd <sub>2</sub> O <sub>4</sub>                                                           | $Pnma$ (62)      | $Pnma'$ (62.445)       | $m'mm$     | PT-wP    | ×   |
| 0.822  | Nd <sub>2</sub> ScNbO <sub>7</sub>                                                         | $Fd3m$ (227)     | $Fd3m'$ (227.131)      | $m3m'$     | ×        | ×   |
| 0.823  | Sr <sub>2</sub> MnGaO <sub>5</sub>                                                         | $Ima2$ (46)      | $Im'a2'$ (46.243)      | $m'm2'$    | BW-woP   | ✓   |
| 0.824  | Sr <sub>2</sub> MnGaO <sub>5.5</sub>                                                       | $P4/mmm$ (123)   | $P_C4/mbm$ (127.397)   | $4/mmm1'$  | ×        | ×   |
| 0.825  | Ca <sub>2</sub> MnGaO <sub>5</sub>                                                         | $Pnma$ (62)      | $Pnm'a'$ (62.447)      | $m'm'm$    | ×        | ✓   |
| 0.826  | MnTeLi <sub>0.003</sub>                                                                    | $P6_3/mmc$ (194) | $C2'/m'$ (12.62)       | $2'/m'$    | ×        | ✓   |
| 0.827  | Na <sub>2</sub> MnPO <sub>4</sub> F                                                        | $P2_1/c$ (14)    | $P2_1/c'$ (14.78)      | $2/m'$     | PT-wP    | ×   |
| 0.828  | Na <sub>2</sub> MnPO <sub>4</sub> F                                                        | $P2_1/n$ (14)    | $P2_1/c'$ (14.78)      | $2/m'$     | PT-wP    | ×   |
| 0.829  | Na <sub>2</sub> MnPO <sub>4</sub> F                                                        | $P2_1/n$ (14)    | $P2_1/c'$ (14.78)      | $2/m'$     | PT-wP    | ×   |
| 0.830  | Na <sub>2</sub> MnPO <sub>4</sub> F                                                        | $P2_1/n$ (14)    | $P2_1/c'$ (14.78)      | $2/m'$     | PT-wP    | ×   |
| 0.831  | BaCaFe <sub>4</sub> O <sub>7</sub>                                                         | $Pbn2_1$ (33)    | $Pn'a'2_1$ (33.148)    | $m'm'2$    | BW-woP   | ✓   |
| 0.832  | CeAuGe                                                                                     | $P6_3mc$ (186)   | $Cmc'2'_1$ (36.175)    | $m'm2'$    | BW-woP   | ✓   |
| 0.833  | CeCuGe                                                                                     | $P6_3/mmc$ (194) | $Cmc'm'$ (63.463)      | $m'm'm$    | ×        | ✓   |
| 0.834  | CrSbSe <sub>3</sub>                                                                        | $Pnma$ (62)      | $Pnm'a'$ (62.447)      | $m'm'm$    | ×        | ✓   |
| 0.835  | Dy <sub>5</sub> Pd <sub>2</sub> In <sub>4</sub>                                            | $PPbam$ (55)     | $Pb'a'm$ (55.357)      | $m'm'm$    | ×        | ✓   |
| 1.0.1  | Ag <sub>2</sub> CrO <sub>2</sub>                                                           | $P3m1$ (164)     | $C2'/m$ (12.60)        | $2'/m$     | PT-wP    | ×   |
| 1.0.2  | URu <sub>0.96</sub> Rh <sub>0.04</sub> Si <sub>2</sub>                                     | $I4/mmm$ (139)   | $Im'm'm$ (71.536)      | $m'm'm$    | ×        | ✓   |
| 1.0.3  | CsCoBr <sub>3</sub>                                                                        | $P6_3/mmc$ (194) | $Cm'c2'_1$ (36.174)    | $m'm2'$    | BW-wP    | ✓   |
| 1.0.4  | CsNiCl <sub>3</sub>                                                                        | $P6_3/mmc$ (194) | $C22'2'_1$ (20.34)     | $2'2'2$    | BW-wP    | ✓   |
| 1.0.5  | Sr <sub>3</sub> CoIrO <sub>6</sub>                                                         | $R3c$ (167)      | $P3c'1$ (165.95)       | $3m'$      | ×        | ✓   |
| 1.0.6  | CoV <sub>2</sub> O <sub>6</sub>                                                            | $C2/m$ (12)      | $C2'/m'$ (12.62)       | $2'/m'$    | ×        | ✓   |
| 1.0.7  | LuFe <sub>2</sub> O <sub>4</sub>                                                           | $R3m$ (166)      | $C2'/m'$ (12.62)       | $2'/m'$    | ×        | ✓   |
| 1.0.8  | Ba <sub>3</sub> MnNb <sub>2</sub> O <sub>9</sub>                                           | $P3m1$ (164)     | $P31m$ (157.53)        | $3m$       | O-wP     | ×   |
| 1.0.9  | CsCoCl <sub>3</sub>                                                                        | $P6_3/mmc$ (194) | $P6_3/m'cm'$ (193.259) | $6'/m'mm'$ | ×        | ×   |
| 1.0.10 | Sr <sub>3</sub> NiIrO <sub>6</sub>                                                         | $R3c$ (167)      | $P3c'1$ (165.95)       | $3m'$      | ×        | ✓   |
| 1.0.11 | CeCoGe <sub>3</sub>                                                                        | $I4mm$ (107)     | $I4m'm'$ (107.231)     | $4m'm'$    | BW-woP   | ✓   |
| 1.0.12 | UAu <sub>2</sub> Si <sub>2</sub>                                                           | $I4/mmm$ (139)   | $Im'm'm$ (71.536)      | $m'm'm$    | ×        | ✓   |
| 1.0.13 | FeI <sub>2</sub>                                                                           | $P3m1$ (164)     | $C2'/m'$ (12.62)       | $2'/m'$    | ×        | ✓   |
| 1.0.14 | CsFeCl <sub>3</sub>                                                                        | $P6_3/mmc$ (194) | $P6'2'm$ (189.223)     | $6'm2'$    | BW-wP    | ×   |
| 1.0.15 | La <sub>0.33</sub> Sr <sub>0.67</sub> FeO <sub>3</sub>                                     | $R3c$ (167)      | $P322_1$ (154.41)      | $32$       | O-wP     | ×   |
| 1.0.16 | La <sub>0.33</sub> Sr <sub>0.67</sub> FeO <sub>3</sub>                                     | $R3c$ (167)      | $C2/c$ (15.85)         | $2/m$      | ×        | ✓   |
| 1.0.17 | CaBaCo <sub>2</sub> Fe <sub>2</sub> O <sub>7</sub>                                         | $P6_3mc$ (186)   | $P31m'$ (157.55)       | $3m'$      | BW-woP   | ✓   |
| 1.0.18 | Cs <sub>2</sub> MnU <sub>3</sub> F <sub>16</sub>                                           | $P6_3/mmc$ (194) | $P6_3/mc'm'$ (193.260) | $6/mm'm'$  | ×        | ✓   |
| 1.0.19 | Cs <sub>2</sub> CoU <sub>3</sub> F <sub>16</sub>                                           | $P6_3/mmc$ (194) | $P6_3/mc'm'$ (193.260) | $6/mm'm'$  | ×        | ✓   |
| 1.0.20 | Cs <sub>2</sub> NiU <sub>3</sub> F <sub>16</sub>                                           | $P6_3/mmc$ (194) | $P6_3/mc'm'$ (193.260) | $6/mm'm'$  | ×        | ✓   |
| 1.0.21 | K <sub>2</sub> Mn <sub>3</sub> (VO <sub>4</sub> ) <sub>2</sub> CO <sub>3</sub>             | $P6_3/m$ (176)   | $P6_3/m$ (176.145)     | $6'/m$     | PT-wP    | ×   |
| 1.0.22 | K <sub>2</sub> Mn <sub>3</sub> (VO <sub>4</sub> ) <sub>2</sub> CO <sub>3</sub>             | $P6_3/m$ (176)   | $P2'_1$ (4.9)          | $2'$       | BW-wP    | ✓   |

Continued on next page

TABLE S7 – continued from previous page

| BCS-ID | Formula                                                                     | Parent                                     | MSG                                                            | MPG                                | SHG type | LMO |
|--------|-----------------------------------------------------------------------------|--------------------------------------------|----------------------------------------------------------------|------------------------------------|----------|-----|
| 1.0.23 | <a href="#">Dy<sub>3</sub>Ru<sub>4</sub>Al<sub>12</sub></a>                 | <i>P</i> 6 <sub>3</sub> / <i>mmc</i> (194) | <i>C</i> 2'/ <i>m</i> ' (12.62)                                | 2'/ <i>m</i> '                     | ×        | ✓   |
| 1.0.24 | <a href="#">ThMn<sub>2</sub></a>                                            | <i>P</i> 6 <sub>3</sub> / <i>mmc</i> (194) | <i>P</i> 6'2' <i>m</i> (189.223)                               | 6'2' <i>m</i> '                    | BW-wP    | ×   |
| 1.0.25 | <a href="#">CaBaCo<sub>3</sub>FeO<sub>7</sub></a>                           | <i>P</i> na2 <sub>1</sub> (33)             | <i>P</i> n' <i>a</i> ' <sub>2</sub> (33.148)                   | <i>m</i> ' <i>m</i> ' <sub>2</sub> | BW-woP   | ✓   |
| 1.0.26 | <a href="#">RbCoBr<sub>3</sub></a>                                          | <i>P</i> 6 <sub>3</sub> / <i>mmc</i> (194) | <i>P</i> 6 <sub>3</sub> '/ <i>m</i> ' <i>cm</i> ' (193.259)    | 6'/ <i>m</i> ' <i>mm</i> '         | ×        | ×   |
| 1.0.27 | <a href="#">Li<sub>2</sub>MnTeO<sub>6</sub></a>                             | <i>P</i> 31 <i>c</i> (163)                 | <i>P</i> 3 <i>c</i> 1 (165.91)                                 | 3 <i>m</i>                         | ×        | ×   |
| 1.0.28 | <a href="#">Tb(DCO<sub>2</sub>)<sub>3</sub></a>                             | <i>R</i> 3 <i>m</i> (160)                  | <i>P</i> 3 <i>m</i> ' <sub>1</sub> (156.51)                    | 3 <i>m</i> '                       | BW-woP   | ✓   |
| 1.0.29 | <a href="#">CeIrGe<sub>3</sub></a>                                          | <i>I</i> 4 <i>mm</i> (107)                 | <i>I</i> 4 <i>m</i> ' <i>m</i> ' (107.231)                     | 4 <i>m</i> ' <i>m</i> '            | BW-woP   | ✓   |
| 1.0.30 | <a href="#">LaCa<sub>2</sub>Fe<sub>3</sub>O<sub>9</sub></a>                 | <i>P</i> n <i>ma</i> (62)                  | <i>P</i> mn2 <sub>1</sub> (31.123)                             | <i>mm</i> 2                        | O-wP     | ×   |
| 1.0.31 | <a href="#">EuIn<sub>2</sub>As<sub>2</sub></a>                              | <i>P</i> 6 <sub>3</sub> / <i>mmc</i> (194) | <i>C</i> 2'2' <sub>2</sub> (20.33)                             | 2'2' <sub>2</sub>                  | BW-wP    | ✓   |
| 1.0.32 | <a href="#">EuIn<sub>2</sub>As<sub>2</sub></a>                              | <i>P</i> 6 <sub>3</sub> / <i>mmc</i> (194) | <i>P</i> 612'2' (178.159)                                      | 62'2'                              | BW-wP    | ✓   |
| 1.0.33 | <a href="#">FeF<sub>3</sub></a>                                             | <i>P</i> 6/ <i>mmm</i> (191)               | <i>P</i> 6 <sub>3</sub> '/ <i>m</i> ' (176.143)                | 6/ <i>m</i>                        | ×        | ✓   |
| 1.0.34 | <a href="#">RbNiCl<sub>3</sub></a>                                          | <i>P</i> 6 <sub>3</sub> / <i>mmc</i> (194) | <i>C</i> m' <i>c</i> 2' <sub>1</sub> (36.174)                  | <i>m</i> ' <i>m</i> 2'             | BW-wP    | ✓   |
| 1.0.35 | <a href="#">CsMnBr<sub>3</sub></a>                                          | <i>P</i> 6 <sub>3</sub> / <i>mmc</i> (194) | <i>P</i> 6'2' <i>m</i> ' (189.225)                             | 6' <i>m</i> ' <sub>2</sub> '       | BW-wP    | ✓   |
| 1.0.36 | <a href="#">CsMnI<sub>3</sub></a>                                           | <i>P</i> 6 <sub>3</sub> / <i>mmc</i> (194) | <i>C</i> m' <i>c</i> 2' <sub>1</sub> (36.174)                  | <i>m</i> ' <i>m</i> 2'             | BW-wP    | ✓   |
| 1.0.37 | <a href="#">CsMnI<sub>3</sub></a>                                           | <i>P</i> 6 <sub>3</sub> / <i>mmc</i> (194) | <i>C</i> m' <i>c</i> 2' <sub>1</sub> (36.174)                  | <i>m</i> ' <i>m</i> 2'             | BW-wP    | ✓   |
| 1.0.38 | <a href="#">CsCoCl<sub>3</sub></a>                                          | <i>P</i> 6 <sub>3</sub> / <i>mmc</i> (194) | <i>P</i> 6 <sub>3</sub> '/ <i>m</i> ' <i>cm</i> ' (193.259)    | 6'/ <i>m</i> ' <i>mm</i> '         | ×        | ×   |
| 1.0.39 | <a href="#">BaMnO<sub>3</sub></a>                                           | <i>P</i> 6 <sub>3</sub> / <i>mmc</i> (194) | <i>P</i> 6 <sub>3</sub> '/ <i>m</i> ' <i>cm</i> ' (193.259)    | 6'/ <i>m</i> ' <i>mm</i> '         | ×        | ×   |
| 1.0.40 | <a href="#">RbFeCl<sub>3</sub></a>                                          | <i>P</i> 6 <sub>3</sub> / <i>mmc</i> (194) | <i>P</i> 6'2' <i>m</i> ' (189.224)                             | 6' <i>m</i> ' <sub>2</sub>         | BW-wP    | ×   |
| 1.0.41 | <a href="#">RbNiCl<sub>3</sub></a>                                          | <i>P</i> 6 <sub>3</sub> / <i>mmc</i> (194) | <i>C</i> 22'2' <sub>1</sub> (20.34)                            | 2'2' <sub>2</sub>                  | BW-wP    | ✓   |
| 1.0.42 | <a href="#">CsNiCl<sub>3</sub></a>                                          | <i>P</i> 6 <sub>3</sub> / <i>mmc</i> (194) | <i>C</i> 22'2' <sub>1</sub> (20.34)                            | 2'2' <sub>2</sub>                  | BW-wP    | ✓   |
| 1.0.43 | <a href="#">UPd<sub>2</sub>Si<sub>2</sub></a>                               | <i>I</i> 4/ <i>mmm</i> (139)               | <i>I</i> 4/ <i>mm</i> ' <i>m</i> ' (139.537)                   | 4/ <i>mm</i> ' <i>m</i> '          | ×        | ✓   |
| 1.0.44 | <a href="#">Ba<sub>3</sub>CoSb<sub>2</sub>O<sub>9</sub></a>                 | <i>P</i> 6 <sub>3</sub> / <i>mmc</i> (194) | <i>C</i> m' <i>c</i> 2' <sub>1</sub> (36.174)                  | <i>m</i> ' <i>m</i> 2'             | BW-wP    | ✓   |
| 1.0.45 | <a href="#">Ba<sub>3</sub>CoSb<sub>2</sub>O<sub>9</sub></a>                 | <i>P</i> 6 <sub>3</sub> / <i>mmc</i> (194) | <i>P</i> 62 <i>m</i> (189.221)                                 | 6 <i>m</i> 2                       | O-wP     | ×   |
| 1.0.46 | <a href="#">Ba<sub>3</sub>MnSb<sub>2</sub>O<sub>9</sub></a>                 | <i>C</i> 2/ <i>c</i> (15)                  | <i>C</i> 2 (5.13)                                              | 2                                  | O-wP     | ✓   |
| 1.0.47 | <a href="#">MnSe<sub>2</sub></a>                                            | <i>P</i> a3 (205)                          | <i>P</i> bca (61.433)                                          | <i>mmm</i>                         | ×        | ×   |
| 1.0.48 | <a href="#">MnSe<sub>2</sub></a>                                            | <i>P</i> a3 (205)                          | <i>P</i> ca'2' <sub>1</sub> (29.102)                           | <i>m</i> ' <i>m</i> 2'             | BW-wP    | ✓   |
| 1.0.49 | <a href="#">BaCoSiO<sub>4</sub></a>                                         | <i>P</i> 6 <sub>3</sub> (173)              | <i>P</i> 6 <sub>3</sub> (173.129)                              | 6                                  | O-woP    | ✓   |
| 1.0.50 | <a href="#">CoGeO<sub>3</sub></a>                                           | <i>C</i> 2/ <i>c</i> (15)                  | <i>C</i> 2'/ <i>c</i> ' (15.89)                                | 2'/ <i>m</i> '                     | ×        | ✓   |
| 1.0.51 | <a href="#">Na<sub>2</sub>MnTeO<sub>6</sub></a>                             | <i>P</i> 31 <i>c</i> (163)                 | <i>R</i> 3' <i>c</i> ' (167.106)                               | 3' <i>m</i> '                      | PT-wP    | ×   |
| 1.0.52 | <a href="#">Tb<sub>14</sub>Ag<sub>51</sub></a>                              | <i>P</i> 6/ <i>m</i> (175)                 | <i>P</i> 6' (174.135)                                          | 6'                                 | BW-wP    | ×   |
| 1.1    | <a href="#">Mn<sub>3</sub>O<sub>4</sub></a>                                 | <i>P</i> bcm (57)                          | <i>P</i> <sub><i>c</i></sub> <i>nma</i> (62.452)               | <i>mmm</i> 1'                      | ×        | ×   |
| 1.2    | <a href="#">CuSe<sub>2</sub>O<sub>5</sub></a>                               | <i>C</i> 2/ <i>c</i> (15)                  | <i>P</i> <sub><i>c</i></sub> 2 <sub>1</sub> / <i>c</i> (14.84) | 2/ <i>m</i> 1'                     | ×        | ×   |
| 1.3    | <a href="#">Sr<sub>2</sub>IrO<sub>4</sub></a>                               | <i>I</i> 4 <sub>1</sub> / <i>acd</i> (142) | <i>P</i> <sub><i>I</i></sub> cca (54.352)                      | <i>mmm</i> 1'                      | ×        | ×   |
| 1.4    | <a href="#">YBa<sub>2</sub>Cu<sub>3</sub>O<sub>6+d</sub></a>                | <i>P</i> 4/ <i>mmm</i> (123)               | <i>C</i> <sub><i>a</i></sub> <i>mmm</i> (65.489)               | <i>mmm</i> 1'                      | ×        | ×   |
| 1.5    | <a href="#">YBa<sub>2</sub>Cu<sub>3</sub>O<sub>6+d</sub></a>                | <i>P</i> 4/ <i>mmm</i> (123)               | <i>F</i> <sub><i>S</i></sub> <i>mmm</i> (69.526)               | <i>mmm</i> 1'                      | ×        | ×   |
| 1.6    | <a href="#">NiO</a>                                                         | <i>F</i> m3 <i>m</i> (225)                 | <i>C</i> <sub><i>c</i></sub> 2/ <i>c</i> (15.90)               | 2/ <i>m</i> 1'                     | ×        | ×   |
| 1.7    | <a href="#">NdFe<sub>3</sub>B<sub>4</sub>O<sub>12</sub></a>                 | <i>R</i> 32 (155)                          | <i>C</i> <sub><i>c</i></sub> 2 (5.16)                          | 21'                                | G-woP    | ×   |
| 1.8    | <a href="#">CeRu<sub>2</sub>Al<sub>10</sub></a>                             | <i>C</i> mcm (63)                          | <i>P</i> <sub><i>C</i></sub> bcm (57.391)                      | <i>mmm</i> 1'                      | ×        | ×   |
| 1.9    | <a href="#">Li<sub>2</sub>VOSiO<sub>4</sub></a>                             | <i>P</i> 4/ <i>nm</i> m (129)              | <i>P</i> <sub><i>A</i></sub> bcm (57.389)                      | <i>mmm</i> 1'                      | ×        | ×   |
| 1.1    | <a href="#">Na<sub>2</sub>IrO<sub>3</sub></a>                               | <i>C</i> 2/ <i>m</i> (12)                  | <i>C</i> <sub><i>c</i></sub> 2/ <i>m</i> (12.63)               | 2/ <i>m</i> 1'                     | ×        | ×   |
| 1.11   | <a href="#">Bi<sub>4</sub>Fe<sub>5</sub>O<sub>13</sub>F</a>                 | <i>P</i> 4 <sub>2</sub> / <i>mbc</i> (135) | <i>P</i> <sub><i>C</i></sub> 42/ <i>n</i> (86.73)              | 4/ <i>m</i> 1'                     | ×        | ×   |
| 1.12   | <a href="#">BaNd<sub>0.9</sub>Y<sub>0.1</sub>MoO<sub>6</sub></a>            | <i>I</i> 4/ <i>m</i> (87)                  | <i>P</i> <sub><i>I</i></sub> 4/ <i>m</i> (83.50)               | 4/ <i>m</i> 1'                     | ×        | ×   |
| 1.13   | <a href="#">Ba<sub>3</sub>Nb<sub>2</sub>NiO<sub>9</sub></a>                 | <i>P</i> 3 <i>m</i> 1 (164)                | <i>P</i> <sub><i>c</i></sub> 31 <i>c</i> (159.64)              | 3 <i>m</i> 1'                      | G-wP     | ×   |
| 1.14   | <a href="#">Ho<sub>2</sub>BaNiO<sub>5</sub></a>                             | <i>I</i> mmm (71)                          | <i>C</i> <sub><i>c</i></sub> 2/ <i>c</i> (15.90)               | 2/ <i>m</i> 1'                     | ×        | ×   |
| 1.15   | <a href="#">Er<sub>2</sub>BaNiO<sub>5</sub></a>                             | <i>I</i> mmm (71)                          | <i>C</i> <sub><i>c</i></sub> 2/ <i>c</i> (15.90)               | 2/ <i>m</i> 1'                     | ×        | ×   |
| 1.16   | <a href="#">BaFe<sub>2</sub>As<sub>2</sub></a>                              | <i>I</i> 4/ <i>mmm</i> (139)               | <i>C</i> <sub><i>A</i></sub> <i>mca</i> (64.480)               | <i>mmm</i> 1'                      | ×        | ×   |
| 1.17   | <a href="#">CoV<sub>2</sub>O<sub>6</sub>-alpha</a>                          | <i>C</i> 2/ <i>m</i> (12)                  | <i>C</i> <sub><i>c</i></sub> 2/ <i>c</i> (15.90)               | 2/ <i>m</i> 1'                     | ×        | ×   |
| 1.18   | <a href="#">MnS<sub>2</sub></a>                                             | <i>P</i> a3 (205)                          | <i>P</i> <sub><i>b</i></sub> ca2 <sub>1</sub> (29.105)         | <i>mm</i> 21'                      | G-wP     | ×   |
| 1.19   | <a href="#">PrMn<sub>2</sub>O<sub>5</sub></a>                               | <i>P</i> bam (55)                          | <i>P</i> <sub><i>a</i></sub> ca2 <sub>1</sub> (29.104)         | <i>mm</i> 21'                      | G-wP     | ×   |
| 1.20   | <a href="#">HoMnO<sub>3</sub></a>                                           | <i>P</i> n <i>ma</i> (62)                  | <i>P</i> <sub><i>b</i></sub> mn2 <sub>1</sub> (31.129)         | <i>mm</i> 21'                      | G-wP     | ×   |
| 1.21   | <a href="#">DyCo<sub>2</sub>Si<sub>2</sub></a>                              | <i>I</i> 4/ <i>mmm</i> (139)               | <i>P</i> <sub><i>I</i></sub> 4/ <i>mnc</i> (128.410)           | 4/ <i>mmm</i> 1'                   | ×        | ×   |
| 1.22   | <a href="#">DyCu<sub>2</sub>Si<sub>2</sub></a>                              | <i>I</i> 4/ <i>mmm</i> (139)               | <i>C</i> <sub><i>c</i></sub> 2/ <i>m</i> (12.63)               | 2/ <i>m</i> 1'                     | ×        | ×   |
| 1.23   | <a href="#">La<sub>2</sub>CuO<sub>4</sub></a>                               | <i>C</i> mce (64)                          | <i>P</i> <sub><i>A</i></sub> ccn (56.374)                      | <i>mmm</i> 1'                      | ×        | ×   |
| 1.24   | <a href="#">ZnV<sub>2</sub>O<sub>4</sub></a>                                | <i>I</i> 4 <sub>1</sub> / <i>amd</i> (141) | <i>P</i> <sub><i>I</i></sub> 432 <sub>1</sub> 2 (96.150)       | 4221'                              | G-wP     | ×   |
| 1.25   | <a href="#">KFe<sub>3</sub>(OH)<sub>6</sub>(SO<sub>4</sub>)<sub>2</sub></a> | <i>R</i> 3 <i>m</i> (166)                  | <i>R</i> <sub><i>I</i></sub> 3 <i>c</i> (167.108)              | 3 <i>m</i> 1'                      | ×        | ×   |
| 1.26   | <a href="#">CsFe<sub>2</sub>Se<sub>3</sub></a>                              | <i>C</i> mcm (63)                          | <i>P</i> <sub><i>c</i></sub> 2 <sub>1</sub> / <i>c</i> (14.82) | 2/ <i>m</i> 1'                     | ×        | ×   |
| 1.27   | <a href="#">TaFe<sub>1+y</sub>Te<sub>3</sub></a>                            | <i>P</i> 2 <sub>1</sub> / <i>m</i> (11)    | <i>P</i> <sub><i>c</i></sub> 2 <sub>1</sub> / <i>c</i> (14.82) | 2/ <i>m</i> 1'                     | ×        | ×   |

Continued on next page

TABLE S7 – continued from previous page

| BCS-ID | Formula                                                         | Parent             | MSG                       | MPG          | SHG type | LMO |
|--------|-----------------------------------------------------------------|--------------------|---------------------------|--------------|----------|-----|
| 1.28   | CrN                                                             | $Fm\bar{3}m$ (225) | $P_{anma}$ (62.450)       | $mmm1'$      | ×        | ×   |
| 1.29   | LaSrFeO <sub>4</sub>                                            | $I4/mmm$ (139)     | $C_{AMca}$ (64.480)       | $mmm1'$      | ×        | ×   |
| 1.30   | BaCo <sub>2</sub> V <sub>2</sub> O <sub>8</sub>                 | $I4_1/acd$ (142)   | $P_{Icca}$ (54.352)       | $mmm1'$      | ×        | ×   |
| 1.31   | MnO                                                             | $Fm\bar{3}m$ (225) | $C_{c2/c}$ (15.90)        | $2/m1'$      | ×        | ×   |
| 1.32   | Lu <sub>2</sub> MnCoO <sub>6</sub>                              | $P2_1/n$ (14)      | $P_{a21}$ (4.10)          | $21'$        | G-wP     | ×   |
| 1.33   | ErAuGe                                                          | $P6_3mc$ (186)     | $P_{Cna21}$ (33.154)      | $mm21'$      | G-woP    | ×   |
| 1.34   | HoAuGe                                                          | $P6_3mc$ (186)     | $P_{Cna21}$ (33.154)      | $mm21'$      | G-woP    | ×   |
| 1.35   | LiErF <sub>4</sub>                                              | $I4_1/a$ (88)      | $P_{C21/c}$ (14.84)       | $2/m1'$      | ×        | ×   |
| 1.36   | Dy <sub>2</sub> BaNiO <sub>5</sub>                              | $Immm$ (71)        | $C_{c2/c}$ (15.90)        | $2/m1'$      | ×        | ×   |
| 1.37   | VOCl                                                            | $Pmmn$ (59)        | $C_{a2/c}$ (15.91)        | $2/m1'$      | ×        | ×   |
| 1.38   | Nd <sub>2</sub> NaOsO <sub>6</sub>                              | $P2_1/n$ (14)      | $P_S\bar{1}$ (2.7)        | $11'$        | ×        | ×   |
| 1.39   | LiFeGe <sub>2</sub> O <sub>6</sub>                              | $P2_1/c$ (14)      | $P_{a21/c}$ (14.80)       | $2/m1'$      | ×        | ×   |
| 1.40   | SrNdFeO <sub>4</sub>                                            | $I4/mmm$ (139)     | $C_{Accm}$ (66.5)         | $mmm1'$      | ×        | ×   |
| 1.41   | SrNdFeO <sub>4</sub>                                            | $I4/mmm$ (139)     | $C_{AMca}$ (64.480)       | $mmm1'$      | ×        | ×   |
| 1.42   | La <sub>2</sub> NiO <sub>4</sub>                                | $Bmcb$ (64)        | $P_{Cmna}$ (53.335)       | $mmm1'$      | ×        | ×   |
| 1.43   | PrNiO <sub>3</sub>                                              | $Pbnm$ (62)        | $C_{amc21}$ (36.178)      | $mm21'$      | G-wP     | ×   |
| 1.44   | NdNiO <sub>3</sub>                                              | $Pbnm$ (62)        | $C_{amc21}$ (36.178)      | $mm21'$      | G-wP     | ×   |
| 1.45   | NdNiO <sub>3</sub>                                              | $Pbnm$ (62)        | $C_{amc21}$ (36.178)      | $mm21'$      | G-wP     | ×   |
| 1.46   | Sr <sub>2</sub> FeOsO <sub>6</sub>                              | $I4/m$ (87)        | $P_{c4/n}$ (85.64)        | $4/m1'$      | ×        | ×   |
| 1.47   | Sr <sub>2</sub> FeOsO <sub>6</sub>                              | $I4/m$ (87)        | $P_{I4/m}$ (83.50)        | $4/m1'$      | ×        | ×   |
| 1.48   | HoNiO <sub>3</sub>                                              | $P2_1/n$ (14)      | $P_{a21}$ (4.10)          | $21'$        | G-wP     | ×   |
| 1.49   | Ag <sub>2</sub> NiO <sub>2</sub>                                | $C2/m$ (12)        | $C_{c2/c}$ (15.90)        | $2/m1'$      | ×        | ×   |
| 1.50   | AgNiO <sub>2</sub>                                              | $P6_322$ (182)     | $P_{B21212}$ (18.22)      | $2221'$      | G-woP    | ×   |
| 1.51   | Cs <sub>2</sub> CoCl <sub>4</sub>                               | $Pnma$ (62)        | $P_{a21}$ (4.10)          | $21'$        | G-wP     | ×   |
| 1.52   | CaFe <sub>2</sub> As <sub>2</sub>                               | $I4/mmm$ (139)     | $C_{AMca}$ (64.480)       | $mmm1'$      | ×        | ×   |
| 1.53   | Er <sub>2</sub> BaNiO <sub>5</sub>                              | $Immm$ (71)        | $C_{c2/c}$ (15.90)        | $2/m1'$      | ×        | ×   |
| 1.54   | GdMn <sub>2</sub> O <sub>5</sub>                                | $Pbam$ (55)        | $P_{aca21}$ (29.104)      | $mm21'$      | G-wP     | ×   |
| 1.55   | Na <sub>2</sub> MnF <sub>5</sub>                                | $P2_1/c$ (14)      | $P_{bc}$ (7.29)           | $m1'$        | G-wP     | ×   |
| 1.56   | Gd <sub>2</sub> Ti <sub>2</sub> O <sub>7</sub>                  | $Fd\bar{3}m$ (227) | $R_{I\bar{3}m}$ (166.102) | $\bar{3}m1'$ | ×        | ×   |
| 1.57   | CuMnO <sub>2</sub>                                              | $C2/m$ (12)        | $P_S\bar{1}$ (2.7)        | $\bar{1}1'$  | ×        | ×   |
| 1.58   | La <sub>2</sub> O <sub>2</sub> Fe <sub>2</sub> OSe <sub>2</sub> | $I4/mmm$ (139)     | $C_{cc}$ (9.40)           | $m1'$        | G-wP     | ×   |
| 1.59   | KTb <sub>3</sub> F <sub>12</sub>                                | $I4/m$ (87)        | $P_{I42/m}$ (84.58)       | $4/m1'$      | ×        | ×   |
| 1.60   | Ca <sub>3</sub> CoO <sub>6</sub>                                | $R\bar{3}c$ (167)  | $P_{C21/c}$ (14.84)       | $2/m1'$      | ×        | ×   |
| 1.61   | MnWO <sub>4</sub>                                               | $P2/c$ (13)        | $C_{a2/c}$ (15.91)        | $2/m1'$      | ×        | ×   |
| 1.62   | CuO                                                             | $C2/c$ (15)        | $P_{a21/c}$ (14.80)       | $2/m1'$      | ×        | ×   |
| 1.63   | MnPb <sub>4</sub> Sb <sub>6</sub> S <sub>14</sub>               | $P2_1/c$ (14)      | $P_{a21/c}$ (14.80)       | $2/m1'$      | ×        | ×   |
| 1.64   | BaNiF <sub>4</sub>                                              | $Cmc2_1$ (36)      | $P_{a21}$ (4.10)          | $21'$        | G-woP    | ×   |
| 1.65   | SrFeO <sub>2</sub>                                              | $P4/mmm$ (123)     | $F_Smmmm$ (69.526)        | $mmm1'$      | ×        | ×   |
| 1.66   | Fe(ND <sub>3</sub> ) <sub>2</sub> PO <sub>4</sub>               | $P2_1/n$ (14)      | $P_S\bar{1}$ (2.7)        | $11'$        | ×        | ×   |
| 1.67   | TmPtIn                                                          | $P62m$ (189)       | $A_bbm2$ (39.201)         | $mm21'$      | G-woP    | ×   |
| 1.68   | NaNdFeWO <sub>6</sub>                                           | $P2_1$ (4)         | $P_S\bar{1}$ (1.3)        | $11'$        | G-woP    | ×   |
| 1.69   | CoO                                                             | $Fm\bar{3}m$ (225) | $C_{c2/c}$ (15.90)        | $2/m1'$      | ×        | ×   |
| 1.70   | CoV <sub>2</sub> O <sub>6</sub>                                 | $C2/m$ (12)        | $C_{c2/c}$ (15.90)        | $2/m1'$      | ×        | ×   |
| 1.71   | SrCo <sub>2</sub> V <sub>2</sub> O <sub>8</sub>                 | $I4_1cd$ (110)     | $P_{Ica21}$ (29.110)      | $mm21'$      | G-woP    | ×   |
| 1.72   | Sr <sub>2</sub> CoOsO <sub>6</sub>                              | $I4/m$ (87)        | $C_{c2/c}$ (15.90)        | $2/m1'$      | ×        | ×   |
| 1.73   | CaV <sub>2</sub> O <sub>4</sub>                                 | $P2_1/n11$ (14)    | $P_{a21/c}$ (14.80)       | $2/m1'$      | ×        | ×   |
| 1.74   | BiMn <sub>2</sub> O <sub>5</sub>                                | $Pbam$ (55)        | $C_{amc21}$ (36.178)      | $mm21'$      | G-wP     | ×   |
| 1.75   | BiMn <sub>2</sub> O <sub>5</sub>                                | $Pbam$ (55)        | $C_{am}$ (8.36)           | $m1'$        | G-wP     | ×   |
| 1.76   | DyMn <sub>2</sub> O <sub>5</sub>                                | $Pbam$ (55)        | $P_{aca21}$ (29.104)      | $mm21'$      | G-wP     | ×   |
| 1.77   | Sr <sub>2</sub> IrO <sub>4</sub>                                | $I4_1/acd$ (142)   | $P_{Icca}$ (54.352)       | $mmm1'$      | ×        | ×   |
| 1.78   | Li <sub>2</sub> MnSiO <sub>4</sub>                              | $P2_1/n$ (14)      | $P_{a21/c}$ (14.80)       | $2/m1'$      | ×        | ×   |
| 1.79   | Li <sub>2</sub> CoSiO <sub>4</sub>                              | $Pna2_1$ (33)      | $C_{ac}$ (9.41)           | $m1'$        | G-woP    | ×   |
| 1.80   | Dy <sub>2</sub> CoGa <sub>8</sub>                               | $P4/mmm$ (123)     | $I_{c4/mcm}$ (140.550)    | $4/mmm1'$    | ×        | ×   |
| 1.81   | GdIn <sub>3</sub>                                               | $Pm\bar{3}m$ (221) | $P_{C4/mbm}$ (127.397)    | $4/mmm1'$    | ×        | ×   |
| 1.82   | Nd <sub>2</sub> RhIn <sub>8</sub>                               | $P4/mmm$ (123)     | $I_{c4/mcm}$ (140.550)    | $4/mmm1'$    | ×        | ×   |
| 1.83   | BaFeO <sub>2.5</sub>                                            | $P2_1/c$ (14)      | $P_{a21/c}$ (14.80)       | $2/m1'$      | ×        | ×   |
| 1.84   | SrFeO <sub>2</sub> F                                            | $Pm\bar{3}m$ (221) | $I_{c4/mcm}$ (140.550)    | $4/mmm1'$    | ×        | ×   |
| 1.85   | alpha-Mn                                                        | $I43m$ (217)       | $P_{I421c}$ (114.282)     | $42m1'$      | G-woP    | ×   |

Continued on next page

TABLE S7 – continued from previous page

| BCS-ID | Formula                                                              | Parent                                     | MSG                                                         | MPG              | SHG type | LMO |
|--------|----------------------------------------------------------------------|--------------------------------------------|-------------------------------------------------------------|------------------|----------|-----|
| 1.86   | GeV <sub>4</sub> S <sub>8</sub>                                      | <i>F</i> 43 <i>m</i> (216)                 | <i>P</i> <sub>6</sub> <i>na</i> 2 <sub>1</sub> (33.149)     | <i>mm</i> 21'    | G-woP    | ×   |
| 1.87   | Tb <sub>2</sub> CoGa <sub>8</sub>                                    | <i>P</i> 4/ <i>mmm</i> (123)               | <i>I</i> <sub>4</sub> 4/ <i>mcm</i> (140.550)               | 4/ <i>mmm</i> 1' | ×        | ×   |
| 1.88   | Mn <sub>5</sub> Si <sub>3</sub>                                      | <i>P</i> 6 <sub>3</sub> / <i>mcm</i> (193) | <i>P</i> <sub>C</sub> <i>bcn</i> (60.431)                   | <i>mmm</i> 1'    | ×        | ×   |
| 1.89   | DyFe <sub>3</sub> (BO <sub>3</sub> ) <sub>4</sub>                    | <i>P</i> 312 <sub>1</sub> (152)            | <i>P</i> <sub>c</sub> 322 <sub>1</sub> (154.44)             | 321'             | G-woP    | ×   |
| 1.90   | YFe <sub>3</sub> (BO <sub>3</sub> ) <sub>4</sub>                     | <i>P</i> 312 <sub>1</sub> (152)            | <i>C</i> <sub>c</sub> 2 (5.16)                              | 21'              | G-woP    | ×   |
| 1.91   | TbFe <sub>3</sub> (BO <sub>3</sub> ) <sub>4</sub>                    | <i>P</i> 312 <sub>1</sub> (152)            | <i>P</i> <sub>c</sub> 322 <sub>1</sub> (154.44)             | 321'             | G-woP    | ×   |
| 1.92   | HoFe <sub>3</sub> (BO <sub>3</sub> ) <sub>4</sub>                    | <i>P</i> 312 <sub>1</sub> (152)            | <i>P</i> <sub>c</sub> 322 <sub>1</sub> (154.44)             | 321'             | G-woP    | ×   |
| 1.93   | HoFe <sub>3</sub> (BO <sub>3</sub> ) <sub>4</sub>                    | <i>P</i> 312 <sub>1</sub> (152)            | <i>P</i> <sub>S</sub> 1 (1.3)                               | 11'              | G-woP    | ×   |
| 1.94   | Ba <sub>3</sub> LaRu <sub>2</sub> O <sub>9</sub>                     | <i>P</i> 6 <sub>3</sub> / <i>mmc</i> (194) | <i>P</i> <sub>C</sub> 2 <sub>1</sub> / <i>c</i> (14.84)     | 2/ <i>m</i> 1'   | ×        | ×   |
| 1.95   | BaNd <sub>2</sub> O <sub>4</sub>                                     | <i>Pnam</i> (62)                           | <i>P</i> <sub>a</sub> 2 <sub>1</sub> / <i>c</i> (14.80)     | 2/ <i>m</i> 1'   | ×        | ×   |
| 1.96   | BaNd <sub>2</sub> O <sub>4</sub>                                     | <i>Pnam</i> (62)                           | <i>P</i> <sub>a</sub> 2 <sub>1</sub> / <i>c</i> (14.80)     | 2/ <i>m</i> 1'   | ×        | ×   |
| 1.97   | Li <sub>2</sub> MnO <sub>3</sub>                                     | <i>C</i> 2/ <i>m</i> (12)                  | <i>C</i> <sub>c</sub> 2/ <i>m</i> (12.63)                   | 2/ <i>m</i> 1'   | ×        | ×   |
| 1.98   | DyFe <sub>4</sub> Ge <sub>2</sub>                                    | <i>P</i> 4 <sub>2</sub> / <i>mnm</i> (136) | <i>P</i> <sub>c</sub> cc2 (27.82)                           | <i>mm</i> 21'    | G-wP     | ×   |
| 1.99   | CsCoCl <sub>3</sub> (D <sub>2</sub> O) <sub>2</sub>                  | <i>Pcca</i> (54)                           | <i>P</i> <sub>b</sub> ccn (56.372)                          | <i>mmm</i> 1'    | ×        | ×   |
| 1.100  | Cu <sub>2</sub> MnSnS <sub>4</sub>                                   | <i>I</i> 42 <i>m</i> (121)                 | <i>C</i> <sub>c</sub> 2 (5.16)                              | 21'              | G-woP    | ×   |
| 1.101  | LuMnO <sub>3</sub>                                                   | <i>Pbnm</i> (62)                           | <i>P</i> <sub>b</sub> mn2 <sub>1</sub> (31.129)             | <i>mm</i> 21'    | G-wP     | ×   |
| 1.102  | U <sub>2</sub> Ni <sub>2</sub> In                                    | <i>P</i> 4/ <i>mbm</i> (127)               | <i>P</i> <sub>c</sub> 4/ <i>mnc</i> (128.408)               | 4/ <i>mmm</i> 1' | ×        | ×   |
| 1.103  | U <sub>2</sub> Rh <sub>2</sub> Sn                                    | <i>P</i> 4/ <i>mbm</i> (127)               | <i>P</i> <sub>c</sub> 4 <sub>2</sub> / <i>mbc</i> (135.492) | 4/ <i>mmm</i> 1' | ×        | ×   |
| 1.104  | Gd <sub>2</sub> CuO <sub>4</sub>                                     | <i>I</i> 4/ <i>mmm</i> (139)               | <i>C</i> <sub>A</sub> ccm (66.5)                            | <i>mmm</i> 1'    | ×        | ×   |
| 1.105  | Gd <sub>2</sub> CuO <sub>4</sub>                                     | <i>Aeam</i> (64)                           | <i>P</i> <sub>A</sub> ccn (56.374)                          | <i>mmm</i> 1'    | ×        | ×   |
| 1.106  | Pr <sub>2</sub> CuO <sub>4</sub>                                     | <i>I</i> 4/ <i>mmm</i> (139)               | <i>C</i> <sub>A</sub> ccm (66.5)                            | <i>mmm</i> 1'    | ×        | ×   |
| 1.107  | Sm <sub>2</sub> CuO <sub>4</sub>                                     | <i>I</i> 4/ <i>mmm</i> (139)               | <i>C</i> <sub>A</sub> mca (64.480)                          | <i>mmm</i> 1'    | ×        | ×   |
| 1.108  | TbMn <sub>2</sub> O <sub>5</sub>                                     | <i>Pbam</i> (55)                           | <i>C</i> <sub>a</sub> m (8.36)                              | <i>m</i> 1'      | G-wP     | ×   |
| 1.109  | HoMn <sub>2</sub> O <sub>5</sub>                                     | <i>Pbam</i> (55)                           | <i>C</i> <sub>a</sub> m (8.36)                              | <i>m</i> 1'      | G-wP     | ×   |
| 1.110  | ScMn <sub>6</sub> Ge <sub>6</sub>                                    | <i>P</i> 6/ <i>mmm</i> (191)               | <i>P</i> <sub>c</sub> 6/ <i>mcc</i> (192.252)               | 6/ <i>mmm</i> 1' | ×        | ×   |
| 1.111  | GdBiPt                                                               | <i>F</i> 43 <i>m</i> (216)                 | <i>C</i> <sub>c</sub> c (9.40)                              | <i>m</i> 1'      | G-woP    | ×   |
| 1.112  | NiTa <sub>2</sub> O <sub>6</sub>                                     | <i>P</i> 4 <sub>2</sub> / <i>mnm</i> (136) | <i>P</i> <sub>c</sub> 2 <sub>1</sub> / <i>c</i> (14.82)     | 2/ <i>m</i> 1'   | ×        | ×   |
| 1.113  | NiSb <sub>2</sub> O <sub>6</sub>                                     | <i>P</i> 4 <sub>2</sub> / <i>mnm</i> (136) | <i>P</i> <sub>S</sub> 1 (2.7)                               | 11'              | ×        | ×   |
| 1.114  | Ca <sub>4</sub> IrO <sub>6</sub>                                     | <i>R</i> 3 <i>c</i> (167)                  | <i>P</i> <sub>C</sub> 2/ <i>c</i> (13.74)                   | 2/ <i>m</i> 1'   | ×        | ×   |
| 1.115  | Dy <sub>3</sub> Ru <sub>4</sub> Al <sub>12</sub>                     | <i>P</i> 6 <sub>3</sub> / <i>mmc</i> (194) | <i>C</i> <sub>c</sub> 2/ <i>c</i> (15.90)                   | 2/ <i>m</i> 1'   | ×        | ×   |
| 1.116  | AgMnVO <sub>4</sub>                                                  | <i>Pnma</i> (62)                           | <i>P</i> <sub>a</sub> 2 <sub>1</sub> / <i>m</i> (11.55)     | 2/ <i>m</i> 1'   | ×        | ×   |
| 1.117  | NaFePO <sub>4</sub>                                                  | <i>Pnma</i> (62)                           | <i>P</i> <sub>c</sub> 2 <sub>1</sub> / <i>c</i> (14.82)     | 2/ <i>m</i> 1'   | ×        | ×   |
| 1.118  | GdPO <sub>4</sub>                                                    | <i>P</i> 2 <sub>1</sub> / <i>n</i> (14)    | <i>P</i> <sub>a</sub> 2 <sub>1</sub> / <i>c</i> (14.80)     | 2/ <i>m</i> 1'   | ×        | ×   |
| 1.119  | LaMn <sub>3</sub> V <sub>4</sub> O <sub>12</sub>                     | <i>Im</i> 3̄ (204)                         | <i>R</i> <sub>I</sub> 3̄ (148.20)                           | 31'              | ×        | ×   |
| 1.120  | BaFe <sub>2</sub> Se <sub>3</sub>                                    | <i>Pnma</i> (62)                           | <i>C</i> <sub>a</sub> c (9.41)                              | <i>m</i> 1'      | G-wP     | ×   |
| 1.121  | NaFeSO <sub>4</sub> F                                                | <i>C</i> 2/ <i>c</i> (15)                  | <i>P</i> <sub>C</sub> 2/ <i>c</i> (13.74)                   | 2/ <i>m</i> 1'   | ×        | ×   |
| 1.122  | Cu <sub>3</sub> Bi(SeO <sub>3</sub> ) <sub>2</sub> O <sub>2</sub> Br | <i>Pmmn</i> (59)                           | <i>P</i> <sub>c</sub> ccn (56.373)                          | <i>mmm</i> 1'    | ×        | ×   |
| 1.123  | Cu <sub>3</sub> Y(SeO <sub>3</sub> ) <sub>2</sub> O <sub>2</sub> Cl  | <i>Pmmn</i> (59)                           | <i>P</i> <sub>c</sub> ccn (56.373)                          | <i>mmm</i> 1'    | ×        | ×   |
| 1.124  | YBaFe <sub>4</sub> O <sub>7</sub>                                    | <i>P</i> 2 <sub>1</sub> (4)                | <i>P</i> <sub>a</sub> 2 <sub>1</sub> (4.10)                 | 21'              | G-woP    | ×   |
| 1.125  | LaFeAsO                                                              | <i>Cmme</i> (67)                           | <i>I</i> <sub>c</sub> bca (73.553)                          | <i>mmm</i> 1'    | ×        | ×   |
| 1.126  | NaCoSO <sub>4</sub> F                                                | <i>C</i> 2/ <i>c</i> (15)                  | <i>P</i> <sub>C</sub> 2/ <i>c</i> (13.74)                   | 2/ <i>m</i> 1'   | ×        | ×   |
| 1.127  | BiNiO(PO <sub>4</sub> )                                              | <i>P</i> 2 <sub>1</sub> / <i>n</i> (14)    | <i>P</i> <sub>a</sub> 2 <sub>1</sub> / <i>c</i> (14.80)     | 2/ <i>m</i> 1'   | ×        | ×   |
| 1.128  | BiCoO(PO <sub>4</sub> )                                              | <i>P</i> 2 <sub>1</sub> / <i>n</i> (14)    | <i>P</i> <sub>a</sub> 2 <sub>1</sub> / <i>c</i> (14.80)     | 2/ <i>m</i> 1'   | ×        | ×   |
| 1.129  | AgFe <sub>3</sub> (SO <sub>4</sub> ) <sub>2</sub> (OD) <sub>4</sub>  | <i>R</i> 3 <i>m</i> (166)                  | <i>R</i> <sub>I</sub> 3 <i>c</i> (167.108)                  | 3 <i>m</i> 1'    | ×        | ×   |
| 1.130  | Cr <sub>2</sub> As                                                   | <i>P</i> 4/ <i>nmm</i> (129)               | <i>P</i> <sub>a</sub> <i>nma</i> (62.450)                   | <i>mmm</i> 1'    | ×        | ×   |
| 1.131  | Fe <sub>2</sub> As                                                   | <i>P</i> 4/ <i>nmm</i> (129)               | <i>P</i> <sub>a</sub> <i>nma</i> (62.450)                   | <i>mmm</i> 1'    | ×        | ×   |
| 1.132  | Mn <sub>2</sub> As                                                   | <i>P</i> 4/ <i>nmm</i> (129)               | <i>P</i> <sub>a</sub> <i>nma</i> (62.450)                   | <i>mmm</i> 1'    | ×        | ×   |
| 1.133  | CuSb <sub>2</sub> O <sub>6</sub>                                     | <i>P</i> 2 <sub>1</sub> / <i>n</i> (14)    | <i>P</i> <sub>a</sub> 2 <sub>1</sub> / <i>c</i> (14.80)     | 2/ <i>m</i> 1'   | ×        | ×   |
| 1.134  | Co <sub>2</sub> C10O <sub>8</sub> H <sub>2</sub>                     | <i>C</i> 2/ <i>m</i> (12)                  | <i>P</i> <sub>C</sub> 2 <sub>1</sub> / <i>m</i> (11.57)     | 2/ <i>m</i> 1'   | ×        | ×   |
| 1.135  | C <sub>8</sub> H10C <sub>2</sub> O <sub>11</sub>                     | <i>P</i> 1 (2)                             | <i>P</i> <sub>S</sub> 1 (2.7)                               | 11'              | ×        | ×   |
| 1.136  | AgCrS <sub>2</sub>                                                   | <i>R</i> 3 <i>m</i> (160)                  | <i>C</i> <sub>c</sub> m (8.35)                              | <i>m</i> 1'      | G-woP    | ×   |
| 1.137  | Sr <sub>2</sub> CaIrO <sub>6</sub>                                   | <i>P</i> 2 <sub>1</sub> / <i>n</i> (14)    | <i>P</i> <sub>S</sub> 1 (2.7)                               | 11'              | ×        | ×   |
| 1.138  | MgV <sub>2</sub> O <sub>4</sub>                                      | <i>I</i> 4 <i>m</i> 2 (119)                | <i>C</i> <sub>A</sub> 222 <sub>1</sub> (20.37)              | 2221'            | G-woP    | ×   |
| 1.139  | Ho <sub>2</sub> RhIn <sub>8</sub>                                    | <i>P</i> 4/ <i>mmm</i> (123)               | <i>P</i> <sub>c</sub> ccm (49.273)                          | <i>mmm</i> 1'    | ×        | ×   |
| 1.140  | PrMgPb                                                               | <i>I</i> 4/ <i>mmm</i> (139)               | <i>P</i> <sub>A</sub> 2/ <i>c</i> (13.73)                   | 2/ <i>m</i> 1'   | ×        | ×   |
| 1.141  | NdMgPb                                                               | <i>I</i> 4/ <i>mmm</i> (139)               | <i>P</i> <sub>A</sub> 2/ <i>c</i> (13.73)                   | 2/ <i>m</i> 1'   | ×        | ×   |
| 1.142  | CeMgPb                                                               | <i>I</i> 4/ <i>mmm</i> (139)               | <i>C</i> <sub>A</sub> mma (67.510)                          | <i>mmm</i> 1'    | ×        | ×   |
| 1.143  | Mn <sub>3</sub> Pt                                                   | <i>Pm</i> 3̄ <i>m</i> (221)                | <i>P</i> <sub>c</sub> 4 <sub>2</sub> / <i>mcm</i> (132.456) | 4/ <i>mmm</i> 1' | ×        | ×   |

Continued on next page

TABLE S7 – continued from previous page

| BCS-ID | Formula                                                          | Parent             | MSG                      | MPG       | SHG type | LMO |
|--------|------------------------------------------------------------------|--------------------|--------------------------|-----------|----------|-----|
| 1.144  | $\text{NH}_4\text{FeCl}_2(\text{HCOO})$                          | $C2/c$ (15)        | $P_C2_1/c$ (14.84)       | $2/m1'$   | ×        | ×   |
| 1.145  | $\text{Mn}_3\text{Ni}_2\text{OP}_6$                              | $Fm\bar{3}m$ (225) | $C_{AM}ca$ (64.480)      | $mmm1'$   | ×        | ×   |
| 1.146  | $\text{LaCrAsO}$                                                 | $P4/nmm$ (129)     | $P_c4_2/ncm$ (138.528)   | $4/mmm1'$ | ×        | ×   |
| 1.147  | $\text{Li}_2\text{Fe}(\text{SO}_4)_2$                            | $P2_1/c$ (14)      | $P_a2_1/c$ (14.80)       | $2/m1'$   | ×        | ×   |
| 1.148  | $\text{CeOs}_{1.84}\text{Ir}_{0.16}\text{Al}_{10}$               | $Cmcm$ (63)        | $P_{AN}ma$ (62.453)      | $mmm1'$   | ×        | ×   |
| 1.149  | $\text{La}_{0.8}\text{Bi}_{0.2}\text{Mn}_2\text{O}_5$            | $Pbam$ (55)        | $P_{cbam}$ (55.361)      | $mmm1'$   | ×        | ×   |
| 1.150  | $\text{PrAg}$                                                    | $Pm\bar{3}m$ (221) | $P_{BM}na$ (53.334)      | $mmm1'$   | ×        | ×   |
| 1.151  | $\text{Mn}_{0.375}\text{Co}_{0.375}\text{Fe}_{0.25}$             | $Fm\bar{3}m$ (225) | $P_A2_1/c$ (14.83)       | $2/m1'$   | ×        | ×   |
| 1.152  | $\text{Ce}_3\text{NiIn}$                                         | $Pm\bar{3}m$ (221) | $P_C4b2$ (117.305)       | $42m1'$   | G-wP     | ×   |
| 1.153  | $\text{Mn}_3\text{GaC}$                                          | $Pm\bar{3}m$ (221) | $R_I\bar{3}c$ (167.108)  | $3m1'$    | ×        | ×   |
| 1.154  | $\text{NaFeSi}_2\text{O}_6$                                      | $C2/c$ (15)        | $P_C2_1/c$ (14.84)       | $2/m1'$   | ×        | ×   |
| 1.155  | $\text{LiFeSO}_4\text{F}$                                        | $P1$ (2)           | $P_S\bar{1}$ (2.7)       | $11'$     | ×        | ×   |
| 1.156  | $\text{LaMn}_3\text{Cr}_4\text{O}_{12}$                          | $Im\bar{3}$ (204)  | $R_I\bar{3}$ (146.12)    | $31'$     | G-wP     | ×   |
| 1.157  | $\text{FeF}_3(\text{H}_2\text{O})_2\text{H}_2\text{O}$           | $P4/n$ (85)        | $P_b2_1/c$ (14.81)       | $2/m1'$   | ×        | ×   |
| 1.158  | $\text{YMn}_3\text{Al}_4\text{O}_{12}$                           | $Im\bar{3}$ (204)  | $P_{Innm}$ (58.404)      | $mmm1'$   | ×        | ×   |
| 1.159  | $\text{Li}_2\text{Ni}(\text{WO}_4)_2$                            | $P1$ (2)           | $P_S\bar{1}$ (2.7)       | $11'$     | ×        | ×   |
| 1.160  | $\text{UP}$                                                      | $Fm\bar{3}m$ (225) | $P_{I4/mnc}$ (128.410)   | $4/mmm1'$ | ×        | ×   |
| 1.161  | $\text{PrFe}_3(\text{BO}_3)_4$                                   | $R32$ (155)        | $R_I32$ (155.48)         | $321'$    | G-woP    | ×   |
| 1.162  | $\text{NdMg}$                                                    | $Pm\bar{3}m$ (221) | $P_c4/mcc$ (124.360)     | $4/mmm1'$ | ×        | ×   |
| 1.163  | $\text{TmPdIn}$                                                  | $P\bar{6}2m$ (189) | $P_c\bar{6}$ (174.136)   | $61'$     | G-woP    | ×   |
| 1.164  | $\text{Co}_3\text{TeO}_6$                                        | $C2/c$ (15)        | $P_S\bar{1}$ (2.7)       | $11'$     | ×        | ×   |
| 1.165  | $\text{Ni}_3\text{TeO}_6$                                        | $R3$ (146)         | $R_I\bar{3}$ (146.12)    | $31'$     | G-woP    | ×   |
| 1.166  | $\text{La}_2\text{LiOsO}_6$                                      | $P2_1/n$ (14)      | $P_S\bar{1}$ (2.7)       | $11'$     | ×        | ×   |
| 1.167  | $\text{NiS}_2$                                                   | $Pa\bar{3}$ (205)  | $P_S\bar{1}$ (2.7)       | $11'$     | ×        | ×   |
| 1.168  | $\text{Sr}_2\text{CuTeO}_6$                                      | $I4/m$ (87)        | $C_c2/c$ (15.90)         | $2/m1'$   | ×        | ×   |
| 1.169  | $\text{CaCoGe}_2\text{O}_6$                                      | $C2/c$ (15)        | $P_C2_1/c$ (14.84)       | $2/m1'$   | ×        | ×   |
| 1.170  | $\text{Tm}_5\text{Ni}_2\text{In}_4$                              | $Pbam$ (55)        | $C_a m$ (8.36)           | $m1'$     | G-wP     | ×   |
| 1.171  | $\text{Tb}_2\text{Fe}_2\text{Si}_2\text{C}$                      | $C2/m$ (12)        | $C_c2/m$ (12.63)         | $2/m1'$   | ×        | ×   |
| 1.172  | $\text{NiTa}_2\text{O}_6$                                        | $P4_2/mnm$ (136)   | $A_bba2$ (41.217)        | $mm21'$   | G-wP     | ×   |
| 1.173  | $\text{La}_{0.375}\text{Ca}_{0.625}\text{MnO}_5$                 | $Pnma$ (62)        | $P_bmc2_1$ (26.72)       | $mm21'$   | G-wP     | ×   |
| 1.174  | $\text{La}_{0.333}\text{Ca}_{0.667}\text{MnO}_5$                 | $Pnma$ (62)        | $P_bmc2_1$ (26.72)       | $mm21'$   | G-wP     | ×   |
| 1.175  | $\text{La}_{0.333}\text{Ca}_{0.667}\text{MnO}_5$                 | $Pbnm$ (62)        | $P_bmn2_1$ (31.129)      | $mm21'$   | G-wP     | ×   |
| 1.176  | $\text{YbCo}_2\text{Si}_2$                                       | $I4/mmm$ (139)     | $I_c bca$ (73.553)       | $mmm1'$   | ×        | ×   |
| 1.177  | $\text{Sr}_2\text{CuWO}_6$                                       | $I4/m$ (87)        | $P_S\bar{1}$ (2.7)       | $11'$     | ×        | ×   |
| 1.178  | $\text{Cu}_{1.07}\text{Mn}_{0.93}\text{O}_2$                     | $C2/m$ (12)        | $P_S\bar{1}$ (2.7)       | $11'$     | ×        | ×   |
| 1.179  | $\text{NdCoAsO}$                                                 | $P4/nmm$ (129)     | $P_a nma$ (62.450)       | $mmm1'$   | ×        | ×   |
| 1.180  | $\text{Na}_3\text{Co}_2\text{SbO}_6$                             | $C2/m$ (12)        | $P_S\bar{1}$ (2.7)       | $11'$     | ×        | ×   |
| 1.181  | $\text{Ba}_3\text{Fe}_3\text{O}_7\text{F}$                       | $P2_1/m$ (11)      | $P_a2_1/m$ (11.55)       | $2/m1'$   | ×        | ×   |
| 1.182  | $\text{TlMnO}_3$                                                 | $Pm\bar{3}m$ (221) | $P_S\bar{1}$ (2.7)       | $11'$     | ×        | ×   |
| 1.183  | $\text{FePS}_3$                                                  | $C2/m$ (12)        | $C_c2/m$ (12.63)         | $2/m1'$   | ×        | ×   |
| 1.184  | $\text{Na}_2\text{Co}_2\text{TeO}_6$                             | $P6_322$ (182)     | $P_C2_12_12_1$ (19.29)   | $2221'$   | G-woP    | ×   |
| 1.185  | $\text{GeCu}_2\text{O}_4$                                        | $I4_1/amd$ (141)   | $I_c42d$ (122.338)       | $42m1'$   | G-wP     | ×   |
| 1.186  | $\text{SrRu}_2\text{O}_6$                                        | $P31m$ (162)       | $P_c31m$ (162.78)        | $3m1'$    | ×        | ×   |
| 1.187  | $\text{TbRh}_2\text{Si}_2$                                       | $I4/mmm$ (139)     | $P_{I4/mnc}$ (128.410)   | $4/mmm1'$ | ×        | ×   |
| 1.188  | $\text{CeRh}_2\text{Si}_2$                                       | $I4/mmm$ (139)     | $C_{AM}ca$ (64.480)      | $mmm1'$   | ×        | ×   |
| 1.189  | $\text{TbMg}_3$                                                  | $Fm\bar{3}m$ (225) | $R_I\bar{3}c$ (167.108)  | $3m1'$    | ×        | ×   |
| 1.190  | $\text{YCr}(\text{BO}_3)_2$                                      | $R3$ (148)         | $P_S\bar{1}$ (2.7)       | $11'$     | ×        | ×   |
| 1.191  | $\text{HoCr}(\text{BO}_3)_2$                                     | $R3$ (148)         | $P_S\bar{1}$ (2.7)       | $11'$     | ×        | ×   |
| 1.192  | $\text{SmMn}_2\text{O}_5$                                        | $Pbam$ (55)        | $P_bmc2_1$ (26.72)       | $mm21'$   | G-wP     | ×   |
| 1.193  | $\text{CrTe}_3$                                                  | $P2_1/c$ (14)      | $P_S\bar{1}$ (2.7)       | $11'$     | ×        | ×   |
| 1.194  | $\text{NiWO}_4$                                                  | $P2/c$ (13)        | $P_a2/c$ (13.70)         | $2/m1'$   | ×        | ×   |
| 1.195  | $\text{Er}_2\text{Ni}_2\text{In}$                                | $Cmmm$ (65)        | $C_a mcm$ (63.467)       | $mmm1'$   | ×        | ×   |
| 1.196  | $\text{MnV}_2\text{O}_6$                                         | $Pbcn$ (60)        | $P_a2_1/c$ (14.80)       | $2/m1'$   | ×        | ×   |
| 1.197  | $\text{Fe}_4\text{Si}_2\text{Sn}_7\text{O}_{16}$                 | $P3m1$ (164)       | $C_c2/m$ (12.63)         | $2/m1'$   | ×        | ×   |
| 1.198  | $\text{Ni}_{1.64}\text{Co}_{0.36}\text{Mn}_{1.28}\text{O}_{7.2}$ | $C4/mmm$ (139)     | $P_{I4_2/mnm}$ (136.506) | $4/mmm1'$ | ×        | ×   |
| 1.199  | $\text{Sc}_2\text{NiMnO}_6$                                      | $P2_1/c$ (14)      | $P_a2_1/c$ (14.80)       | $2/m1'$   | ×        | ×   |
| 1.200  | $\text{U}_2\text{Ni}_2\text{Sn}$                                 | $P4/mbm$ (127)     | $C_c mcm$ (63.466)       | $mmm1'$   | ×        | ×   |

Continued on next page

TABLE S7 – continued from previous page

| BCS-ID | Formula                                                | Parent                                        | MSG                                                         | MPG              | SHG type | LMO |
|--------|--------------------------------------------------------|-----------------------------------------------|-------------------------------------------------------------|------------------|----------|-----|
| 1.201  | Cr <sub>2</sub> ReO <sub>6</sub>                       | <i>P</i> 4 <sub>2</sub> / <i>mnm</i> (136)    | <i>P</i> <sub>a</sub> 2 <sub>1</sub> / <i>c</i> (14.80)     | 2/ <i>m</i> 1'   | ×        | ×   |
| 1.202  | CrReO <sub>4</sub>                                     | <i>C</i> 2/ <i>m</i> (12)                     | <i>C</i> <sub>c</sub> 2/ <i>c</i> (15.90)                   | 2/ <i>m</i> 1'   | ×        | ×   |
| 1.203  | Ni <sub>2</sub> SiO <sub>4</sub>                       | <i>Pnma</i> (62)                              | <i>P</i> <sub>c</sub> 2 <sub>1</sub> / <i>c</i> (14.82)     | 2/ <i>m</i> 1'   | ×        | ×   |
| 1.204  | Ni <sub>2</sub> SiO <sub>4</sub>                       | <i>Pnma</i> (62)                              | <i>P</i> <sub>c</sub> 2 <sub>1</sub> / <i>c</i> (14.82)     | 2/ <i>m</i> 1'   | ×        | ×   |
| 1.205  | Dy <sub>2</sub> Fe <sub>2</sub> Si <sub>2</sub> C      | <i>C</i> 2/ <i>m</i> (12)                     | <i>C</i> <sub>c</sub> 2/ <i>m</i> (12.63)                   | 2/ <i>m</i> 1'   | ×        | ×   |
| 1.206  | Dy <sub>2</sub> Fe <sub>2</sub> Si <sub>2</sub> C      | <i>C</i> 2/ <i>m</i> (12)                     | <i>P</i> <sub>S</sub> 1̄ (2.7)                              | 11'              | ×        | ×   |
| 1.207  | U <sub>2</sub> Rh <sub>2</sub> Sn                      | <i>P</i> 4/ <i>mbm</i> (127)                  | <i>P</i> <sub>c</sub> 4 <sub>2</sub> / <i>mbc</i> (135.492) | 4/ <i>mmm</i> 1' | ×        | ×   |
| 1.208  | UAs                                                    | <i>Fm</i> 3̄ <i>m</i> (225)                   | <i>P</i> <sub>1</sub> 4/ <i>mnc</i> (128.410)               | 4/ <i>mmm</i> 1' | ×        | ×   |
| 1.209  | FeI <sub>2</sub>                                       | <i>P</i> 3̄ <i>m</i> 1 (164)                  | <i>C</i> <sub>c</sub> 2/ <i>c</i> (15.90)                   | 2/ <i>m</i> 1'   | ×        | ×   |
| 1.210  | FePSe <sub>3</sub>                                     | <i>R</i> 3̄ (148)                             | <i>P</i> <sub>S</sub> 1̄ (2.7)                              | 11'              | ×        | ×   |
| 1.211  | Dy <sub>2</sub> O <sub>2</sub> S                       | <i>P</i> 3̄ <i>m</i> 1 (164)                  | <i>C</i> <sub>c</sub> 2/ <i>c</i> (15.90)                   | 2/ <i>m</i> 1'   | ×        | ×   |
| 1.212  | Dy <sub>2</sub> O <sub>2</sub> Se                      | <i>P</i> 3̄ <i>m</i> 1 (164)                  | <i>C</i> <sub>c</sub> 2/ <i>c</i> (15.90)                   | 2/ <i>m</i> 1'   | ×        | ×   |
| 1.213  | Ho <sub>2</sub> O <sub>2</sub> Se                      | <i>P</i> 3̄ <i>m</i> 1 (164)                  | <i>P</i> <sub>A</sub> 2/ <i>c</i> (13.73)                   | 2/ <i>m</i> 1'   | ×        | ×   |
| 1.214  | Yb <sub>2</sub> O <sub>2</sub> Se                      | <i>P</i> 3̄ <i>m</i> 1 (164)                  | <i>C</i> <sub>c</sub> 2/ <i>c</i> (15.90)                   | 2/ <i>m</i> 1'   | ×        | ×   |
| 1.215  | UP <sub>2</sub>                                        | <i>P</i> 4/ <i>nmm</i> (129)                  | <i>P</i> <sub>c</sub> 4/ <i>ncc</i> (130.432)               | 4/ <i>mmm</i> 1' | ×        | ×   |
| 1.216  | Nd <sub>2</sub> BaNiO <sub>5</sub>                     | <i>Immm</i> (71)                              | <i>C</i> <sub>c</sub> 2/ <i>c</i> (15.90)                   | 2/ <i>m</i> 1'   | ×        | ×   |
| 1.217  | Tb <sub>2</sub> BaNiO <sub>5</sub>                     | <i>Immm</i> (71)                              | <i>C</i> <sub>c</sub> 2/ <i>c</i> (15.90)                   | 2/ <i>m</i> 1'   | ×        | ×   |
| 1.218  | Tm <sub>2</sub> BaNiO <sub>5</sub>                     | <i>Immm</i> (71)                              | <i>P</i> <sub>S</sub> 1̄ (2.7)                              | 11'              | ×        | ×   |
| 1.219  | CuF <sub>2</sub>                                       | <i>P</i> 2 <sub>1</sub> / <i>c</i> (14)       | <i>P</i> <sub>S</sub> 1̄ (2.7)                              | 11'              | ×        | ×   |
| 1.220  | YBa <sub>2</sub> Fe <sub>3</sub> O <sub>8.08</sub>     | <i>P</i> 4/ <i>mmm</i> (123)                  | <i>I</i> <sub>b</sub> <i>m</i> <i>m</i> <i>a</i> (74.562)   | <i>mmm</i> 1'    | ×        | ×   |
| 1.221  | YBa <sub>2</sub> Fe <sub>3</sub> O <sub>7.84</sub>     | <i>Pmmm</i> (47)                              | <i>C</i> <sub>a</sub> 2/ <i>m</i> (12.64)                   | 2/ <i>m</i> 1'   | ×        | ×   |
| 1.222  | Er <sub>2</sub> CoGa <sub>8</sub>                      | <i>P</i> 4/ <i>mmm</i> (123)                  | <i>P</i> <sub>a</sub> <i>m</i> <i>m</i> <i>a</i> (51.298)   | <i>mmm</i> 1'    | ×        | ×   |
| 1.223  | Tm <sub>2</sub> CoGa <sub>8</sub>                      | <i>P</i> 4/ <i>mmm</i> (123)                  | <i>C</i> <sub>a</sub> <i>m</i> <i>m</i> <i>m</i> (65.489)   | <i>mmm</i> 1'    | ×        | ×   |
| 1.224  | CoNb <sub>2</sub> O <sub>6</sub>                       | <i>Pbcn</i> (60)                              | <i>P</i> <sub>c</sub> 2 <sub>1</sub> 2 <sub>1</sub> (19.28) | 2221'            | G-wP     | ×   |
| 1.225  | ScMn <sub>6</sub> Ge <sub>6</sub>                      | <i>P</i> 6/ <i>mmm</i> (191)                  | <i>P</i> <sub>c</sub> 6/ <i>mcc</i> (192.252)               | 6/ <i>mmm</i> 1' | ×        | ×   |
| 1.226  | CeCo <sub>2</sub> Ge <sub>4</sub> O <sub>12</sub>      | <i>P</i> 4/ <i>nbm</i> (125)                  | <i>P</i> <sub>b</sub> <i>n</i> <i>n</i> <i>a</i> (52.315)   | <i>mmm</i> 1'    | ×        | ×   |
| 1.227  | Ca <sub>2</sub> Cr <sub>2</sub> O <sub>5</sub>         | <i>I</i> 2 <i>mb</i> (46)                     | <i>P</i> <sub>C</sub> 2 <sub>1</sub> (4.12)                 | 21'              | G-woP    | ×   |
| 1.228  | RuCl <sub>3</sub>                                      | <i>C</i> 2/ <i>m</i> (12)                     | <i>P</i> <sub>C</sub> 2/ <i>m</i> (10.49)                   | 2/ <i>m</i> 1'   | ×        | ×   |
| 1.229  | BaMoP <sub>2</sub> O <sub>8</sub>                      | <i>C</i> 2/ <i>m</i> (12)                     | <i>P</i> <sub>S</sub> 1̄ (2.7)                              | 11'              | ×        | ×   |
| 1.230  | NiPS <sub>3</sub>                                      | <i>C</i> 2/ <i>m</i> (12)                     | <i>P</i> <sub>C</sub> 2 <sub>1</sub> / <i>m</i> (11.57)     | 2/ <i>m</i> 1'   | ×        | ×   |
| 1.231  | NiPS <sub>3</sub>                                      | <i>C</i> 2/ <i>m</i> (12)                     | <i>P</i> <sub>S</sub> 1̄ (1.3)                              | 11'              | G-wP     | ×   |
| 1.232  | CuMnSb                                                 | <i>F</i> 43 <i>m</i> (216)                    | <i>C</i> <sub>cc</sub> (9.40)                               | <i>m</i> 1'      | G-woP    | ×   |
| 1.233  | CuMnSb                                                 | <i>F</i> 43 <i>m</i> (216)                    | <i>R</i> <sub>I</sub> 3 <i>c</i> (161.72)                   | 3 <i>m</i> 1'    | G-woP    | ×   |
| 1.234  | Ca <sub>2</sub> Sr <sub>2</sub> IrO <sub>6</sub>       | <i>R</i> 3̄ (148)                             | <i>P</i> <sub>S</sub> 1̄ (2.7)                              | 11'              | ×        | ×   |
| 1.235  | Ba(TiO)Cu <sub>4</sub> (PO <sub>4</sub> ) <sub>2</sub> | <i>P</i> 4 <sub>2</sub> 2 <sub>1</sub> 2 (90) | <i>P</i> <sub>c</sub> 422 <sub>1</sub> 2 (94.132)           | 4221'            | G-woP    | ×   |
| 1.236  | ErFeCuGe <sub>4</sub> O <sub>12</sub>                  | <i>P</i> 4/ <i>nbm</i> (125)                  | <i>P</i> <sub>c</sub> 4/ <i>nnc</i> (126.384)               | 4/ <i>mmm</i> 1' | ×        | ×   |
| 1.237  | VCl <sub>2</sub>                                       | <i>P</i> 3̄ <i>m</i> 1 (164)                  | <i>P</i> <sub>c</sub> 31 <i>c</i> (159.64)                  | 3 <i>m</i> 1'    | G-wP     | ×   |
| 1.238  | VBr <sub>2</sub>                                       | <i>P</i> 3̄ <i>m</i> 1 (164)                  | <i>P</i> <sub>c</sub> 31 <i>c</i> (159.64)                  | 3 <i>m</i> 1'    | G-wP     | ×   |
| 1.239  | MnBr <sub>2</sub>                                      | <i>P</i> 3̄ <i>m</i> 1 (164)                  | <i>C</i> <sub>c</sub> 2/ <i>m</i> (12.63)                   | 2/ <i>m</i> 1'   | ×        | ×   |
| 1.240  | FeI <sub>2</sub>                                       | <i>P</i> 3̄ <i>m</i> 1 (164)                  | <i>P</i> <sub>S</sub> 1̄ (2.7)                              | 11'              | ×        | ×   |
| 1.241  | FeCl <sub>2</sub>                                      | <i>R</i> 3̄ <i>m</i> (166)                    | <i>R</i> <sub>I</sub> 3 <i>c</i> (167.108)                  | 3 <i>m</i> 1'    | ×        | ×   |
| 1.242  | FeBr <sub>2</sub>                                      | <i>P</i> 3̄ <i>m</i> 1 (164)                  | <i>P</i> <sub>c</sub> 3 <i>c</i> 1 (165.96)                 | 3 <i>m</i> 1'    | ×        | ×   |
| 1.243  | Sr <sub>2</sub> CoOsO <sub>6</sub>                     | <i>I</i> 2/ <i>m</i> (12)                     | <i>P</i> <sub>S</sub> 1̄ (2.7)                              | 11'              | ×        | ×   |
| 1.244  | CrCl <sub>3</sub>                                      | <i>R</i> 3̄ (148)                             | <i>P</i> <sub>S</sub> 1̄ (2.7)                              | 11'              | ×        | ×   |
| 1.245  | CoBr <sub>2</sub>                                      | <i>P</i> 3̄ <i>m</i> 1 (164)                  | <i>C</i> <sub>c</sub> 2/ <i>c</i> (15.90)                   | 2/ <i>m</i> 1'   | ×        | ×   |
| 1.246  | CoCl <sub>2</sub>                                      | <i>R</i> 3̄ <i>m</i> (166)                    | <i>C</i> <sub>c</sub> 2/ <i>c</i> (15.90)                   | 2/ <i>m</i> 1'   | ×        | ×   |
| 1.247  | NiCl <sub>2</sub>                                      | <i>R</i> 3̄ <i>m</i> (166)                    | <i>C</i> <sub>c</sub> 2/ <i>c</i> (15.90)                   | 2/ <i>m</i> 1'   | ×        | ×   |
| 1.248  | NiBr <sub>2</sub>                                      | <i>R</i> 3̄ <i>m</i> (166)                    | <i>C</i> <sub>c</sub> 2/ <i>c</i> (15.90)                   | 2/ <i>m</i> 1'   | ×        | ×   |
| 1.249  | K <sub>2</sub> NiF <sub>4</sub>                        | <i>I</i> 4/ <i>mmm</i> (139)                  | <i>C</i> <sub>A</sub> <i>m</i> <i>c</i> <i>a</i> (64.480)   | <i>mmm</i> 1'    | ×        | ×   |
| 1.250  | KNiF <sub>3</sub>                                      | <i>Pm</i> 3̄ <i>m</i> (221)                   | <i>I</i> <sub>c</sub> 4/ <i>mcm</i> (140.550)               | 4/ <i>mmm</i> 1' | ×        | ×   |
| 1.251  | NdCo <sub>2</sub> P <sub>2</sub>                       | <i>I</i> 4/ <i>mmm</i> (139)                  | <i>P</i> <sub>c</sub> 4/ <i>mcc</i> (124.360)               | 4/ <i>mmm</i> 1' | ×        | ×   |
| 1.252  | CaCo <sub>2</sub> P <sub>2</sub>                       | <i>I</i> 4/ <i>mmm</i> (139)                  | <i>P</i> <sub>I</sub> <i>m</i> <i>m</i> <i>n</i> (59.416)   | <i>mmm</i> 1'    | ×        | ×   |
| 1.253  | CeCo <sub>2</sub> P <sub>2</sub>                       | <i>I</i> 4/ <i>mmm</i> (139)                  | <i>P</i> <sub>I</sub> 4/ <i>nnc</i> (126.386)               | 4/ <i>mmm</i> 1' | ×        | ×   |
| 1.254  | UNiGa <sub>5</sub>                                     | <i>P</i> 4/ <i>mmm</i> (123)                  | <i>I</i> <sub>c</sub> 4/ <i>mcm</i> (140.550)               | 4/ <i>mmm</i> 1' | ×        | ×   |
| 1.255  | UPtGa <sub>5</sub>                                     | <i>P</i> 4/ <i>mmm</i> (123)                  | <i>P</i> <sub>c</sub> 4/ <i>mcc</i> (124.360)               | 4/ <i>mmm</i> 1' | ×        | ×   |
| 1.256  | BaNi <sub>2</sub> V <sub>2</sub> O <sub>8</sub>        | <i>R</i> 3̄ (148)                             | <i>P</i> <sub>S</sub> 1̄ (2.7)                              | 11'              | ×        | ×   |
| 1.257  | BaNi <sub>2</sub> As <sub>2</sub> O <sub>8</sub>       | <i>R</i> 3̄ (148)                             | <i>P</i> <sub>S</sub> 1̄ (2.7)                              | 11'              | ×        | ×   |

Continued on next page

TABLE S7 – continued from previous page

| BCS-ID | Formula                                                                                | Parent                                     | MSG                                                     | MPG              | SHG type | LMO |
|--------|----------------------------------------------------------------------------------------|--------------------------------------------|---------------------------------------------------------|------------------|----------|-----|
| 1.258  | <a href="#">Cu<sub>3</sub>Co<sub>2</sub>SbO<sub>6</sub></a>                            | <i>C</i> 2/ <i>c</i> (15)                  | <i>P</i> <sub>C</sub> 2 <sub>1</sub> / <i>c</i> (14.84) | 2/ <i>m</i> 1'   | ×        | ×   |
| 1.259  | <a href="#">Cu<sub>3</sub>Ni<sub>2</sub>SbO<sub>6</sub></a>                            | <i>C</i> 2/ <i>c</i> (15)                  | <i>P</i> <sub>C</sub> 2/ <i>c</i> (13.74)               | 2/ <i>m</i> 1'   | ×        | ×   |
| 1.260  | <a href="#">NaMnGe<sub>2</sub>O<sub>6</sub></a>                                        | <i>C</i> 2/ <i>c</i> (15)                  | <i>P</i> <sub>S</sub> 1 (2.7)                           | 11'              | ×        | ×   |
| 1.261  | <a href="#">NpRhGa<sub>5</sub></a>                                                     | <i>P</i> 4/ <i>mmm</i> (123)               | <i>P</i> <sub>c</sub> 4/ <i>mcc</i> (124.360)           | 4/ <i>mmm</i> 1' | ×        | ×   |
| 1.262  | <a href="#">NpRhGa<sub>5</sub></a>                                                     | <i>P</i> 4/ <i>mmm</i> (123)               | <i>C</i> <sub>c</sub> <i>mcm</i> (63.466)               | <i>mmm</i> 1'    | ×        | ×   |
| 1.263  | <a href="#">Ca<sub>3</sub>Ru<sub>2</sub>O<sub>7</sub></a>                              | <i>Bb</i> 2 <sub>1</sub> <i>m</i> (36)     | <i>P</i> <sub>C</sub> <i>na</i> 2 <sub>1</sub> (33.154) | <i>mm</i> 21'    | G-woP    | ×   |
| 1.264  | <a href="#">CoPS<sub>3</sub></a>                                                       | <i>C</i> 2/ <i>m</i> (12)                  | <i>P</i> <sub>C</sub> 2 <sub>1</sub> / <i>m</i> (11.57) | 2/ <i>m</i> 1'   | ×        | ×   |
| 1.265  | <a href="#">CuMnSb</a>                                                                 | <i>F</i> 43 <i>m</i> (216)                 | <i>R</i> <sub>I</sub> 3 <i>c</i> (161.72)               | 3 <i>m</i> 1'    | G-woP    | ×   |
| 1.266  | <a href="#">SmFe<sub>3</sub>(BO<sub>3</sub>)<sub>4</sub></a>                           | <i>R</i> 32 (155)                          | <i>P</i> <sub>S</sub> 1 (1.3)                           | 11'              | G-woP    | ×   |
| 1.267  | <a href="#">Dy<sub>2</sub>Co<sub>3</sub>Al<sub>9</sub></a>                             | <i>C</i> <i>mcm</i> (63)                   | <i>A</i> <sub>a</sub> <i>mm</i> 2 (38.192)              | <i>mm</i> 21'    | G-wP     | ×   |
| 1.268  | <a href="#">Fe<sub>0.48</sub>TiSe<sub>2</sub></a>                                      | <i>I</i> 2/ <i>m</i> (12)                  | <i>C</i> <sub>c</sub> 2/ <i>c</i> (15.90)               | 2/ <i>m</i> 1'   | ×        | ×   |
| 1.269  | <a href="#">Fe<sub>0.48</sub>TiSe<sub>2</sub></a>                                      | <i>I</i> 2/ <i>m</i> (12)                  | <i>C</i> <sub>c</sub> 2/ <i>c</i> (15.90)               | 2/ <i>m</i> 1'   | ×        | ×   |
| 1.270  | <a href="#">Fe<sub>0.25</sub>TiSe<sub>2</sub></a>                                      | <i>F</i> 2/ <i>m</i> (12)                  | <i>C</i> <sub>c</sub> 2/ <i>c</i> (15.90)               | 2/ <i>m</i> 1'   | ×        | ×   |
| 1.271  | <a href="#">CeSbTe</a>                                                                 | <i>P</i> 4/ <i>nmm</i> (129)               | <i>P</i> <sub>c</sub> 4/ <i>ncc</i> (130.432)           | 4/ <i>mmm</i> 1' | ×        | ×   |
| 1.272  | <a href="#">CeNiAsO</a>                                                                | <i>P</i> 4/ <i>nmm</i> (129)               | <i>P</i> <sub>a</sub> 2 <sub>1</sub> (4.10)             | 21'              | G-wP     | ×   |
| 1.273  | <a href="#">Pr<sub>0.5</sub>Sr<sub>0.5</sub>MnO<sub>3</sub></a>                        | <i>I</i> 4/ <i>mcm</i> (140)               | <i>C</i> <sub>AM</sub> <i>mcm</i> (63.468)              | <i>mmm</i> 1'    | ×        | ×   |
| 1.274  | <a href="#">DyFeWO<sub>6</sub></a>                                                     | <i>P</i> <i>na</i> 2 <sub>1</sub> (33)     | <i>C</i> <sub>a</sub> <i>c</i> (9.41)                   | <i>m</i> 1'      | G-woP    | ×   |
| 1.275  | <a href="#">Ba<sub>6</sub>Co<sub>6</sub>ClO<sub>15.5</sub></a>                         | <i>P</i> 6 <i>m</i> 2 (187)                | <i>P</i> <sub>c</sub> 6 <i>c</i> 2 (188.220)            | 6 <i>m</i> 21'   | G-woP    | ×   |
| 1.276  | <a href="#">Na<sub>0.5</sub>Li<sub>0.5</sub>FeGe<sub>2</sub>O<sub>6</sub></a>          | <i>P</i> 2 <sub>1</sub> / <i>c</i> (14)    | <i>P</i> <sub>a</sub> 2 <sub>1</sub> / <i>c</i> (14.80) | 2/ <i>m</i> 1'   | ×        | ×   |
| 1.277  | <a href="#">LiFeCr<sub>4</sub>O<sub>8</sub></a>                                        | <i>F</i> 43 <i>m</i> (216)                 | <i>I</i> 4 <i>m</i> '2' (119.319)                       | 42' <i>m</i> '   | BW-woP   | ✓   |
| 1.278  | <a href="#">Cu(NCS)<sub>2</sub></a>                                                    | <i>P</i> 1 (2)                             | <i>P</i> <sub>S</sub> 1 (2.7)                           | 11'              | ×        | ×   |
| 1.279  | <a href="#">Ho<sub>2</sub>Cu<sub>2</sub>O<sub>5</sub></a>                              | <i>P</i> <i>na</i> 2 <sub>1</sub> (33)     | <i>P</i> <sub>a</sub> 2 <sub>1</sub> (4.10)             | 21'              | G-woP    | ×   |
| 1.280  | <a href="#">Yb<sub>2</sub>Cu<sub>2</sub>O<sub>5</sub></a>                              | <i>P</i> <i>na</i> 2 <sub>1</sub> (33)     | <i>P</i> <sub>a</sub> <i>c</i> (7.27)                   | <i>m</i> 1'      | G-woP    | ×   |
| 1.281  | <a href="#">YBaCuFeO<sub>5</sub></a>                                                   | <i>P</i> 4 <i>mm</i> (99)                  | <i>F</i> <sub>S</sub> <i>mm</i> 2 (42.223)              | <i>mm</i> 21'    | G-woP    | ×   |
| 1.282  | <a href="#">YBaCuFeO<sub>5</sub></a>                                                   | <i>P</i> 4/ <i>mmm</i> (123)               | <i>C</i> <sub>a</sub> 2/ <i>m</i> (12.64)               | 2/ <i>m</i> 1'   | ×        | ×   |
| 1.283  | <a href="#">YBaCuFeO<sub>5</sub></a>                                                   | <i>P</i> 4/ <i>mmm</i> (123)               | <i>C</i> <sub>a</sub> 2/ <i>m</i> (12.64)               | 2/ <i>m</i> 1'   | ×        | ×   |
| 1.284  | <a href="#">YBaCuFeO<sub>5</sub></a>                                                   | <i>P</i> 4/ <i>mmm</i> (123)               | <i>C</i> <sub>a</sub> 2/ <i>m</i> (12.64)               | 2/ <i>m</i> 1'   | ×        | ×   |
| 1.285  | <a href="#">YBaCuFeO<sub>5</sub></a>                                                   | <i>P</i> 4/ <i>mmm</i> (123)               | <i>F</i> <sub>S</sub> <i>mmm</i> (69.526)               | <i>mmm</i> 1'    | ×        | ×   |
| 1.286  | <a href="#">Fe<sub>2</sub>(C<sub>2</sub>O<sub>4</sub>)<sub>3.4</sub>H<sub>2</sub>O</a> | <i>P</i> 1 (2)                             | <i>P</i> <sub>S</sub> 1 (2.7)                           | 11'              | ×        | ×   |
| 1.287  | <a href="#">V<sub>2</sub>O<sub>3</sub></a>                                             | <i>I</i> 2/ <i>a</i> (15)                  | <i>P</i> <sub>C</sub> 2 <sub>1</sub> / <i>c</i> (14.84) | 2/ <i>m</i> 1'   | ×        | ×   |
| 1.288  | <a href="#">CePd<sub>2</sub>Si<sub>2</sub></a>                                         | <i>I</i> 4/ <i>mmm</i> (139)               | <i>C</i> <sub>AC</sub> <i>m</i> (66.5)                  | <i>mmm</i> 1'    | ×        | ×   |
| 1.289  | <a href="#">CePd<sub>2</sub>Ge<sub>2</sub></a>                                         | <i>I</i> 4/ <i>mmm</i> (139)               | <i>C</i> <sub>AC</sub> <i>m</i> (66.5)                  | <i>mmm</i> 1'    | ×        | ×   |
| 1.290  | <a href="#">CeRh<sub>2</sub>Si<sub>2</sub></a>                                         | <i>I</i> 4/ <i>mmm</i> (139)               | <i>C</i> <sub>AM</sub> <i>ca</i> (64.480)               | <i>mmm</i> 1'    | ×        | ×   |
| 1.291  | <a href="#">CeAu<sub>2</sub>Si<sub>2</sub></a>                                         | <i>I</i> 4/ <i>mmm</i> (139)               | <i>P</i> <sub>I</sub> 4/ <i>mnc</i> (128.410)           | 4/ <i>mmm</i> 1' | ×        | ×   |
| 1.292  | <a href="#">HoNi<sub>2</sub>B<sub>2</sub>C</a>                                         | <i>I</i> 4/ <i>mmm</i> (139)               | <i>C</i> <sub>AM</sub> <i>ca</i> (64.480)               | <i>mmm</i> 1'    | ×        | ×   |
| 1.293  | <a href="#">NdNi<sub>2</sub>B<sub>2</sub>C</a>                                         | <i>I</i> 4/ <i>mmm</i> (139)               | <i>C</i> <sub>c</sub> 2/ <i>c</i> (15.90)               | 2/ <i>m</i> 1'   | ×        | ×   |
| 1.294  | <a href="#">HoNi<sub>2</sub>B<sub>2</sub>C</a>                                         | <i>I</i> 4/ <i>mmm</i> (139)               | <i>C</i> <sub>AM</sub> <i>ca</i> (64.480)               | <i>mmm</i> 1'    | ×        | ×   |
| 1.295  | <a href="#">DyNi<sub>2</sub>B<sub>2</sub>C</a>                                         | <i>I</i> 4/ <i>mmm</i> (139)               | <i>C</i> <sub>AM</sub> <i>ca</i> (64.480)               | <i>mmm</i> 1'    | ×        | ×   |
| 1.296  | <a href="#">PrNi<sub>2</sub>B<sub>2</sub>C</a>                                         | <i>I</i> 4/ <i>mmm</i> (139)               | <i>C</i> <sub>AM</sub> <i>ca</i> (64.480)               | <i>mmm</i> 1'    | ×        | ×   |
| 1.297  | <a href="#">CuFe<sub>2</sub>(P<sub>2</sub>O<sub>7</sub>)<sub>2</sub></a>               | <i>P</i> 2 <sub>1</sub> / <i>n</i> (14)    | <i>P</i> <sub>a</sub> 2 <sub>1</sub> / <i>c</i> (14.80) | 2/ <i>m</i> 1'   | ×        | ×   |
| 1.298  | <a href="#">BaCdVO(PO<sub>4</sub>)<sub>2</sub></a>                                     | <i>P</i> <i>bca</i> (61)                   | <i>P</i> <sub>b</sub> <i>na</i> 2 <sub>1</sub> (33.150) | <i>mm</i> 21'    | G-wP     | ×   |
| 1.299  | <a href="#">GdMn<sub>2</sub>O<sub>5</sub></a>                                          | <i>P</i> <i>bam</i> (55)                   | <i>P</i> <sub>a</sub> <i>ca</i> 2 <sub>1</sub> (29.104) | <i>mm</i> 21'    | G-wP     | ×   |
| 1.300  | <a href="#">GdMn<sub>2</sub>O<sub>5</sub></a>                                          | <i>P</i> <i>bam</i> (55)                   | <i>P</i> <sub>a</sub> <i>ca</i> 2 <sub>1</sub> (29.104) | <i>mm</i> 21'    | G-wP     | ×   |
| 1.301  | <a href="#">BiMnTeO<sub>6</sub></a>                                                    | <i>P</i> 2 <sub>1</sub> / <i>c</i> (14)    | <i>P</i> <sub>a</sub> 2 <sub>1</sub> / <i>c</i> (14.80) | 2/ <i>m</i> 1'   | ×        | ×   |
| 1.302  | <a href="#">Ba<sub>2</sub>CoO<sub>4</sub></a>                                          | <i>P</i> 2 <sub>1</sub> / <i>n</i> (14)    | <i>P</i> <sub>a</sub> 2 <sub>1</sub> / <i>c</i> (14.80) | 2/ <i>m</i> 1'   | ×        | ×   |
| 1.303  | <a href="#">Dy<sub>3</sub>Ru<sub>4</sub>Al<sub>12</sub></a>                            | <i>P</i> 6 <sub>3</sub> / <i>mmc</i> (194) | <i>C</i> <sub>c</sub> 2/ <i>c</i> (15.90)               | 2/ <i>m</i> 1'   | ×        | ×   |
| 1.304  | <a href="#">ZnMnO<sub>3</sub></a>                                                      | <i>R</i> 3 (148)                           | <i>P</i> <sub>S</sub> 1 (2.7)                           | 11'              | ×        | ×   |
| 1.305  | <a href="#">Mn<sub>5</sub>Si<sub>3</sub></a>                                           | <i>P</i> 6 <sub>3</sub> / <i>mcm</i> (193) | <i>P</i> <sub>C</sub> <i>bcn</i> (60.431)               | <i>mmm</i> 1'    | ×        | ×   |
| 1.306  | <a href="#">Na<sub>2</sub>BaMn(VO<sub>4</sub>)<sub>2</sub></a>                         | <i>C</i> 2/ <i>c</i> (15)                  | <i>P</i> <sub>C</sub> 2 <sub>1</sub> / <i>c</i> (14.84) | 2/ <i>m</i> 1'   | ×        | ×   |
| 1.307  | <a href="#">Mn<sub>5</sub>Si<sub>3</sub></a>                                           | <i>P</i> 6 <sub>3</sub> / <i>mcm</i> (193) | <i>P</i> <sub>S</sub> 1 (1.3)                           | 11'              | G-wP     | ×   |
| 1.308  | <a href="#">MnBi<sub>2</sub>Te<sub>4</sub></a>                                         | <i>R</i> 3 <i>m</i> (166)                  | <i>R</i> <sub>I</sub> 3 <i>c</i> (167.108)              | 3 <i>m</i> 1'    | ×        | ×   |
| 1.309  | <a href="#">MnBi<sub>2</sub>Te<sub>4</sub></a>                                         | <i>R</i> 3 <i>m</i> (166)                  | <i>R</i> <sub>I</sub> 3 <i>c</i> (167.108)              | 3 <i>m</i> 1'    | ×        | ×   |
| 1.310  | <a href="#">MnBi<sub>4</sub>Te<sub>7</sub></a>                                         | <i>P</i> 3 <i>m</i> 1 (164)                | <i>P</i> <sub>c</sub> 3 <i>c</i> 1 (165.96)             | 3 <i>m</i> 1'    | ×        | ×   |
| 1.311  | <a href="#">BaMo(PO<sub>4</sub>)<sub>2</sub></a>                                       | <i>C</i> 2/ <i>m</i> (12)                  | <i>P</i> <sub>S</sub> 1 (2.7)                           | 11'              | ×        | ×   |
| 1.312  | <a href="#">HoNi<sub>2</sub>B<sub>2</sub>C</a>                                         | <i>I</i> 4/ <i>mmm</i> (139)               | <i>C</i> <sub>AM</sub> <i>ca</i> (64.480)               | <i>mmm</i> 1'    | ×        | ×   |
| 1.313  | <a href="#">GdFeZnGe<sub>4</sub>O<sub>12</sub></a>                                     | <i>P</i> 4/ <i>nbm</i> (125)               | <i>P</i> <sub>b</sub> <i>nna</i> (52.315)               | <i>mmm</i> 1'    | ×        | ×   |
| 1.314  | <a href="#">NaFeSi<sub>2</sub>O<sub>6</sub></a>                                        | <i>C</i> 2/ <i>c</i> (15)                  | <i>P</i> <sub>C</sub> 2 <sub>1</sub> / <i>c</i> (14.84) | 2/ <i>m</i> 1'   | ×        | ×   |

Continued on next page

TABLE S7 – continued from previous page

| BCS-ID | Formula                                                                                    | Parent                        | MSG                                                     | MPG            | SHG type | LMO |
|--------|--------------------------------------------------------------------------------------------|-------------------------------|---------------------------------------------------------|----------------|----------|-----|
| 1.315  | <a href="#">Mn<sub>0.8</sub>ICu<sub>0.19</sub>WO<sub>4</sub></a>                           | <i>P2/c</i> (13)              | <i>P<sub>a</sub>2/c</i> (13.70)                         | <i>2/m1'</i>   | ×        | ×   |
| 1.316  | <a href="#">La<sub>0.25</sub>Pr<sub>0.75</sub>Co<sub>2</sub>P<sub>2</sub></a>              | <i>I4/mmm</i> (139)           | <i>P<sub>c</sub>4/mcc</i> (124.360)                     | <i>4/mmm1'</i> | ×        | ×   |
| 1.317  | <a href="#">La<sub>0.25</sub>Pr<sub>0.75</sub>Co<sub>2</sub>P<sub>2</sub></a>              | <i>I4/mmm</i> (139)           | <i>C<sub>c</sub>2/c</i> (15.90)                         | <i>2/m1'</i>   | ×        | ×   |
| 1.318  | <a href="#">Sr<sub>2</sub>Ru<sub>0.95</sub>Fe<sub>0.05</sub>O<sub>4</sub></a>              | <i>I4/mmm</i> (139)           | <i>C<sub>c</sub>mca</i> (64.478)                        | <i>mmm1'</i>   | ×        | ×   |
| 1.319  | <a href="#">Sr<sub>2</sub>Ru<sub>0.95</sub>Fe<sub>0.05</sub>O<sub>4</sub></a>              | <i>I4/mmm</i> (139)           | <i>C<sub>c</sub>mcm</i> (63.466)                        | <i>mmm1'</i>   | ×        | ×   |
| 1.320  | <a href="#">Sr<sub>2</sub>FeWO<sub>6</sub></a>                                             | <i>P2<sub>1</sub>/n</i> (14)  | <i>P<sub>S</sub>1</i> (2.7)                             | <i>11'</i>     | ×        | ×   |
| 1.321  | <a href="#">Ba<sub>2</sub>FeWO<sub>6</sub></a>                                             | <i>I4/m</i> (87)              | <i>P<sub>S</sub>1</i> (2.7)                             | <i>11'</i>     | ×        | ×   |
| 1.322  | <a href="#">Sr<sub>2</sub>FeWO<sub>5</sub>N</a>                                            | <i>I4/m</i> (87)              | <i>P<sub>S</sub>1</i> (2.7)                             | <i>11'</i>     | ×        | ×   |
| 1.323  | <a href="#">CoGeO<sub>3</sub></a>                                                          | <i>C2/c</i> (15)              | <i>P<sub>C</sub>2<sub>1</sub>/c</i> (14.84)             | <i>2/m1'</i>   | ×        | ×   |
| 1.324  | <a href="#">DyMn<sub>2</sub>O<sub>5</sub></a>                                              | <i>Pbam</i> (55)              | <i>P<sub>a</sub>ca2<sub>1</sub></i> (29.104)            | <i>mm21'</i>   | G-wP     | ×   |
| 1.325  | <a href="#">PrMn<sub>2</sub>O<sub>5</sub></a>                                              | <i>Pbam</i> (55)              | <i>P<sub>c</sub>c</i> (7.28)                            | <i>m1'</i>     | G-wP     | ×   |
| 1.326  | <a href="#">PrMn<sub>2</sub>O<sub>5</sub></a>                                              | <i>Pbam</i> (55)              | <i>P<sub>b</sub>nma</i> (62.451)                        | <i>mmm1'</i>   | ×        | ×   |
| 1.327  | <a href="#">LaMn<sub>2</sub>O<sub>5</sub></a>                                              | <i>Pbam</i> (55)              | <i>P<sub>b</sub>bam</i> (55.361)                        | <i>mmm1'</i>   | ×        | ×   |
| 1.328  | <a href="#">Yb<sub>2</sub>CoMnO<sub>6</sub></a>                                            | <i>P2<sub>1</sub>/c</i> (14)  | <i>P<sub>a</sub>2<sub>1</sub></i> (4.10)                | <i>21'</i>     | G-wP     | ×   |
| 1.329  | <a href="#">YbLuCoMnO<sub>6</sub></a>                                                      | <i>P2<sub>1</sub>/c</i> (14)  | <i>P<sub>a</sub>2<sub>1</sub></i> (4.10)                | <i>21'</i>     | G-wP     | ×   |
| 1.330  | <a href="#">Lu<sub>2</sub>CoMnO<sub>6</sub></a>                                            | <i>P2<sub>1</sub>/c</i> (14)  | <i>P<sub>a</sub>2<sub>1</sub></i> (4.10)                | <i>21'</i>     | G-wP     | ×   |
| 1.331  | <a href="#">Li<sub>0.3</sub>INa<sub>0.69</sub>FeGe<sub>2</sub>O<sub>6</sub></a>            | <i>P2<sub>1</sub>/c</i> (14)  | <i>P<sub>a</sub>2<sub>1</sub>/c</i> (14.80)             | <i>2/m1'</i>   | ×        | ×   |
| 1.332  | <a href="#">Li<sub>0.22</sub>Na<sub>0.78</sub>FeGe<sub>2</sub>O<sub>6</sub></a>            | <i>C2/c</i> (15)              | <i>P<sub>C</sub>2<sub>1</sub>/c</i> (14.84)             | <i>2/m1'</i>   | ×        | ×   |
| 1.333  | <a href="#">Yb<sub>2</sub>Pd<sub>2</sub>(In<sub>0.4</sub>Sn<sub>0.6</sub>)<sub>2</sub></a> | <i>P4/mbm</i> (127)           | <i>P<sub>c</sub>4/mbm</i> (127.396)                     | <i>4/mmm1'</i> | ×        | ×   |
| 1.334  | <a href="#">Pr<sub>2</sub>Pd<sub>2</sub>In</a>                                             | <i>P4/mbm</i> (127)           | <i>P<sub>b</sub>nma</i> (62.451)                        | <i>mmm1'</i>   | ×        | ×   |
| 1.335  | <a href="#">Nd<sub>2</sub>Pd<sub>2</sub>In</a>                                             | <i>P4/mbm</i> (127)           | <i>P<sub>c</sub>mc2<sub>1</sub></i> (26.73)             | <i>mm21'</i>   | G-wP     | ×   |
| 1.336  | <a href="#">Tb<sub>2</sub>Pd<sub>2</sub>.05Sn<sub>0.95</sub></a>                           | <i>P4/mbm</i> (127)           | <i>P<sub>b</sub>nma</i> (62.451)                        | <i>mmm1'</i>   | ×        | ×   |
| 1.337  | <a href="#">U<sub>2</sub>Pd<sub>2.35</sub>Sn<sub>0.65</sub></a>                            | <i>P4/mbm</i> (127)           | <i>P<sub>c</sub>4/mnc</i> (128.408)                     | <i>4/mmm1'</i> | ×        | ×   |
| 1.338  | <a href="#">U<sub>2</sub>Ni<sub>2</sub>In</a>                                              | <i>P4/mbm</i> (127)           | <i>P<sub>c</sub>4/mnc</i> (128.408)                     | <i>4/mmm1'</i> | ×        | ×   |
| 1.339  | <a href="#">EuAs<sub>3</sub></a>                                                           | <i>C2/m</i> (12)              | <i>C<sub>c</sub>2/m</i> (12.63)                         | <i>2/m1'</i>   | ×        | ×   |
| 1.340  | <a href="#">LuMnO<sub>3</sub></a>                                                          | <i>Pbnm</i> (62)              | <i>P<sub>b</sub>mn2<sub>1</sub></i> (31.129)            | <i>mm21'</i>   | G-wP     | ×   |
| 1.341  | <a href="#">TmMnO<sub>3</sub></a>                                                          | <i>Pnma</i> (62)              | <i>P<sub>b</sub>mn2<sub>1</sub></i> (31.129)            | <i>mm21'</i>   | G-wP     | ×   |
| 1.342  | <a href="#">Co<sub>3</sub>(PO<sub>4</sub>)<sub>2</sub></a>                                 | <i>P2<sub>1</sub>/c</i> (14)  | <i>P<sub>a</sub>2<sub>1</sub>/c</i> (14.80)             | <i>2/m1'</i>   | ×        | ×   |
| 1.343  | <a href="#">Ba<sub>2</sub>Co<sub>9</sub>O<sub>14</sub></a>                                 | <i>R3m</i> (166)              | <i>C<sub>c</sub>2/c</i> (15.90)                         | <i>2/m1'</i>   | ×        | ×   |
| 1.344  | <a href="#">Ba<sub>2</sub>Co<sub>9</sub>O<sub>14</sub></a>                                 | <i>R3m</i> (166)              | <i>C<sub>c</sub>2/m</i> (12.63)                         | <i>2/m1'</i>   | ×        | ×   |
| 1.345  | <a href="#">NaMnF<sub>4</sub></a>                                                          | <i>P2<sub>1</sub>/c</i> (14)  | <i>P<sub>a</sub>2<sub>1</sub>/c</i> (14.80)             | <i>2/m1'</i>   | ×        | ×   |
| 1.346  | <a href="#">TiMnF<sub>4</sub></a>                                                          | <i>I2/a</i> (15)              | <i>P<sub>C</sub>2/c</i> (13.74)                         | <i>2/m1'</i>   | ×        | ×   |
| 1.347  | <a href="#">CuFeO<sub>2</sub></a>                                                          | <i>R3m</i> (166)              | <i>C<sub>a</sub>2/c</i> (15.91)                         | <i>2/m1'</i>   | ×        | ×   |
| 1.348  | <a href="#">CuFeO<sub>2</sub></a>                                                          | <i>R3m</i> (166)              | <i>C<sub>c</sub>2/c</i> (15.90)                         | <i>2/m1'</i>   | ×        | ×   |
| 1.349  | <a href="#">CoNb<sub>3</sub>S<sub>6</sub></a>                                              | <i>P6<sub>3</sub>22</i> (182) | <i>P<sub>B</sub>2<sub>1</sub>2<sub>1</sub>2</i> (18.22) | <i>2221'</i>   | G-woP    | ×   |
| 1.350  | <a href="#">Nd<sub>2</sub>BaCoO<sub>5</sub></a>                                            | <i>Immm</i> (71)              | <i>C<sub>c</sub>2/c</i> (15.90)                         | <i>2/m1'</i>   | ×        | ×   |
| 1.351  | <a href="#">Ba<sub>2</sub>Co<sub>2</sub>F<sub>7</sub>Cl</a>                                | <i>P2<sub>1</sub>/m</i> (11)  | <i>P<sub>a</sub>2<sub>1</sub>/m</i> (11.55)             | <i>2/m1'</i>   | ×        | ×   |
| 1.352  | <a href="#">Ba<sub>2</sub>Ni<sub>2</sub>F<sub>7</sub>Cl</a>                                | <i>P2<sub>1</sub>/m</i> (11)  | <i>P<sub>c</sub>2<sub>1</sub>/c</i> (14.82)             | <i>2/m1'</i>   | ×        | ×   |
| 1.353  | <a href="#">SmNiO<sub>3</sub></a>                                                          | <i>Pnma</i> (62)              | <i>C<sub>a</sub>mc2<sub>1</sub></i> (36.178)            | <i>mm21'</i>   | G-wP     | ×   |
| 1.354  | <a href="#">EuNiO<sub>3</sub></a>                                                          | <i>Pnma</i> (62)              | <i>C<sub>a</sub>mc2<sub>1</sub></i> (36.178)            | <i>mm21'</i>   | G-wP     | ×   |
| 1.355  | <a href="#">DyGe<sub>3</sub></a>                                                           | <i>Cmcm</i> (63)              | <i>P<sub>a</sub>2<sub>1</sub>/m</i> (11.55)             | <i>2/m1'</i>   | ×        | ×   |
| 1.356  | <a href="#">Ho<sub>3</sub>Ge<sub>4</sub></a>                                               | <i>Cmcm</i> (63)              | <i>P<sub>B</sub>nna</i> (52.318)                        | <i>mmm1'</i>   | ×        | ×   |
| 1.357  | <a href="#">Ho<sub>3</sub>Ge<sub>4</sub></a>                                               | <i>Cmcm</i> (63)              | <i>P<sub>c</sub>2<sub>1</sub>/c</i> (14.82)             | <i>2/m1'</i>   | ×        | ×   |
| 1.358  | <a href="#">HoGe<sub>1.5</sub></a>                                                         | <i>P6/mmm</i> (191)           | <i>C<sub>c</sub>mcm</i> (63.466)                        | <i>mmm1'</i>   | ×        | ×   |
| 1.359  | <a href="#">Dy<sub>3</sub>Ge<sub>4</sub></a>                                               | <i>Cmcm</i> (63)              | <i>P<sub>a</sub>2<sub>1</sub>/m</i> (11.55)             | <i>2/m1'</i>   | ×        | ×   |
| 1.360  | <a href="#">DyGe<sub>1.3</sub></a>                                                         | <i>P6/mmm</i> (191)           | <i>C<sub>c</sub>mcm</i> (63.466)                        | <i>mmm1'</i>   | ×        | ×   |
| 1.361  | <a href="#">DyGe</a>                                                                       | <i>Cmcm</i> (63)              | <i>C<sub>c</sub>2/c</i> (15.90)                         | <i>2/m1'</i>   | ×        | ×   |
| 1.362  | <a href="#">Er<sub>3</sub>Ge<sub>4</sub></a>                                               | <i>Cmcm</i> (63)              | <i>P<sub>C</sub>bcm</i> (57.391)                        | <i>mmm1'</i>   | ×        | ×   |
| 1.363  | <a href="#">TbCu<sub>2</sub>Si<sub>2</sub></a>                                             | <i>I4/mmm</i> (139)           | <i>P<sub>S</sub>1</i> (2.7)                             | <i>11'</i>     | ×        | ×   |
| 1.364  | <a href="#">HoCu<sub>2</sub>Si<sub>2</sub></a>                                             | <i>I4/mmm</i> (139)           | <i>P<sub>S</sub>1</i> (2.7)                             | <i>11'</i>     | ×        | ×   |
| 1.365  | <a href="#">TbCu<sub>2</sub>Si<sub>2</sub></a>                                             | <i>I4/mmm</i> (139)           | <i>P<sub>S</sub>1</i> (2.7)                             | <i>11'</i>     | ×        | ×   |
| 1.366  | <a href="#">HoCu<sub>2</sub>Si<sub>2</sub></a>                                             | <i>I4/mmm</i> (139)           | <i>C<sub>c</sub>2/m</i> (12.63)                         | <i>2/m1'</i>   | ×        | ×   |
| 1.367  | <a href="#">Pu<sub>2</sub>O<sub>3</sub></a>                                                | <i>P3m1</i> (164)             | <i>C<sub>c</sub>2/c</i> (15.90)                         | <i>2/m1'</i>   | ×        | ×   |
| 1.368  | <a href="#">Tb<sub>2</sub>Ni<sub>3</sub>Si<sub>5</sub></a>                                 | <i>Ibam</i> (72)              | <i>P<sub>i</sub>bam</i> (55.364)                        | <i>mmm1'</i>   | ×        | ×   |
| 1.369  | <a href="#">HFe<sub>2</sub>Ge<sub>2</sub></a>                                              | <i>I4/mmm</i> (139)           | <i>C<sub>AM</sub>ca</i> (64.480)                        | <i>mmm1'</i>   | ×        | ×   |
| 1.370  | <a href="#">Li<sub>2</sub>CuO<sub>2</sub></a>                                              | <i>Immm</i> (71)              | <i>P<sub>I</sub>nnm</i> (58.404)                        | <i>mmm1'</i>   | ×        | ×   |
| 1.371  | <a href="#">Nd<sub>2</sub>NiO<sub>4</sub></a>                                              | <i>Cmce</i> (64)              | <i>P<sub>C</sub>mna</i> (53.335)                        | <i>mmm1'</i>   | ×        | ×   |
| 1.372  | <a href="#">Sr<sub>2</sub>MnO<sub>2</sub>Ag<sub>1.5</sub>Se<sub>2</sub></a>                | <i>I4/mmm</i> (139)           | <i>P<sub>I</sub>4/mnc</i> (128.410)                     | <i>4/mmm1'</i> | ×        | ×   |

Continued on next page

TABLE S7 – continued from previous page

| BCS-ID | Formula                                                                     | Parent                          | MSG                                                      | MPG             | SHG type | LMO |
|--------|-----------------------------------------------------------------------------|---------------------------------|----------------------------------------------------------|-----------------|----------|-----|
| 1.373  | <a href="#">Li<sub>3</sub>Ni<sub>2</sub>SbO<sub>6</sub></a>                 | <i>C2/m</i> (12)                | <i>P<sub>S</sub>1</i> (2.7)                              | 11'             | ×        | ×   |
| 1.374  | <a href="#">HoNiGe</a>                                                      | <i>Pnma</i> (62)                | <i>P<sub>c</sub>c</i> (7.28)                             | <i>m1'</i>      | G-wP     | ×   |
| 1.375  | <a href="#">CeScGe</a>                                                      | <i>I4/mmm</i> (139)             | <i>P<sub>S</sub>1</i> (2.7)                              | 11'             | ×        | ×   |
| 1.376  | <a href="#">CeScGe</a>                                                      | <i>I4/mmm</i> (139)             | <i>C<sub>Amcm</sub></i> (63.468)                         | <i>mmm1'</i>    | ×        | ×   |
| 1.377  | <a href="#">CeScSi</a>                                                      | <i>I4/mmm</i> (139)             | <i>P<sub>S</sub>1</i> (2.7)                              | 11'             | ×        | ×   |
| 1.378  | <a href="#">CeScSi</a>                                                      | <i>I4/mmm</i> (139)             | <i>C<sub>Amcm</sub></i> (63.468)                         | <i>mmm1'</i>    | ×        | ×   |
| 1.379  | <a href="#">ErNiGe</a>                                                      | <i>Pnma</i> (62)                | <i>P<sub>a</sub>2<sub>1</sub>/c</i> (14.80)              | 2/ <i>m1'</i>   | ×        | ×   |
| 1.380  | <a href="#">Sr<sub>2</sub>FeO<sub>3</sub>Cl</a>                             | <i>P4/nmm</i> (129)             | <i>P<sub>C</sub>4<sub>2</sub>1<sub>m</sub></i> (113.273) | 42 <i>m1'</i>   | G-wP     | ×   |
| 1.381  | <a href="#">Sr<sub>2</sub>FeO<sub>3</sub>Br</a>                             | <i>P4/nmm</i> (129)             | <i>P<sub>C</sub>4<sub>2</sub>1<sub>m</sub></i> (113.273) | 42 <i>m1'</i>   | G-wP     | ×   |
| 1.382  | <a href="#">Ca<sub>2</sub>FeO<sub>3</sub>Cl</a>                             | <i>P4/nmm</i> (129)             | <i>P<sub>C</sub>4<sub>2</sub>1<sub>m</sub></i> (113.273) | 42 <i>m1'</i>   | G-wP     | ×   |
| 1.383  | <a href="#">Ca<sub>2</sub>FeO<sub>3</sub>Br</a>                             | <i>P4/nmm</i> (129)             | <i>P<sub>C</sub>4<sub>2</sub>1<sub>m</sub></i> (113.273) | 42 <i>m1'</i>   | G-wP     | ×   |
| 1.384  | <a href="#">USb<sub>2</sub></a>                                             | <i>P4/nmm</i> (129)             | <i>P<sub>c</sub>4/ncc</i> (130.432)                      | 4/ <i>mmm1'</i> | ×        | ×   |
| 1.385  | <a href="#">Sr<sub>2</sub>FeO<sub>3</sub>F</a>                              | <i>P4/nmm</i> (129)             | <i>P<sub>C</sub>4<sub>2</sub>1<sub>m</sub></i> (113.273) | 42 <i>m1'</i>   | G-wP     | ×   |
| 1.386  | <a href="#">Sr<sub>2</sub>FeO<sub>3</sub>F</a>                              | <i>P4/nmm</i> (129)             | <i>I<sub>c</sub>4<sub>2</sub>m</i> (121.332)             | 42 <i>m1'</i>   | G-wP     | ×   |
| 1.387  | <a href="#">Sr<sub>2</sub>FeO<sub>3</sub>F</a>                              | <i>P4/nmm</i> (129)             | <i>P<sub>C</sub>4<sub>2</sub>m</i> (111.257)             | 42 <i>m1'</i>   | G-wP     | ×   |
| 1.388  | <a href="#">La<sub>2</sub>NiO<sub>3</sub>F<sub>2</sub></a>                  | <i>Cccm</i> (66)                | <i>P<sub>Amna</sub></i> (53.333)                         | <i>mmm1'</i>    | ×        | ×   |
| 1.389  | <a href="#">Sr<sub>2</sub>CoO<sub>3</sub>Cl</a>                             | <i>P4/nmm</i> (129)             | <i>P<sub>B</sub>ccm</i> (49.274)                         | <i>mmm1'</i>    | ×        | ×   |
| 1.390  | <a href="#">La<sub>2</sub>NiO<sub>3</sub>F<sub>1.93</sub></a>               | <i>C2/c</i> (15)                | <i>P<sub>C</sub>2<sub>1</sub>/c</i> (14.84)              | 2/ <i>m1'</i>   | ×        | ×   |
| 1.391  | <a href="#">Fe<sub>2</sub>MnBO<sub>5</sub></a>                              | <i>Pbam</i> (55)                | <i>P<sub>b</sub>nma</i> (62.451)                         | <i>mmm1'</i>    | ×        | ×   |
| 1.392  | <a href="#">KCuMnS<sub>2</sub></a>                                          | <i>I4/mmm</i> (139)             | <i>C<sub>Ammm</sub></i> (65.490)                         | <i>mmm1'</i>    | ×        | ×   |
| 1.393  | <a href="#">Pb<sub>2</sub>BaCuFeO<sub>5</sub>Br</a>                         | <i>P4/mmm</i> (123)             | <i>I<sub>b</sub>mna</i> (74.562)                         | <i>mmm1'</i>    | ×        | ×   |
| 1.394  | <a href="#">Pb<sub>2</sub>BaCuFeO<sub>5</sub>Cl</a>                         | <i>P4/mmm</i> (123)             | <i>I<sub>b</sub>mna</i> (74.562)                         | <i>mmm1'</i>    | ×        | ×   |
| 1.395  | <a href="#">NdCeBaCuFeO<sub>7</sub></a>                                     | <i>I4/mmm</i> (139)             | <i>C<sub>Accm</sub></i> (66.5)                           | <i>mmm1'</i>    | ×        | ×   |
| 1.396  | <a href="#">NdCeBaCu<sub>0.9</sub>Co<sub>1.1</sub></a>                      | <i>I4/mmm</i> (139)             | <i>C<sub>Amca</sub></i> (64.480)                         | <i>mmm1'</i>    | ×        | ×   |
| 1.397  | <a href="#">Cu<sub>3</sub>Mg(OD)<sub>6</sub>Br<sub>2</sub></a>              | <i>P3m1</i> (164)               | <i>C<sub>c</sub>2/m</i> (12.63)                          | 2/ <i>m1'</i>   | ×        | ×   |
| 1.398  | <a href="#">Pr<sub>2</sub>CuO<sub>4</sub></a>                               | <i>I4/mmm</i> (139)             | <i>C<sub>Accm</sub></i> (66.5)                           | <i>mmm1'</i>    | ×        | ×   |
| 1.399  | <a href="#">Pr<sub>2</sub>CuO<sub>4</sub></a>                               | <i>I4/mmm</i> (139)             | <i>C<sub>Accm</sub></i> (66.5)                           | <i>mmm1'</i>    | ×        | ×   |
| 1.400  | <a href="#">TbAg<sub>2</sub></a>                                            | <i>I4/mmm</i> (139)             | <i>C<sub>Amca</sub></i> (64.480)                         | <i>mmm1'</i>    | ×        | ×   |
| 1.401  | <a href="#">Nd<sub>5</sub>Pb<sub>3</sub></a>                                | <i>P6<sub>3</sub>/mcm</i> (193) | <i>P<sub>B</sub>nma</i> (62.454)                         | <i>mmm1'</i>    | ×        | ×   |
| 1.402  | <a href="#">Nd<sub>5</sub>Pb<sub>3</sub></a>                                | <i>P6<sub>3</sub>/mcm</i> (193) | <i>P<sub>B</sub>nma</i> (62.454)                         | <i>mmm1'</i>    | ×        | ×   |
| 1.403  | <a href="#">La<sub>2</sub>CoO<sub>4</sub></a>                               | <i>Cmce</i> (64)                | <i>P<sub>C</sub>mna</i> (53.335)                         | <i>mmm1'</i>    | ×        | ×   |
| 1.404  | <a href="#">Sr<sub>2</sub>CuO<sub>2</sub>Cl<sub>2</sub></a>                 | <i>I4/mmm</i> (139)             | <i>C<sub>Amca</sub></i> (64.480)                         | <i>mmm1'</i>    | ×        | ×   |
| 1.405  | <a href="#">La<sub>2</sub>CuO<sub>4</sub></a>                               | <i>Bmeb</i> (64)                | <i>P<sub>Accn</sub></i> (56.374)                         | <i>mmm1'</i>    | ×        | ×   |
| 1.406  | <a href="#">Nd<sub>2</sub>CuO<sub>4</sub></a>                               | <i>I4/mmm</i> (139)             | <i>C<sub>Accm</sub></i> (66.5)                           | <i>mmm1'</i>    | ×        | ×   |
| 1.407  | <a href="#">Nd<sub>2</sub>CuO<sub>4</sub></a>                               | <i>I4/mmm</i> (139)             | <i>C<sub>Amca</sub></i> (64.480)                         | <i>mmm1'</i>    | ×        | ×   |
| 1.408  | <a href="#">Nd<sub>2</sub>CuO<sub>4</sub></a>                               | <i>I4/mmm</i> (139)             | <i>C<sub>Accm</sub></i> (66.5)                           | <i>mmm1'</i>    | ×        | ×   |
| 1.409  | <a href="#">NaMnO<sub>2</sub></a>                                           | <i>C2/m</i> (12)                | <i>P<sub>S</sub>1</i> (2.7)                              | 11'             | ×        | ×   |
| 1.410  | <a href="#">Sr<sub>2</sub>Fe<sub>1.9</sub>Cr<sub>0.1</sub>O<sub>5</sub></a> | <i>Icnm</i> (74)                | <i>P<sub>Imna</sub></i> (53.336)                         | <i>mmm1'</i>    | ×        | ×   |
| 1.411  | <a href="#">EuMn<sub>2</sub>P<sub>2</sub></a>                               | <i>P3m1</i> (164)               | <i>C<sub>c</sub>2/m</i> (12.63)                          | 2/ <i>m1'</i>   | ×        | ×   |
| 1.412  | <a href="#">Au<sub>72</sub>Al<sub>14</sub>Tb<sub>14</sub></a>               | <i>Im3</i> (204)                | <i>P<sub>I</sub>n3</i> (201.21)                          | <i>m31'</i>     | ×        | ×   |
| 1.413  | <a href="#">Ce<sub>3</sub>Ni<sub>2</sub>Ge<sub>7</sub></a>                  | <i>Cmmm</i> (65)                | <i>P<sub>C</sub>mmn</i> (59.415)                         | <i>mmm1'</i>    | ×        | ×   |
| 1.414  | <a href="#">CeNiGe<sub>3</sub></a>                                          | <i>Cmmm</i> (65)                | <i>P<sub>C</sub>mmn</i> (59.415)                         | <i>mmm1'</i>    | ×        | ×   |
| 1.415  | <a href="#">Tb<sub>2</sub>Pd<sub>2</sub>In</a>                              | <i>P4/mbm</i> (127)             | <i>C<sub>a</sub>mca</i> (64.479)                         | <i>mmm1'</i>    | ×        | ×   |
| 1.416  | <a href="#">Tb<sub>2</sub>O<sub>2</sub>S</a>                                | <i>P3m1</i> (164)               | <i>C<sub>c</sub>2/c</i> (15.90)                          | 2/ <i>m1'</i>   | ×        | ×   |
| 1.417  | <a href="#">Tb<sub>2</sub>O<sub>2</sub>Se</a>                               | <i>P3m1</i> (164)               | <i>C<sub>c</sub>2/c</i> (15.90)                          | 2/ <i>m1'</i>   | ×        | ×   |
| 1.418  | <a href="#">Cu<sub>4</sub>O<sub>3</sub></a>                                 | <i>I4<sub>1</sub>/amd</i> (141) | <i>I<sub>c</sub>4<sub>2</sub>m</i> (121.332)             | 42 <i>m1'</i>   | G-wP     | ×   |
| 1.419  | <a href="#">GdIn<sub>3</sub></a>                                            | <i>Pm3m</i> (221)               | <i>P<sub>C</sub>4/mbm</i> (127.397)                      | 4/ <i>mmm1'</i> | ×        | ×   |
| 1.420  | <a href="#">YBa<sub>2</sub>Cu<sub>3</sub>O<sub>6</sub></a>                  | <i>P4/mmm</i> (123)             | <i>C<sub>a</sub>mmm</i> (65.489)                         | <i>mmm1'</i>    | ×        | ×   |
| 1.421  | <a href="#">NdRh<sub>2</sub>Si<sub>2</sub></a>                              | <i>I4/mmm</i> (139)             | <i>P<sub>I</sub>4/mnc</i> (128.410)                      | 4/ <i>mmm1'</i> | ×        | ×   |
| 1.422  | <a href="#">ErRh<sub>2</sub>Si<sub>2</sub></a>                              | <i>I4/mmm</i> (139)             | <i>P<sub>I</sub>nm</i> (58.404)                          | <i>mmm1'</i>    | ×        | ×   |
| 1.423  | <a href="#">UPb<sub>3</sub></a>                                             | <i>Pm3m</i> (221)               | <i>P<sub>c</sub>4/mcc</i> (124.360)                      | 4/ <i>mmm1'</i> | ×        | ×   |
| 1.424  | <a href="#">UCu<sub>5</sub></a>                                             | <i>F43m</i> (216)               | <i>R<sub>I</sub>3c</i> (161.72)                          | 3 <i>m1'</i>    | G-woP    | ×   |
| 1.425  | <a href="#">UGeTe</a>                                                       | <i>I4/mmm</i> (139)             | <i>P<sub>I</sub>4/nnc</i> (126.386)                      | 4/ <i>mmm1'</i> | ×        | ×   |
| 1.426  | <a href="#">UGeS</a>                                                        | <i>P4/nmm</i> (129)             | <i>P<sub>c</sub>4/ncc</i> (130.432)                      | 4/ <i>mmm1'</i> | ×        | ×   |
| 1.427  | <a href="#">HoCo<sub>2</sub>Ge<sub>2</sub></a>                              | <i>I4/mmm</i> (139)             | <i>P<sub>I</sub>4/mnc</i> (128.410)                      | 4/ <i>mmm1'</i> | ×        | ×   |
| 1.428  | <a href="#">UN</a>                                                          | <i>Fm3m</i> (225)               | <i>P<sub>I</sub>4/mnc</i> (128.410)                      | 4/ <i>mmm1'</i> | ×        | ×   |
| 1.429  | <a href="#">BaFe<sub>2</sub>Se<sub>3</sub></a>                              | <i>Pnma</i> (62)                | <i>C<sub>a</sub>m</i> (8.36)                             | <i>m1'</i>      | G-wP     | ×   |

Continued on next page

TABLE S7 – continued from previous page

| BCS-ID | Formula                                                     | Parent             | MSG                    | MPG       | SHG type | LMO |
|--------|-------------------------------------------------------------|--------------------|------------------------|-----------|----------|-----|
| 1.430  | $\text{Mn}_5(\text{VO}_4)_2(\text{OH})_4$                   | $C2/m$ (12)        | $P_62/c$ (13.71)       | $2/m1'$   | ×        | ×   |
| 1.431  | $\text{Ca}_2\text{Mn}_3\text{O}_8$                          | $C2/m$ (12)        | $P_S1$ (2.7)           | $11'$     | ×        | ×   |
| 1.432  | $\text{Ba}_2\text{LuRuO}_6$                                 | $Fm\bar{3}m$ (225) | $C_{Amca}$ (64.480)    | $mmm1'$   | ×        | ×   |
| 1.433  | $\text{Ba}_2\text{YRuO}_6$                                  | $Fm\bar{3}m$ (225) | $C_{Amca}$ (64.480)    | $mmm1'$   | ×        | ×   |
| 1.434  | $\text{Fe}_{1.05}\text{Te}$                                 | $P4/nmm$ (129)     | $P_a2_1/m$ (11.55)     | $2/m1'$   | ×        | ×   |
| 1.435  | $\text{Fe}_{1.05}\text{Te}$                                 | $P4/nmm$ (129)     | $P_a2_1/m$ (11.55)     | $2/m1'$   | ×        | ×   |
| 1.436  | $\text{Fe}_{1.125}\text{Te}$                                | $P4/nmm$ (129)     | $P_S1$ (2.7)           | $11'$     | ×        | ×   |
| 1.437  | $\text{Fe}_{1.068}\text{Te}$                                | $P4/nmm$ (129)     | $P_S1$ (2.7)           | $11'$     | ×        | ×   |
| 1.438  | $\text{BaCoF}_4$                                            | $A2_1am$ (36)      | $P_a2_1$ (4.10)        | $21'$     | G-woP    | ×   |
| 1.439  | $\text{BaCoF}_4$                                            | $A2_1am$ (36)      | $P_bca2_1$ (29.105)    | $mm21'$   | G-woP    | ×   |
| 1.440  | $\text{CrPS}_4$                                             | $C2$ (5)           | $C_2$ (5.16)           | $21'$     | G-woP    | ×   |
| 1.441  | $\text{NaFe}_3(\text{SO}_4)_2(\text{OH})_6$                 | $R\bar{3}m$ (166)  | $R_13c$ (167.108)      | $3m1'$    | ×        | ×   |
| 1.442  | $\text{URu}_2\text{Si}_2$                                   | $I4/mmm$ (139)     | $P_14/mnc$ (128.410)   | $4/mmm1'$ | ×        | ×   |
| 1.443  | $\text{Gd}_2\text{BaCuO}_5$                                 | $Pnma$ (62)        | $P_a2_1$ (29.104)      | $mm21'$   | G-wP     | ×   |
| 1.444  | $\text{Er}_2\text{Pt}$                                      | $Pnma$ (62)        | $P_a2_1$ (33.149)      | $mm21'$   | G-wP     | ×   |
| 1.445  | $\text{Y}_2\text{BaCuO}_5$                                  | $Pnma$ (62)        | $P_a2_1/c$ (14.80)     | $2/m1'$   | ×        | ×   |
| 1.446  | $\text{CeCoAl}_4$                                           | $Pmma$ (51)        | $C_{Amca}$ (64.479)    | $mmm1'$   | ×        | ×   |
| 1.447  | $\text{Ce}_3\text{Ni}_2\text{Sn}_7$                         | $Cmmm$ (65)        | $P_Cmmn$ (59.415)      | $mmm1'$   | ×        | ×   |
| 1.448  | $\text{HoSi}$                                               | $Cmcm$ (63)        | $C_a2/c$ (15.91)       | $2/m1'$   | ×        | ×   |
| 1.449  | $\text{Li}_2\text{CuW}_2\text{O}_8$                         | $P1$ (2)           | $P_S1$ (2.7)           | $11'$     | ×        | ×   |
| 1.450  | $\text{Pr}_6\text{Fe}_{13}\text{Sn}$                        | $I4/mcm$ (140)     | $P_1bcn$ (60.432)      | $mmm1'$   | ×        | ×   |
| 1.451  | $\text{Nd}_6\text{Fe}_{13}\text{Sn}$                        | $I4/mcm$ (140)     | $P_14/mcc$ (124.362)   | $4/mmm1'$ | ×        | ×   |
| 1.452  | $\text{FeSn}$                                               | $P6/mmm$ (191)     | $C_mcm$ (63.466)       | $mmm1'$   | ×        | ×   |
| 1.453  | $\text{EuMn}_2\text{Si}_2$                                  | $I4/mmm$ (139)     | $P_14/nnc$ (126.386)   | $4/mmm1'$ | ×        | ×   |
| 1.454  | $\text{Mn}_6\text{Ni}_{16}\text{Si}_7$                      | $Fm\bar{3}m$ (225) | $C_{Amca}$ (64.480)    | $mmm1'$   | ×        | ×   |
| 1.455  | $\text{Mn}_6\text{Ni}_{16}\text{Si}_7$                      | $Fm\bar{3}m$ (225) | $P_A2_1/c$ (14.83)     | $2/m1'$   | ×        | ×   |
| 1.456  | $\text{Sr}_2\text{CuO}_2\text{Cu}_2\text{S}_2$              | $I4/mmm$ (139)     | $I_42d$ (122.338)      | $42m1'$   | G-wP     | ×   |
| 1.457  | $\text{NdNiMg}_{15}$                                        | $P4/nmm$ (129)     | $P_Bcca$ (54.350)      | $mmm1'$   | ×        | ×   |
| 1.458  | $\text{CsCo}_2\text{Se}_2$                                  | $I4/mmm$ (139)     | $C_{Amcm}$ (63.468)    | $mmm1'$   | ×        | ×   |
| 1.459  | $\text{CeFe}_3(\text{BO}_3)_4$                              | $R32$ (155)        | $C_c2$ (5.16)          | $21'$     | G-woP    | ×   |
| 1.460  | $\text{PrCuSi}$                                             | $P6_3/mmc$ (194)   | $P_Cbcn$ (60.431)      | $mmm1'$   | ×        | ×   |
| 1.461  | $\text{Sr}_2\text{Cr}_3\text{As}_2\text{O}_2$               | $I4/mmm$ (139)     | $P_14_2/mnm$ (136.506) | $4/mmm1'$ | ×        | ×   |
| 1.462  | $\text{La}_2\text{CoPtO}_6$                                 | $P2_1/n$ (14)      | $P_a2_1/c$ (14.80)     | $2/m1'$   | ×        | ×   |
| 1.463  | $\text{Sr}_2\text{Fe}_3\text{Se}_2\text{O}_3$               | $Pbam$ (55)        | $C_a2c2_1$ (36.178)    | $mm21'$   | G-wP     | ×   |
| 1.464  | $\text{U}_2\text{N}_2\text{P}$                              | $P3m1$ (164)       | $P_c3c1$ (165.96)      | $3m1'$    | ×        | ×   |
| 1.465  | $\text{U}_2\text{N}_2\text{As}$                             | $P3m1$ (164)       | $P_c3c1$ (165.96)      | $3m1'$    | ×        | ×   |
| 1.466  | $\text{MnPt}_{0.5}\text{Pd}_{0.5}$                          | $P4/mmm$ (123)     | $C_{Amma}$ (67.509)    | $mmm1'$   | ×        | ×   |
| 1.467  | $\text{Tb}_{0.6}\text{Y}_{0.4}\text{RhIn}_5$                | $P4/mmm$ (123)     | $C_{Amma}$ (67.509)    | $mmm1'$   | ×        | ×   |
| 1.468  | $\text{TbMn}_2\text{Si}_2$                                  | $I4/mmm$ (139)     | $P_14/nnc$ (126.386)   | $4/mmm1'$ | ×        | ×   |
| 1.469  | $\text{YMn}_2\text{Si}_2$                                   | $I4/mmm$ (139)     | $P_14/nnc$ (126.386)   | $4/mmm1'$ | ×        | ×   |
| 1.470  | $\text{UCr}_2\text{Si}_2$                                   | $C2/m$ (12)        | $C_c2/c$ (15.90)       | $2/m1'$   | ×        | ×   |
| 1.471  | $\text{EuCd}_2\text{As}_2$                                  | $P3m1$ (164)       | $C_c2/m$ (12.63)       | $2/m1'$   | ×        | ×   |
| 1.472  | $\text{CaOFeS}$                                             | $P6_3mc$ (186)     | $P_Cca2_1$ (29.109)    | $mm21'$   | G-woP    | ×   |
| 1.473  | $\text{CuBr}(\text{C}_4\text{H}_4\text{N}_2)_2(\text{BP4})$ | $P4/nbm$ (125)     | $P_bnna$ (52.315)      | $mmm1'$   | ×        | ×   |
| 1.474  | $\text{CuCl}(\text{C}_4\text{H}_4\text{N}_2)_2(\text{BP4})$ | $P4/nbm$ (125)     | $P_bnna$ (52.315)      | $mmm1'$   | ×        | ×   |
| 1.475  | $\text{DyNiAl}_4$                                           | $Cmcm$ (63)        | $P_Anma$ (62.453)      | $mmm1'$   | ×        | ×   |
| 1.476  | $\text{Ba}_2\text{CoO}_4$                                   | $P2_1/n$ (14)      | $P_a2_1/c$ (14.80)     | $2/m1'$   | ×        | ×   |
| 1.477  | $\text{Ba}_2\text{CoO}_4$                                   | $P2_1/n$ (14)      | $P_a2_1/c$ (14.80)     | $2/m1'$   | ×        | ×   |
| 1.478  | $\text{CoTi}_2\text{O}_5$                                   | $Cmcm$ (63)        | $P_a2_1/m$ (11.55)     | $2/m1'$   | ×        | ×   |
| 1.479  | $\text{U}_2\text{Ni}_2\text{Sn}$                            | $P4/mbm$ (127)     | $P_c4_2/mbc$ (135.492) | $4/mmm1'$ | ×        | ×   |
| 1.480  | $\text{Mn}_2\text{CoReO}_6$                                 | $P2_1/n$ (14)      | $P_S1$ (2.7)           | $11'$     | ×        | ×   |
| 1.481  | $\text{LaSr}_3\text{Fe}_3\text{O}_9$                        | $Cmcm$ (63)        | $P_Cbcm$ (57.391)      | $mmm1'$   | ×        | ×   |
| 1.482  | $\text{Er}_2\text{Fe}_2\text{Si}_2\text{C}$                 | $C2/m$ (12)        | $P_S1$ (2.7)           | $11'$     | ×        | ×   |
| 1.483  | $\text{Eu}_{0.5}\text{Ca}_{0.5}\text{Fe}_2\text{As}_2$      | $Fmmm$ (69)        | $C_{Amca}$ (64.480)    | $mmm1'$   | ×        | ×   |
| 1.484  | $\text{Li}_2\text{MnGeO}_4$                                 | $Pmn2_1$ (31)      | $C_{ac}$ (9.41)        | $m1'$     | G-woP    | ×   |
| 1.485  | $\text{Mn}_3\text{TeO}_6$                                   | $P2_1/c$ (14)      | $P_a2_1/c$ (14.80)     | $2/m1'$   | ×        | ×   |
| 1.486  | $\text{CeRhAl}_4\text{Si}_2$                                | $P4/mmm$ (123)     | $P_c4/mcc$ (124.360)   | $4/mmm1'$ | ×        | ×   |
| 1.487  | $\text{CeIrAl}_4\text{Si}_2$                                | $P4/mmm$ (123)     | $P_c4/mcc$ (124.360)   | $4/mmm1'$ | ×        | ×   |

Continued on next page

TABLE S7 – continued from previous page

| BCS-ID | Formula                                                                                 | Parent                                             | MSG                                                                | MPG            | SHG type | LMO |
|--------|-----------------------------------------------------------------------------------------|----------------------------------------------------|--------------------------------------------------------------------|----------------|----------|-----|
| 1.488  | <a href="#">CeMn<sub>2</sub>Si<sub>2</sub></a>                                          | <i>I4/mmm</i> (139)                                | <i>P</i> <sub>1</sub> <i>4/nnc</i> (126.386)                       | <i>4/mmm1'</i> | ×        | ×   |
| 1.489  | <a href="#">CeMn<sub>2</sub>Si<sub>2</sub></a>                                          | <i>I4/mmm</i> (139)                                | <i>P</i> <sub>1</sub> <i>4/nnc</i> (126.386)                       | <i>4/mmm1'</i> | ×        | ×   |
| 1.490  | <a href="#">CeMn<sub>2</sub>Si<sub>2</sub></a>                                          | <i>I4/mmm</i> (139)                                | <i>P</i> <sub>1</sub> <i>4/nnc</i> (126.386)                       | <i>4/mmm1'</i> | ×        | ×   |
| 1.491  | <a href="#">PrMn<sub>2</sub>Si<sub>2</sub></a>                                          | <i>I4/mmm</i> (139)                                | <i>P</i> <sub>1</sub> <i>4/nnc</i> (126.386)                       | <i>4/mmm1'</i> | ×        | ×   |
| 1.492  | <a href="#">PrMn<sub>2</sub>Si<sub>2</sub></a>                                          | <i>I4/mmm</i> (139)                                | <i>P</i> <sub>1</sub> <i>4/nnc</i> (126.386)                       | <i>4/mmm1'</i> | ×        | ×   |
| 1.493  | <a href="#">NdMn<sub>2</sub>Si<sub>2</sub></a>                                          | <i>I4/mmm</i> (139)                                | <i>P</i> <sub>1</sub> <i>4/nnc</i> (126.386)                       | <i>4/mmm1'</i> | ×        | ×   |
| 1.494  | <a href="#">NdMn<sub>2</sub>Si<sub>2</sub></a>                                          | <i>I4/mmm</i> (139)                                | <i>P</i> <sub>1</sub> <i>4/nnc</i> (126.386)                       | <i>4/mmm1'</i> | ×        | ×   |
| 1.495  | <a href="#">YMn<sub>2</sub>Si<sub>2</sub></a>                                           | <i>I4/mmm</i> (139)                                | <i>P</i> <sub>1</sub> <i>4/nnc</i> (126.386)                       | <i>4/mmm1'</i> | ×        | ×   |
| 1.496  | <a href="#">YMn<sub>2</sub>Ge<sub>2</sub></a>                                           | <i>I4/mmm</i> (139)                                | <i>P</i> <sub>1</sub> <i>4/nnc</i> (126.386)                       | <i>4/mmm1'</i> | ×        | ×   |
| 1.497  | <a href="#">EuMg<sub>2</sub>Bi<sub>2</sub></a>                                          | <i>P</i> <sub>3</sub> <i>m</i> 1 (164)             | <i>C</i> <sub>c</sub> <i>2/m</i> (12.63)                           | <i>2/m1'</i>   | ×        | ×   |
| 1.498  | <a href="#">Cu<sub>6</sub>(SiO<sub>3</sub>)<sub>6</sub>(H<sub>2</sub>O)<sub>6</sub></a> | <i>R</i> <sub>3</sub> (148)                        | <i>R</i> <sub>1</sub> <i>3</i> (148.20)                            | <i>31'</i>     | ×        | ×   |
| 1.499  | <a href="#">CsFe(MoO<sub>4</sub>)<sub>2</sub></a>                                       | <i>P</i> <sub>3</sub> (147)                        | <i>P</i> <sub>c</sub> <i>3</i> (143.3)                             | <i>31'</i>     | G-wP     | ×   |
| 1.500  | <a href="#">Sr<sub>2</sub>CoO<sub>2</sub>Cu<sub>2</sub>S<sub>2</sub></a>                | <i>I4/mmm</i> (139)                                | <i>P</i> <sub>S</sub> <i>1</i> (2.7)                               | <i>11'</i>     | ×        | ×   |
| 1.501  | <a href="#">Ba<sub>2</sub>CoO<sub>2</sub>Cu<sub>2</sub>S<sub>2</sub></a>                | <i>I4/mmm</i> (139)                                | <i>P</i> <sub>S</sub> <i>1</i> (2.7)                               | <i>11'</i>     | ×        | ×   |
| 1.502  | <a href="#">Li<sub>3</sub>Co<sub>2</sub>SbO<sub>6</sub></a>                             | <i>C</i> <sub>2</sub> / <i>m</i> (12)              | <i>C</i> <sub>c</sub> <i>2/m</i> (12.63)                           | <i>2/m1'</i>   | ×        | ×   |
| 1.503  | <a href="#">NdScSiC<sub>0.5</sub>H<sub>0.2</sub></a>                                    | <i>I4/mmm</i> (139)                                | <i>P</i> <sub>1</sub> <i>4/nnc</i> (126.386)                       | <i>4/mmm1'</i> | ×        | ×   |
| 1.504  | <a href="#">GdCuSn</a>                                                                  | <i>P</i> <sub>6</sub> <i>3mc</i> (186)             | <i>P</i> <sub>C</sub> <i>na2</i> <sub>1</sub> (33.154)             | <i>mm21'</i>   | G-woP    | ×   |
| 1.505  | <a href="#">GdAgSn</a>                                                                  | <i>P</i> <sub>6</sub> <i>3mc</i> (186)             | <i>P</i> <sub>C</sub> <i>na2</i> <sub>1</sub> (33.154)             | <i>mm21'</i>   | G-woP    | ×   |
| 1.506  | <a href="#">GdAuSn</a>                                                                  | <i>P</i> <sub>6</sub> <i>3mc</i> (186)             | <i>P</i> <sub>C</sub> <i>na2</i> <sub>1</sub> (33.154)             | <i>mm21'</i>   | G-woP    | ×   |
| 1.507  | <a href="#">NdPd<sub>5</sub>Al<sub>2</sub></a>                                          | <i>I4/mmm</i> (139)                                | <i>P</i> <sub>a</sub> <i>nma</i> (62.450)                          | <i>mmm1'</i>   | ×        | ×   |
| 1.508  | <a href="#">Mn<sub>2</sub>AlB<sub>2</sub></a>                                           | <i>Cmmm</i> (65)                                   | <i>C</i> <sub>c</sub> <i>mcm</i> (63.466)                          | <i>mmm1'</i>   | ×        | ×   |
| 1.509  | <a href="#">Pd<sub>2.87</sub>Mn<sub>0.88</sub></a>                                      | <i>I4/mmm</i> (139)                                | <i>P</i> <sub>A</sub> <i>2</i> <sub>1</sub> / <i>c</i> (14.83)     | <i>2/m1'</i>   | ×        | ×   |
| 1.510  | <a href="#">TbNi<sub>2</sub>Ge<sub>2</sub></a>                                          | <i>I4/mmm</i> (139)                                | <i>P</i> <sub>c</sub> <i>4/mcc</i> (124.360)                       | <i>4/mmm1'</i> | ×        | ×   |
| 1.511  | <a href="#">TbNi<sub>2</sub>Si<sub>2</sub></a>                                          | <i>I4/mmm</i> (139)                                | <i>C</i> <sub>Amca</sub> (64.480)                                  | <i>mmm1'</i>   | ×        | ×   |
| 1.512  | <a href="#">TbCo<sub>2</sub>Si<sub>2</sub></a>                                          | <i>I4/mmm</i> (139)                                | <i>P</i> <sub>1</sub> <i>4/mnc</i> (128.410)                       | <i>4/mmm1'</i> | ×        | ×   |
| 1.513  | <a href="#">HoCo<sub>2</sub>Si<sub>2</sub></a>                                          | <i>I4/mmm</i> (139)                                | <i>P</i> <sub>1</sub> <i>4/mnc</i> (128.410)                       | <i>4/mmm1'</i> | ×        | ×   |
| 1.514  | <a href="#">HoCo<sub>2</sub>Si<sub>2</sub></a>                                          | <i>I4/mmm</i> (139)                                | <i>P</i> <sub>1</sub> <i>4/mnc</i> (128.410)                       | <i>4/mmm1'</i> | ×        | ×   |
| 1.515  | <a href="#">ErCo<sub>2</sub>Si<sub>2</sub></a>                                          | <i>I4/mmm</i> (139)                                | <i>P</i> <sub>A</sub> <i>2</i> <sub>1</sub> / <i>c</i> (14.83)     | <i>2/m1'</i>   | ×        | ×   |
| 1.516  | <a href="#">ErCo<sub>2</sub>Si<sub>2</sub></a>                                          | <i>I4/mmm</i> (139)                                | <i>P</i> <sub>I</sub> <i>nnm</i> (58.404)                          | <i>mmm1'</i>   | ×        | ×   |
| 1.517  | <a href="#">DyBe<sub>13</sub></a>                                                       | <i>Fm</i> <sub>3</sub> <i>c</i> (226)              | <i>C</i> <sub>A</sub> <i>222</i> <sub>1</sub> (20.37)              | <i>2221'</i>   | G-wP     | ×   |
| 1.518  | <a href="#">TbBe<sub>13</sub></a>                                                       | <i>Fm</i> <sub>3</sub> <i>c</i> (226)              | <i>C</i> <sub>A</sub> <i>222</i> <sub>1</sub> (20.37)              | <i>2221'</i>   | G-wP     | ×   |
| 1.519  | <a href="#">CoSO<sub>4</sub></a>                                                        | <i>Cmcm</i> (63)                                   | <i>P</i> <sub>C</sub> <i>bcn</i> (60.431)                          | <i>mmm1'</i>   | ×        | ×   |
| 1.520  | <a href="#">NiSO<sub>4</sub></a>                                                        | <i>Cmcm</i> (63)                                   | <i>P</i> <sub>C</sub> <i>bcn</i> (60.431)                          | <i>mmm1'</i>   | ×        | ×   |
| 1.521  | <a href="#">FeSO<sub>4</sub></a>                                                        | <i>Cmcm</i> (63)                                   | <i>P</i> <sub>C</sub> <i>bcn</i> (60.431)                          | <i>mmm1'</i>   | ×        | ×   |
| 1.522  | <a href="#">CrVO<sub>4</sub></a>                                                        | <i>Cmcm</i> (63)                                   | <i>P</i> <sub>1</sub> (2.4)                                        | <i>1</i>       | ×        | ✓   |
| 1.523  | <a href="#">VPO<sub>4</sub></a>                                                         | <i>Cmcm</i> (63)                                   | <i>P</i> <sub>c</sub> <i>nma</i> (62.452)                          | <i>mmm1'</i>   | ×        | ×   |
| 1.524  | <a href="#">InMnO<sub>3</sub></a>                                                       | <i>P</i> <sub>6</sub> <i>3cm</i> (185)             | <i>P</i> <sub>c</sub> <i>31c</i> (159.64)                          | <i>3m1'</i>    | G-woP    | ×   |
| 1.525  | <a href="#">InMnO<sub>3</sub></a>                                                       | <i>P</i> <sub>6</sub> <i>3cm</i> (185)             | <i>P</i> <sub>c</sub> <i>31m</i> (157.56)                          | <i>3m1'</i>    | G-woP    | ×   |
| 1.526  | <a href="#">LiCoF<sub>4</sub></a>                                                       | <i>P</i> <sub>2</sub> <sub>1</sub> / <i>c</i> (14) | <i>P</i> <sub>a</sub> <i>2</i> <sub>1</sub> / <i>c</i> (14.80)     | <i>2/m1'</i>   | ×        | ×   |
| 1.527  | <a href="#">CsNiF<sub>3</sub></a>                                                       | <i>P</i> <sub>6</sub> <i>3/mnc</i> (194)           | <i>P</i> <sub>B</sub> <i>nnm</i> (58.402)                          | <i>mmm1'</i>   | ×        | ×   |
| 1.528  | <a href="#">Bi<sub>2</sub>Fe<sub>4</sub>O<sub>9</sub></a>                               | <i>Pbam</i> (55)                                   | <i>C</i> <sub>a</sub> <i>2/m</i> (12.64)                           | <i>2/m1'</i>   | ×        | ×   |
| 1.529  | <a href="#">MnBi<sub>6</sub>Te<sub>10</sub></a>                                         | <i>R</i> <sub>3</sub> <i>m</i> (166)               | <i>R</i> <sub>I</sub> <i>3c</i> (167.108)                          | <i>3m1'</i>    | ×        | ×   |
| 1.530  | <a href="#">CeC<sub>2</sub></a>                                                         | <i>I4/mmm</i> (139)                                | <i>P</i> <sub>1</sub> <i>4/mnc</i> (128.410)                       | <i>4/mmm1'</i> | ×        | ×   |
| 1.531  | <a href="#">PrC<sub>2</sub></a>                                                         | <i>I4/mmm</i> (139)                                | <i>P</i> <sub>1</sub> <i>4/mnc</i> (128.410)                       | <i>4/mmm1'</i> | ×        | ×   |
| 1.532  | <a href="#">NdC<sub>2</sub></a>                                                         | <i>I4/mmm</i> (139)                                | <i>P</i> <sub>1</sub> <i>4/mnc</i> (128.410)                       | <i>4/mmm1'</i> | ×        | ×   |
| 1.533  | <a href="#">TbC<sub>2</sub></a>                                                         | <i>I4/mmm</i> (139)                                | <i>P</i> <sub>c</sub> <i>222</i> <sub>1</sub> (17.12)              | <i>2221'</i>   | G-wP     | ×   |
| 1.534  | <a href="#">HoC<sub>2</sub></a>                                                         | <i>I4/mmm</i> (139)                                | <i>P</i> <sub>a</sub> <i>nma</i> (51.298)                          | <i>mmm1'</i>   | ×        | ×   |
| 1.535  | <a href="#">UPd<sub>2</sub>Ge<sub>2</sub></a>                                           | <i>I4/mmm</i> (139)                                | <i>P</i> <sub>c</sub> <i>4/ncc</i> (130.432)                       | <i>4/mmm1'</i> | ×        | ×   |
| 1.536  | <a href="#">UPd<sub>2</sub>Si<sub>2</sub></a>                                           | <i>I4/mmm</i> (139)                                | <i>P</i> <sub>1</sub> <i>4/mnc</i> (128.410)                       | <i>4/mmm1'</i> | ×        | ×   |
| 1.537  | <a href="#">URh<sub>2</sub>Si<sub>2</sub></a>                                           | <i>I4/mmm</i> (139)                                | <i>P</i> <sub>1</sub> <i>4/mnc</i> (128.410)                       | <i>4/mmm1'</i> | ×        | ×   |
| 1.538  | <a href="#">Ba<sub>2</sub>MnTeO<sub>6</sub></a>                                         | <i>R</i> <sub>3</sub> <i>m</i> (166)               | <i>P</i> <sub>A</sub> <i>2</i> <sub>1</sub> / <i>c</i> (14.83)     | <i>2/m1'</i>   | ×        | ×   |
| 1.539  | <a href="#">KMnP</a>                                                                    | <i>P</i> <sub>4</sub> / <i>nnm</i> (129)           | <i>P</i> <sub>c</sub> <i>4</i> <sub>2</sub> / <i>ncm</i> (138.528) | <i>4/mmm1'</i> | ×        | ×   |
| 1.540  | <a href="#">KMnP</a>                                                                    | <i>P</i> <sub>4</sub> / <i>nnm</i> (129)           | <i>P</i> <sub>c</sub> <i>4</i> <sub>2</sub> / <i>ncm</i> (138.528) | <i>4/mmm1'</i> | ×        | ×   |
| 1.541  | <a href="#">RbMnP</a>                                                                   | <i>P</i> <sub>4</sub> / <i>nnm</i> (129)           | <i>P</i> <sub>c</sub> <i>4</i> <sub>2</sub> / <i>ncm</i> (138.528) | <i>4/mmm1'</i> | ×        | ×   |
| 1.542  | <a href="#">RbMnP</a>                                                                   | <i>P</i> <sub>4</sub> / <i>nnm</i> (129)           | <i>P</i> <sub>c</sub> <i>4</i> <sub>2</sub> / <i>ncm</i> (138.528) | <i>4/mmm1'</i> | ×        | ×   |
| 1.543  | <a href="#">RbMnAs</a>                                                                  | <i>P</i> <sub>4</sub> / <i>nnm</i> (129)           | <i>P</i> <sub>c</sub> <i>4</i> <sub>2</sub> / <i>ncm</i> (138.528) | <i>4/mmm1'</i> | ×        | ×   |
| 1.544  | <a href="#">RbMnAs</a>                                                                  | <i>P</i> <sub>4</sub> / <i>nnm</i> (129)           | <i>P</i> <sub>c</sub> <i>4</i> <sub>2</sub> / <i>ncm</i> (138.528) | <i>4/mmm1'</i> | ×        | ×   |
| 1.545  | <a href="#">RbMnBi</a>                                                                  | <i>P</i> <sub>4</sub> / <i>nnm</i> (129)           | <i>P</i> <sub>c</sub> <i>4</i> <sub>2</sub> / <i>ncm</i> (138.528) | <i>4/mmm1'</i> | ×        | ×   |

Continued on next page

TABLE S7 – continued from previous page

| BCS-ID | Formula                                                                                          | Parent           | MSG                      | MPG       | SHG type | LMO |
|--------|--------------------------------------------------------------------------------------------------|------------------|--------------------------|-----------|----------|-----|
| 1.546  | <a href="#">CsMnBi</a>                                                                           | $P4/nmm$ (129)   | $P_{c4_2}/ncm$ (138.528) | $4/mmm1'$ | ×        | ×   |
| 1.547  | <a href="#">CsMnP</a>                                                                            | $P4/nmm$ (129)   | $P_{c4_2}/ncm$ (138.528) | $4/mmm1'$ | ×        | ×   |
| 1.548  | <a href="#">CsMnP</a>                                                                            | $P4/nmm$ (129)   | $P_{c4_2}/ncm$ (138.528) | $4/mmm1'$ | ×        | ×   |
| 1.549  | <a href="#">U<sub>2</sub>Ni<sub>2</sub>In</a>                                                    | $P4/mbm$ (127)   | $P_{c4}/mnc$ (128.408)   | $4/mmm1'$ | ×        | ×   |
| 1.550  | <a href="#">LiMnAs</a>                                                                           | $P4/nmm$ (129)   | $P_{c4_2}/ncm$ (138.528) | $4/mmm1'$ | ×        | ×   |
| 1.551  | <a href="#">LiMnAs</a>                                                                           | $P4/nmm$ (129)   | $P_{c4_2}/ncm$ (138.528) | $4/mmm1'$ | ×        | ×   |
| 1.552  | <a href="#">LiMnAs</a>                                                                           | $P4/nmm$ (129)   | $P_{c4_2}/ncm$ (138.528) | $4/mmm1'$ | ×        | ×   |
| 1.553  | <a href="#">KMnAs</a>                                                                            | $P4/nmm$ (129)   | $P_{c4_2}/ncm$ (138.528) | $4/mmm1'$ | ×        | ×   |
| 1.554  | <a href="#">KMnAs</a>                                                                            | $P4/nmm$ (129)   | $P_{c4_2}/ncm$ (138.528) | $4/mmm1'$ | ×        | ×   |
| 1.555  | <a href="#">Mn<sub>3</sub>B<sub>4</sub></a>                                                      | $Immm$ (71)      | $P_{1nnm}$ (58.404)      | $mmm1'$   | ×        | ×   |
| 1.556  | <a href="#">FeSn<sub>2</sub></a>                                                                 | $I4/mcm$ (140)   | $P_{1bcn}$ (60.432)      | $mmm1'$   | ×        | ×   |
| 1.557  | <a href="#">FeGe<sub>2</sub></a>                                                                 | $I4/mcm$ (140)   | $P_{1bcn}$ (60.432)      | $mmm1'$   | ×        | ×   |
| 1.558  | <a href="#">MnSn<sub>2</sub></a>                                                                 | $I4/mcm$ (140)   | $C_{Acca}$ (68.520)      | $mmm1'$   | ×        | ×   |
| 1.559  | <a href="#">MnSn<sub>2</sub></a>                                                                 | $I4/mcm$ (140)   | $C_{ccm}$ (66.498)       | $mmm1'$   | ×        | ×   |
| 1.560  | <a href="#">GeNi<sub>2</sub>O<sub>4</sub></a>                                                    | $Fd3m$ (227)     | $C_{c2}/m$ (12.63)       | $2/m1'$   | ×        | ×   |
| 1.561  | <a href="#">GeNi<sub>2</sub>O<sub>4</sub></a>                                                    | $Fd3m$ (227)     | $C_{cm}$ (8.35)          | $m1'$     | G-wP     | ×   |
| 1.562  | <a href="#">GeNi<sub>2</sub>O<sub>4</sub></a>                                                    | $Fd3m$ (227)     | $C_{c2}$ (5.16)          | $21'$     | G-wP     | ×   |
| 1.563  | <a href="#">GeNi<sub>2</sub>O<sub>4</sub></a>                                                    | $Fd3m$ (227)     | $C_{cm}$ (8.35)          | $m1'$     | G-wP     | ×   |
| 1.564  | <a href="#">GeCo<sub>2</sub>O<sub>4</sub></a>                                                    | $Fd3m$ (227)     | $C_{c2}$ (5.16)          | $21'$     | G-wP     | ×   |
| 1.565  | <a href="#">Pb<sub>2</sub>CoOsO<sub>6</sub></a>                                                  | $P2_1/n$ (14)    | $P_{ac}$ (7.27)          | $m1'$     | G-wP     | ×   |
| 1.566  | <a href="#">Ba<sub>2</sub>YbRuO<sub>6</sub></a>                                                  | $Fm3m$ (225)     | $P_{14}/mnc$ (128.410)   | $4/mmm1'$ | ×        | ×   |
| 1.567  | <a href="#">Ba<sub>2</sub>TmRuO<sub>6</sub></a>                                                  | $Fm3m$ (225)     | $P_{14}/mnc$ (128.410)   | $4/mmm1'$ | ×        | ×   |
| 1.568  | <a href="#">GdCu<sub>2</sub>Si<sub>2</sub></a>                                                   | $I4/mmm$ (139)   | $C_{c2}/m$ (12.63)       | $2/m1'$   | ×        | ×   |
| 1.569  | <a href="#">SrRu<sub>2</sub>O<sub>6</sub></a>                                                    | $P31m$ (162)     | $P_{c31m}$ (162.78)      | $3m1'$    | ×        | ×   |
| 1.570  | <a href="#">La<sub>3</sub>OsO<sub>7</sub></a>                                                    | $Cmcm$ (63)      | $P_{a2_1}/m$ (11.55)     | $2/m1'$   | ×        | ×   |
| 1.571  | <a href="#">La<sub>3</sub>OsO<sub>7</sub></a>                                                    | $Cmcm$ (63)      | $P_{a2_1}/m$ (11.55)     | $2/m1'$   | ×        | ×   |
| 1.572  | <a href="#">La<sub>2.8</sub>Ca<sub>0.2</sub>OsO<sub>7</sub></a>                                  | $Cmcm$ (63)      | $P_{a2_1}/m$ (11.55)     | $2/m1'$   | ×        | ×   |
| 1.573  | <a href="#">FeSO<sub>4</sub></a>                                                                 | $Pbnm$ (62)      | $P_{c2_1}/c$ (14.82)     | $2/m1'$   | ×        | ×   |
| 1.574  | <a href="#">NdBiPt</a>                                                                           | $F43m$ (216)     | $P_{14n2}$ (118.314)     | $42m1'$   | G-woP    | ×   |
| 1.575  | <a href="#">ErRh</a>                                                                             | $Pm3m$ (221)     | $P_{amma}$ (51.298)      | $mmm1'$   | ×        | ×   |
| 1.576  | <a href="#">Yb<sub>2</sub>O<sub>2</sub>S</a>                                                     | $P3m1$ (164)     | $C_{c2}/m$ (12.63)       | $2/m1'$   | ×        | ×   |
| 1.577  | <a href="#">SrNd<sub>2</sub>O<sub>4</sub></a>                                                    | $Pnam$ (62)      | $P_{a2_1}/c$ (14.80)     | $2/m1'$   | ×        | ×   |
| 1.578  | <a href="#">KErSe<sub>2</sub></a>                                                                | $R3m$ (166)      | $C_{c2}/m$ (12.63)       | $2/m1'$   | ×        | ×   |
| 1.579  | <a href="#">NiTiO<sub>3</sub></a>                                                                | $R3$ (148)       | $P_{S1}$ (2.7)           | $11'$     | ×        | ×   |
| 1.580  | <a href="#">NiTiO<sub>3</sub></a>                                                                | $R3$ (148)       | $P_{S1}$ (2.7)           | $11'$     | ×        | ×   |
| 1.581  | <a href="#">FeTiO<sub>3</sub></a>                                                                | $R3$ (148)       | $R_{I3}$ (148.20)        | $31'$     | ×        | ×   |
| 1.582  | <a href="#">Fe<sub>0.945</sub>O</a>                                                              | $Fm3m$ (225)     | $R_{I3c}$ (167.108)      | $3m1'$    | ×        | ×   |
| 1.583  | <a href="#">La<sub>1.5</sub>Ca<sub>0.5</sub>CoO<sub>4</sub></a>                                  | $Cmm2$ (35)      | $P_{cc}$ (7.28)          | $m1'$     | G-woP    | ×   |
| 1.584  | <a href="#">PrFeAsO</a>                                                                          | $Cmme$ (67)      | $P_{Bcca}$ (54.350)      | $mmm1'$   | ×        | ×   |
| 1.585  | <a href="#">PrFeAsO</a>                                                                          | $Cmme$ (67)      | $P_{Bcca}$ (54.350)      | $mmm1'$   | ×        | ×   |
| 1.586  | <a href="#">PrFeAsO</a>                                                                          | $Cmme$ (67)      | $P_{Acc2}$ (27.85)       | $mm21'$   | G-wP     | ×   |
| 1.587  | <a href="#">NdFeAsO</a>                                                                          | $Cmme$ (67)      | $P_{A2}/c$ (13.73)       | $2/m1'$   | ×        | ×   |
| 1.588  | <a href="#">NdFeAsO</a>                                                                          | $Cmme$ (67)      | $I_{bcu}$ (73.553)       | $mmm1'$   | ×        | ×   |
| 1.589  | <a href="#">Fe<sub>0.967</sub>Nb<sub>3</sub>S<sub>6</sub></a>                                    | $P6_322$ (182)   | $P_{c2_12_12}$ (18.21)   | $2221'$   | G-woP    | ×   |
| 1.590  | <a href="#">Pb<sub>0.8</sub>Bi<sub>0.2</sub>Fe<sub>0.728</sub>W<sub>0.308</sub>O<sub>6</sub></a> | $Pm3m$ (221)     | $I_{c4}/mcm$ (140.550)   | $4/mmm1'$ | ×        | ×   |
| 1.591  | <a href="#">Pb<sub>0.7</sub>Bi<sub>0.3</sub>Fe<sub>0.762</sub>W<sub>0.308</sub>O<sub>6</sub></a> | $Pm3m$ (221)     | $I_{c4}/mcm$ (140.550)   | $4/mmm1'$ | ×        | ×   |
| 1.592  | <a href="#">Pb<sub>2</sub>NiOsO<sub>6</sub></a>                                                  | $P2_1/n$ (14)    | $P_{ac}$ (7.27)          | $m1'$     | G-wP     | ×   |
| 1.593  | <a href="#">BaCoSO</a>                                                                           | $Cmcm$ (63)      | $P_{abcm}$ (57.386)      | $mmm1'$   | ×        | ×   |
| 1.594  | <a href="#">BaCoSO</a>                                                                           | $Cmcm$ (63)      | $P_{abcm}$ (57.386)      | $mmm1'$   | ×        | ×   |
| 1.595  | <a href="#">CaCoSO</a>                                                                           | $P6_3mc$ (186)   | $C_{cc}$ (9.40)          | $m1'$     | G-woP    | ×   |
| 1.596  | <a href="#">TbCuSb<sub>2</sub></a>                                                               | $P4/nmm$ (129)   | $P_{S1}$ (2.7)           | $11'$     | ×        | ×   |
| 1.597  | <a href="#">TbCuSb<sub>2</sub></a>                                                               | $P4/nmm$ (129)   | $P_{a2_1}/m$ (11.55)     | $2/m1'$   | ×        | ×   |
| 1.598  | <a href="#">CeIr(In<sub>0.97</sub>Cd<sub>0.03</sub>)<sub>5</sub></a>                             | $P4/mmm$ (123)   | $I_{c4}/mcm$ (140.550)   | $4/mmm1'$ | ×        | ×   |
| 1.599  | <a href="#">DyMn<sub>2</sub>O<sub>5</sub></a>                                                    | $Pbam$ (55)      | $P_{cc}$ (7.28)          | $m1'$     | G-wP     | ×   |
| 1.600  | <a href="#">Bi<sub>4</sub>Fe<sub>5</sub>O<sub>13</sub>F</a>                                      | $P4_2/mbc$ (135) | $P_{C42}/n$ (86.73)      | $4/m1'$   | ×        | ×   |
| 1.601  | <a href="#">Bi<sub>4</sub>Fe<sub>5</sub>O<sub>13</sub>F</a>                                      | $P4_2/mbc$ (135) | $P_{C42}/n$ (86.73)      | $4/m1'$   | ×        | ×   |
| 1.602  | <a href="#">Bi<sub>4</sub>Fe<sub>5</sub>O<sub>13</sub>F</a>                                      | $P4_2/mbc$ (135) | $P_{C42}/n$ (86.73)      | $4/m1'$   | ×        | ×   |

Continued on next page

TABLE S7 – continued from previous page

| BCS-ID | Formula                                                                      | Parent                                     | MSG                                                                        | MPG              | SHG type | LMO |
|--------|------------------------------------------------------------------------------|--------------------------------------------|----------------------------------------------------------------------------|------------------|----------|-----|
| 1.603  | <a href="#">Bi<sub>4</sub>Fe<sub>5</sub>O<sub>13</sub>F</a>                  | <i>P</i> 4 <sub>2</sub> / <i>mbc</i> (135) | <i>P</i> <sub>C</sub> 42/ <i>n</i> (86.73)                                 | 4/ <i>m</i> 1'   | ×        | ×   |
| 1.604  | <a href="#">Bi<sub>4</sub>Fe<sub>5</sub>O<sub>13</sub>F</a>                  | <i>P</i> 4 <sub>2</sub> / <i>mbc</i> (135) | <i>P</i> <sub>C</sub> 42/ <i>n</i> (86.73)                                 | 4/ <i>m</i> 1'   | ×        | ×   |
| 1.605  | <a href="#">Bi<sub>4</sub>Fe<sub>5</sub>O<sub>13</sub>F</a>                  | <i>P</i> 4 <sub>2</sub> / <i>mbc</i> (135) | <i>P</i> <sub>C</sub> 42/ <i>n</i> (86.73)                                 | 4/ <i>m</i> 1'   | ×        | ×   |
| 1.606  | <a href="#">Bi<sub>4</sub>Fe<sub>5</sub>O<sub>13</sub>F</a>                  | <i>P</i> 4 <sub>2</sub> / <i>mbc</i> (135) | <i>P</i> <sub>C</sub> 42/ <i>n</i> (86.73)                                 | 4/ <i>m</i> 1'   | ×        | ×   |
| 1.607  | <a href="#">Bi<sub>4</sub>Fe<sub>5</sub>O<sub>13</sub>F</a>                  | <i>P</i> 4 <sub>2</sub> / <i>mbc</i> (135) | <i>P</i> <sub>C</sub> 42/ <i>n</i> (86.73)                                 | 4/ <i>m</i> 1'   | ×        | ×   |
| 1.608  | <a href="#">Bi<sub>4</sub>Fe<sub>5</sub>O<sub>13</sub>F</a>                  | <i>P</i> 4 <sub>2</sub> / <i>mbc</i> (135) | <i>P</i> <sub>C</sub> 42/ <i>n</i> (86.73)                                 | 4/ <i>m</i> 1'   | ×        | ×   |
| 1.609  | <a href="#">Bi<sub>4</sub>Fe<sub>5</sub>O<sub>13</sub>F</a>                  | <i>P</i> 4 <sub>2</sub> / <i>mbc</i> (135) | <i>P</i> <sub>C</sub> 42/ <i>n</i> (86.73)                                 | 4/ <i>m</i> 1'   | ×        | ×   |
| 1.610  | <a href="#">Bi<sub>4</sub>Fe<sub>5</sub>O<sub>13</sub>F</a>                  | <i>P</i> 4 <sub>2</sub> / <i>mbc</i> (135) | <i>P</i> <sub>C</sub> 42/ <i>n</i> (86.73)                                 | 4/ <i>m</i> 1'   | ×        | ×   |
| 1.611  | <a href="#">Bi<sub>4</sub>Fe<sub>5</sub>O<sub>13</sub>F</a>                  | <i>P</i> 4 <sub>2</sub> / <i>mbc</i> (135) | <i>P</i> <sub>C</sub> 42/ <i>n</i> (86.73)                                 | 4/ <i>m</i> 1'   | ×        | ×   |
| 1.612  | <a href="#">Bi<sub>4</sub>Fe<sub>5</sub>O<sub>13</sub>F</a>                  | <i>P</i> 4 <sub>2</sub> / <i>mbc</i> (135) | <i>P</i> <sub>C</sub> 42/ <i>n</i> (86.73)                                 | 4/ <i>m</i> 1'   | ×        | ×   |
| 1.613  | <a href="#">Bi<sub>4</sub>Fe<sub>5</sub>O<sub>13</sub>F</a>                  | <i>P</i> 4 <sub>2</sub> / <i>mbc</i> (135) | <i>P</i> <sub>C</sub> 42/ <i>n</i> (86.73)                                 | 4/ <i>m</i> 1'   | ×        | ×   |
| 1.614  | <a href="#">Bi<sub>4</sub>Fe<sub>5</sub>O<sub>13</sub>F</a>                  | <i>P</i> 4 <sub>2</sub> / <i>mbc</i> (135) | <i>P</i> <sub>C</sub> 42/ <i>n</i> (86.73)                                 | 4/ <i>m</i> 1'   | ×        | ×   |
| 1.615  | <a href="#">Bi<sub>4</sub>Fe<sub>5</sub>O<sub>13</sub>F</a>                  | <i>P</i> 4 <sub>2</sub> / <i>mbc</i> (135) | <i>P</i> <sub>C</sub> 42/ <i>n</i> (86.73)                                 | 4/ <i>m</i> 1'   | ×        | ×   |
| 1.616  | <a href="#">Bi<sub>4</sub>Fe<sub>5</sub>O<sub>13</sub>F</a>                  | <i>P</i> 4 <sub>2</sub> / <i>mbc</i> (135) | <i>P</i> <sub>C</sub> 42/ <i>n</i> (86.73)                                 | 4/ <i>m</i> 1'   | ×        | ×   |
| 1.617  | <a href="#">LiFe(MoO<sub>4</sub>)<sub>2</sub></a>                            | <i>P</i> 1̄ (2)                            | <i>P</i> <sub>S</sub> 1̄ (2.7)                                             | 11'              | ×        | ×   |
| 1.618  | <a href="#">CoO</a>                                                          | <i>Fm</i> 3̄ <i>m</i> (225)                | <i>C</i> <sub>c</sub> 2/ <i>c</i> (15.90)                                  | 2/ <i>m</i> 1'   | ×        | ×   |
| 1.619  | <a href="#">MnS</a>                                                          | <i>Fm</i> 3̄ <i>m</i> (225)                | <i>C</i> <sub>c</sub> 2/ <i>m</i> (12.63)                                  | 2/ <i>m</i> 1'   | ×        | ×   |
| 1.620  | <a href="#">NdCu<sub>2</sub></a>                                             | <i>Imma</i> (74)                           | <i>P</i> <sub>1</sub> <i>nma</i> (62.456)                                  | <i>mmm</i> 1'    | ×        | ×   |
| 1.621  | <a href="#">La(Fe<sub>0.91</sub>Al<sub>0.09</sub>)<sub>13</sub></a>          | <i>Fm</i> 3̄ <i>c</i> (226)                | <i>P</i> <sub>1</sub> 4/ <i>mcc</i> (124.362)                              | 4/ <i>mmm</i> 1' | ×        | ×   |
| 1.622  | <a href="#">CoGeO<sub>3</sub></a>                                            | <i>C</i> 2/ <i>c</i> (15)                  | <i>P</i> <sub>C</sub> 2 <sub>1</sub> / <i>c</i> (14.84)                    | 2/ <i>m</i> 1'   | ×        | ×   |
| 1.623  | <a href="#">EuMg<sub>2</sub>Bi<sub>2</sub></a>                               | <i>P</i> 3 <i>m</i> 1 (164)                | <i>C</i> <sub>c</sub> 2/ <i>m</i> (12.63)                                  | 2/ <i>m</i> 1'   | ×        | ×   |
| 1.624  | <a href="#">EuSn<sub>2</sub>P<sub>2</sub></a>                                | <i>R</i> 3 <i>m</i> (166)                  | <i>C</i> <sub>c</sub> 2/ <i>m</i> (12.63)                                  | 2/ <i>m</i> 1'   | ×        | ×   |
| 1.625  | <a href="#">Sr<sub>2</sub>Fe<sub>3</sub>S<sub>2</sub>O<sub>3</sub></a>       | <i>Pbam</i> (55)                           | <i>P</i> <sub>6</sub> <i>nma</i> (62.451)                                  | <i>mmm</i> 1'    | ×        | ×   |
| 1.626  | <a href="#">Sr<sub>2</sub>Fe<sub>3</sub>Se<sub>2</sub>O<sub>3</sub></a>      | <i>Pbam</i> (55)                           | <i>C</i> <sub>a</sub> <i>mc</i> 2 <sub>1</sub> (36.178)                    | <i>mm</i> 21'    | G-wP     | ×   |
| 1.627  | <a href="#">KCeS<sub>2</sub></a>                                             | <i>R</i> 3 <i>m</i> (166)                  | <i>C</i> <sub>c</sub> 2/ <i>c</i> (15.90)                                  | 2/ <i>m</i> 1'   | ×        | ×   |
| 1.628  | <a href="#">PrMnSi<sub>2</sub></a>                                           | <i>Cmcm</i> (63)                           | <i>P</i> <sub>B</sub> <i>nna</i> (52.318)                                  | <i>mmm</i> 1'    | ×        | ×   |
| 1.629  | <a href="#">FeGe</a>                                                         | <i>P</i> 6/ <i>mmm</i> (191)               | <i>P</i> <sub>6</sub> 6/ <i>mcc</i> (192.252)                              | 6/ <i>mmm</i> 1' | ×        | ×   |
| 1.630  | <a href="#">LuMn<sub>6</sub>Sn<sub>6</sub></a>                               | <i>P</i> 6/ <i>mmm</i> (191)               | <i>C</i> <sub>e</sub> <i>mcm</i> (63.466)                                  | <i>mmm</i> 1'    | ×        | ×   |
| 1.631  | <a href="#">YMn<sub>6</sub>Ge<sub>6</sub></a>                                | <i>P</i> 6/ <i>mmm</i> (191)               | <i>P</i> <sub>6</sub> 6/ <i>mcc</i> (192.252)                              | 6/ <i>mmm</i> 1' | ×        | ×   |
| 1.632  | <a href="#">ErFe<sub>6</sub>Ge<sub>6</sub></a>                               | <i>Immm</i> (71)                           | <i>P</i> <sub>1</sub> <i>nnn</i> (48.264)                                  | <i>mmm</i> 1'    | ×        | ×   |
| 1.633  | <a href="#">YFe<sub>6</sub>Sn<sub>6</sub></a>                                | <i>Immm</i> (71)                           | <i>P</i> <sub>1</sub> <i>nnn</i> (48.264)                                  | <i>mmm</i> 1'    | ×        | ×   |
| 1.634  | <a href="#">YFe<sub>6</sub>Ge<sub>6</sub></a>                                | <i>Cmcm</i> (63)                           | <i>P</i> <sub>B</sub> <i>nna</i> (52.318)                                  | <i>mmm</i> 1'    | ×        | ×   |
| 1.635  | <a href="#">ErFe<sub>2</sub>Si<sub>2</sub></a>                               | <i>I</i> 4/ <i>mmm</i> (139)               | <i>P</i> <sub>a</sub> <i>nma</i> (62.450)                                  | <i>mmm</i> 1'    | ×        | ×   |
| 1.636  | <a href="#">ErMn<sub>2</sub>Si<sub>2</sub></a>                               | <i>I</i> 4/ <i>mmm</i> (139)               | <i>P</i> <sub>1</sub> 4/ <i>nnc</i> (126.386)                              | 4/ <i>mmm</i> 1' | ×        | ×   |
| 1.637  | <a href="#">ErMn<sub>2</sub>Si<sub>2</sub></a>                               | <i>I</i> 4/ <i>mmm</i> (139)               | <i>P</i> <sub>1</sub> 4/ <i>nnc</i> (126.386)                              | 4/ <i>mmm</i> 1' | ×        | ×   |
| 1.638  | <a href="#">ErMn<sub>2</sub>Ge<sub>2</sub></a>                               | <i>I</i> 4/ <i>mmm</i> (139)               | <i>P</i> <sub>1</sub> 4/ <i>nnc</i> (126.386)                              | 4/ <i>mmm</i> 1' | ×        | ×   |
| 1.639  | <a href="#">ErMn<sub>2</sub>Ge<sub>2</sub></a>                               | <i>I</i> 4/ <i>mmm</i> (139)               | <i>P</i> <sub>1</sub> 4/ <i>nnc</i> (126.386)                              | 4/ <i>mmm</i> 1' | ×        | ×   |
| 1.640  | <a href="#">ErMn<sub>2</sub>Ge<sub>2</sub></a>                               | <i>I</i> 4/ <i>mmm</i> (139)               | <i>P</i> <sub>1</sub> 4/ <i>nnc</i> (126.386)                              | 4/ <i>mmm</i> 1' | ×        | ×   |
| 1.641  | <a href="#">Ba<sub>2</sub>FeSi<sub>2</sub>O<sub>7</sub></a>                  | <i>P</i> 4 <sub>2</sub> 1 <i>m</i> (113)   | <i>C</i> <sub>e</sub> <i>mc</i> 2 <sub>1</sub> (36.177)                    | <i>mm</i> 21'    | G-woP    | ×   |
| 1.642  | <a href="#">TlFeS<sub>2</sub></a>                                            | <i>C</i> 2/ <i>m</i> (12)                  | <i>C</i> <sub>c</sub> 2/ <i>m</i> (12.63)                                  | 2/ <i>m</i> 1'   | ×        | ×   |
| 1.643  | <a href="#">DyOCl</a>                                                        | <i>P</i> 4/ <i>nmm</i> (129)               | <i>P</i> <sub>a</sub> <i>nma</i> (62.450)                                  | <i>mmm</i> 1'    | ×        | ×   |
| 1.644  | <a href="#">EuSn<sub>2</sub>As<sub>2</sub></a>                               | <i>R</i> 3 <i>m</i> (166)                  | <i>C</i> <sub>c</sub> 2/ <i>m</i> (12.63)                                  | 2/ <i>m</i> 1'   | ×        | ×   |
| 1.645  | <a href="#">Na<sub>2</sub>Co<sub>2</sub>TeO<sub>6</sub></a>                  | <i>P</i> 6 <sub>3</sub> 22 (182)           | <i>P</i> <sub>C</sub> 2 <sub>1</sub> 2 <sub>1</sub> 2 <sub>1</sub> (19.29) | 2221'            | G-woP    | ×   |
| 1.646  | <a href="#">Na<sub>2</sub>Ni<sub>2</sub>TeO<sub>6</sub></a>                  | <i>P</i> 6 <sub>3</sub> / <i>mcm</i> (193) | <i>I</i> <sub>a</sub> <i>mm</i> 2 (44.234)                                 | <i>mm</i> 21'    | G-wP     | ×   |
| 1.647  | <a href="#">Na<sub>2.4</sub>Ni<sub>2</sub>TeO<sub>6</sub></a>                | <i>P</i> 6 <sub>3</sub> / <i>mcm</i> (193) | <i>P</i> <sub>A</sub> <i>nma</i> (62.453)                                  | <i>mmm</i> 1'    | ×        | ×   |
| 1.648  | <a href="#">Nd<sub>2</sub>O<sub>3</sub></a>                                  | <i>P</i> 3̄ <i>m</i> 1 (164)               | <i>C</i> <sub>c</sub> 2/ <i>m</i> (12.63)                                  | 2/ <i>m</i> 1'   | ×        | ×   |
| 1.649  | <a href="#">Sr<sub>3</sub>ZnIrO<sub>6</sub></a>                              | <i>R</i> 3̄ <i>c</i> (167)                 | <i>P</i> <sub>C</sub> 2/ <i>c</i> (13.74)                                  | 2/ <i>m</i> 1'   | ×        | ×   |
| 1.650  | <a href="#">DyBaCuO<sub>5</sub></a>                                          | <i>P</i> <i>nma</i> (62)                   | <i>P</i> <sub>a</sub> 2 <sub>1</sub> / <i>c</i> (14.80)                    | 2/ <i>m</i> 1'   | ×        | ×   |
| 1.651  | <a href="#">HoBaCuO<sub>5</sub></a>                                          | <i>P</i> <i>nma</i> (62)                   | <i>P</i> <sub>a</sub> 2 <sub>1</sub> / <i>c</i> (14.80)                    | 2/ <i>m</i> 1'   | ×        | ×   |
| 1.652  | <a href="#">Tb<sub>2</sub>Ni<sub>1.78</sub>In</a>                            | <i>P</i> /4 <i>mbm</i> (127)               | <i>C</i> <sub>a</sub> <i>mca</i> (64.479)                                  | <i>mmm</i> 1'    | ×        | ×   |
| 1.653  | <a href="#">FeWO<sub>4</sub></a>                                             | <i>P</i> 2/ <i>c</i> (13)                  | <i>P</i> <sub>a</sub> 2/ <i>c</i> (13.70)                                  | 2/ <i>m</i> 1'   | ×        | ×   |
| 1.654  | <a href="#">NiNb<sub>2</sub>O<sub>6</sub></a>                                | <i>Pbcn</i> (60)                           | <i>P</i> <sub>b</sub> 2 <sub>1</sub> / <i>c</i> (14.81)                    | 2/ <i>m</i> 1'   | ×        | ×   |
| 1.655  | <a href="#">FeNb<sub>2</sub>O<sub>6</sub></a>                                | <i>Pbcn</i> (60)                           | <i>P</i> <sub>c</sub> 2 <sub>1</sub> 2 <sub>1</sub> 2 <sub>1</sub> (19.28) | 2221'            | G-wP     | ×   |
| 1.656  | <a href="#">CoNb<sub>2</sub>O<sub>6</sub></a>                                | <i>Pbcn</i> (60)                           | <i>P</i> <sub>a</sub> 2 <sub>1</sub> / <i>c</i> (14.80)                    | 2/ <i>m</i> 1'   | ×        | ×   |
| 1.657  | <a href="#">LuNiO<sub>3</sub></a>                                            | <i>P</i> 2 <sub>1</sub> / <i>n</i> (14)    | <i>P</i> <sub>a</sub> 2 <sub>1</sub> (4.10)                                | 21'              | G-wP     | ×   |
| 1.658  | <a href="#">DyGa<sub>3</sub></a>                                             | <i>R</i> 3 <i>m</i> (166)                  | <i>C</i> <sub>c</sub> 2/ <i>c</i> (15.90)                                  | 2/ <i>m</i> 1'   | ×        | ×   |
| 1.659  | <a href="#">MnCl<sub>2</sub>(CO(NH<sub>2</sub>)<sub>2</sub>)<sub>2</sub></a> | <i>P</i> ba2 (45)                          | <i>P</i> <sub>1</sub> <i>ca</i> 2 <sub>1</sub> (29.110)                    | <i>mm</i> 21'    | G-woP    | ×   |

Continued on next page

TABLE S7 – continued from previous page

| BCS-ID | Formula                                                              | Parent             | MSG                     | MPG         | SHG type | LMO |
|--------|----------------------------------------------------------------------|--------------------|-------------------------|-------------|----------|-----|
| 1.660  | FePb <sub>4</sub> Sb <sub>6</sub> S <sub>14</sub>                    | $P2_1/c$ (14)      | $P_a2_1/c$ (14.80)      | $2/m1'$     | ×        | ×   |
| 1.661  | La <sub>2</sub> NiIrO <sub>6</sub>                                   | $P2_1/n$ (14)      | $P_S\bar{1}$ (2.7)      | $11'$       | ×        | ×   |
| 1.662  | La <sub>2</sub> NiIrO <sub>6</sub>                                   | $P2_1/n$ (14)      | $P_S\bar{1}$ (2.7)      | $\bar{1}1'$ | ×        | ×   |
| 1.663  | Tb <sub>2</sub> Ni <sub>2</sub> In                                   | $Cmmm$ (65)        | $C_a2/m$ (12.64)        | $2/m1'$     | ×        | ×   |
| 2.1    | EuFe <sub>2</sub> As <sub>2</sub>                                    | $I4/mmm$ (139)     | $P_Cbca$ (61.439)       | $mmm1'$     | ×        | ×   |
| 2.2    | Sr <sub>2</sub> F <sub>2</sub> Fe <sub>2</sub> OS <sub>2</sub>       | $I4/mmm$ (139)     | $C_a2/m$ (12.64)        | $2/m1'$     | ×        | ×   |
| 2.3    | HoNiO <sub>3</sub>                                                   | $P2_1/n$ (14)      | $P2_1$ (4.7)            | 2           | O-wP     | ✓   |
| 2.4    | Eu(Fe <sub>0.82</sub> Co <sub>0.18</sub> )As <sub>2</sub>            | $I4/mmm$ (139)     | $Cmm'm'$ (65.486)       | $m'm'm$     | ×        | ✓   |
| 2.5    | Mn <sub>3</sub> CuN                                                  | $Pm\bar{3}m$ (221) | $P4/n$ (85.59)          | $4/m$       | ×        | ✓   |
| 2.6    | Nd <sub>2</sub> CuO <sub>4</sub>                                     | $I4/mmm$ (139)     | $P_C4_2/nmm$ (134.481)  | $4/mmm1'$   | ×        | ×   |
| 2.7    | Sm <sub>2</sub> CuO <sub>4</sub>                                     | $I4/mmm$ (139)     | $P_C4_2/ncm$ (138.529)  | $4/mmm1'$   | ×        | ×   |
| 2.8    | SrHo <sub>2</sub> O <sub>4</sub>                                     | $Pnam$ (62)        | $P2_1/c'$ (14.78)       | $2/m'$      | PT-wP    | ×   |
| 2.9    | Ca <sub>3</sub> CuNi <sub>2</sub> (PO <sub>4</sub> ) <sub>4</sub>    | $C2/c$ (15)        | $C_a2/c$ (15.91)        | $2/m1'$     | ×        | ×   |
| 2.1    | HoP                                                                  | $Fm\bar{3}m$ (225) | $C2'/c'$ (15.89)        | $2'/m'$     | ×        | ✓   |
| 2.11   | TbMg                                                                 | $Pm\bar{3}m$ (221) | $Pmm'a'$ (51.295)       | $m'm'm$     | ×        | ✓   |
| 2.12   | TbMg                                                                 | $Pm\bar{3}m$ (221) | $Pc'cm'$ (49.270)       | $m'm'm$     | ×        | ✓   |
| 2.13   | UP                                                                   | $Fm\bar{3}m$ (225) | $P_C4_2/nmm$ (134.481)  | $4/mmm1'$   | ×        | ×   |
| 2.14   | NdMg                                                                 | $Pm\bar{3}m$ (221) | $P_C4/nbm$ (125.373)    | $4/mmm1'$   | ×        | ×   |
| 2.15   | Mn <sub>3</sub> Ni <sub>2</sub> O <sub>6</sub>                       | $Fm\bar{3}m$ (225) | $Cmm'm'$ (65.486)       | $m'm'm$     | ×        | ✓   |
| 2.16   | Ce <sub>2</sub> PdGe <sub>3</sub>                                    | $P4_2/mmc$ (131)   | $Pm'$ (6.20)            | $m'$        | BW-wP    | ✓   |
| 2.17   | Pb <sub>2</sub> Mn <sub>0.6</sub> Co <sub>0.4</sub> WO <sub>6</sub>  | $Pm\bar{c}n$ (62)  | $Pm'c_2'$ (26.68)       | $m'm2'$     | BW-wP    | ✓   |
| 2.18   | Sc <sub>2</sub> NiMnO <sub>6</sub>                                   | $P2_1/c$ (14)      | $P_S\bar{1}$ (2.7)      | $\bar{1}1'$ | ×        | ×   |
| 2.19   | Mn <sub>3</sub> ZnC                                                  | $Pm\bar{3}m$ (221) | $I4/mm'm'$ (139.537)    | $4/mm'm'$   | ×        | ✓   |
| 2.20   | UAs                                                                  | $Fm\bar{3}m$ (225) | $P_C4_2/nmm$ (134.481)  | $4/mmm1'$   | ×        | ×   |
| 2.21   | TbOOH                                                                | $P2_1/m$ (11)      | $P2_1/c'$ (14.78)       | $2/m'$      | PT-wP    | ×   |
| 2.22   | FeTa <sub>2</sub> O <sub>6</sub>                                     | $P4_2/nmm$ (136)   | $I_{c4_1}/a$ (88.86)    | $4/m1'$     | ×        | ×   |
| 2.23   | Sr <sub>2</sub> CoO <sub>2</sub> Ag <sub>2</sub> Se <sub>2</sub>     | $I4/mmm$ (139)     | $P_C4_2/n$ (86.73)      | $4/m1'$     | ×        | ×   |
| 2.24   | Ba <sub>2</sub> CoO <sub>2</sub> Ag <sub>2</sub> Se <sub>2</sub>     | $I4/mmm$ (139)     | $P_C4_2/n$ (86.73)      | $4/m1'$     | ×        | ×   |
| 2.25   | Sr <sub>2</sub> CoOsO <sub>6</sub>                                   | $I2/m$ (12)        | $P_S\bar{1}$ (2.7)      | $11'$       | ×        | ×   |
| 2.26   | PrCo <sub>2</sub> P <sub>2</sub>                                     | $I4/mmm$ (139)     | $P4/mm'm'$ (123.345)    | $4/mm'm'$   | ×        | ✓   |
| 2.27   | Sr <sub>2</sub> Mn <sub>3</sub> Sb <sub>2</sub> O <sub>2</sub>       | $I4/mmm$ (139)     | $Cm'cn$ (63.459)        | $m'mm$      | PT-wP    | ×   |
| 2.28   | NpNiGa <sub>5</sub>                                                  | $P4/mmm$ (123)     | $Imm'a'$ (74.559)       | $m'm'm$     | ×        | ✓   |
| 2.29   | Mn <sub>3</sub> O <sub>4</sub>                                       | $I4_1/amd$ (141)   | $Pb'c'n$ (60.422)       | $m'm'm$     | ×        | ✓   |
| 2.30   | CeRh <sub>2</sub> Si <sub>2</sub>                                    | $I4/mmm$ (139)     | $P_Bcca$ (54.350)       | $mmm1'$     | ×        | ×   |
| 2.31   | Mn <sub>3</sub> ZnN                                                  | $Pm\bar{3}m$ (221) | $Pb\bar{c}n$ (60.432)   | $mmm1'$     | ×        | ×   |
| 2.32   | Dy <sub>3</sub> Ru <sub>4</sub> Al <sub>12</sub>                     | $P6_3/mmc$ (194)   | $P3c'1$ (165.95)        | $3m'$       | ×        | ✓   |
| 2.33   | Na <sub>2</sub> Mn <sub>3</sub> Se <sub>4</sub>                      | $C2/m$ (12)        | $P_S\bar{1}$ (2.7)      | $\bar{1}1'$ | ×        | ×   |
| 2.34   | La <sub>0.25</sub> Pr <sub>0.75</sub> Co <sub>2</sub> P <sub>2</sub> | $I4/mmm$ (139)     | $C2'/m'$ (12.62)        | $2'/m'$     | ×        | ✓   |
| 2.35   | CrSe                                                                 | $P6_3/mmc$ (194)   | $P31m'$ (157.55)        | $3m'$       | BW-wP    | ✓   |
| 2.36   | TbGe <sub>3</sub>                                                    | $Cmcm$ (63)        | $P_cnma$ (62.452)       | $mmm1'$     | ×        | ×   |
| 2.37   | La <sub>8</sub> Cu <sub>7</sub> O <sub>19</sub>                      | $C2/c$ (15)        | $P_S\bar{1}$ (2.7)      | $11'$       | ×        | ×   |
| 2.38   | Pb <sub>2</sub> MnWO <sub>6</sub>                                    | $Pmc2_1$ (26)      | $Pmn2_1$ (31.123)       | $mm2$       | O-woP    | ×   |
| 2.39   | LaCaFeO <sub>4</sub>                                                 | $I4/mmm$ (139)     | $P_C4_2/ncm$ (138.529)  | $4/mmm1'$   | ×        | ×   |
| 2.40   | LaBaFeO <sub>4</sub>                                                 | $I4/mmm$ (139)     | $P_C4_2/ncm$ (138.529)  | $4/mmm1'$   | ×        | ×   |
| 2.41   | LaSrFeO <sub>4</sub>                                                 | $I4/mmm$ (139)     | $P_C4_2/ncm$ (138.529)  | $4/mmm1'$   | ×        | ×   |
| 2.42   | LaSrFeO <sub>4</sub>                                                 | $I4/mmm$ (139)     | $P_C4_2/nmm$ (134.481)  | $4/mmm1'$   | ×        | ×   |
| 2.43   | Fe <sub>2</sub> MnBO <sub>5</sub>                                    | $Pbam$ (55)        | $Pb'am'$ (55.358)       | $m'm'm$     | ×        | ✓   |
| 2.44   | KCuMnS <sub>2</sub>                                                  | $I4/mmm$ (139)     | $P_C4/mmm$ (123.349)    | $4/mmm1'$   | ×        | ×   |
| 2.45   | Pb <sub>2</sub> BaCuFeO <sub>5</sub> Br                              | $P4/mmm$ (123)     | $P_C2$ (3.6)            | $21'$       | G-wP     | ×   |
| 2.46   | Pb <sub>2</sub> BaCuFeO <sub>5</sub> Cl                              | $P4/mmm$ (123)     | $P_C2$ (3.6)            | $21'$       | G-wP     | ×   |
| 2.47   | Y <sub>2</sub> SrCuFeO <sub>6.5</sub>                                | $Ibam$ (72)        | $Pc'c'n$ (56.369)       | $m'm'm$     | ×        | ✓   |
| 2.48   | Pr <sub>2</sub> CuO <sub>4</sub>                                     | $I4/mmm$ (139)     | $P_C4_2/nmm$ (134.481)  | $4/mmm1'$   | ×        | ×   |
| 2.49   | La <sub>2</sub> O <sub>2</sub> Fe <sub>2</sub> OSe <sub>2</sub>      | $I4/mmm$ (139)     | $C_a2/m$ (12.64)        | $2/m1'$     | ×        | ×   |
| 2.50   | EuMnBi <sub>2</sub>                                                  | $I4/mmm$ (139)     | $P4_2'/m'm'c$ (131.440) | $4'/m'm'm$  | PT-wP    | ×   |
| 2.51   | EuMnBi <sub>2</sub>                                                  | $I4/mmm$ (139)     | $Pm'n'2_1$ (31.127)     | $m'm'2$     | BW-wP    | ✓   |
| 2.52   | Mn <sub>3</sub> O <sub>4</sub>                                       | $I4_1/amd$ (141)   | $Pc'$ (7.26)            | $m'$        | BW-wP    | ✓   |
| 2.53   | Ba <sub>2</sub> Mn <sub>3</sub> Sb <sub>2</sub> O <sub>2</sub>       | $I4/mmm$ (139)     | $Cm'ma$ (67.503)        | $m'mm$      | PT-wP    | ×   |
| 2.54   | Sr <sub>2</sub> Cr <sub>3</sub> As <sub>2</sub> O <sub>2</sub>       | $I4/mmm$ (139)     | $P_C2_1/c$ (14.84)      | $2/m1'$     | ×        | ×   |

Continued on next page

TABLE S7 – continued from previous page

| BCS-ID | Formula                                                                        | Parent                          | MSG                                             | MPG             | SHG type | LMO |
|--------|--------------------------------------------------------------------------------|---------------------------------|-------------------------------------------------|-----------------|----------|-----|
| 2.55   | <a href="#">Sr<sub>2</sub>Fe<sub>3</sub>Se<sub>2</sub>O<sub>3</sub></a>        | <i>Pbam</i> (55)                | <i>C<sub>2</sub>c</i> (9.40)                    | <i>m1'</i>      | G-wP     | ×   |
| 2.56   | <a href="#">La<sub>2</sub>O<sub>2</sub>Fe<sub>2</sub>OS<sub>2</sub></a>        | <i>I4/mmm</i> (139)             | <i>C<sub>a</sub>2/m</i> (12.64)                 | <i>2/m1'</i>    | ×        | ×   |
| 2.57   | <a href="#">TbMn<sub>2</sub>Si<sub>2</sub></a>                                 | <i>I4/mmm</i> (139)             | <i>Pmm'n'</i> (59.410)                          | <i>m'm'm</i>    | ×        | ✓   |
| 2.58   | <a href="#">La<sub>0.73</sub>Tb<sub>0.27</sub>Mn<sub>2</sub>Si<sub>2</sub></a> | <i>I4/mmm</i> (139)             | <i>Pnnm'</i> (58.396)                           | <i>m'mm</i>     | PT-wP    | ×   |
| 2.59   | <a href="#">Mn<sub>3</sub>As<sub>2</sub></a>                                   | <i>C2/m</i> (12)                | <i>C2/c</i> (15.85)                             | <i>2/m</i>      | ×        | ✓   |
| 2.60   | <a href="#">NdMn<sub>2</sub>Si<sub>2</sub></a>                                 | <i>I4/mmm</i> (139)             | <i>Pmm'n'</i> (59.410)                          | <i>m'm'm</i>    | ×        | ✓   |
| 2.61   | <a href="#">Fe<sub>3</sub>F<sub>8</sub>(H<sub>2</sub>O)<sub>2</sub></a>        | <i>C2/m</i> (12)                | <i>C2'/m'</i> (12.62)                           | <i>2'/m'</i>    | ×        | ✓   |
| 2.62   | <a href="#">TbCrO<sub>3</sub></a>                                              | <i>Pbnm</i> (62)                | <i>Pm'n'2<sub>1</sub></i> (31.127)              | <i>m'm'2</i>    | BW-wP    | ✓   |
| 2.63   | <a href="#">DyCrO<sub>3</sub></a>                                              | <i>Pbnm</i> (62)                | <i>P2'<sub>1</sub>/m'</i> (11.54)               | <i>2'/m'</i>    | ×        | ✓   |
| 2.64   | <a href="#">DyCrO<sub>3</sub></a>                                              | <i>Pbnm</i> (62)                | <i>P2'<sub>1</sub>/m'</i> (11.54)               | <i>2'/m'</i>    | ×        | ✓   |
| 2.65   | <a href="#">UPd<sub>2</sub>Si<sub>2</sub></a>                                  | <i>I4/mmm</i> (139)             | <i>P4/mmm'm'</i> (123.345)                      | <i>4/mmm'm'</i> | ×        | ✓   |
| 2.66   | <a href="#">FeSn<sub>2</sub></a>                                               | <i>I4/mcm</i> (140)             | <i>Cc'ca</i> (68.513)                           | <i>m'mm</i>     | PT-wP    | ×   |
| 2.67   | <a href="#">FeSn<sub>2</sub></a>                                               | <i>I4/mcm</i> (140)             | <i>P<sub>C</sub>bcn</i> (60.431)                | <i>mmm1'</i>    | ×        | ×   |
| 2.68   | <a href="#">FeGe<sub>2</sub></a>                                               | <i>I4/mcm</i> (140)             | <i>Pc'cn</i> (56.367)                           | <i>m'mm</i>     | PT-wP    | ×   |
| 2.69   | <a href="#">La<sub>0.5</sub>Ca<sub>0.5</sub>MnO<sub>3</sub></a>                | <i>Pnma</i> (62)                | <i>P<sub>a</sub>2<sub>1</sub>/m</i> (11.55)     | <i>2/m1'</i>    | ×        | ×   |
| 2.70   | <a href="#">GdMg</a>                                                           | <i>Pm3m</i> (221)               | <i>C2'/c'</i> (15.89)                           | <i>2'/m'</i>    | ×        | ✓   |
| 2.71   | <a href="#">HoRh</a>                                                           | <i>Pm3m</i> (221)               | <i>P<sub>C</sub>2<sub>1</sub>/m</i> (11.57)     | <i>2/m1'</i>    | ×        | ×   |
| 2.72   | <a href="#">VNb<sub>3</sub>S<sub>6</sub></a>                                   | <i>P6<sub>3</sub>22</i> (182)   | <i>C2'2'2<sub>1</sub></i> (20.33)               | <i>2'2'2</i>    | BW-woP   | ✓   |
| 2.73   | <a href="#">BaNd<sub>2</sub>ZnO<sub>5</sub></a>                                | <i>I4/mcm</i> (140)             | <i>P<sub>C</sub>4/ncc</i> (130.433)             | <i>4/mmm1'</i>  | ×        | ×   |
| 2.74   | <a href="#">BaDy<sub>2</sub>O<sub>4</sub></a>                                  | <i>Pnma</i> (62)                | <i>P2'<sub>1</sub></i> (4.9)                    | <i>2'</i>       | BW-wP    | ✓   |
| 2.75   | <a href="#">Sr<sub>2</sub>Fe<sub>3</sub>S<sub>2</sub>O<sub>3</sub></a>         | <i>Pbam</i> (55)                | <i>P<sub>A</sub>2<sub>1</sub>/c</i> (14.83)     | <i>2/m1'</i>    | ×        | ×   |
| 2.76   | <a href="#">Sr<sub>2</sub>Fe<sub>3</sub>Se<sub>2</sub>O<sub>3</sub></a>        | <i>Pbam</i> (55)                | <i>C<sub>2</sub>c</i> (9.40)                    | <i>m1'</i>      | G-wP     | ×   |
| 2.77   | <a href="#">Eu<sub>2</sub>CuO<sub>4</sub></a>                                  | <i>I4/mmm</i> (139)             | <i>P<sub>C</sub>4<sub>2</sub>/ncm</i> (138.529) | <i>4/mmm1'</i>  | ×        | ×   |
| 2.78   | <a href="#">Nd<sub>2</sub>CuO<sub>4</sub></a>                                  | <i>I4/mmm</i> (139)             | <i>P<sub>C</sub>4<sub>2</sub>/nnm</i> (134.481) | <i>4/mmm1'</i>  | ×        | ×   |
| 2.79   | <a href="#">Pr<sub>2</sub>CuO<sub>4</sub></a>                                  | <i>I4/mmm</i> (139)             | <i>P<sub>C</sub>4<sub>2</sub>/nnm</i> (134.481) | <i>4/mmm1'</i>  | ×        | ×   |
| 2.80   | <a href="#">ErFe<sub>6</sub>Ge<sub>6</sub></a>                                 | <i>Immm</i> (71)                | <i>Pm'm'n</i> (59.409)                          | <i>m'm'm</i>    | ×        | ✓   |
| 2.81   | <a href="#">ErMn<sub>2</sub>Si<sub>2</sub></a>                                 | <i>I4/mmm</i> (139)             | <i>Pm'm'n</i> (59.409)                          | <i>m'm'm</i>    | ×        | ✓   |
| 2.82   | <a href="#">ErMn<sub>2</sub>Si<sub>2</sub></a>                                 | <i>I4/mmm</i> (139)             | <i>Pm'm'n</i> (59.409)                          | <i>m'm'm</i>    | ×        | ✓   |
| 2.83   | <a href="#">ErMn<sub>2</sub>Ge<sub>2</sub></a>                                 | <i>I4/mmm</i> (139)             | <i>Pm'm'n</i> (59.409)                          | <i>m'm'm</i>    | ×        | ✓   |
| 2.84   | <a href="#">ErMn<sub>2</sub>Ge<sub>2</sub></a>                                 | <i>I4/mmm</i> (139)             | <i>Pm'm'n</i> (59.409)                          | <i>m'm'm</i>    | ×        | ✓   |
| 2.85   | <a href="#">HoBaCuO<sub>5</sub></a>                                            | <i>Pnma</i> (62)                | <i>P2'<sub>1</sub>/c</i> (14.77)                | <i>2'/m</i>     | PT-wP    | ×   |
| 2.86   | <a href="#">FeTa<sub>2</sub>O<sub>6</sub></a>                                  | <i>P4<sub>2</sub>/mnm</i> (136) | <i>I<sub>4</sub>1/a</i> (88.86)                 | <i>4/m1'</i>    | ×        | ×   |
| 3.1    | <a href="#">TmAgGe</a>                                                         | <i>P62m</i> (189)               | <i>P6'2m'</i> (189.224)                         | <i>6'm'2</i>    | BW-woP   | ×   |
| 3.2    | <a href="#">UO<sub>2</sub></a>                                                 | <i>Fm3m</i> (225)               | <i>Pn3m'</i> (224.113)                          | <i>m3m'</i>     | ×        | ×   |
| 3.3    | <a href="#">Ho<sub>2</sub>RhIn<sub>8</sub></a>                                 | <i>P4/mmm</i> (123)             | <i>Cm'cm'</i> (63.464)                          | <i>m'm'm</i>    | ×        | ✓   |
| 3.4    | <a href="#">MgCr<sub>2</sub>O<sub>4</sub></a>                                  | <i>Fd3m</i> (227)               | <i>P42'm'</i> (111.255)                         | <i>42'm'</i>    | BW-wP    | ✓   |
| 3.5    | <a href="#">Fe<sub>0.7</sub>Mn<sub>0.3</sub></a>                               | <i>Fm3m</i> (225)               | <i>Pn3m'</i> (224.113)                          | <i>m3m'</i>     | ×        | ×   |
| 3.6    | <a href="#">DyCu</a>                                                           | <i>Pm3m</i> (221)               | <i>Im3m'</i> (229.143)                          | <i>m3m'</i>     | ×        | ×   |
| 3.7    | <a href="#">NpBi</a>                                                           | <i>Fm3m</i> (225)               | <i>Pn3m'</i> (224.113)                          | <i>m3m'</i>     | ×        | ×   |
| 3.8    | <a href="#">NdZn</a>                                                           | <i>Pm3m</i> (221)               | <i>P<sub>1</sub>n3n</i> (222.103)               | <i>m3m1'</i>    | ×        | ×   |
| 3.9    | <a href="#">NpS</a>                                                            | <i>Fm3m</i> (225)               | <i>F<sub>S</sub>d3c</i> (228.139)               | <i>m3m1'</i>    | ×        | ×   |
| 3.10   | <a href="#">NpSe</a>                                                           | <i>Fm3m</i> (225)               | <i>F<sub>S</sub>d3c</i> (228.139)               | <i>m3m1'</i>    | ×        | ×   |
| 3.11   | <a href="#">NpTe</a>                                                           | <i>Fm3m</i> (225)               | <i>F<sub>S</sub>d3c</i> (228.139)               | <i>m3m1'</i>    | ×        | ×   |
| 3.12   | <a href="#">USb</a>                                                            | <i>Fm3m</i> (225)               | <i>Pn3m'</i> (224.113)                          | <i>m3m'</i>     | ×        | ×   |
| 3.13   | <a href="#">CeB<sub>6</sub></a>                                                | <i>Pm3m</i> (221)               | <i>C<sub>a</sub>mca</i> (64.479)                | <i>mmm1'</i>    | ×        | ×   |
| 3.14   | <a href="#">FeI<sub>2</sub></a>                                                | <i>P3m1</i> (164)               | <i>C2'/m'</i> (12.62)                           | <i>2'/m'</i>    | ×        | ✓   |
| 3.15   | <a href="#">FeI<sub>2</sub></a>                                                | <i>P3m1</i> (164)               | <i>P3m'1</i> (164.89)                           | <i>3m'</i>      | ×        | ✓   |
| 3.16   | <a href="#">Gd<sub>2</sub>Ti<sub>2</sub>O<sub>7</sub></a>                      | <i>Fd3m</i> (227)               | <i>F<sub>S</sub>43m</i> (216.77)                | <i>43m1'</i>    | G-wP     | ×   |
| 3.17   | <a href="#">BaCu<sub>3</sub>V<sub>2</sub>O<sub>8</sub>(OD)<sub>2</sub></a>     | <i>P312<sub>1</sub></i> (152)   | <i>P312'1</i> (152.35)                          | <i>32'</i>      | BW-woP   | ✓   |
| 3.18   | <a href="#">HoRh</a>                                                           | <i>Pm3m</i> (221)               | <i>P<sub>1</sub>a3</i> (205.36)                 | <i>m31'</i>     | ×        | ×   |
| 3.19   | <a href="#">CoO</a>                                                            | <i>Fm3m</i> (225)               | <i>I<sub>c</sub>4<sub>1</sub>/acd</i> (142.570) | <i>4/mmm1'</i>  | ×        | ×   |

- [1] T. Hahn, U. Shmueli, and J. W. Arthur, International tables for crystallography, Vol. 1 (Reidel Dordrecht, 1983).  
[2] S. V. Gallego, J. Etxebarria, L. Elcoro, E. S. Tasci, and J. M. Perez-Mato, *Acta Crystallogr A Found Adv* **75**, 438 (2019).

- [3] A. P. Cracknell, *Phys. Rev. B* **7**, 2145 (1973).
- [4] A. Kirilyuk, *J. Phys. D: Appl. Phys.* **35**, R189 (2002).
- [5] H. Grimmer, *Acta Crystallogr. A* **49**, 763 (1993).
- [6] C. L. Kane and E. J. Mele, *Phys. Rev. Lett.* **95**, 146802 (2005).
- [7] X. Li, T. Cao, Q. Niu, J. Shi, and J. Feng, *P. Natl. Acad. Sci. USA* **110**, 3738 (2013).
- [8] W. Y. Tong, S. J. Gong, X. Wan, and C. G. Duan, *Nat. Commun.* **7**, 13612 (2016).
- [9] Z. Sun, Y. Yi, T. Song, G. Clark, B. Huang, Y. Shan, S. Wu, D. Huang, C. Gao, Z. Chen, M. McGuire, T. Cao, D. Xiao, W. T. Liu, W. Yao, X. Xu, and S. Wu, *Nature* **572**, 497 (2019).
- [10] V. K. Gudelli and G.-Y. Guo, *Chin. J. Phys.* **68**, 896 (2020).
- [11] W. Song, R. Fei, L. Zhu, and L. Yang, *Phys. Rev. B* **102**, 045411 (2020).
- [12] H. Chu, C. J. Roh, J. O. Island, C. Li, S. Lee, J. Chen, J.-G. Park, A. F. Young, J. S. Lee, and D. Hsieh, *Phys. Rev. Lett.* **124**, 027601 (2020).
- [13] Z. Ni, A. V. Haglund, H. Wang, B. Xu, C. Bernhard, D. G. Mandrus, X. Qian, E. J. Mele, C. L. Kane, and L. Wu, *Nat. Nanotechnol.* **16**, 782 (2021).
- [14] R. Fei, W. Song, and L. Yang, *Phys. Rev. B* **102**, 035440 (2020).
- [15] K. Lee, A. H. Dismukes, E. J. Telford, R. A. Wiscons, J. Wang, X. Xu, C. Nuckolls, C. R. Dean, X. Roy, and X. Zhu, *Nano Lett.* **21**, 3511 (2021).
- [16] N. Sivadas, S. Okamoto, and D. Xiao, *Phys. Rev. Lett.* **117**, 267203 (2016).
- [17] A. Taghizadeh, F. Hipolito, and T. G. Pedersen, *Phys. Rev. B* **96**, 195413 (2017).
- [18] A. Muñoz, J. A. Alonso, M. J. Martínez-Lope, M. T. Casáis, J. L. Martínez, and M. T. Fernández-Díaz, *Phys. Rev. B* **62**, 9498 (2000).
- [19] R. R. Birss, *Symmetry and magnetism* (Symmetry and magnetism, 1964).
